# Supplementary material for: Preferential monitoring site location in the Southern California Air Quality Basin
Source: arXiv:2304.10006 source file (2023-04-19)
Supplement: Supplementary file 1 [file 99_AppendixA_POC-plots.tex]

\section{Appendix A: POC plots}
Plots of individual sites and their individual POCs overlayed on boxplots of the whole data for each year.   Inserted map shows location of site as a red dot with the remaining sites in the network in paler pink..

\begin{figure}
    \centering
    \includegraphics[width = \textwidth]{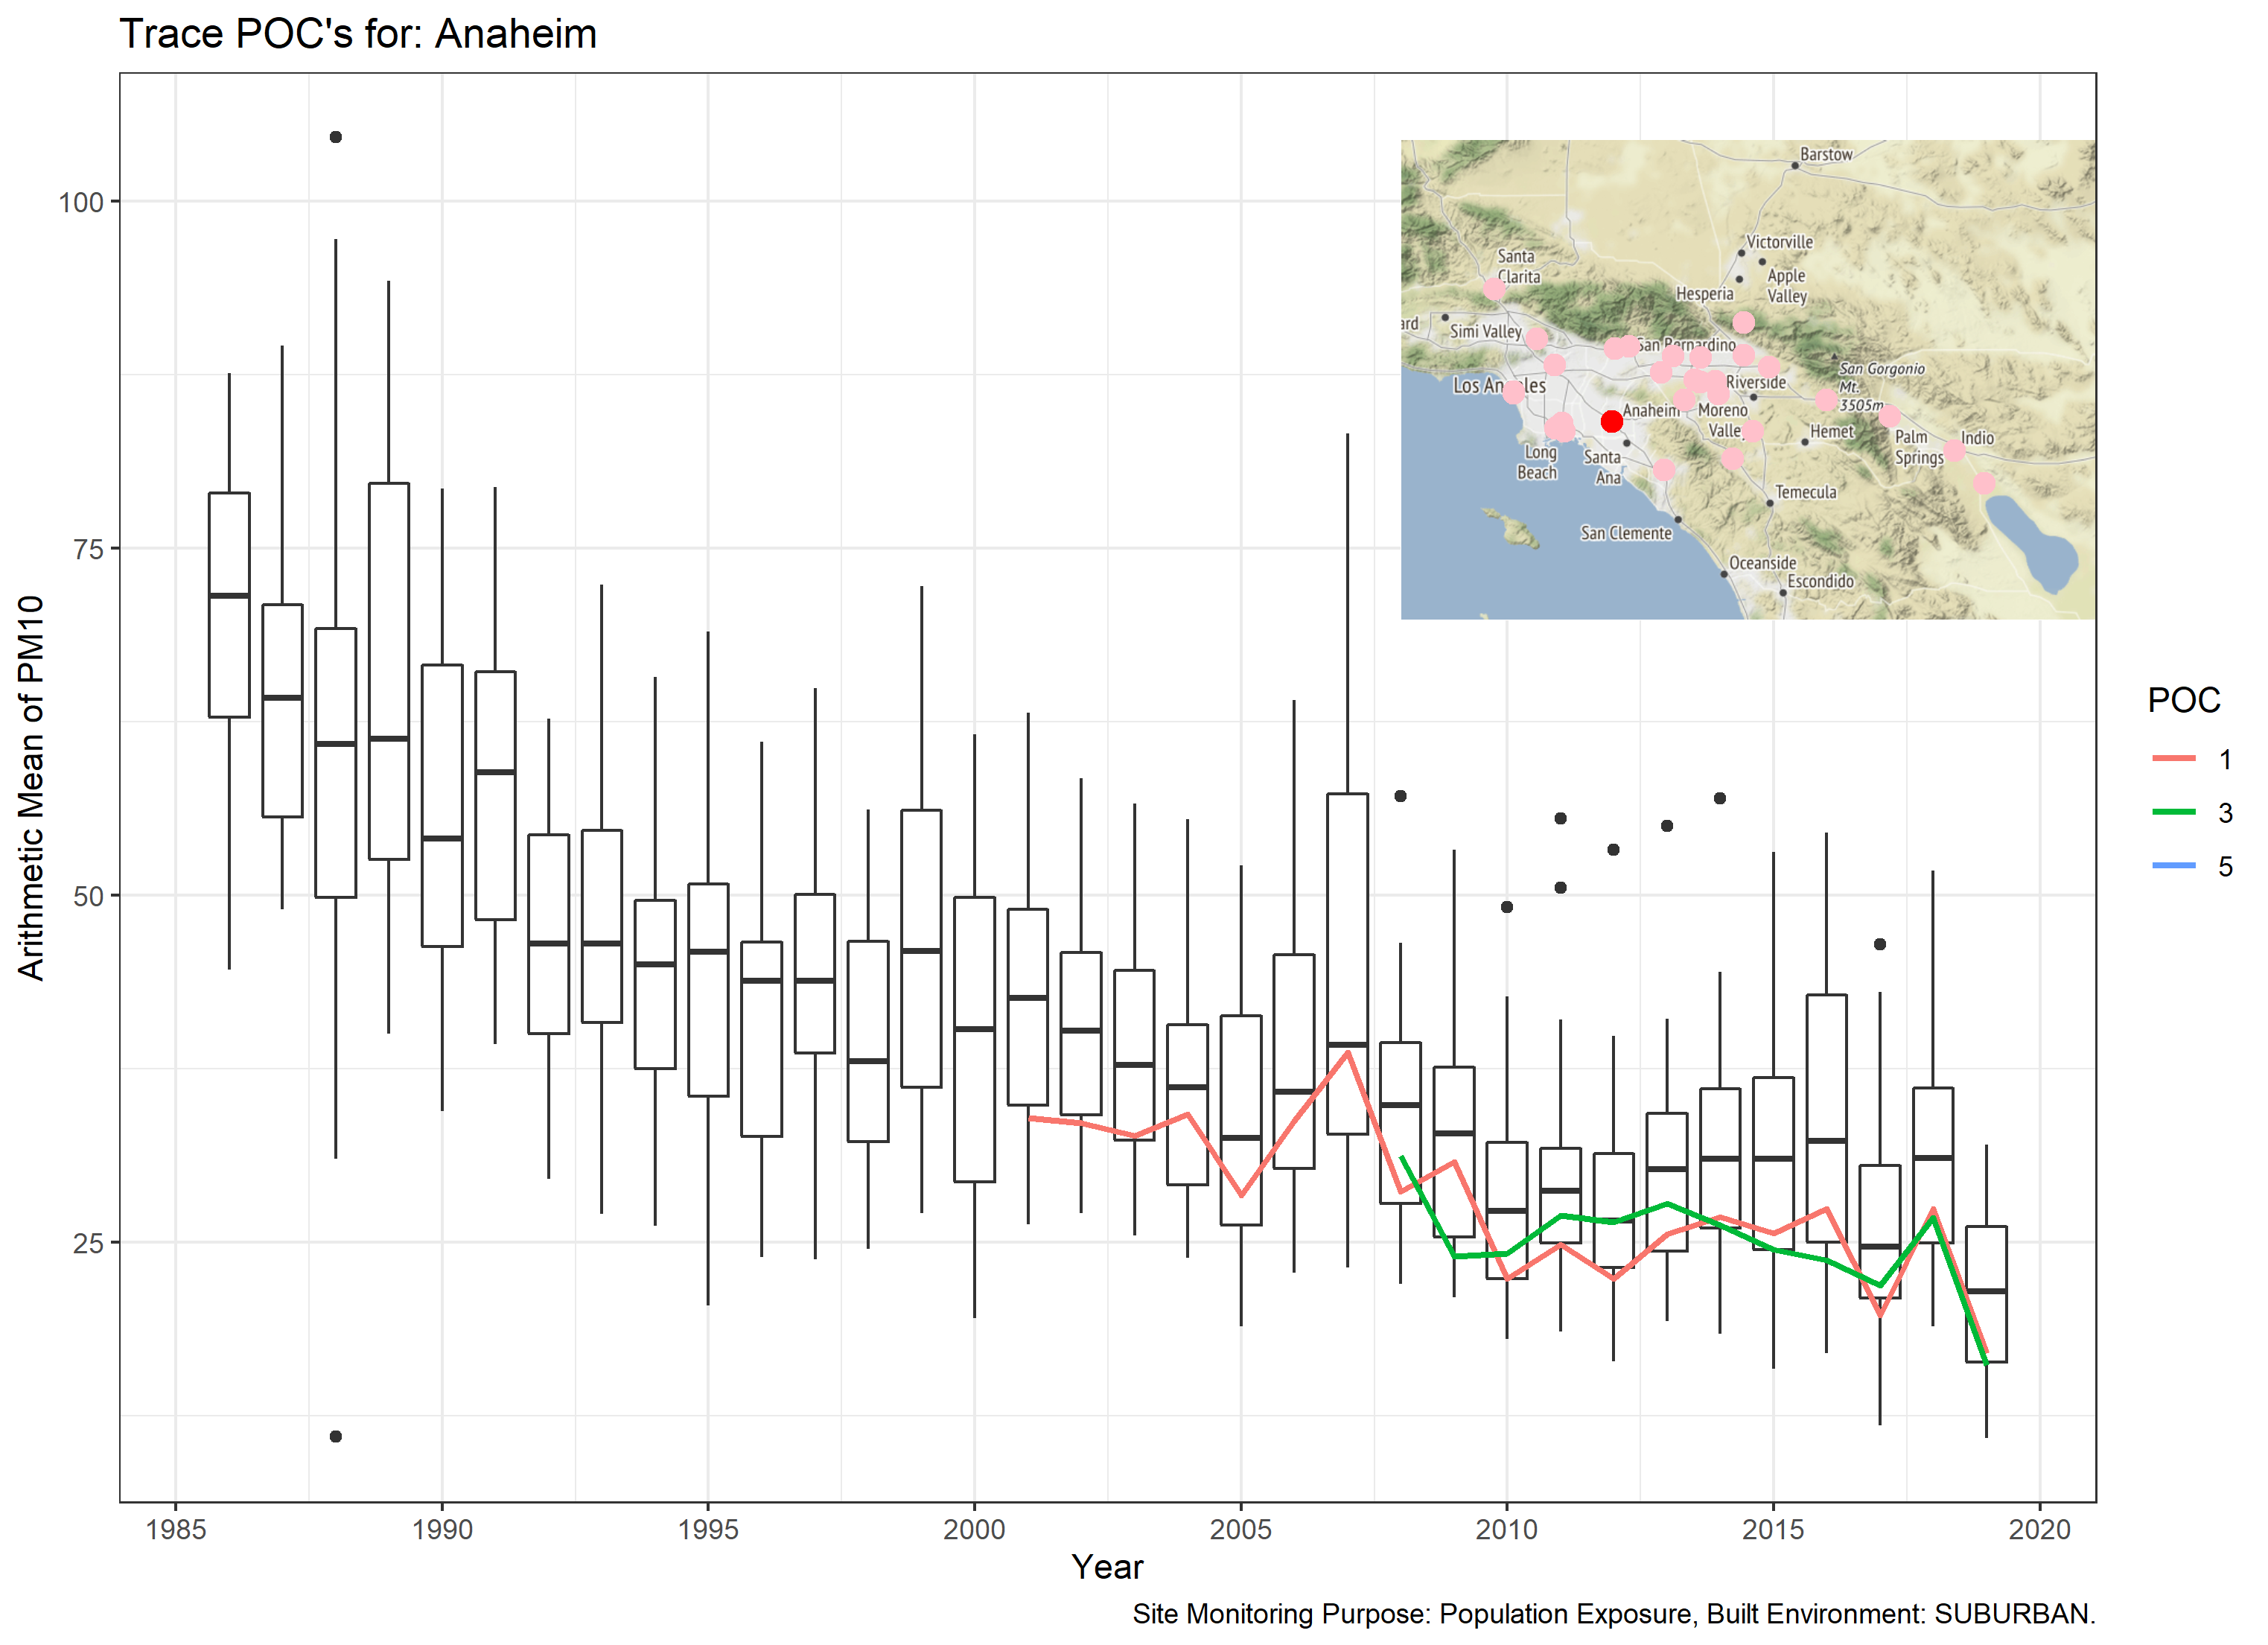}
    \caption{Caption}
    \label{fig:my_label}
\end{figure}

\begin{figure}
    \centering
    \includegraphics[width = \textwidth]{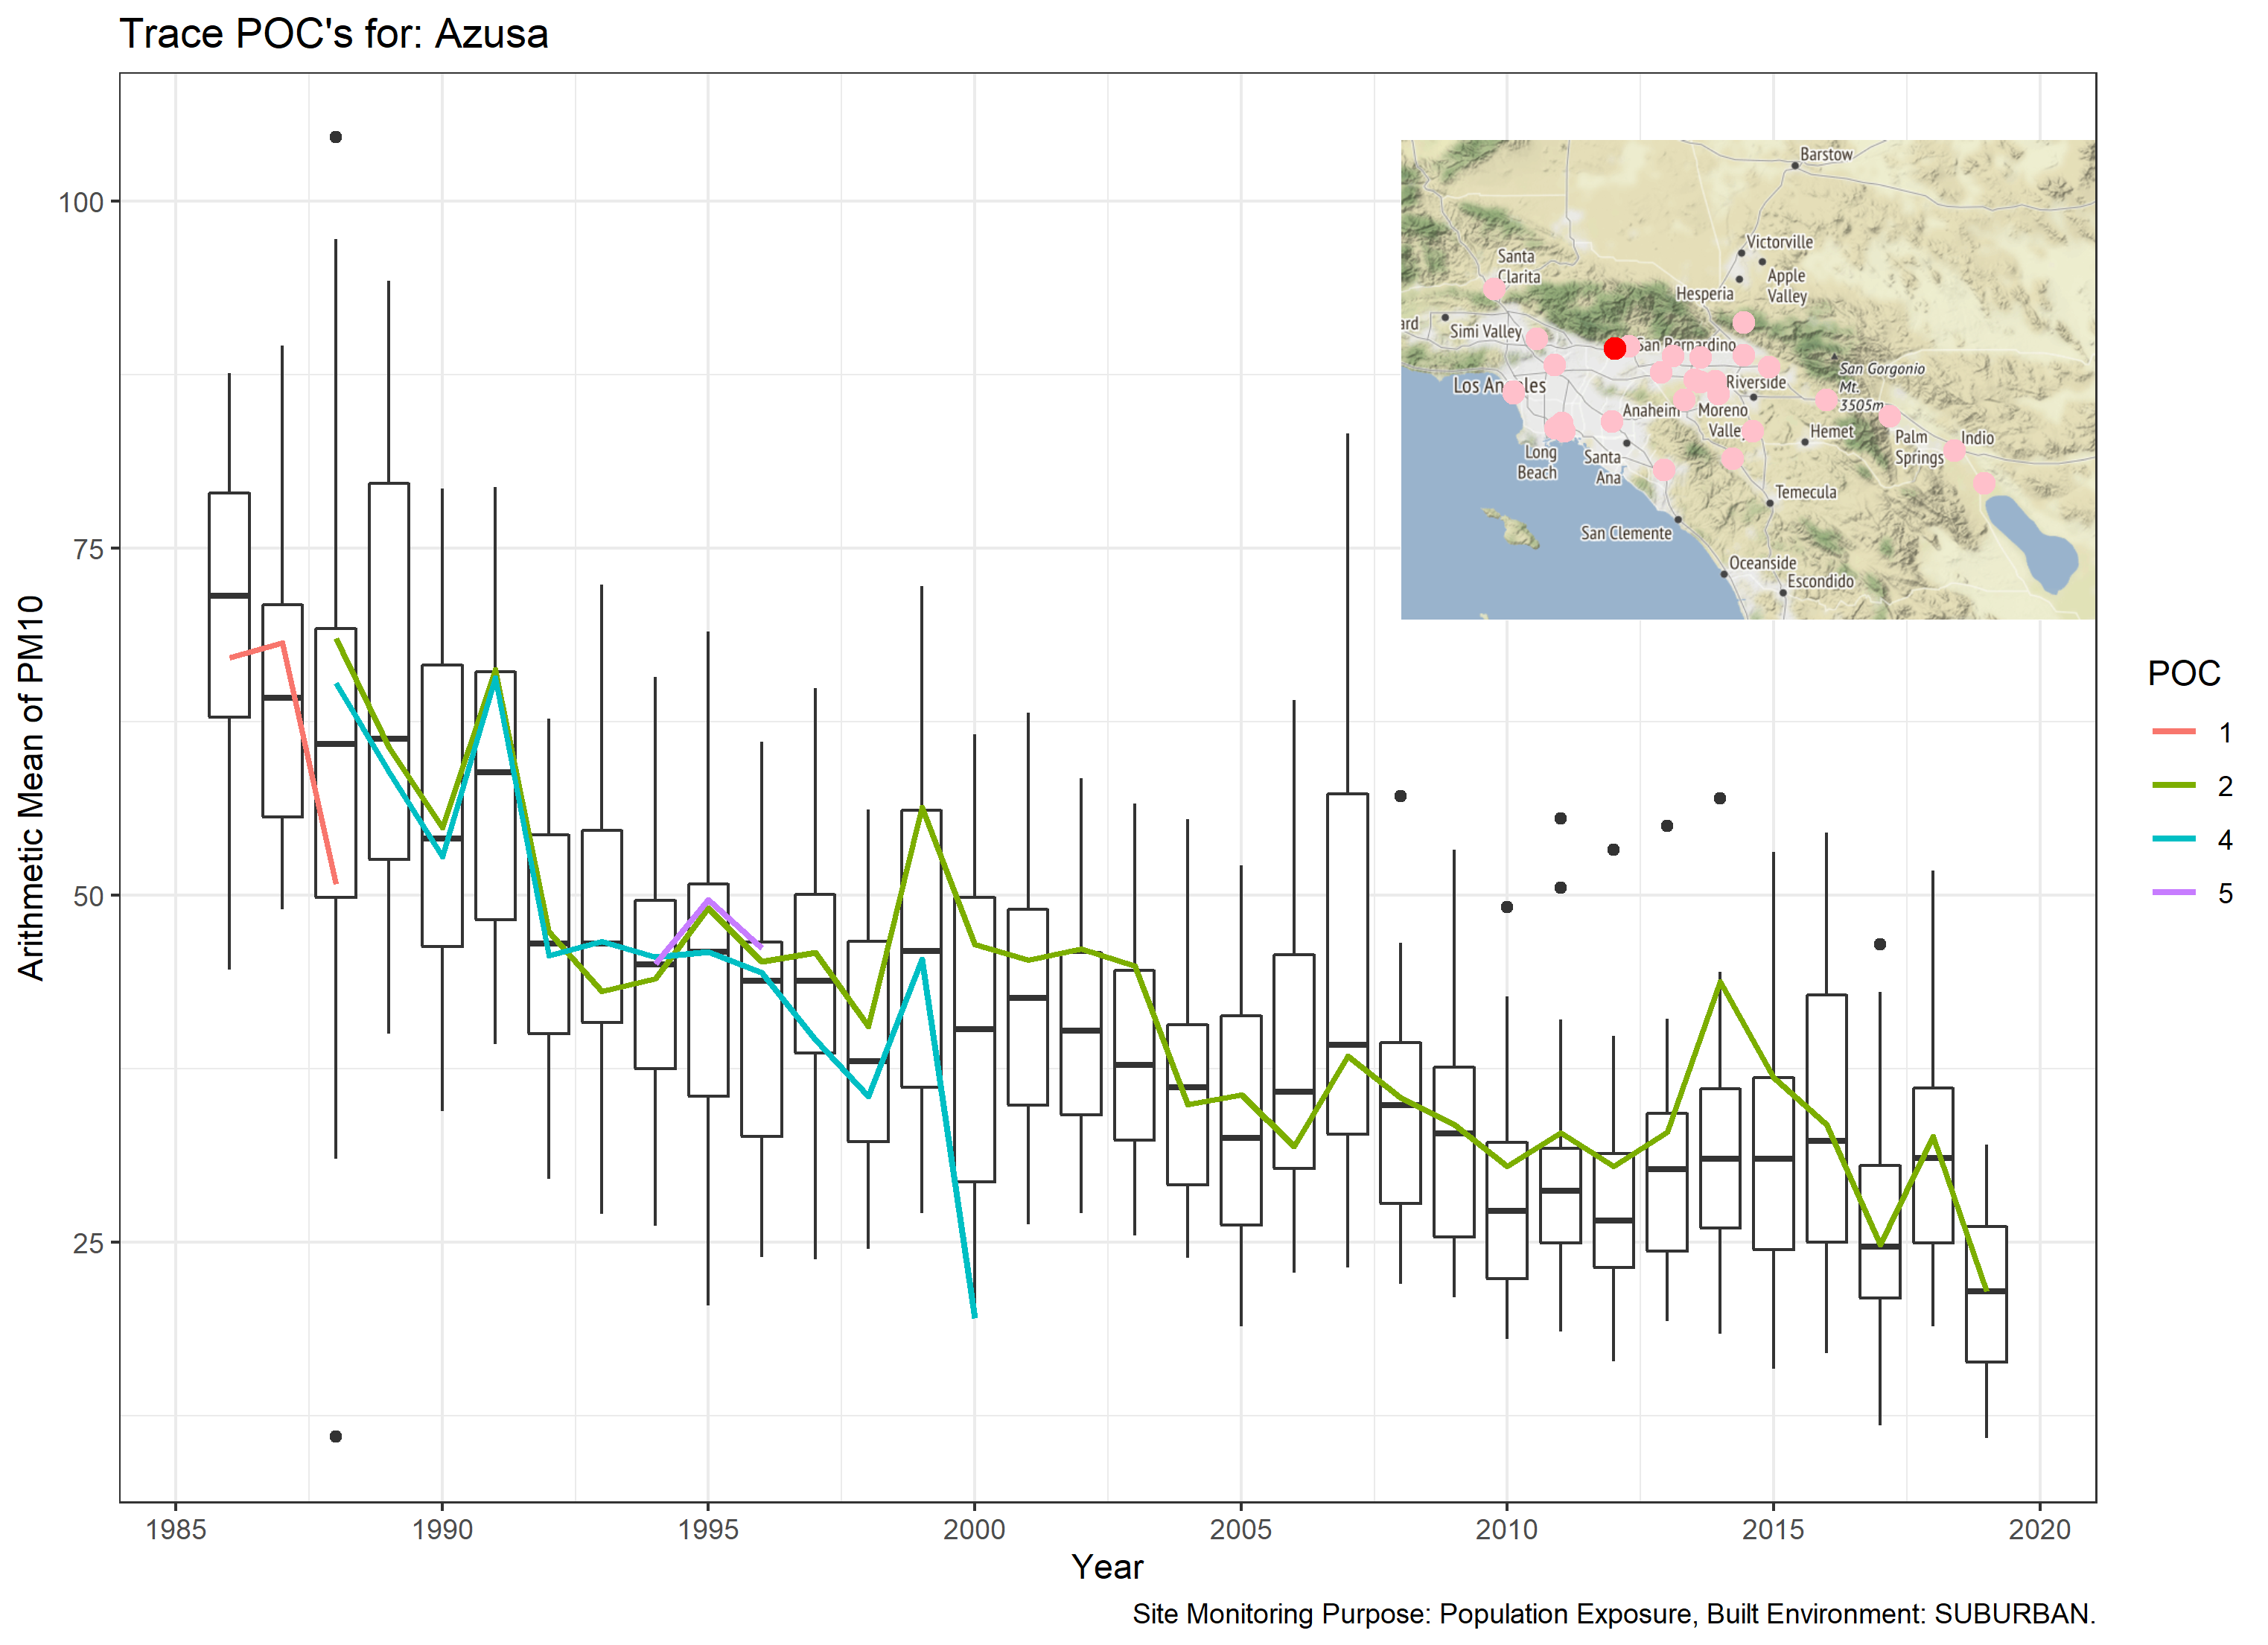}
    \caption{Caption}
    \label{fig:my_label}
\end{figure}

\begin{figure}
    \centering
    \includegraphics[width = \textwidth]{Figures/IndividualSiteTraces/TracePOC_Banning Airport.png}
    \caption{Caption}
    \label{fig:my_label}
\end{figure}

\begin{figure}
    \centering
    \includegraphics[width = \textwidth]{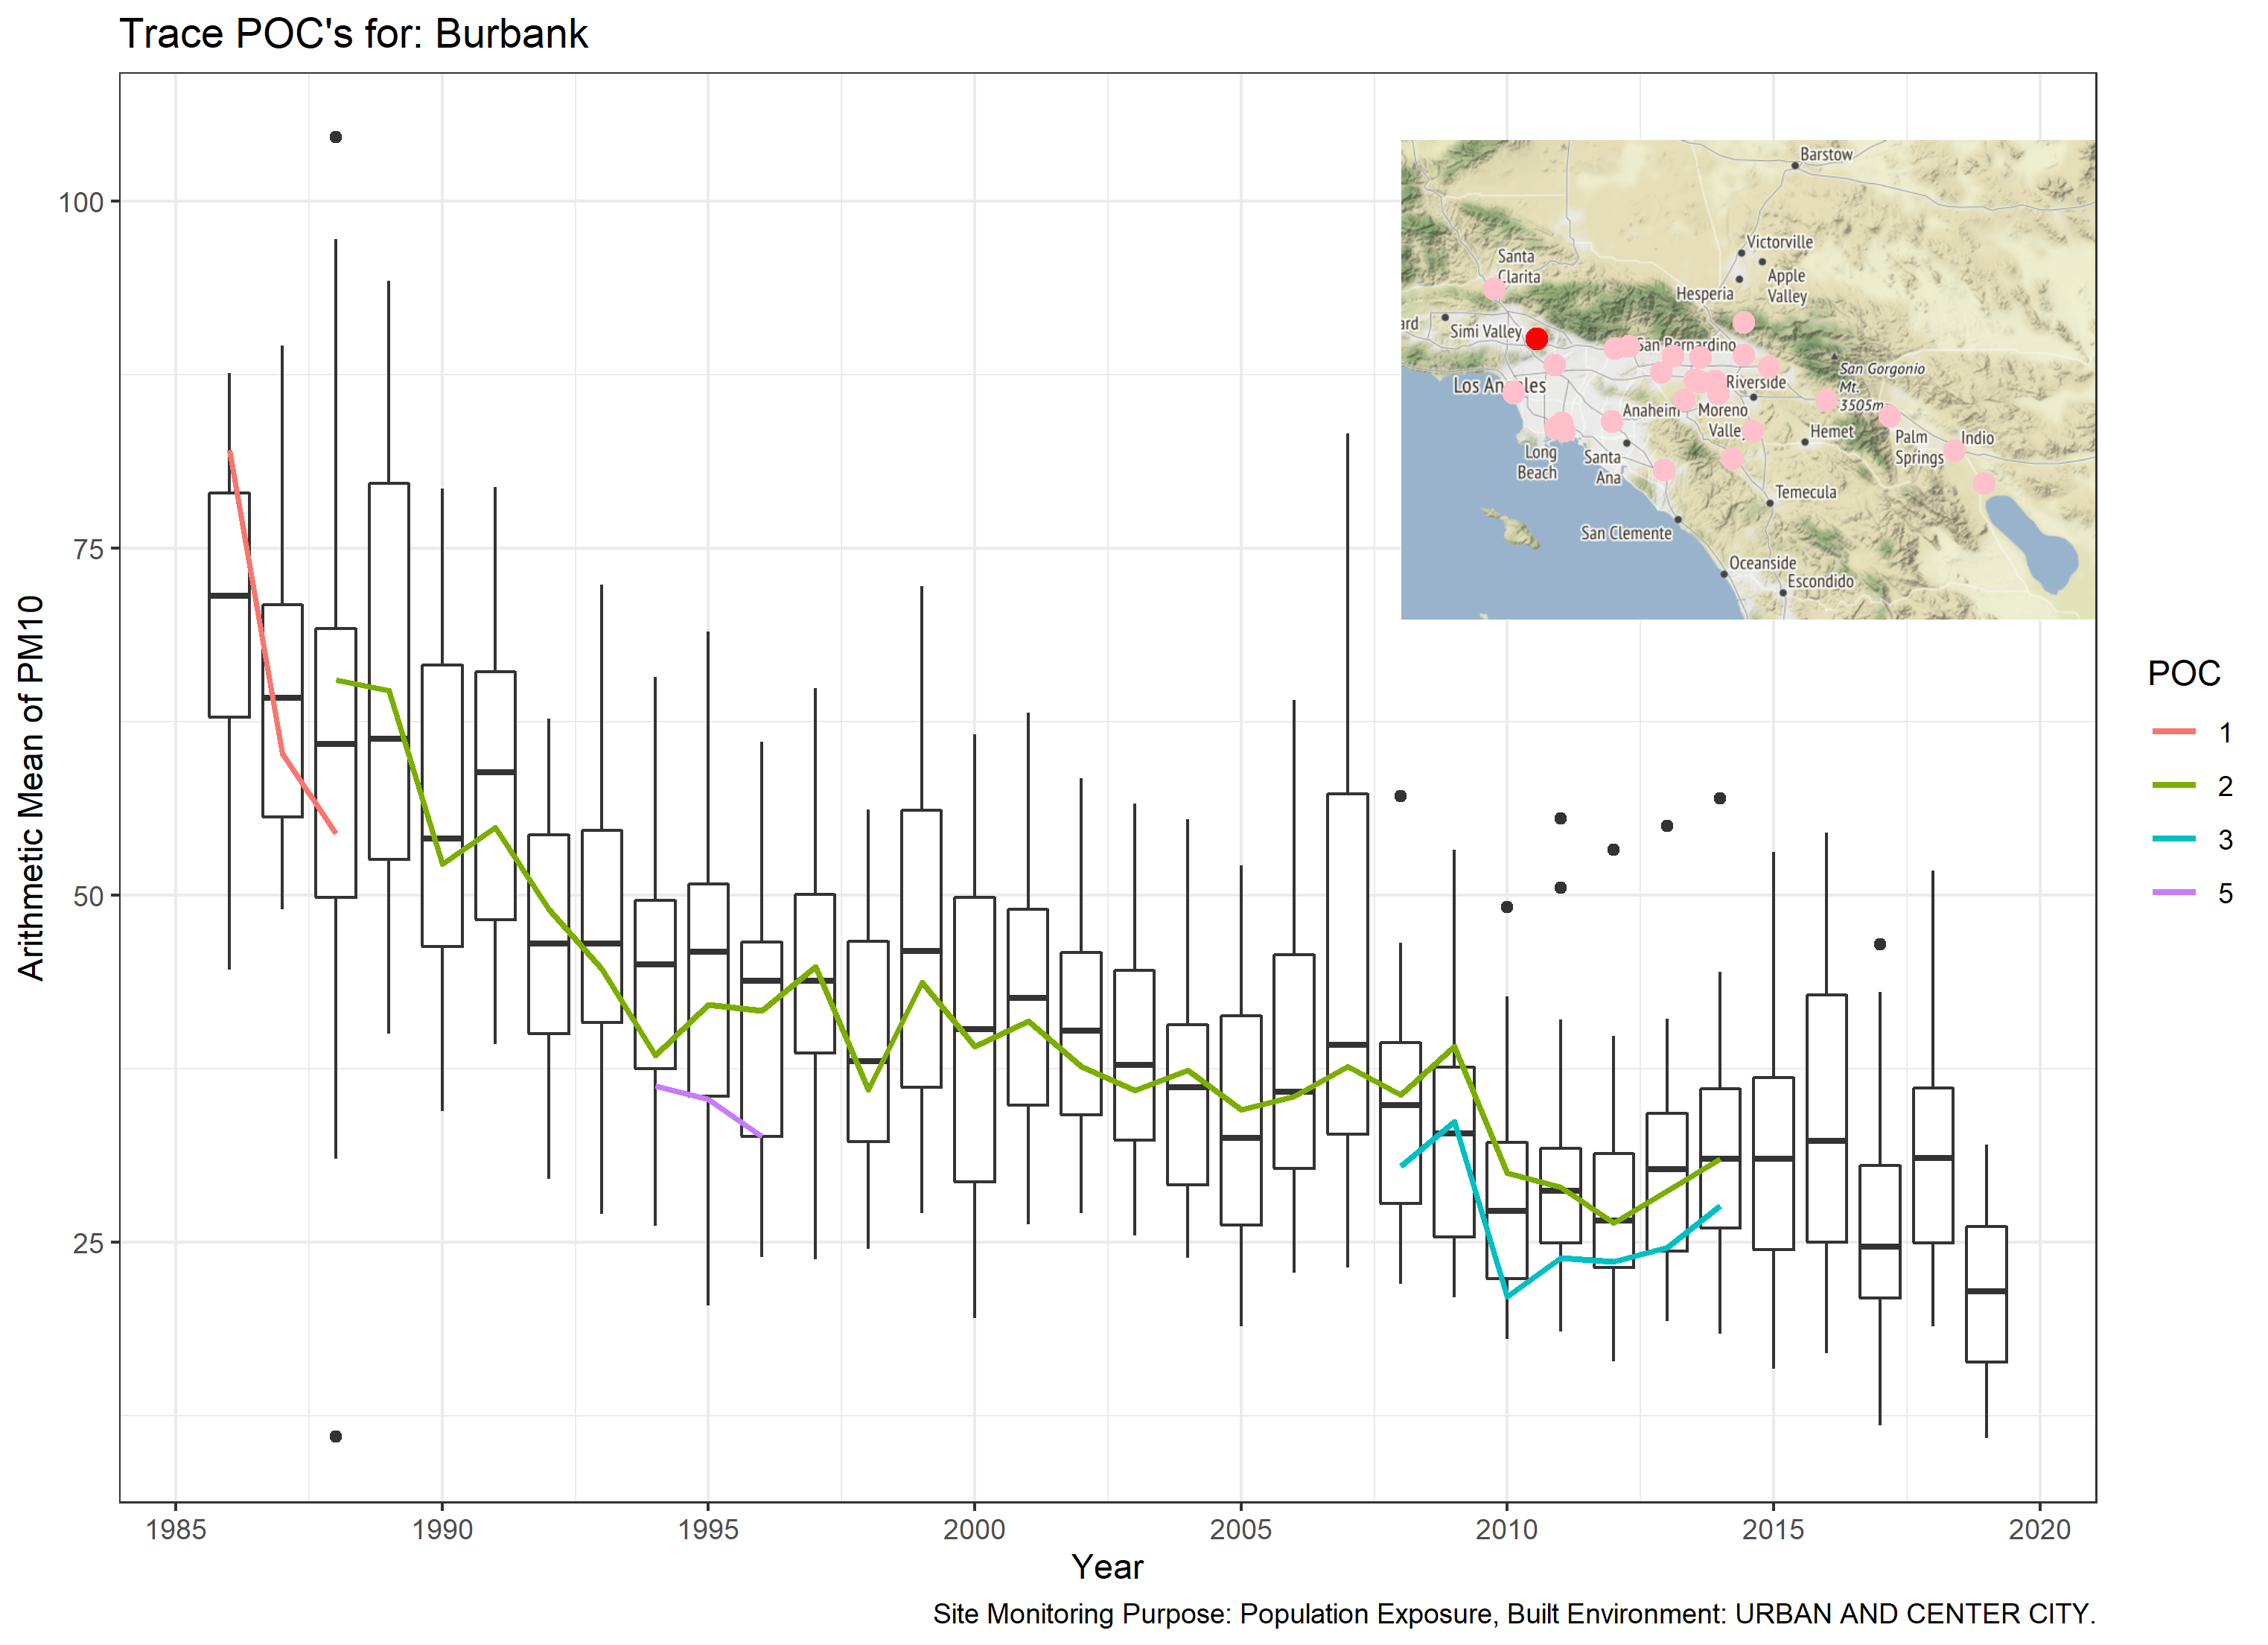}
    \caption{Caption}
    \label{fig:my_label}
\end{figure}

\begin{figure}
    \centering
    \includegraphics[width = \textwidth]{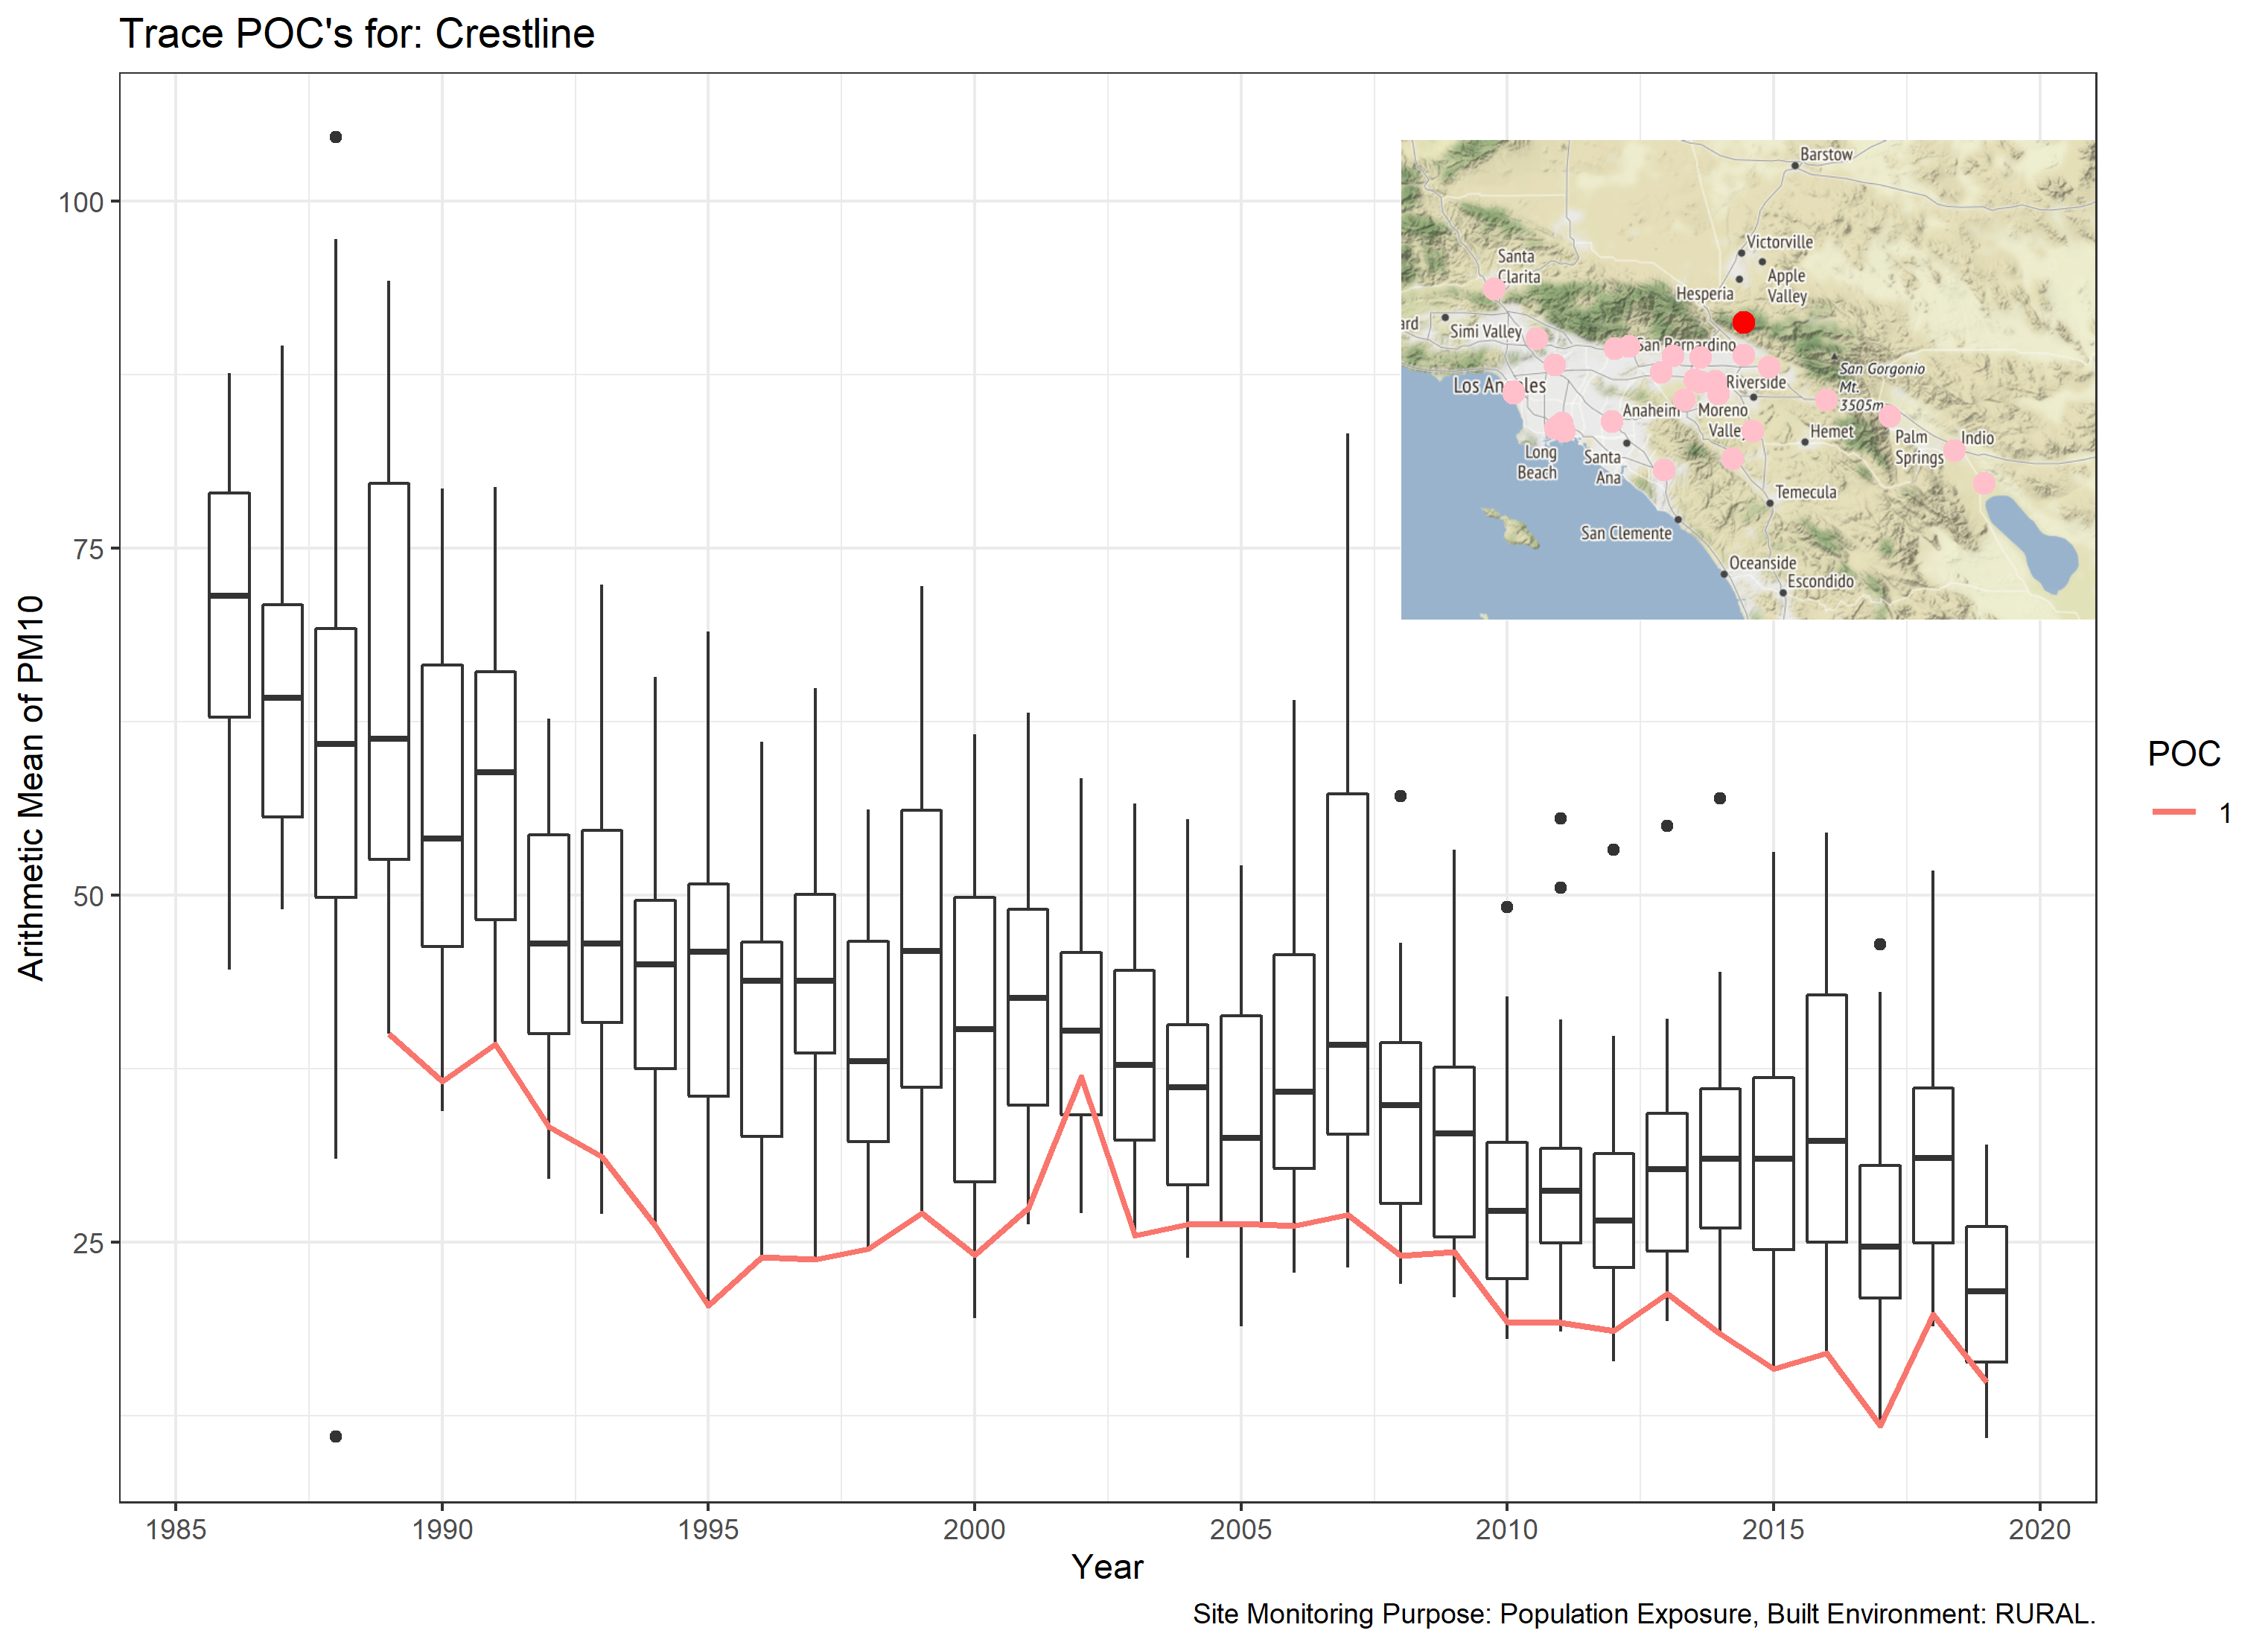}
    \caption{Caption}
    \label{fig:my_label}
\end{figure}

\begin{figure}
    \centering
    \includegraphics[width = \textwidth]{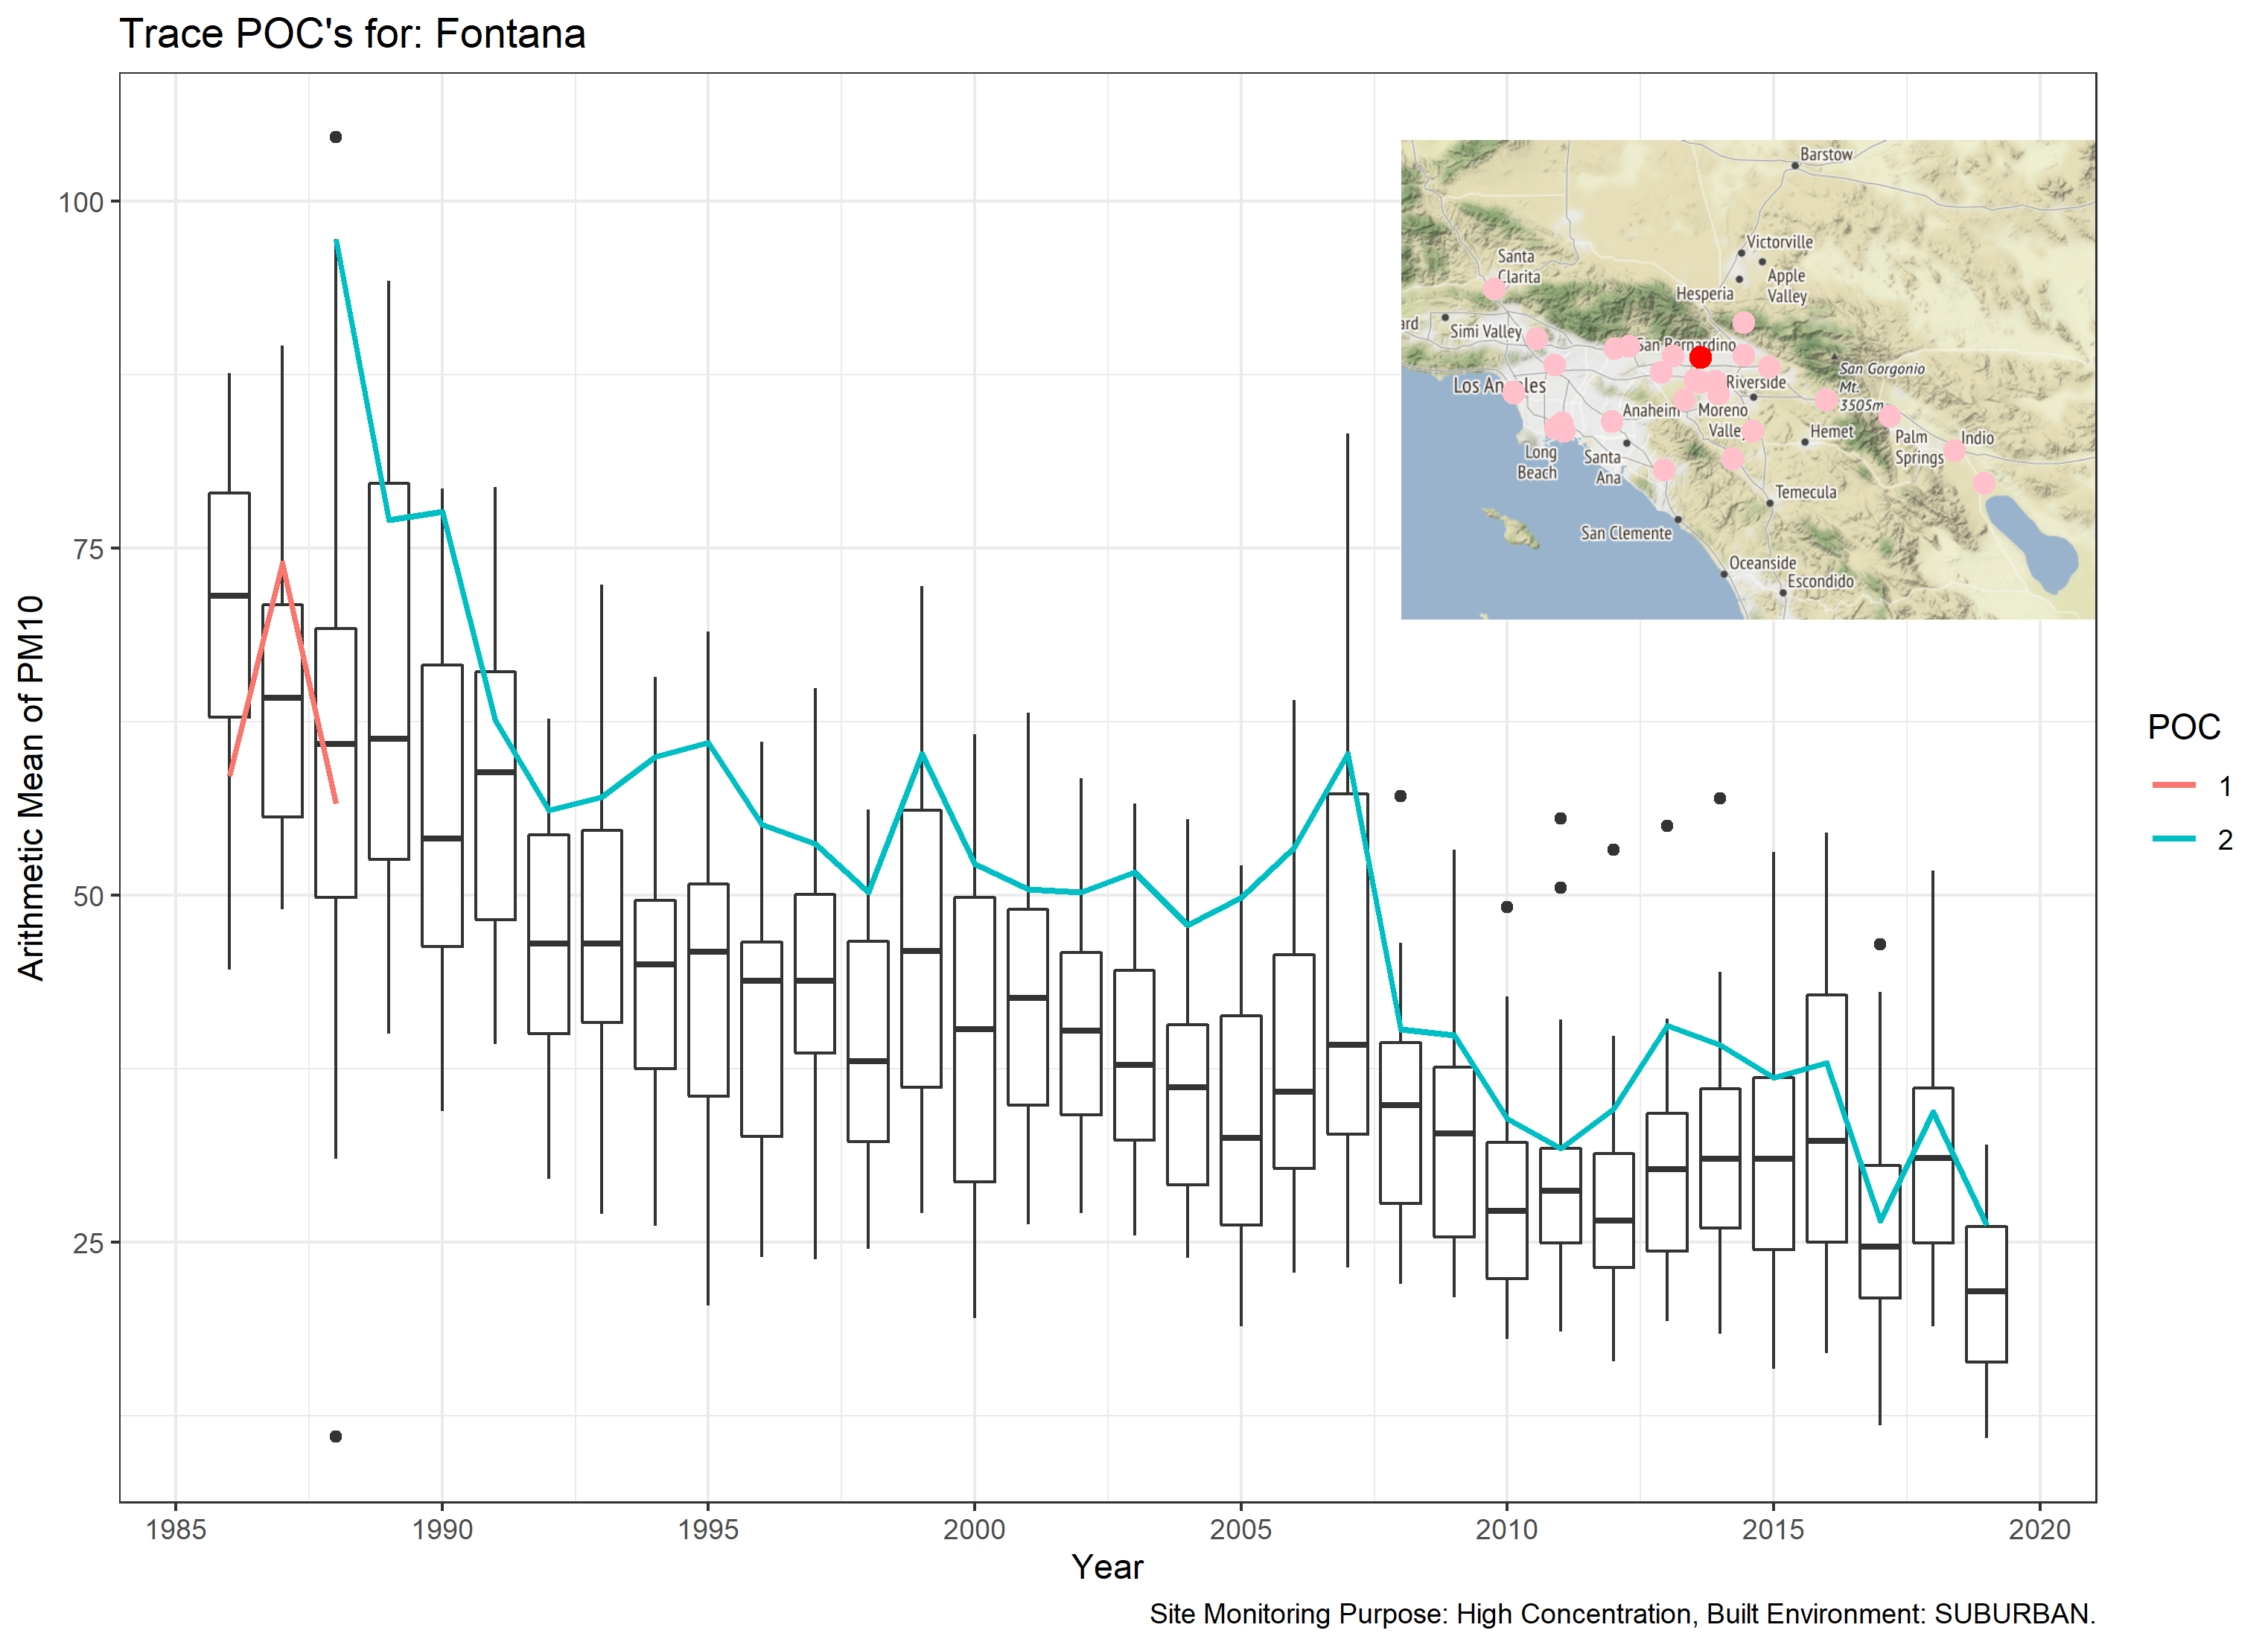}
    \caption{Caption}
    \label{fig:my_label}
\end{figure}

\begin{figure}
    \centering
    \includegraphics[width = \textwidth]{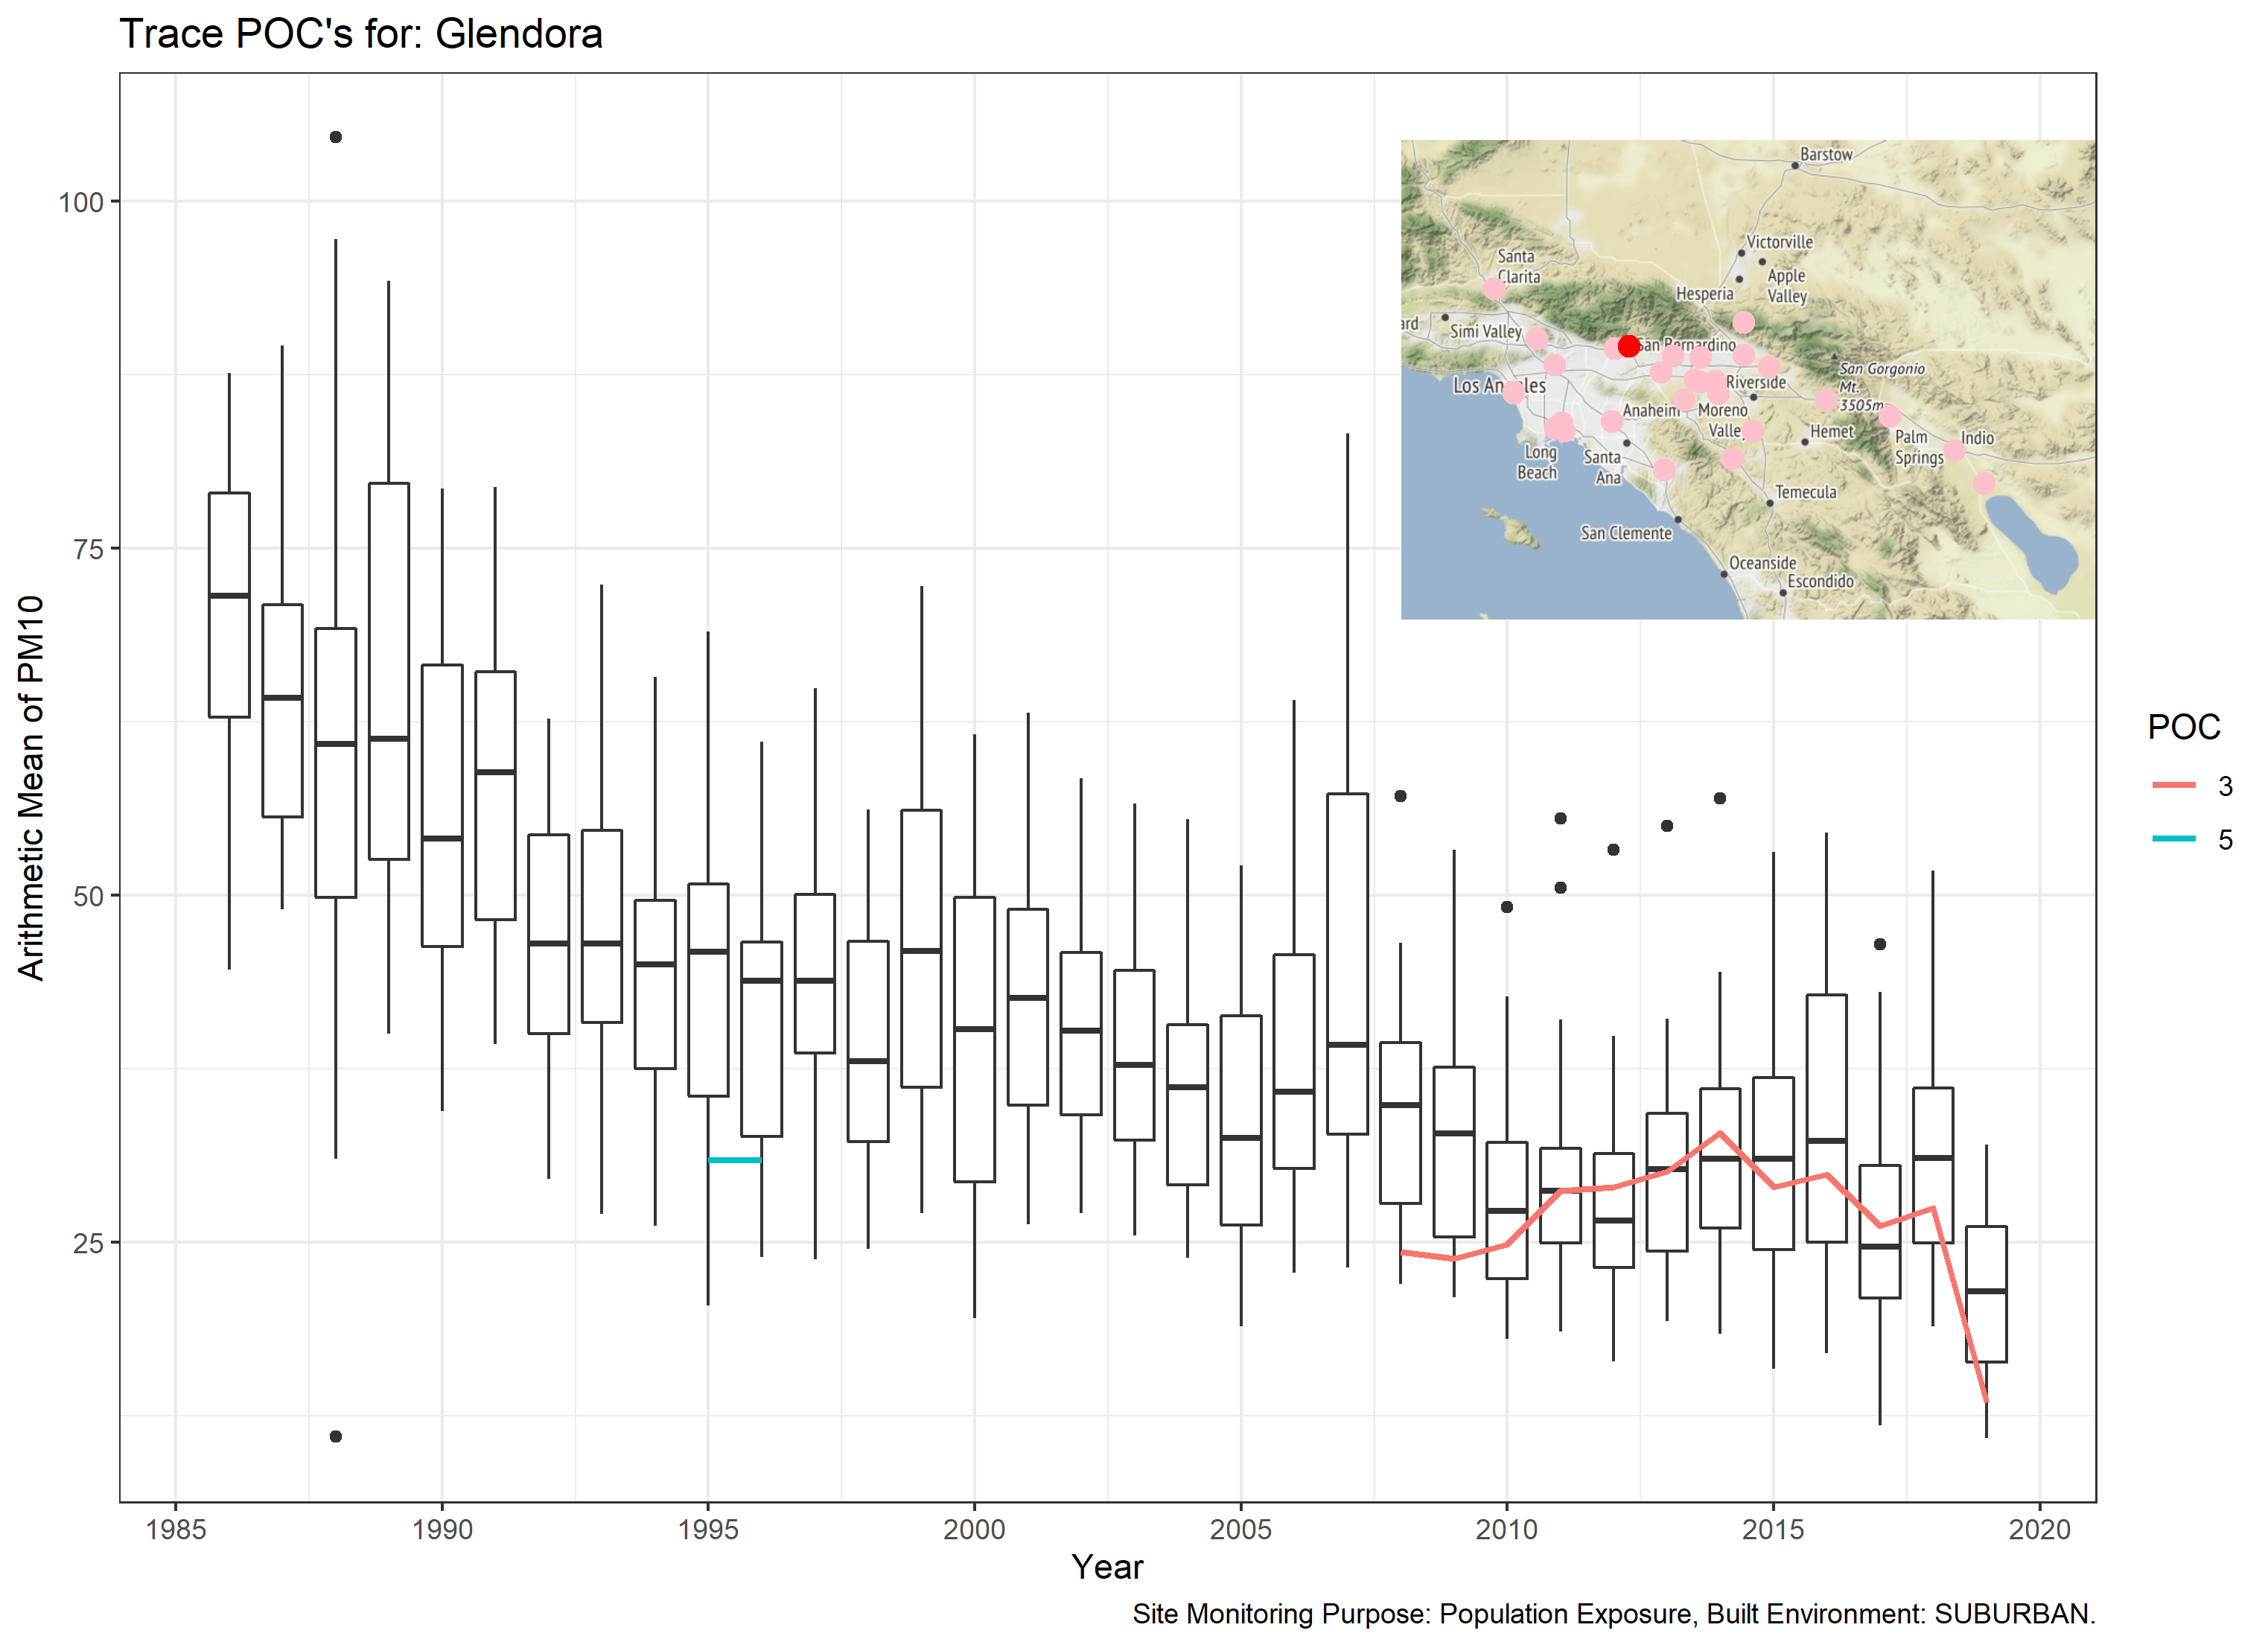}
    \caption{Caption}
    \label{fig:my_label}
\end{figure}

\begin{figure}
    \centering
    \includegraphics[width = \textwidth]{Figures/IndividualSiteTraces/TracePOC_Glendora.png}
    \caption{Caption}
    \label{fig:my_label}
\end{figure}

\begin{figure}
    \centering
    \includegraphics[width = \textwidth]{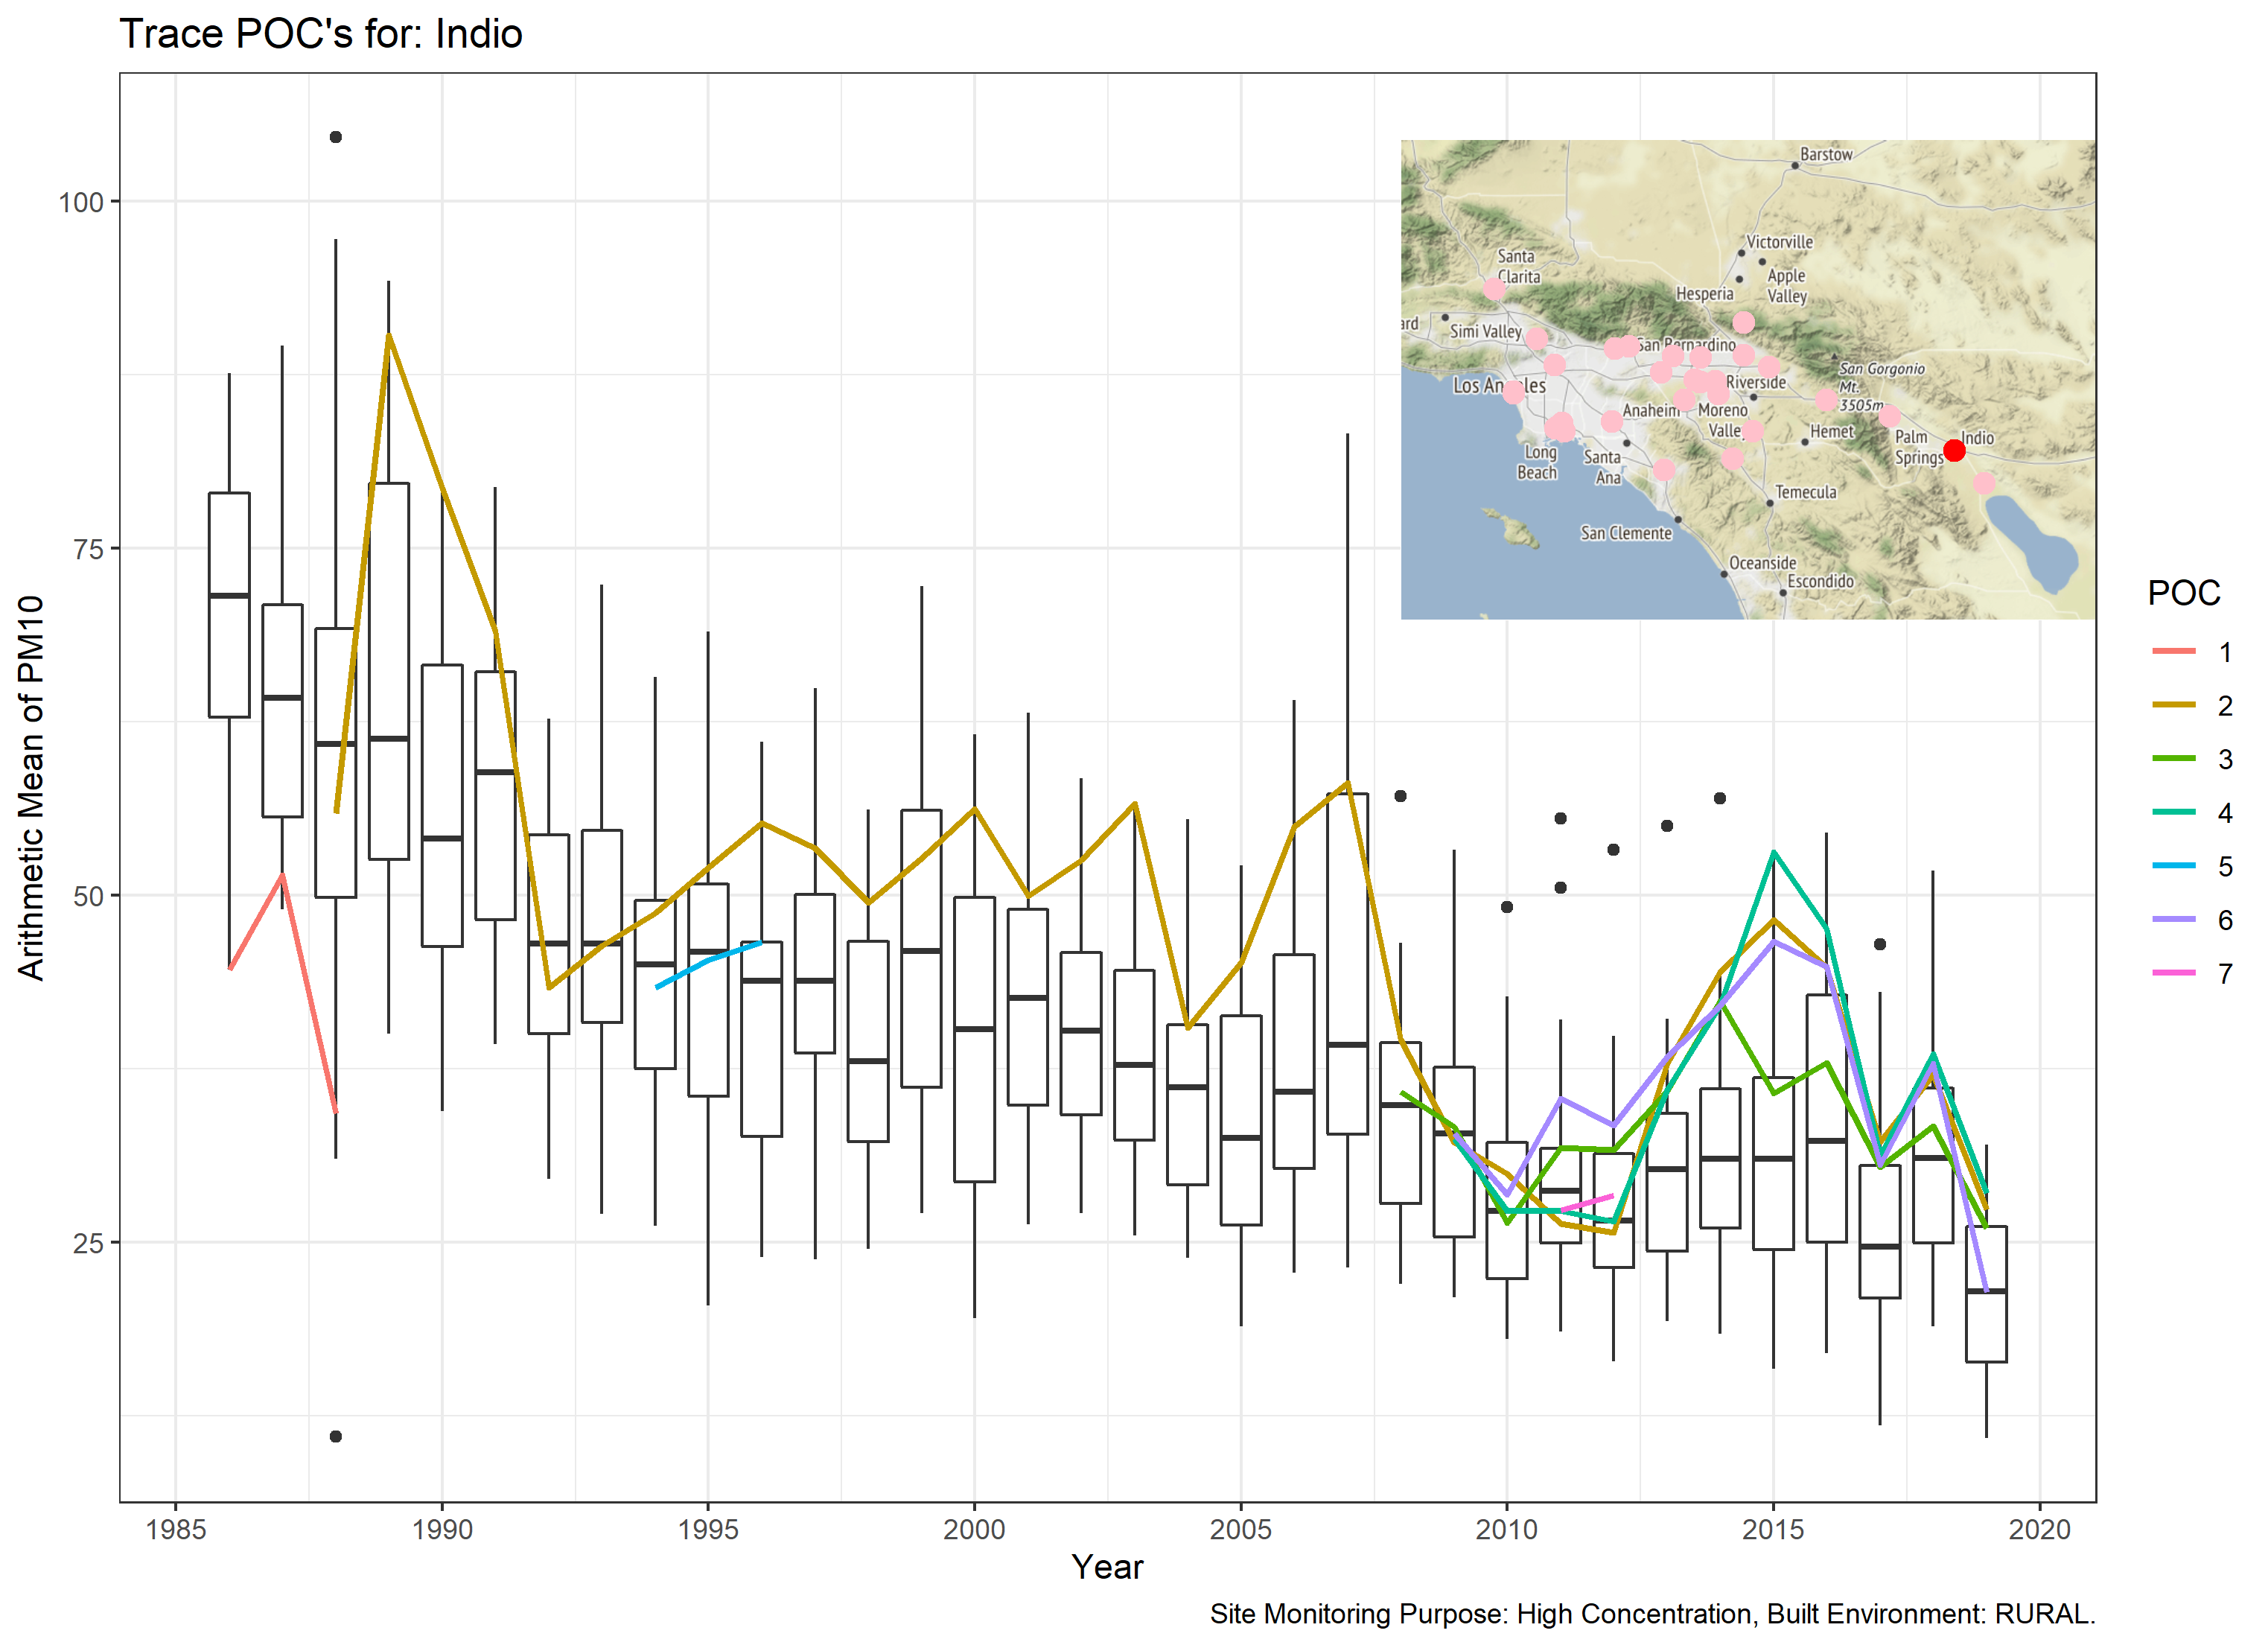}
    \caption{Caption}
    \label{fig:my_label}
\end{figure}

\begin{figure}
    \centering
    \includegraphics[width = \textwidth]{Figures/IndividualSiteTraces/TracePOC_Lake Elsinore.png}
    \caption{Caption}
    \label{fig:my_label}
\end{figure}

\begin{figure}
    \centering
    \includegraphics[width = \textwidth]{Figures/IndividualSiteTraces/TracePOC_LAX Hastings.png}
    \caption{Caption}
    \label{fig:my_label}
\end{figure}

\begin{figure}
    \centering
    \includegraphics[width = \textwidth]{Figures/IndividualSiteTraces/TracePOC_Long Beach (Hudson).png}
    \caption{Caption}
    \label{fig:my_label}
\end{figure}

\begin{figure}
    \centering
    \includegraphics[width = \textwidth]{Figures/IndividualSiteTraces/TracePOC_Long Beach (North).png}
    \caption{Caption}
    \label{fig:my_label}
\end{figure}

\begin{figure}
    \centering
    \includegraphics[width = \textwidth]{Figures/IndividualSiteTraces/TracePOC_Long Beach (South).png}
    \caption{Caption}
    \label{fig:my_label}
\end{figure}

\begin{figure}
    \centering
    \includegraphics[width = \textwidth]{Figures/IndividualSiteTraces/TracePOC_Los Angeles-North Main Street.png}
    \caption{Caption}
    \label{fig:my_label}
\end{figure}

\begin{figure}
    \centering
    \includegraphics[width = \textwidth]{Figures/IndividualSiteTraces/TracePOC_Mecca (Saul Martinez).png}
    \caption{Caption}
    \label{fig:my_label}
\end{figure}

\begin{figure}
    \centering
    \includegraphics[width = \textwidth]{Figures/IndividualSiteTraces/TracePOC_Mira Loma (Bellegrave).png}
    \caption{Caption}
    \label{fig:my_label}
\end{figure}

\begin{figure}
    \centering
    \includegraphics[width = \textwidth]{Figures/IndividualSiteTraces/TracePOC_Mira Loma (Van Buren).png}
    \caption{Caption}
    \label{fig:my_label}
\end{figure}

\begin{figure}
    \centering
    \includegraphics[width = \textwidth]{Figures/IndividualSiteTraces/TracePOC_Mission Viejo.png}
    \caption{Caption}
    \label{fig:my_label}
\end{figure}

\begin{figure}
    \centering
    \includegraphics[width = \textwidth]{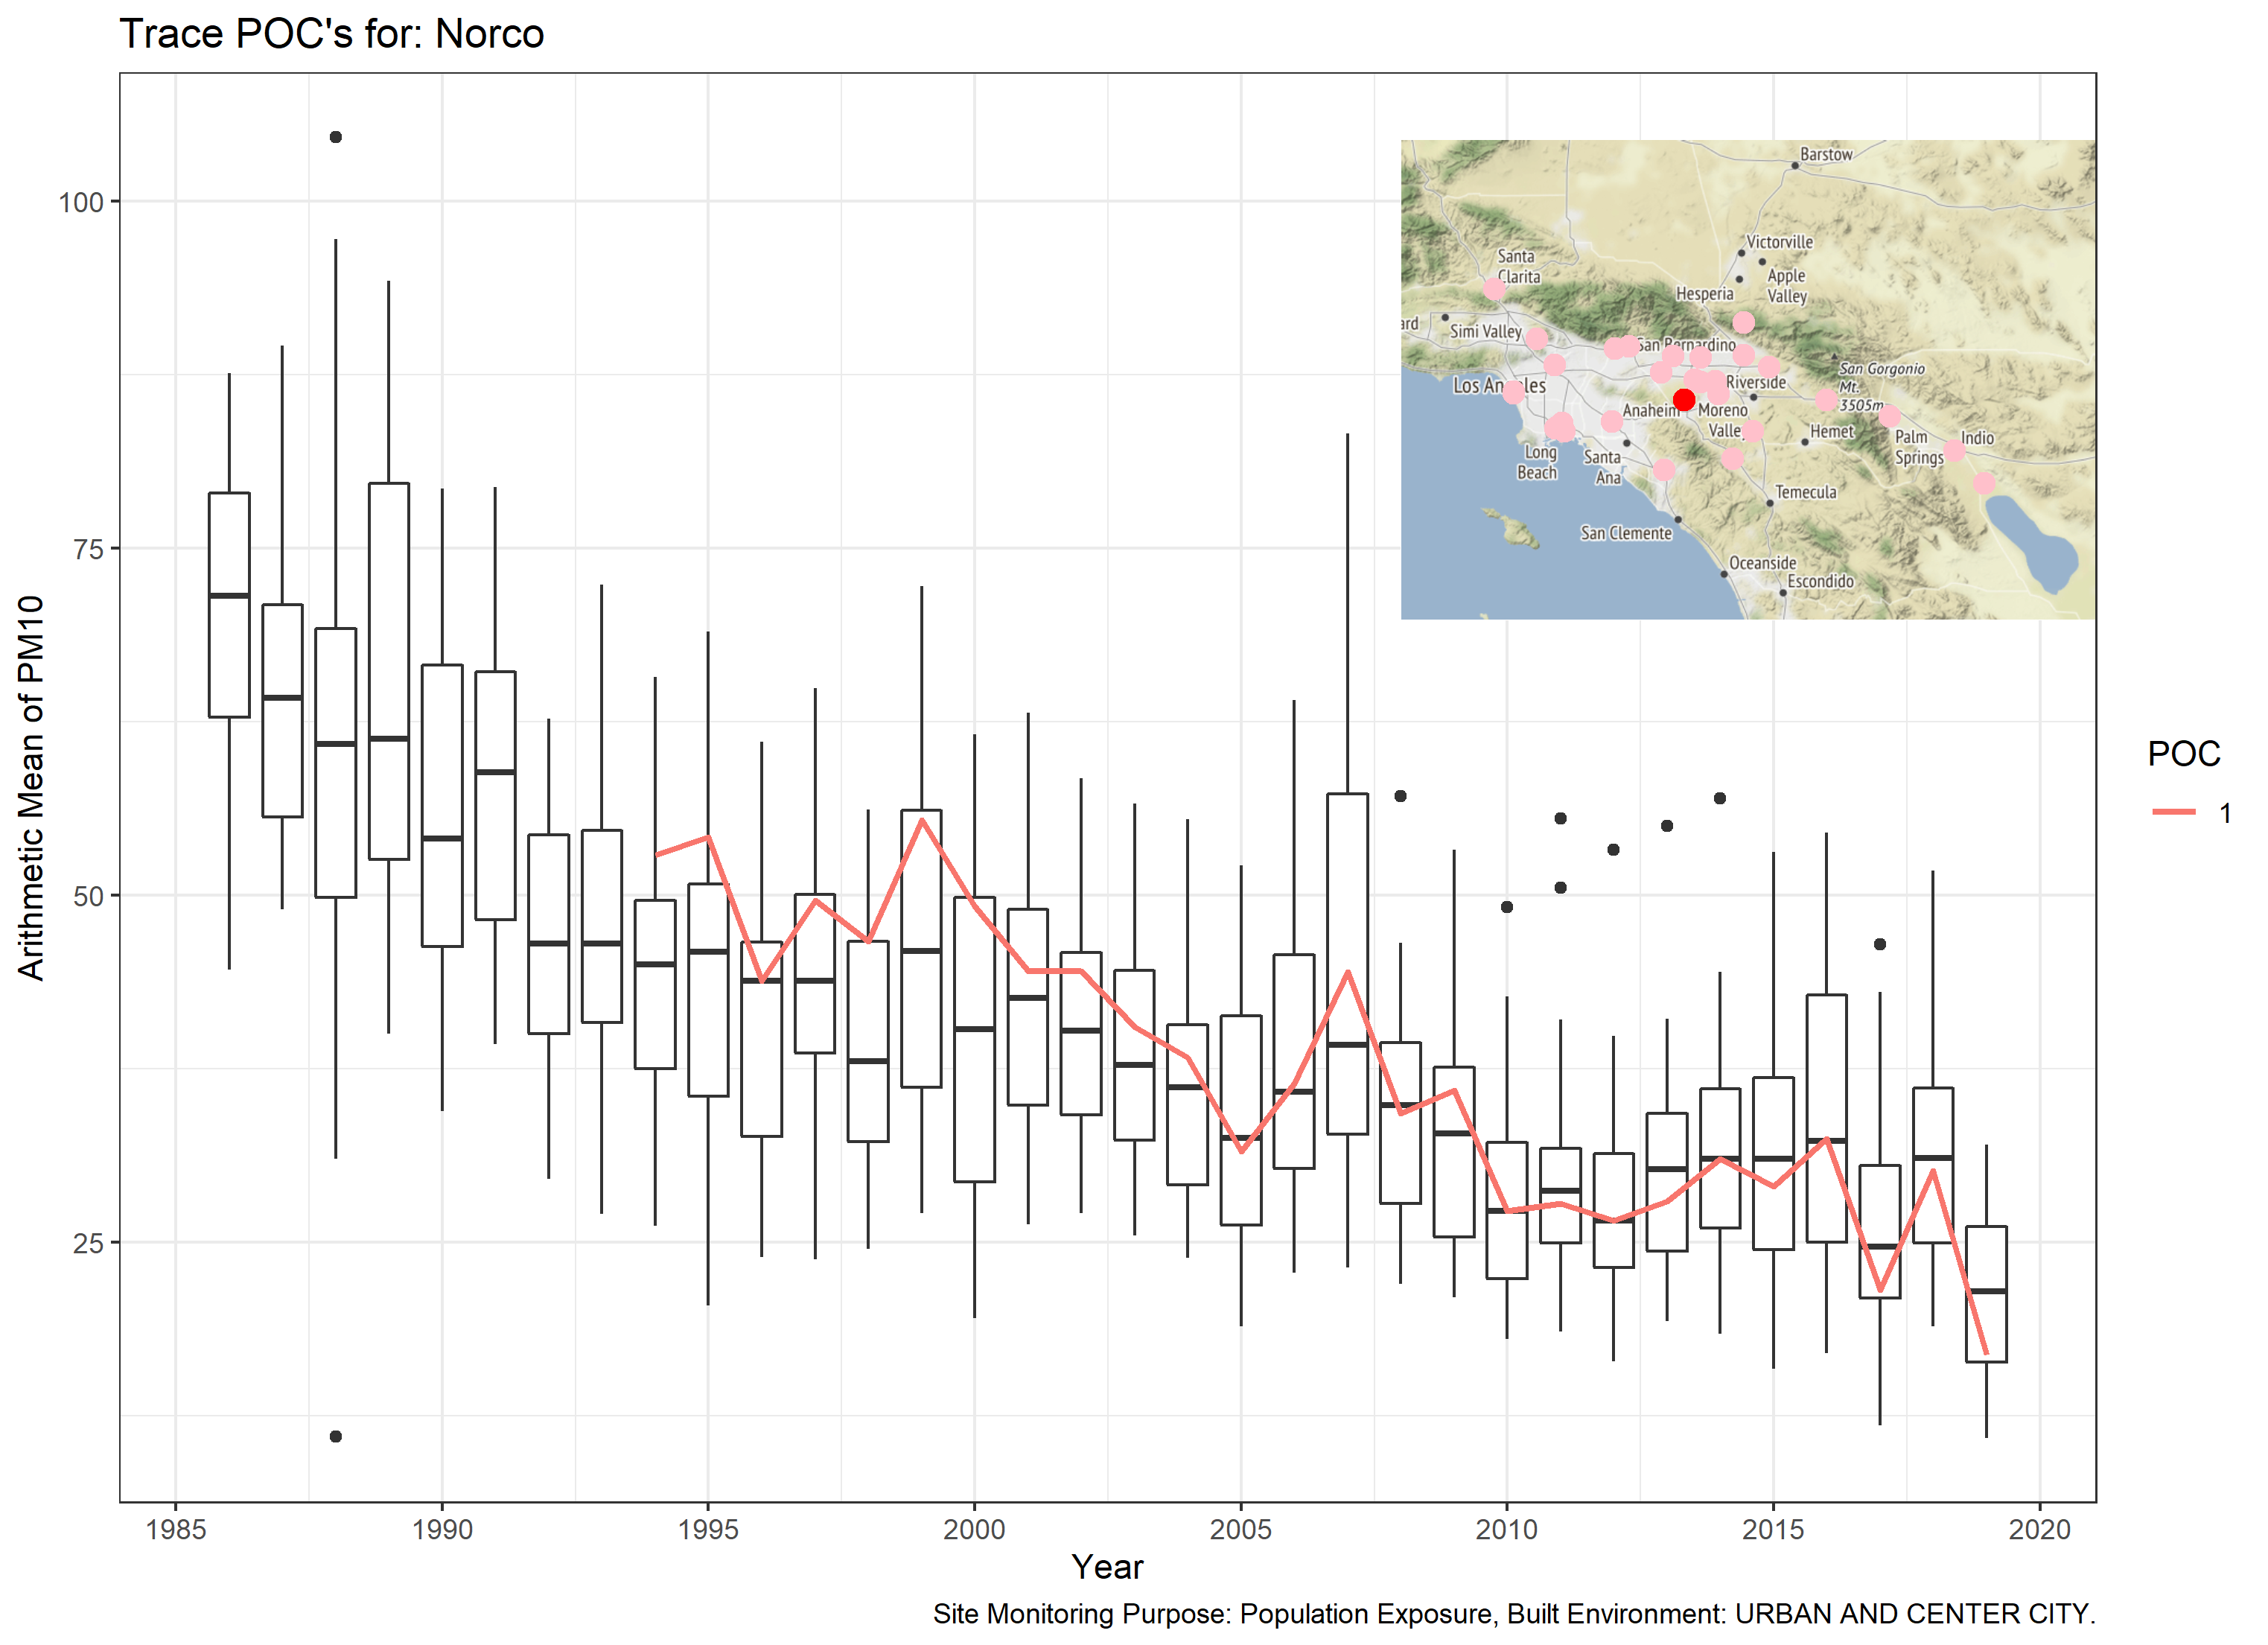}
    \caption{Caption}
    \label{fig:my_label}
\end{figure}

\begin{figure}
    \centering
    \includegraphics[width = \textwidth]{Figures/IndividualSiteTraces/TracePOC_Ontario Fire Station.png}
    \caption{Caption}
    \label{fig:my_label}
\end{figure}

\begin{figure}
    \centering
    \includegraphics[width = \textwidth]{Figures/IndividualSiteTraces/TracePOC_Palm Springs.png}
    \caption{Caption}
    \label{fig:my_label}
\end{figure}

\begin{figure}
    \centering
    \includegraphics[width = \textwidth]{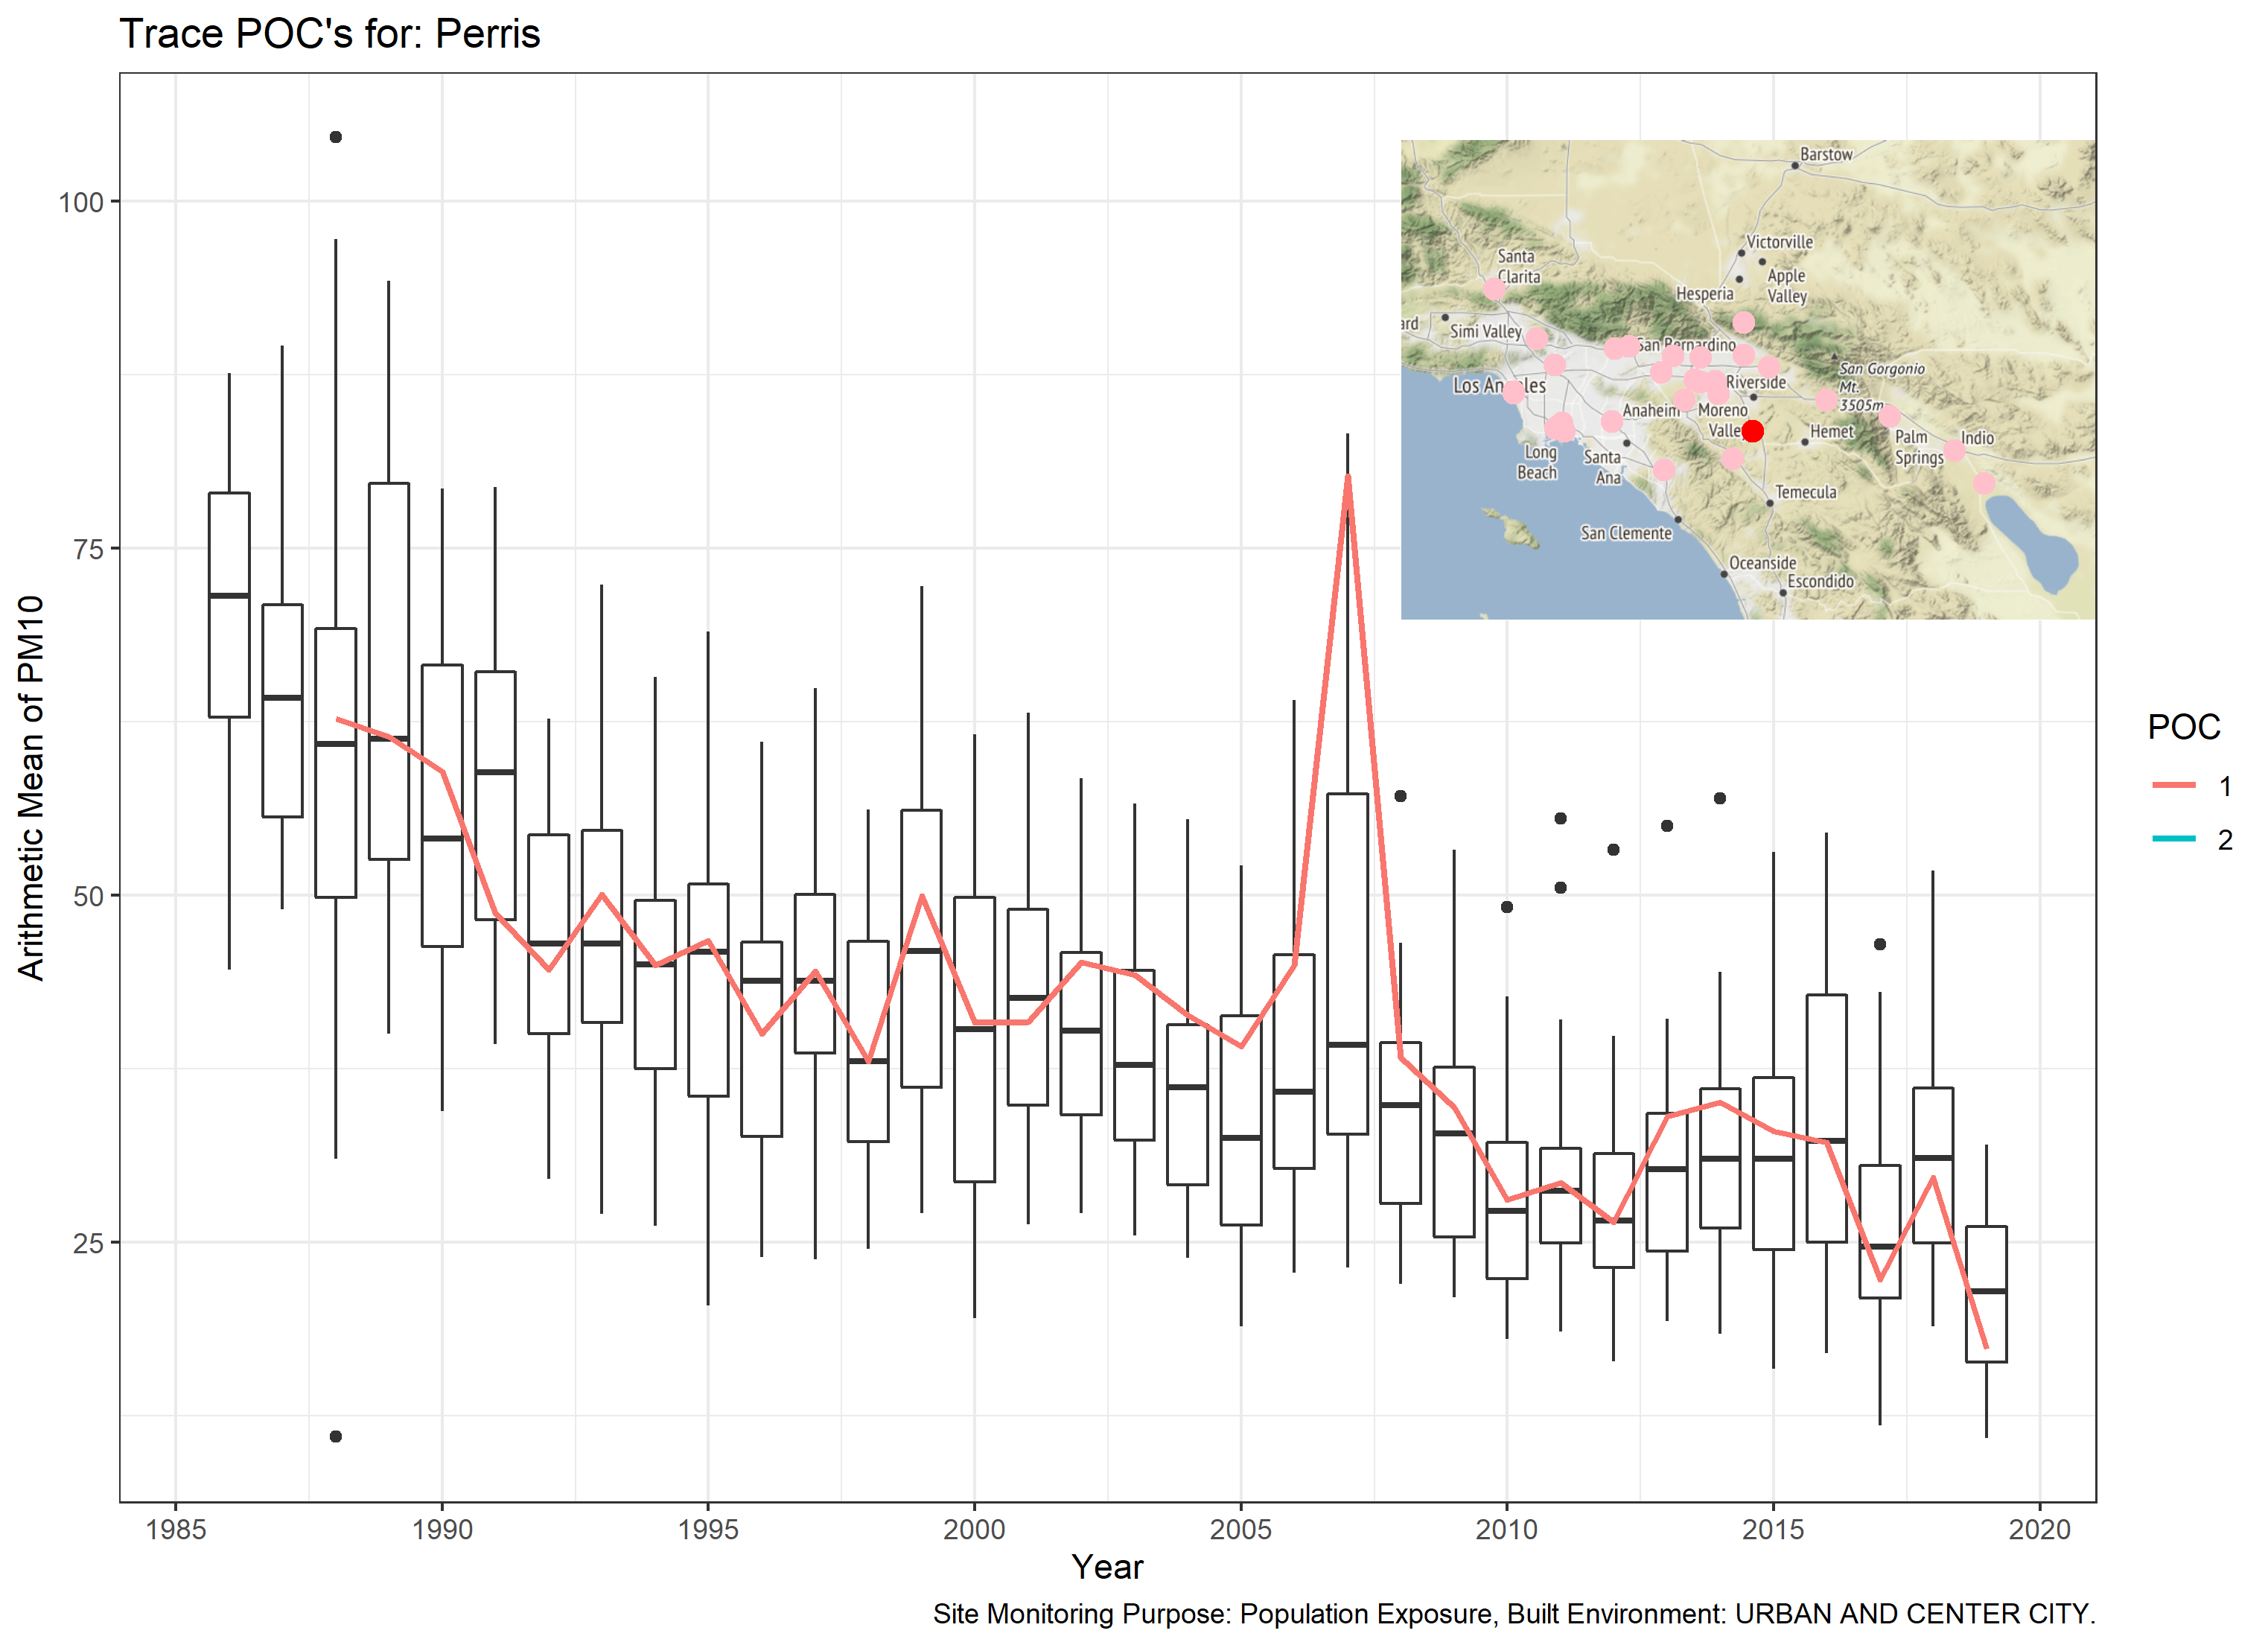}
    \caption{Caption}
    \label{fig:my_label}
\end{figure}

\begin{figure}
    \centering
    \includegraphics[width = \textwidth]{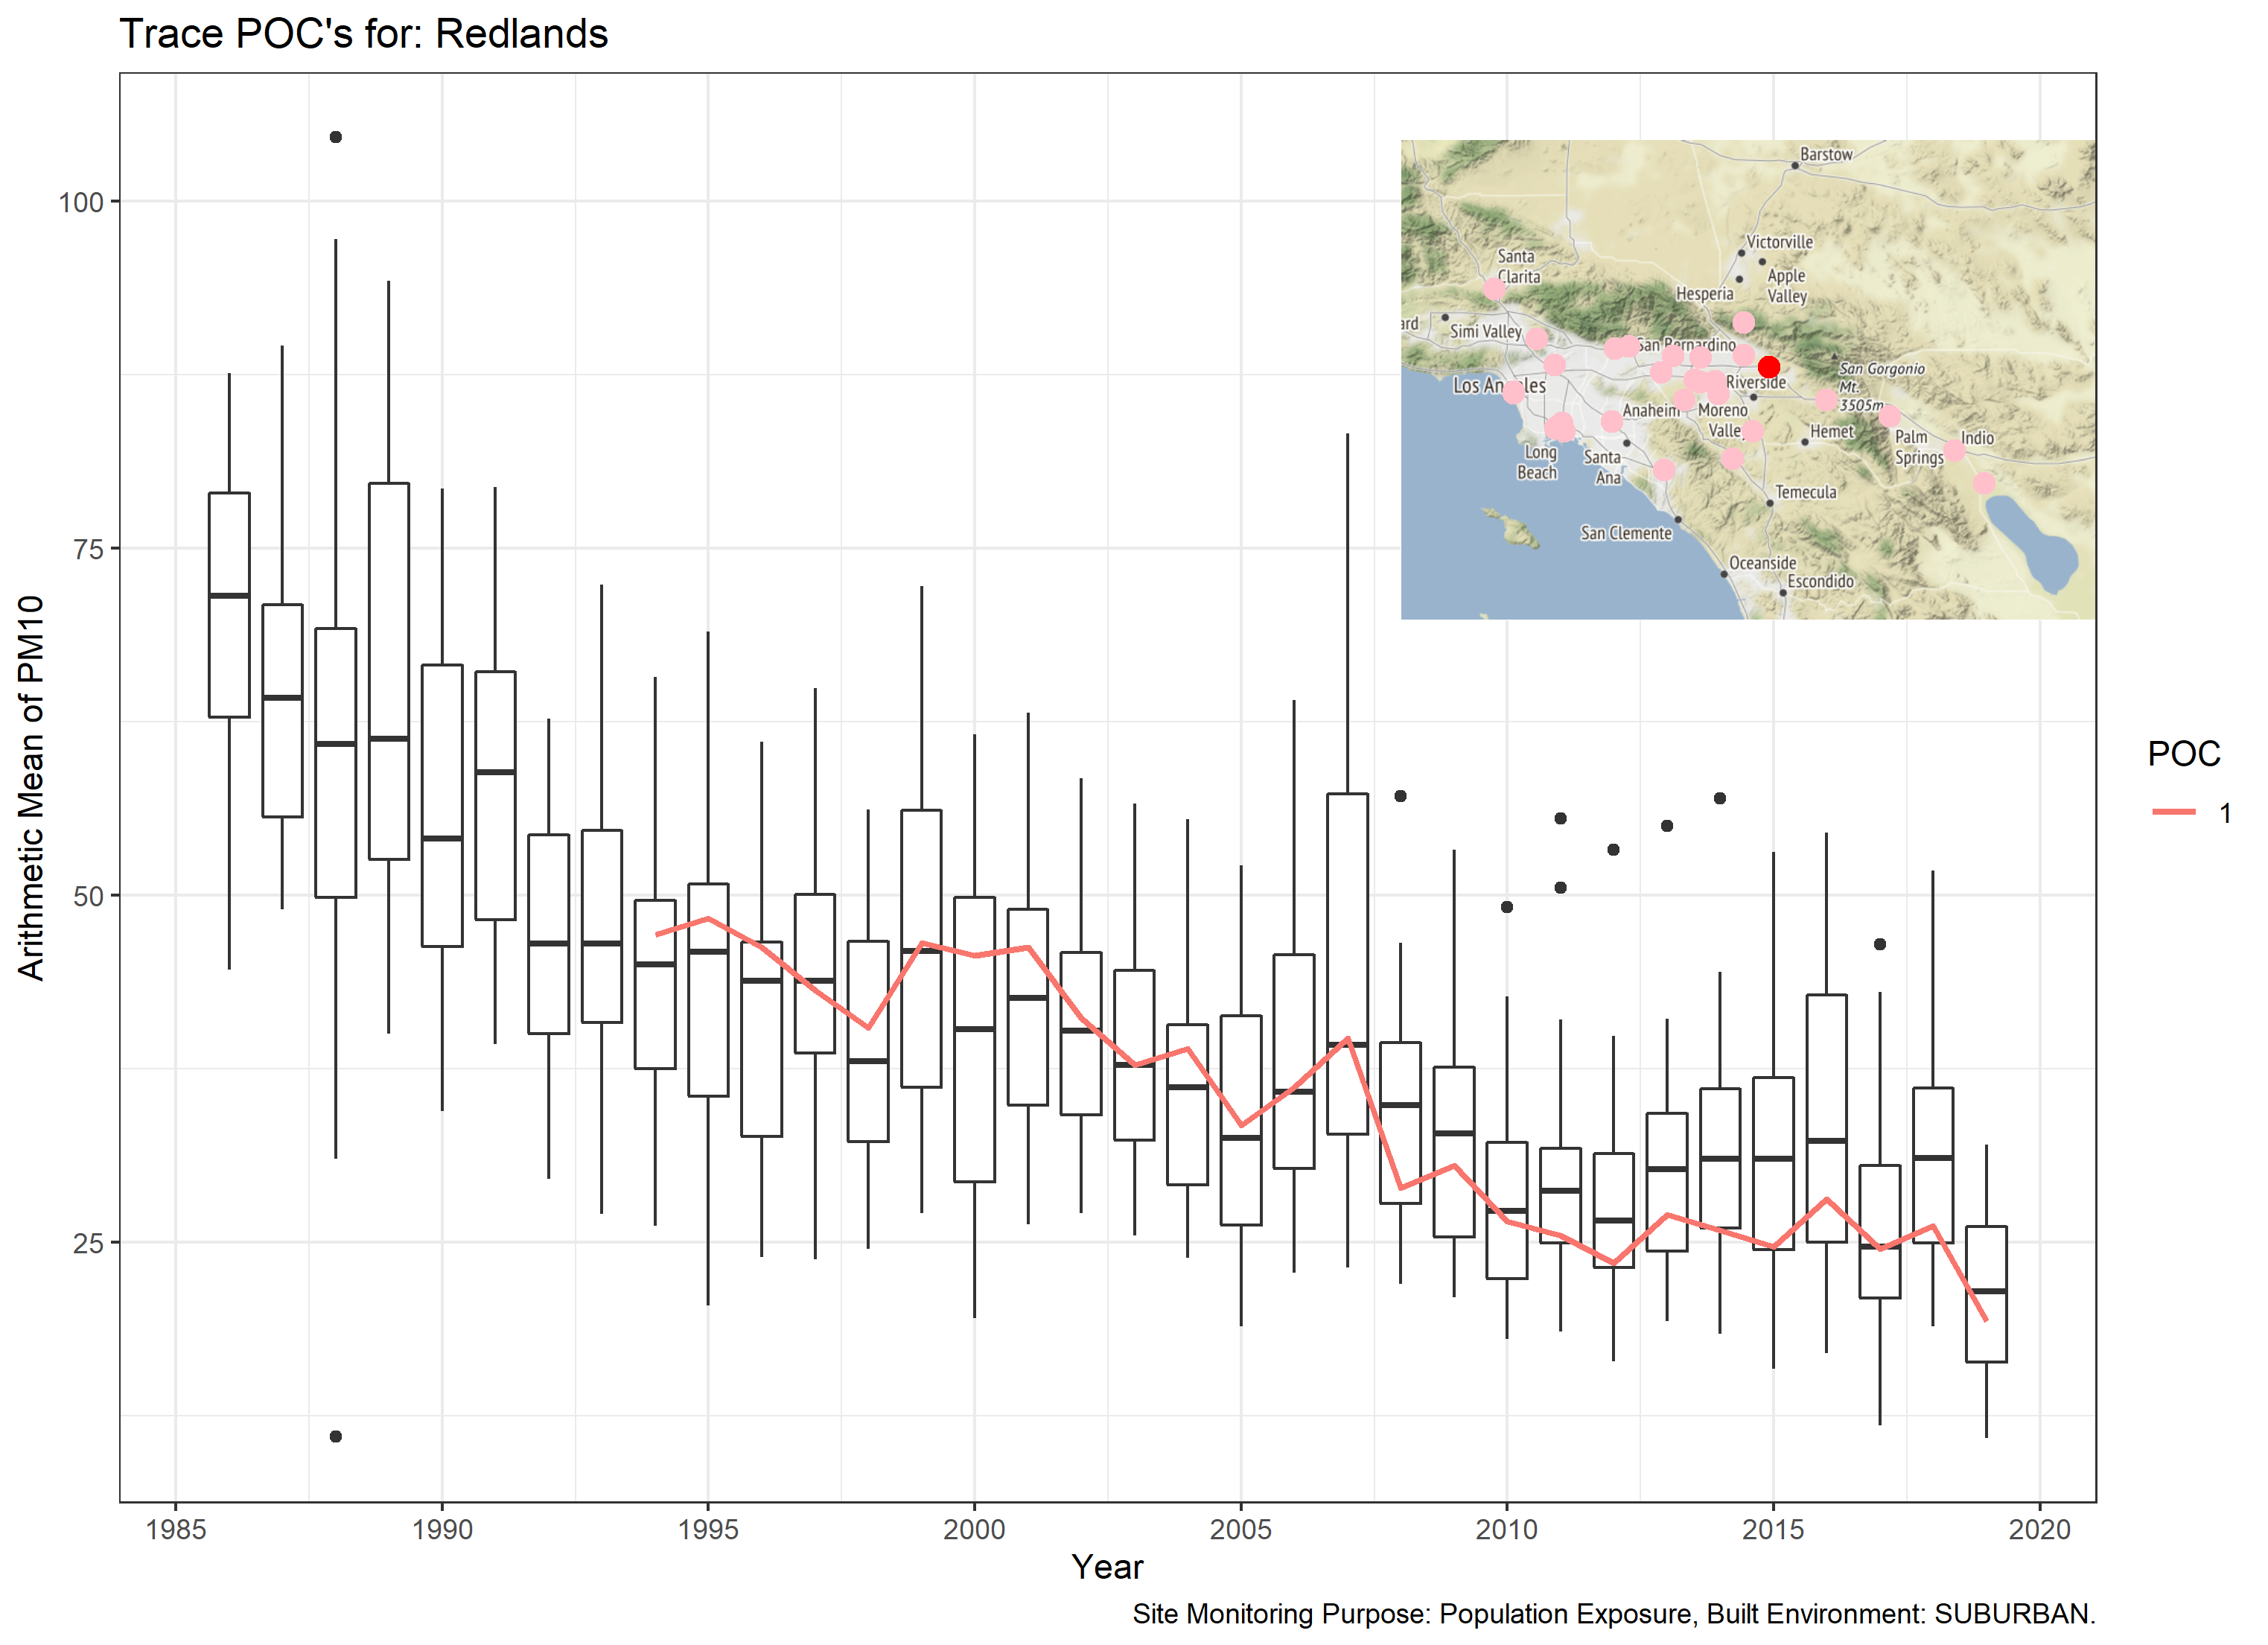}
    \caption{Caption}
    \label{fig:my_label}
\end{figure}

\begin{figure}
    \centering
    \includegraphics[width = \textwidth]{Figures/IndividualSiteTraces/TracePOC_Riverside (Magnolia).png}
    \caption{Caption}
    \label{fig:my_label}
\end{figure}

\begin{figure}
    \centering
    \includegraphics[width = \textwidth]{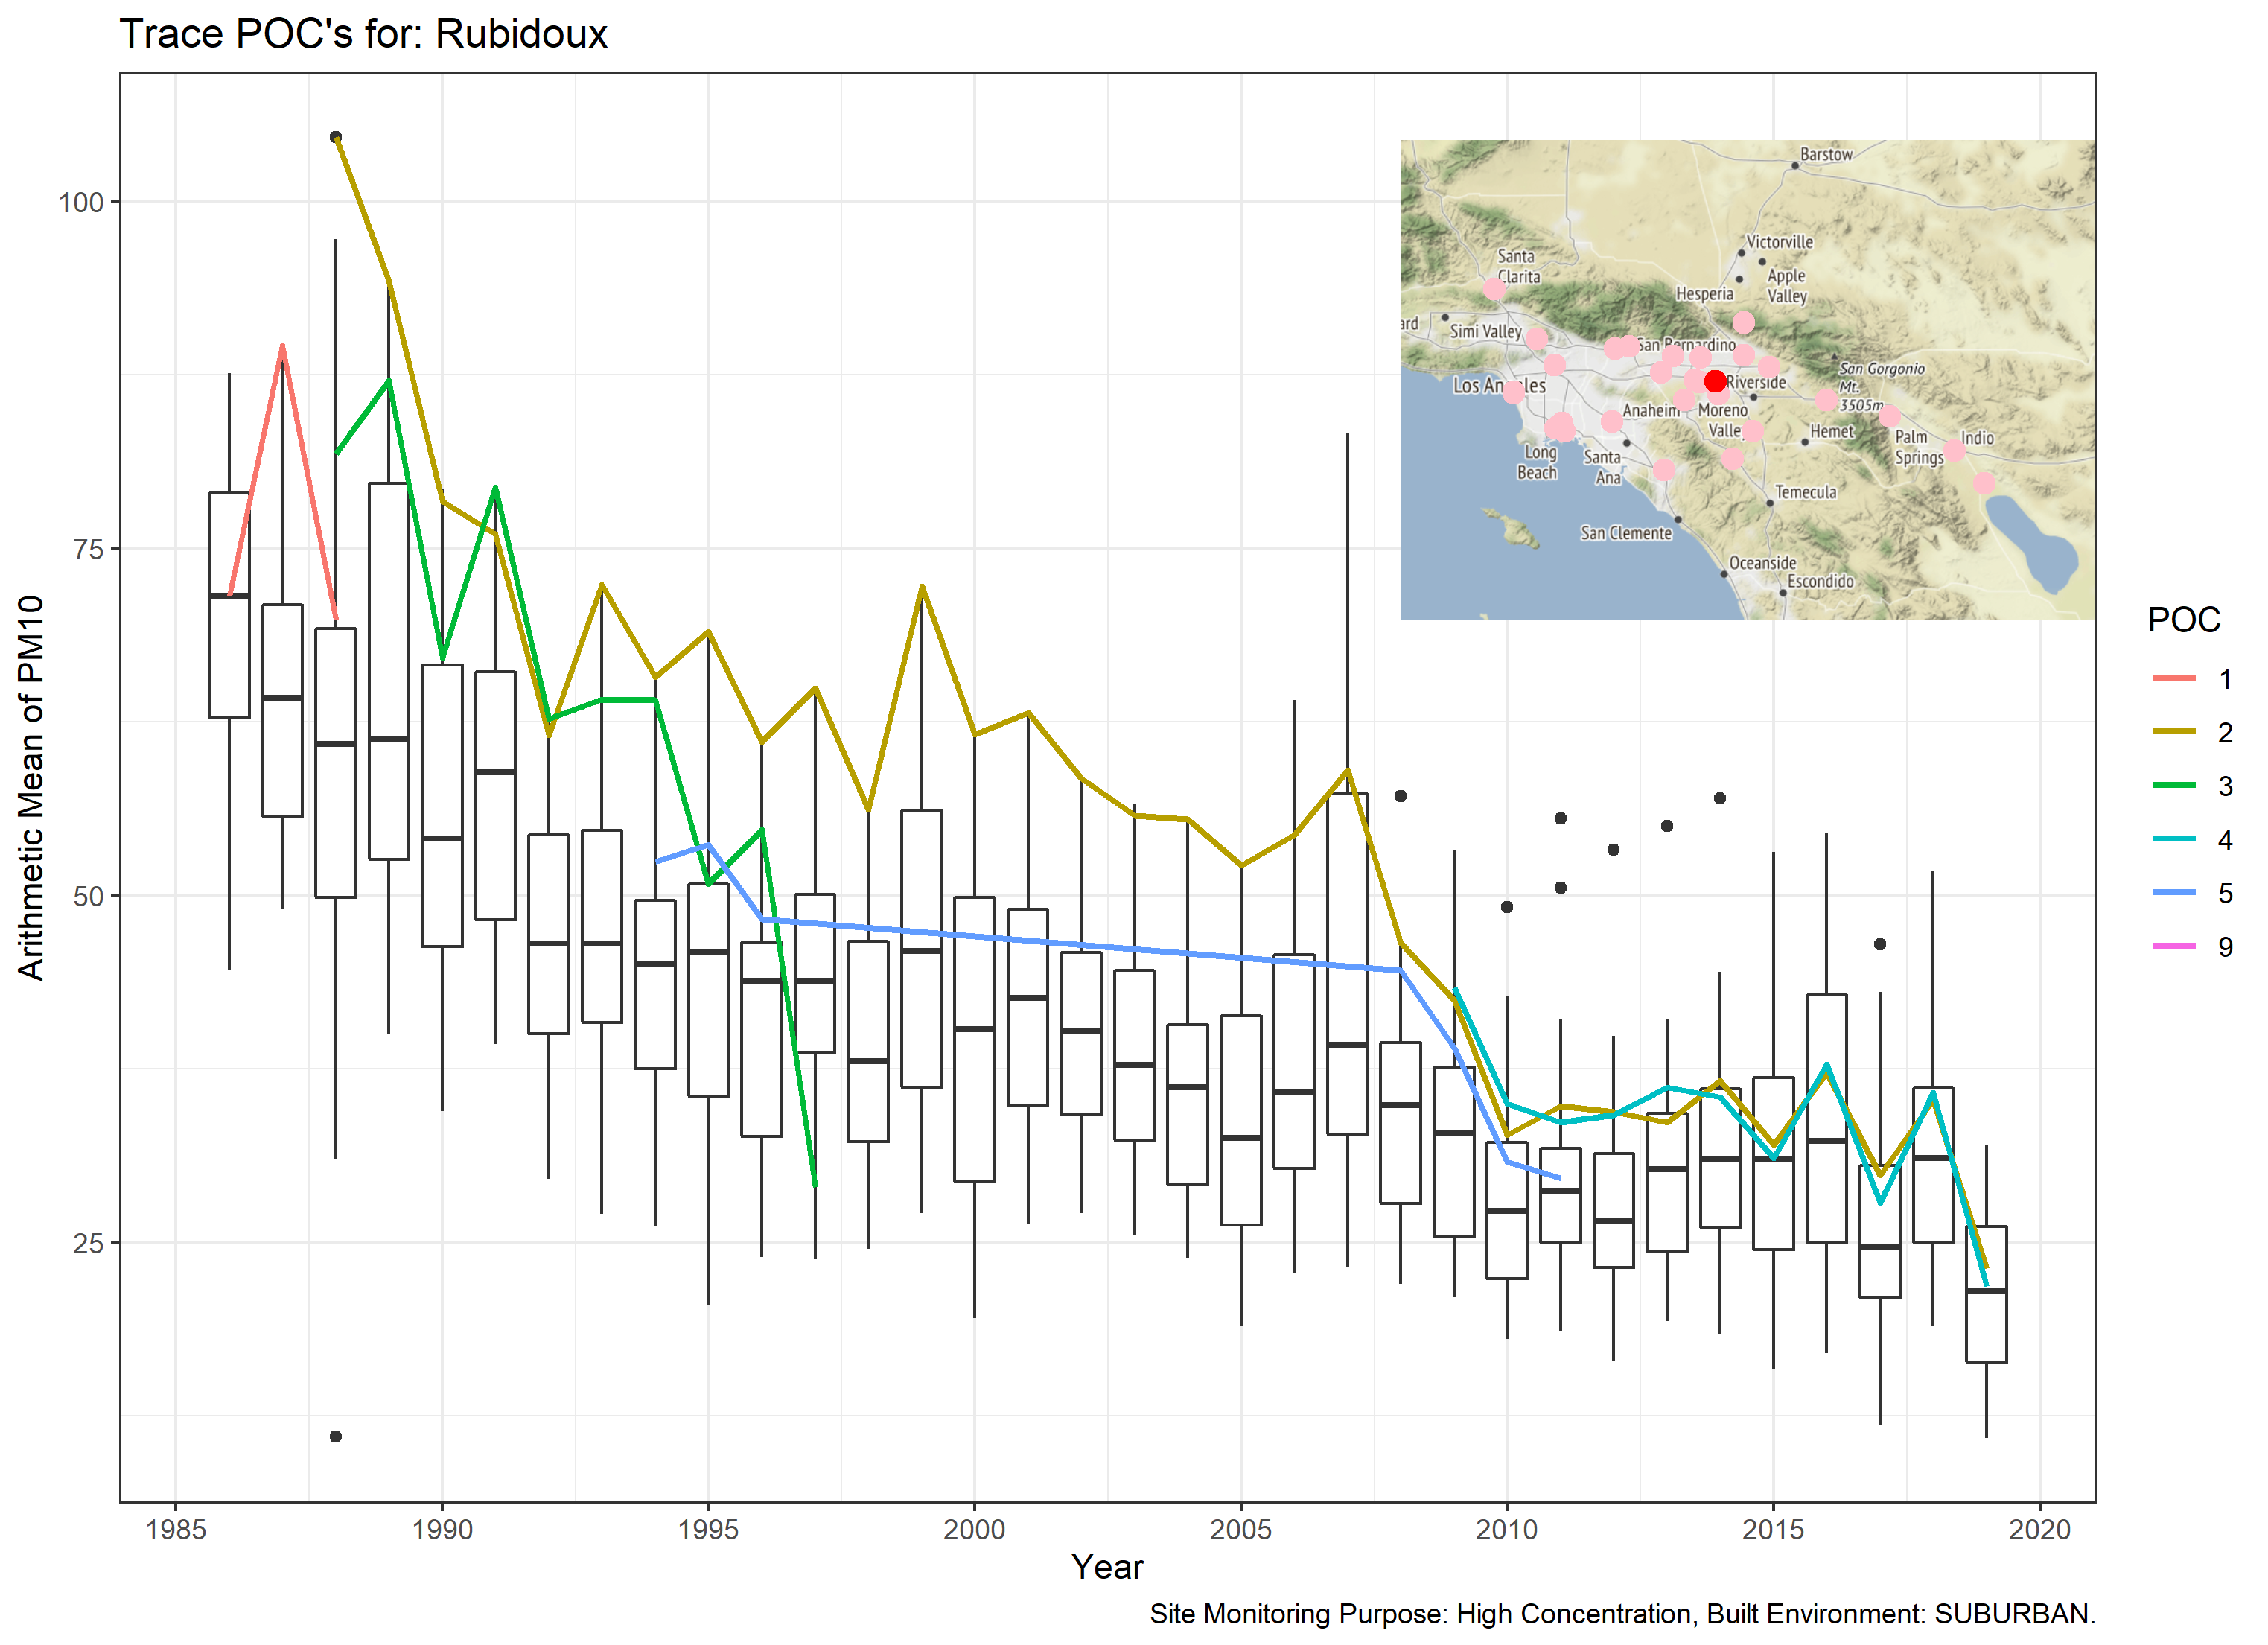}
    \caption{Caption}
    \label{fig:my_label}
\end{figure}

\begin{figure}
    \centering
    \includegraphics[width = \textwidth]{Figures/IndividualSiteTraces/TracePOC_San Bernardino.png}
    \caption{Caption}
    \label{fig:my_label}
\end{figure}

\begin{figure}
    \centering
    \includegraphics[width = \textwidth]{Figures/IndividualSiteTraces/TracePOC_Santa Clarita.png}
    \caption{Caption}
    \label{fig:my_label}
\end{figure}

\begin{figure}
    \centering
    \includegraphics[width = \textwidth]{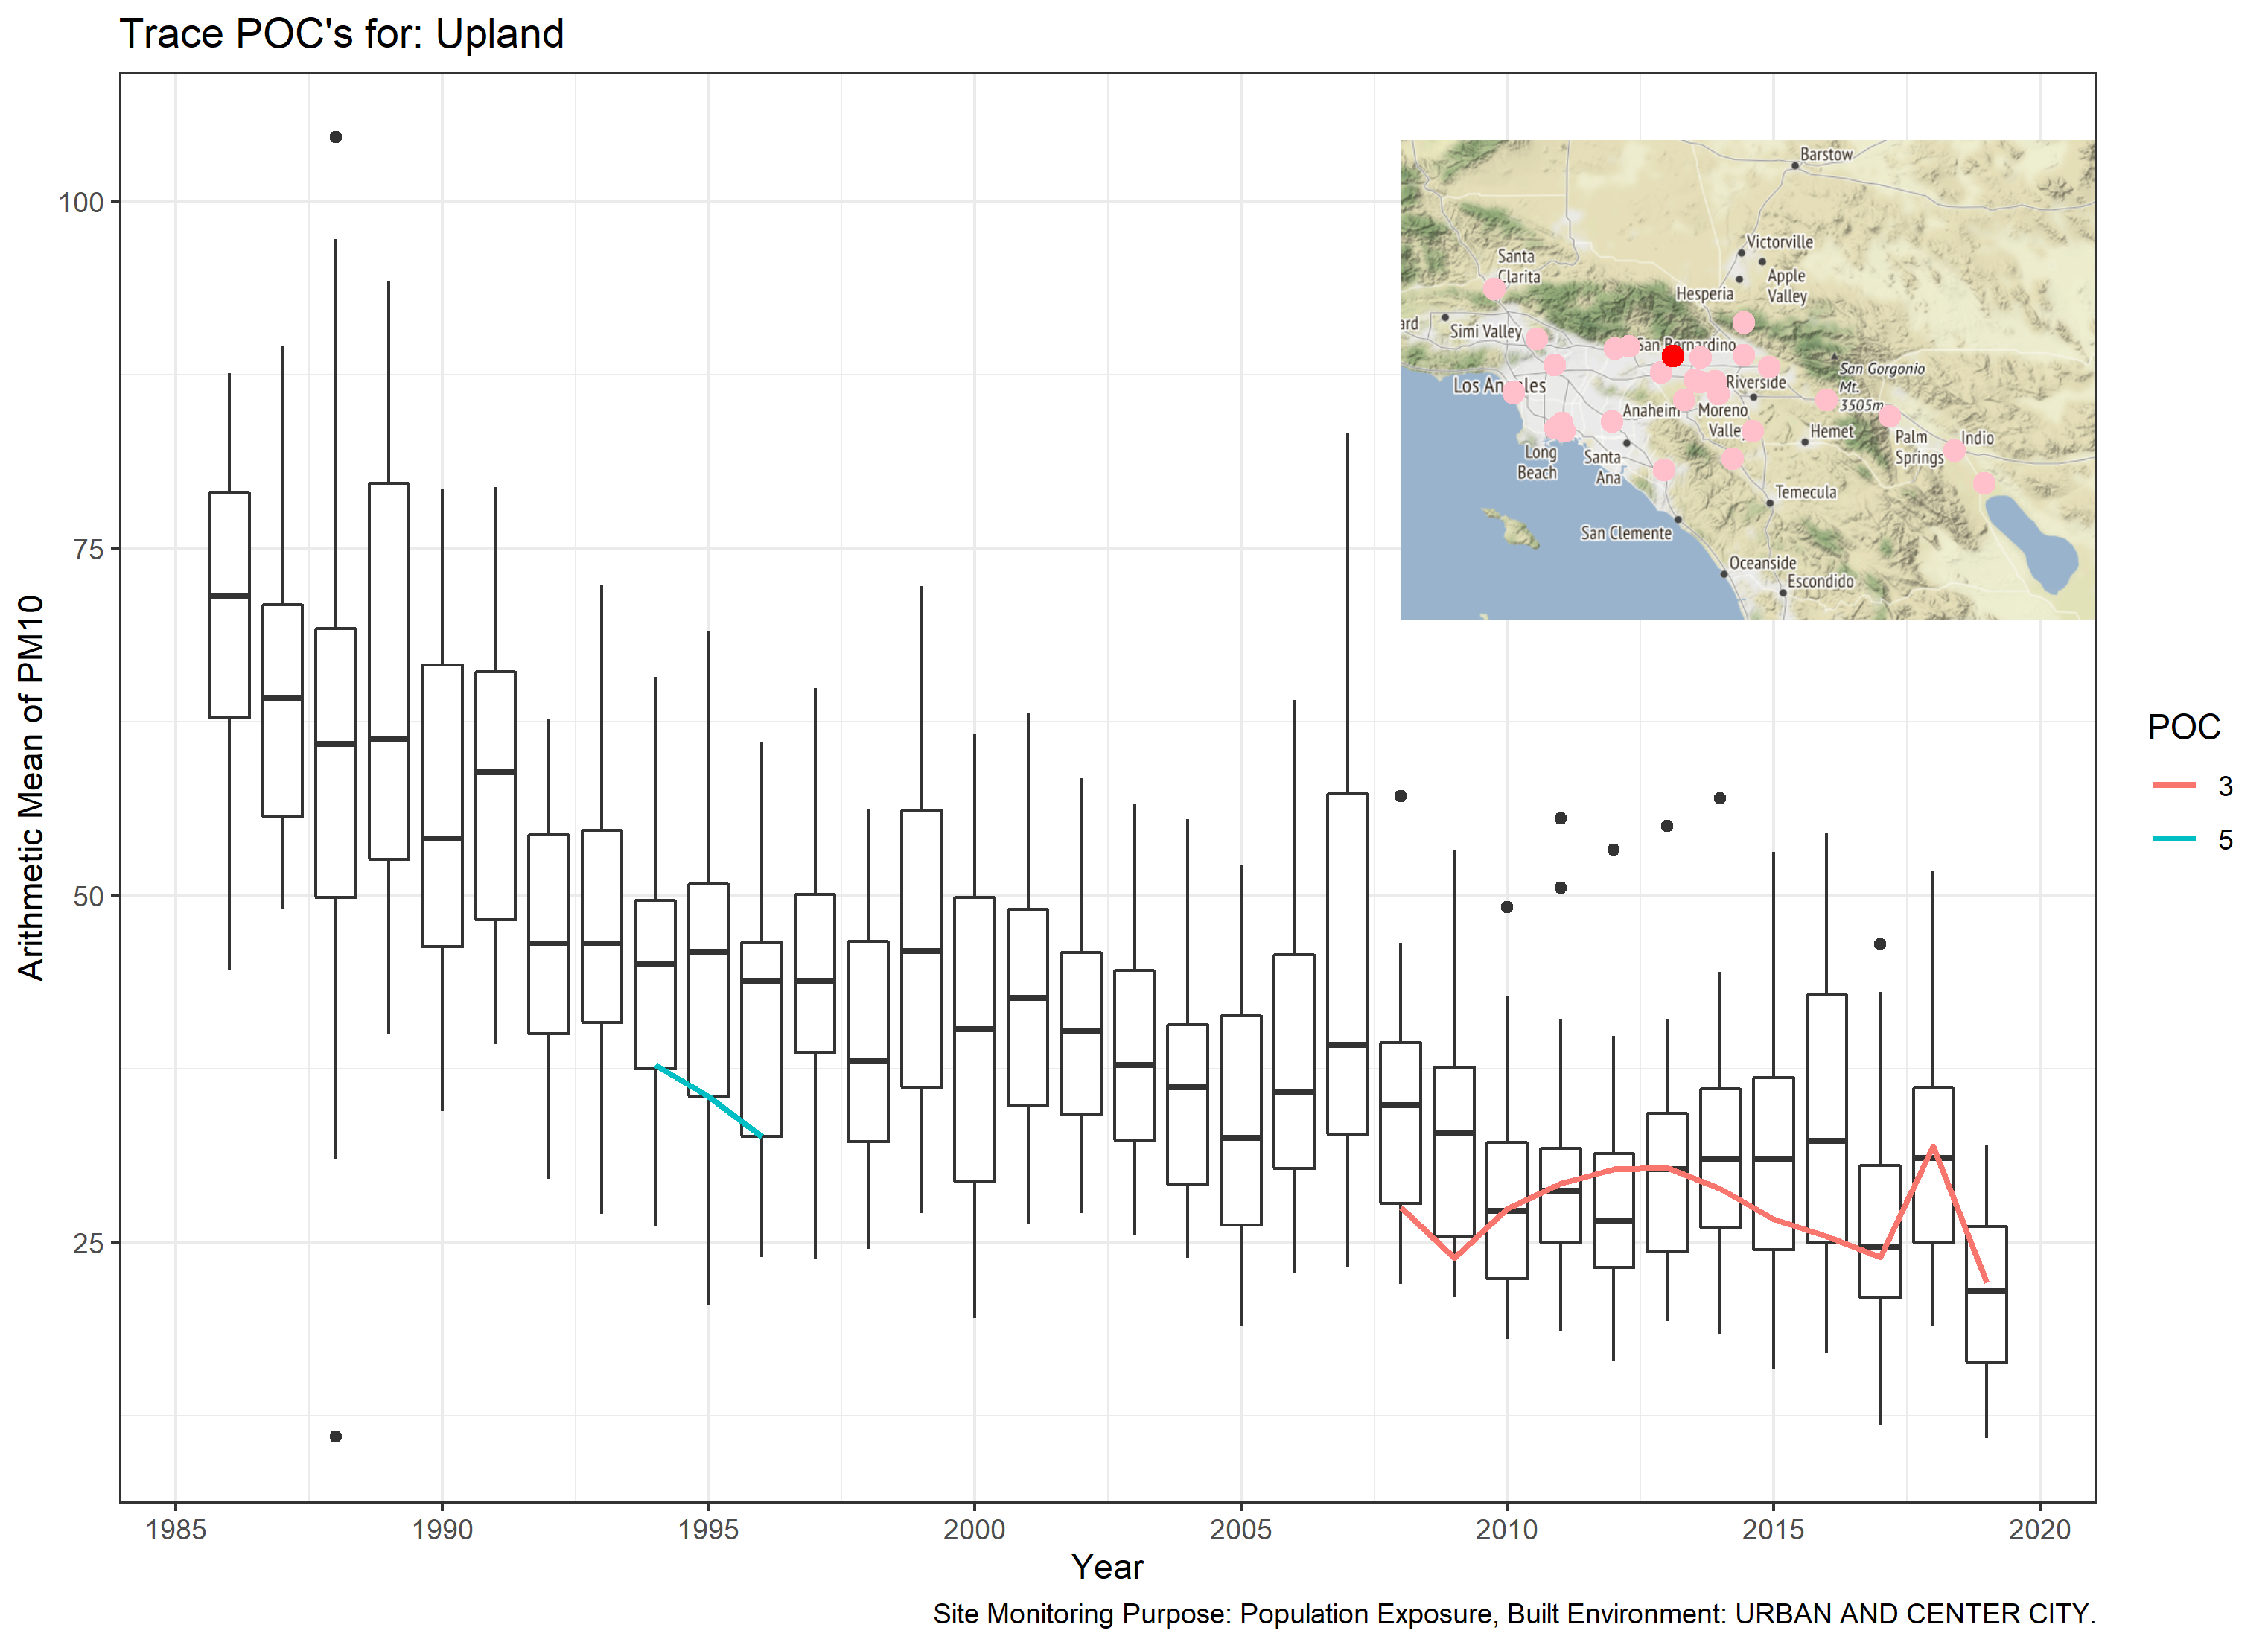}
    \caption{Caption}
    \label{fig:my_label}
\end{figure}
