# Supplementary material for: Preferential monitoring site location in the Southern California Air Quality Basin
Source: arXiv:2304.10006 source file (2023-04-19)
Supplement: Supplementary file 2 [file 99_AppendixB_PosteriorSurfaces.tex]

\section{Appendix B: Posterior Surfaces}
Posterior $log[PM_{10}]$ surfaces for the SOCAB for each year based upon the chosen model.  Solid dots are sites that provided data for that year, empty rings are stites that were present in that year but were randomly withheld for validation.

\begin{figure}
    \centering
    \includegraphics[width = \textwidth]{Figures/PosteriorSurface/SOCAB_posterior_surface_full_data_1986.png}
    \caption{Caption}
    \label{fig:my_label}
\end{figure}

\begin{figure}
    \centering
    \includegraphics[width = \textwidth]{Figures/PosteriorSurface/SOCAB_posterior_surface_full_data_1987.png}
    \caption{Caption}
    \label{fig:my_label}
\end{figure}

\begin{figure}
    \centering
    \includegraphics[width = \textwidth]{Figures/PosteriorSurface/SOCAB_posterior_surface_full_data_1988.png}
    \caption{Caption}
    \label{fig:my_label}
\end{figure}

\begin{figure}
    \centering
    \includegraphics[width = \textwidth]{Figures/PosteriorSurface/SOCAB_posterior_surface_full_data_1989.png}
    \caption{Caption}
    \label{fig:my_label}
\end{figure}

\begin{figure}
    \centering
    \includegraphics[width = \textwidth]{Figures/PosteriorSurface/SOCAB_posterior_surface_full_data_1990.png}
    \caption{Caption}
    \label{fig:my_label}
\end{figure}

\begin{figure}
    \centering
    \includegraphics[width = \textwidth]{Figures/PosteriorSurface/SOCAB_posterior_surface_full_data_1991.png}
    \caption{Caption}
    \label{fig:my_label}
\end{figure}

\begin{figure}
    \centering
    \includegraphics[width = \textwidth]{Figures/PosteriorSurface/SOCAB_posterior_surface_full_data_1992.png}
    \caption{Caption}
    \label{fig:my_label}
\end{figure}

\begin{figure}
    \centering
    \includegraphics[width = \textwidth]{Figures/PosteriorSurface/SOCAB_posterior_surface_full_data_1993.png}
    \caption{Caption}
    \label{fig:my_label}
\end{figure}

\begin{figure}
    \centering
    \includegraphics[width = \textwidth]{Figures/PosteriorSurface/SOCAB_posterior_surface_full_data_1994.png}
    \caption{Caption}
    \label{fig:my_label}
\end{figure}

\begin{figure}
    \centering
    \includegraphics[width = \textwidth]{Figures/PosteriorSurface/SOCAB_posterior_surface_full_data_1995.png}
    \caption{Caption}
    \label{fig:my_label}
\end{figure}

\begin{figure}
    \centering
    \includegraphics[width = \textwidth]{Figures/PosteriorSurface/SOCAB_posterior_surface_full_data_1996.png}
    \caption{Caption}
    \label{fig:my_label}
\end{figure}

\begin{figure}
    \centering
    \includegraphics[width = \textwidth]{Figures/PosteriorSurface/SOCAB_posterior_surface_full_data_1997.png}
    \caption{Caption}
    \label{fig:my_label}
\end{figure}

\begin{figure}
    \centering
    \includegraphics[width = \textwidth]{Figures/PosteriorSurface/SOCAB_posterior_surface_full_data_1998.png}
    \caption{Caption}
    \label{fig:my_label}
\end{figure}

\begin{figure}
    \centering
    \includegraphics[width = \textwidth]{Figures/PosteriorSurface/SOCAB_posterior_surface_full_data_1998.png}
    \caption{Caption}
    \label{fig:my_label}
\end{figure}

\begin{figure}
    \centering
    \includegraphics[width = \textwidth]{Figures/PosteriorSurface/SOCAB_posterior_surface_full_data_1999.png}
    \caption{Caption}
    \label{fig:my_label}
\end{figure}

\begin{figure}
    \centering
    \includegraphics[width = \textwidth]{Figures/PosteriorSurface/SOCAB_posterior_surface_full_data_2000.png}
    \caption{Caption}
    \label{fig:my_label}
\end{figure}

\begin{figure}
    \centering
    \includegraphics[width = \textwidth]{Figures/PosteriorSurface/SOCAB_posterior_surface_full_data_2001.png}
    \caption{Caption}
    \label{fig:my_label}
\end{figure}

\begin{figure}
    \centering
    \includegraphics[width = \textwidth]{Figures/PosteriorSurface/SOCAB_posterior_surface_full_data_2002.png}
    \caption{Caption}
    \label{fig:my_label}
\end{figure}

\begin{figure}
    \centering
    \includegraphics[width = \textwidth]{Figures/PosteriorSurface/SOCAB_posterior_surface_full_data_2003.png}
    \caption{Caption}
    \label{fig:my_label}
\end{figure}

\begin{figure}
    \centering
    \includegraphics[width = \textwidth]{Figures/PosteriorSurface/SOCAB_posterior_surface_full_data_2004.png}
    \caption{Caption}
    \label{fig:my_label}
\end{figure}

\begin{figure}
    \centering
    \includegraphics[width = \textwidth]{Figures/PosteriorSurface/SOCAB_posterior_surface_full_data_2005.png}
    \caption{Caption}
    \label{fig:my_label}
\end{figure}

\begin{figure}
    \centering
    \includegraphics[width = \textwidth]{Figures/PosteriorSurface/SOCAB_posterior_surface_full_data_2006.png}
    \caption{Caption}
    \label{fig:my_label}
\end{figure}

\begin{figure}
    \centering
    \includegraphics[width = \textwidth]{Figures/PosteriorSurface/SOCAB_posterior_surface_full_data_2007.png}
    \caption{Caption}
    \label{fig:my_label}
\end{figure}

\begin{figure}
    \centering
    \includegraphics[width = \textwidth]{Figures/PosteriorSurface/SOCAB_posterior_surface_full_data_2008.png}
    \caption{Caption}
    \label{fig:my_label}
\end{figure}

\begin{figure}
    \centering
    \includegraphics[width = \textwidth]{Figures/PosteriorSurface/SOCAB_posterior_surface_full_data_2009.png}
    \caption{Caption}
    \label{fig:my_label}
\end{figure}

\begin{figure}
    \centering
    \includegraphics[width = \textwidth]{Figures/PosteriorSurface/SOCAB_posterior_surface_full_data_2010.png}
    \caption{Caption}
    \label{fig:my_label}
\end{figure}

\begin{figure}
    \centering
    \includegraphics[width = \textwidth]{Figures/PosteriorSurface/SOCAB_posterior_surface_full_data_2011.png}
    \caption{Caption}
    \label{fig:my_label}
\end{figure}

\begin{figure}
    \centering
    \includegraphics[width = \textwidth]{Figures/PosteriorSurface/SOCAB_posterior_surface_full_data_2012.png}
    \caption{Caption}
    \label{fig:my_label}
\end{figure}

\begin{figure}
    \centering
    \includegraphics[width = \textwidth]{Figures/PosteriorSurface/SOCAB_posterior_surface_full_data_2013.png}
    \caption{Caption}
    \label{fig:my_label}
\end{figure}

\begin{figure}
    \centering
    \includegraphics[width = \textwidth]{Figures/PosteriorSurface/SOCAB_posterior_surface_full_data_2014.png}
    \caption{Caption}
    \label{fig:my_label}
\end{figure}

\begin{figure}
    \centering
    \includegraphics[width = \textwidth]{Figures/PosteriorSurface/SOCAB_posterior_surface_full_data_2015.png}
    \caption{Caption}
    \label{fig:my_label}
\end{figure}

\begin{figure}
    \centering
    \includegraphics[width = \textwidth]{Figures/PosteriorSurface/SOCAB_posterior_surface_full_data_2016.png}
    \caption{Caption}
    \label{fig:my_label}
\end{figure}

\begin{figure}
    \centering
    \includegraphics[width = \textwidth]{Figures/PosteriorSurface/SOCAB_posterior_surface_full_data_2017.png}
    \caption{Caption}
    \label{fig:my_label}
\end{figure}

\begin{figure}
    \centering
    \includegraphics[width = \textwidth]{Figures/PosteriorSurface/SOCAB_posterior_surface_full_data_2018.png}
    \caption{Caption}
    \label{fig:my_label}
\end{figure}

\begin{figure}
    \centering
    \includegraphics[width = \textwidth]{Figures/PosteriorSurface/SOCAB_posterior_surface_full_data_2019.png}
    \caption{Caption}
    \label{fig:my_label}
\end{figure}
