# Supplementary material for: Preferential monitoring site location in the Southern California Air Quality Basin
Source: arXiv:2304.10006 source file (2023-04-19)
Supplement: Supplementary file 3 [file 99_AppendixC_Empirical_Variograms.tex]

\section{Appendix C: Emprirical Variograms}
This appendix shows the empirical variograms created for each year.  The esimations were made with the gstat package in R, use the Matern covariance function with smoothness parameter = 1, and have a maximum distance for computed semivariance of 80 km.

\begin{table}[]
    \centering
    \begin{tabular}{c|c|c|c}
         Year & Nugget & Partial Sill & Range  \\
         \hline
  1986 & 0.012977223 & 0.13793025 & 256.459508 \\
  1987 & 0.015558573 & 2.00537021 & 959.339340 \\
  1988 & 0.000000000 & 4.73672413 & 326.835196 \\
  1989 & 0.000000000 & 0.00000000 &  21.220809 \\
  1990 & 0.000000000 & 0.10044074 &  12.466310 \\
  1991 & 0.000000000 & 0.00000000 &  21.220809 \\
  1992 & 0.000000000 & 0.00000000 &  21.220809 \\
  1993 & 0.000000000 & 0.07718755 &  8.902779 \\
  1994 & 0.000000000 & 0.00000000 &  21.660305 \\
 1995 & 0.083175525 & 0.03778688  & 11.954476 \\
 1996 & 0.062804689 & 0.01244786  &  9.682597 \\
 1997 & 0.000000000 & 0.00000000  & 21.220809 \\
 1998 & 0.000000000 & 0.11058498  & 19.271236 \\
 1999 & 0.000000000 & 0.14840875  & 19.880071 \\
 2000 & 0.000000000 & 0.13607341  & 17.772735 \\
 2001 & 0.038460624 & 0.08470039  & 50.909427 \\
 2002 & 0.005274554 & 0.14179969  & 58.001995 \\
 2003 & 0.011903062 & 0.06156377  & 17.796257 \\
 2004 & 0.004499666 & 0.05171316  &  9.394408 \\
 2005 & 0.059160045 & 46.62114477 & 2882.078708 \\
 2006 & 0.030355313 & 0.10904731  & 24.959699 \\
 2007 & 0.023058025 & 0.18711240  & 26.154094 \\
 2008 & 0.034640584 & 0.02745581  & 10.423383 \\
 2009 & 0.017772428 & 0.04046641  &  5.373636 \\
 2010 & 0.025761760 & 0.05648380  & 36.022770 \\
 2011 & 0.052282701 & 0.81556428 & 359.096106 \\
 2012 & 0.000000000 & 0.06252610  & 10.024093 \\
 2013 & 0.000000000 & 0.05186647  &  8.209326 \\
 2014 & 0.010952103 & 0.05946016  & 11.180113 \\
 2015 & 0.000000000 & 0.07556357  &  4.337855 \\
 2016 & 0.000000000 & 0.07011386  &  6.606370 \\
 2017 & 0.034560403 & 0.04645220  & 11.231063 \\
 2018 & 0.033971352 & 0.04685213  & 36.916630 \\
 2019 & 0.079977592 & 3.32009680 & 795.047015 \\
\end{tabular}
    \caption{The parameters estimated for the empirical variograms of each year in the SOCAB. We can see how widely the estimated parameters vary, particularly for the range. Figures showing the empirical variograms are in the appendix.}
    \label{tab:Emperical_Variogram_Parameter}
\end{table}

\begin{figure}
    \centering
    \includegraphics{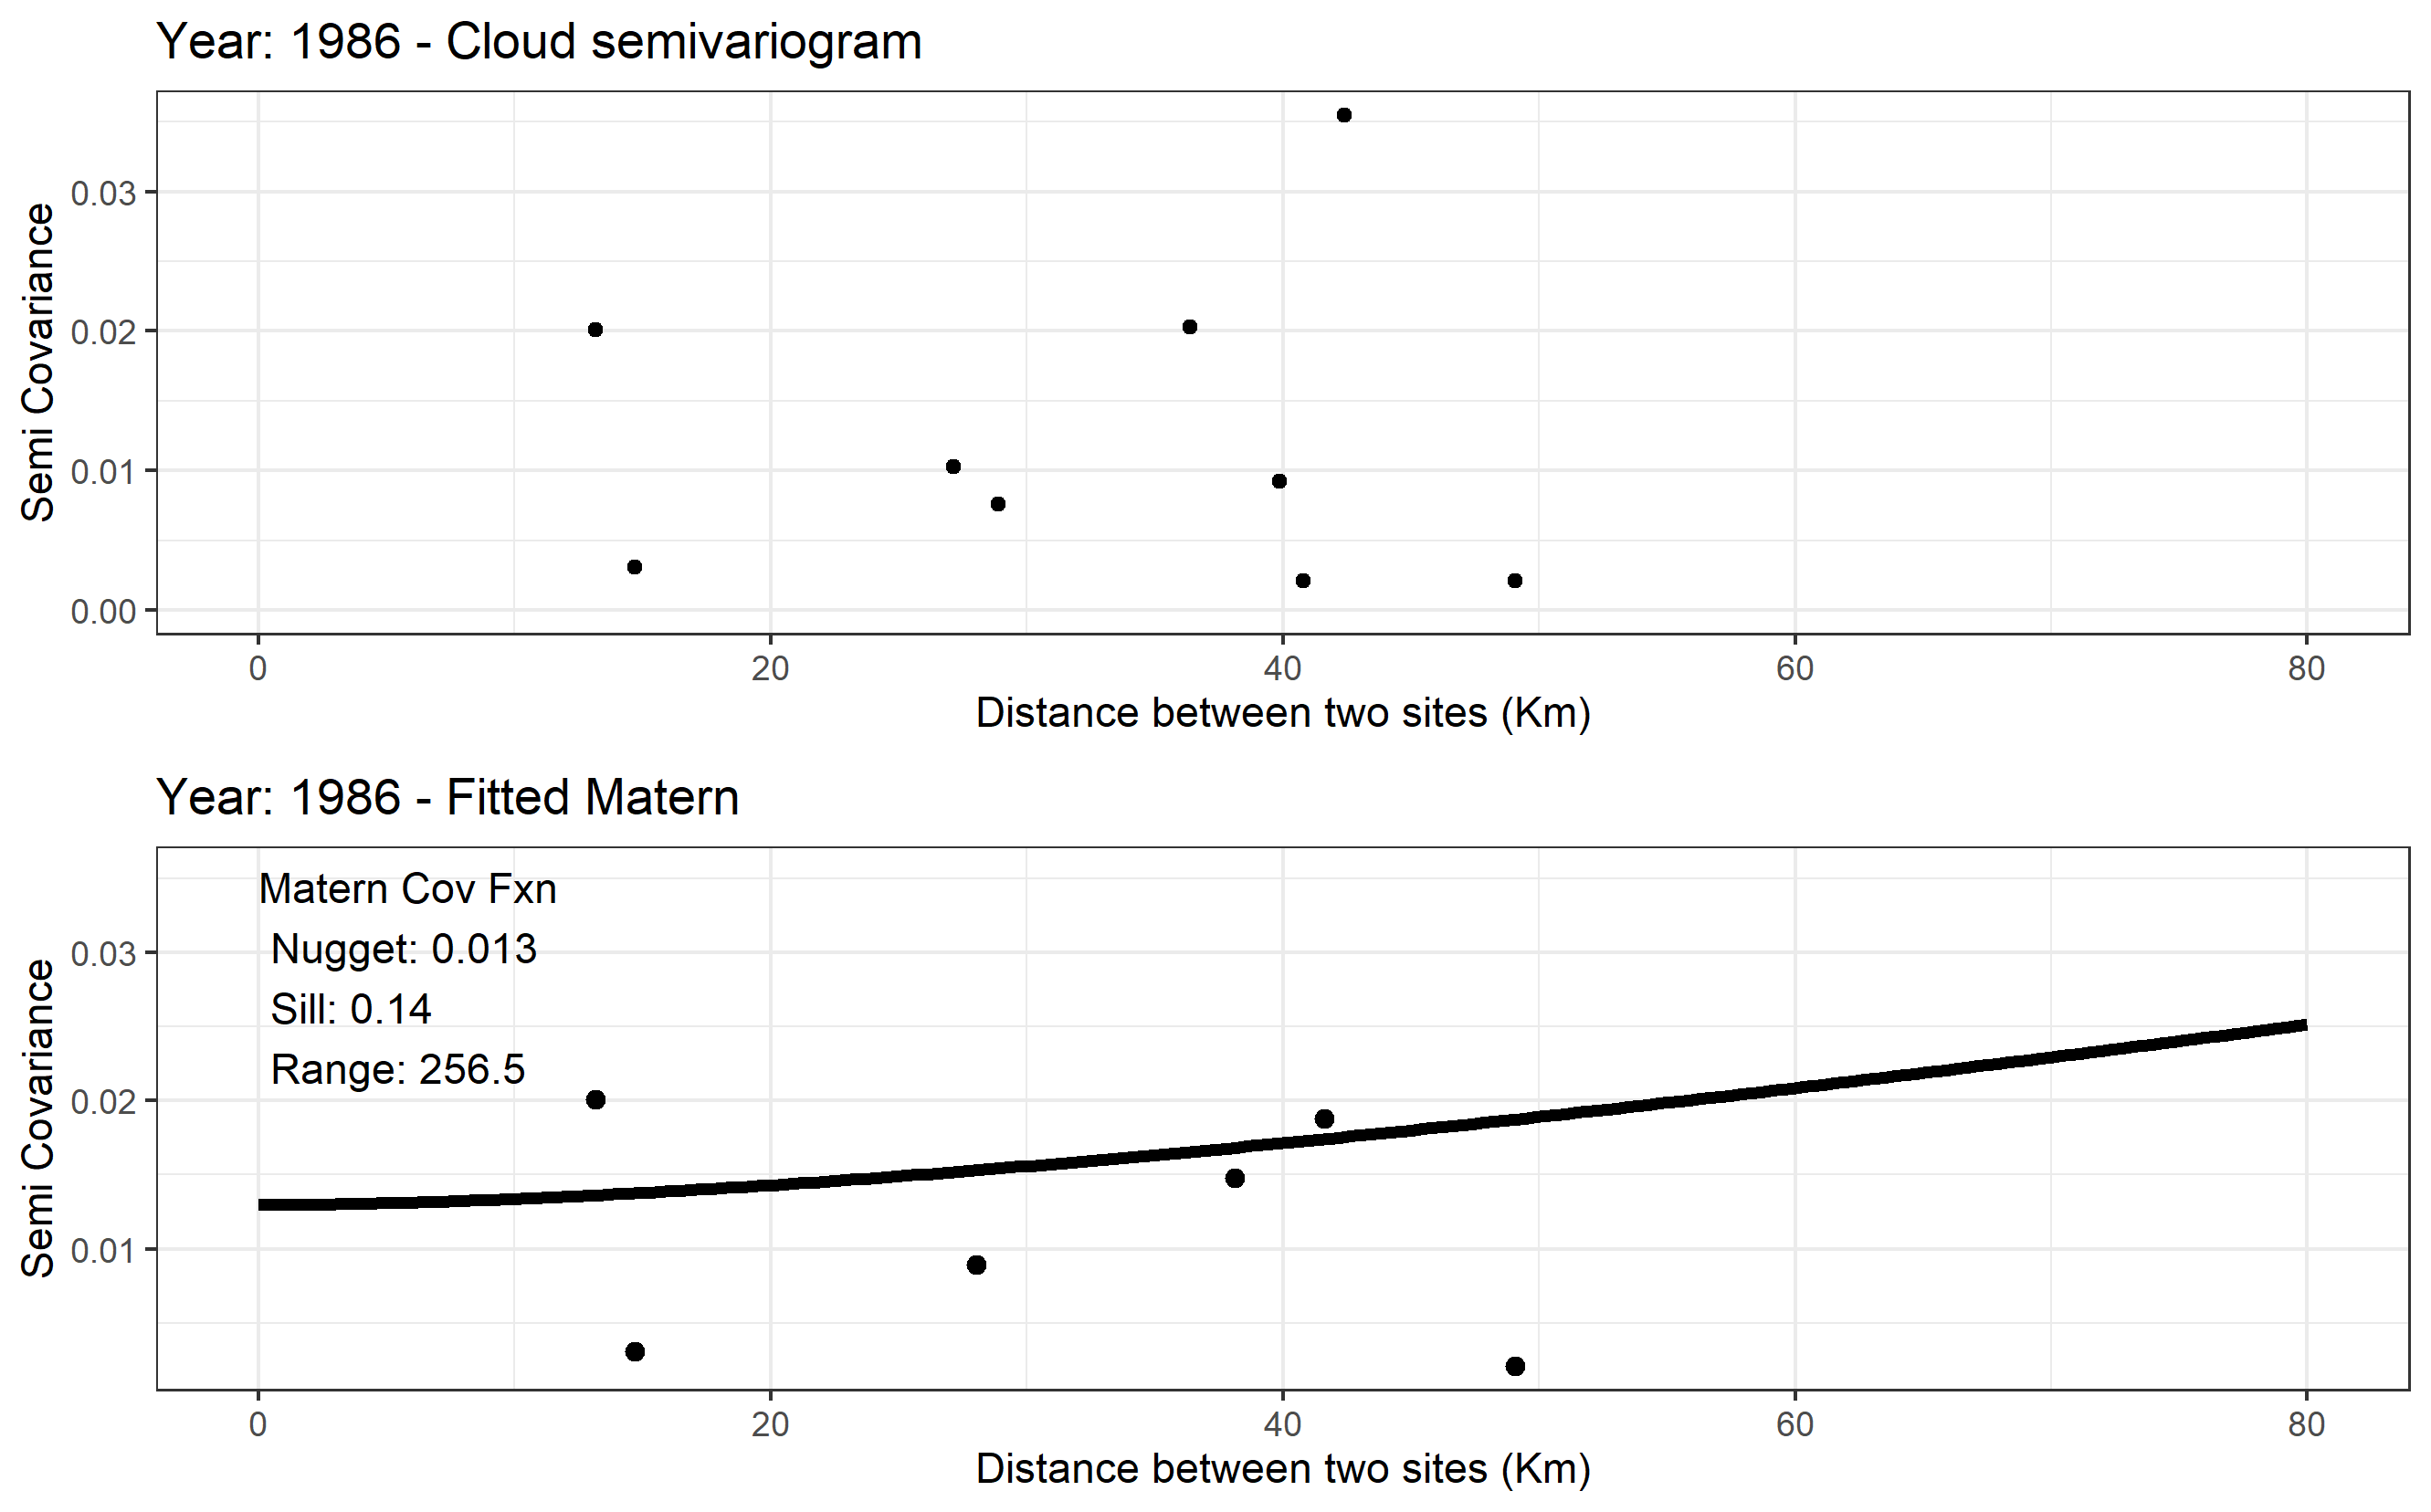}
    \caption{Caption}
    \label{fig:my_label}
\end{figure}

\begin{figure}
    \centering
    \includegraphics{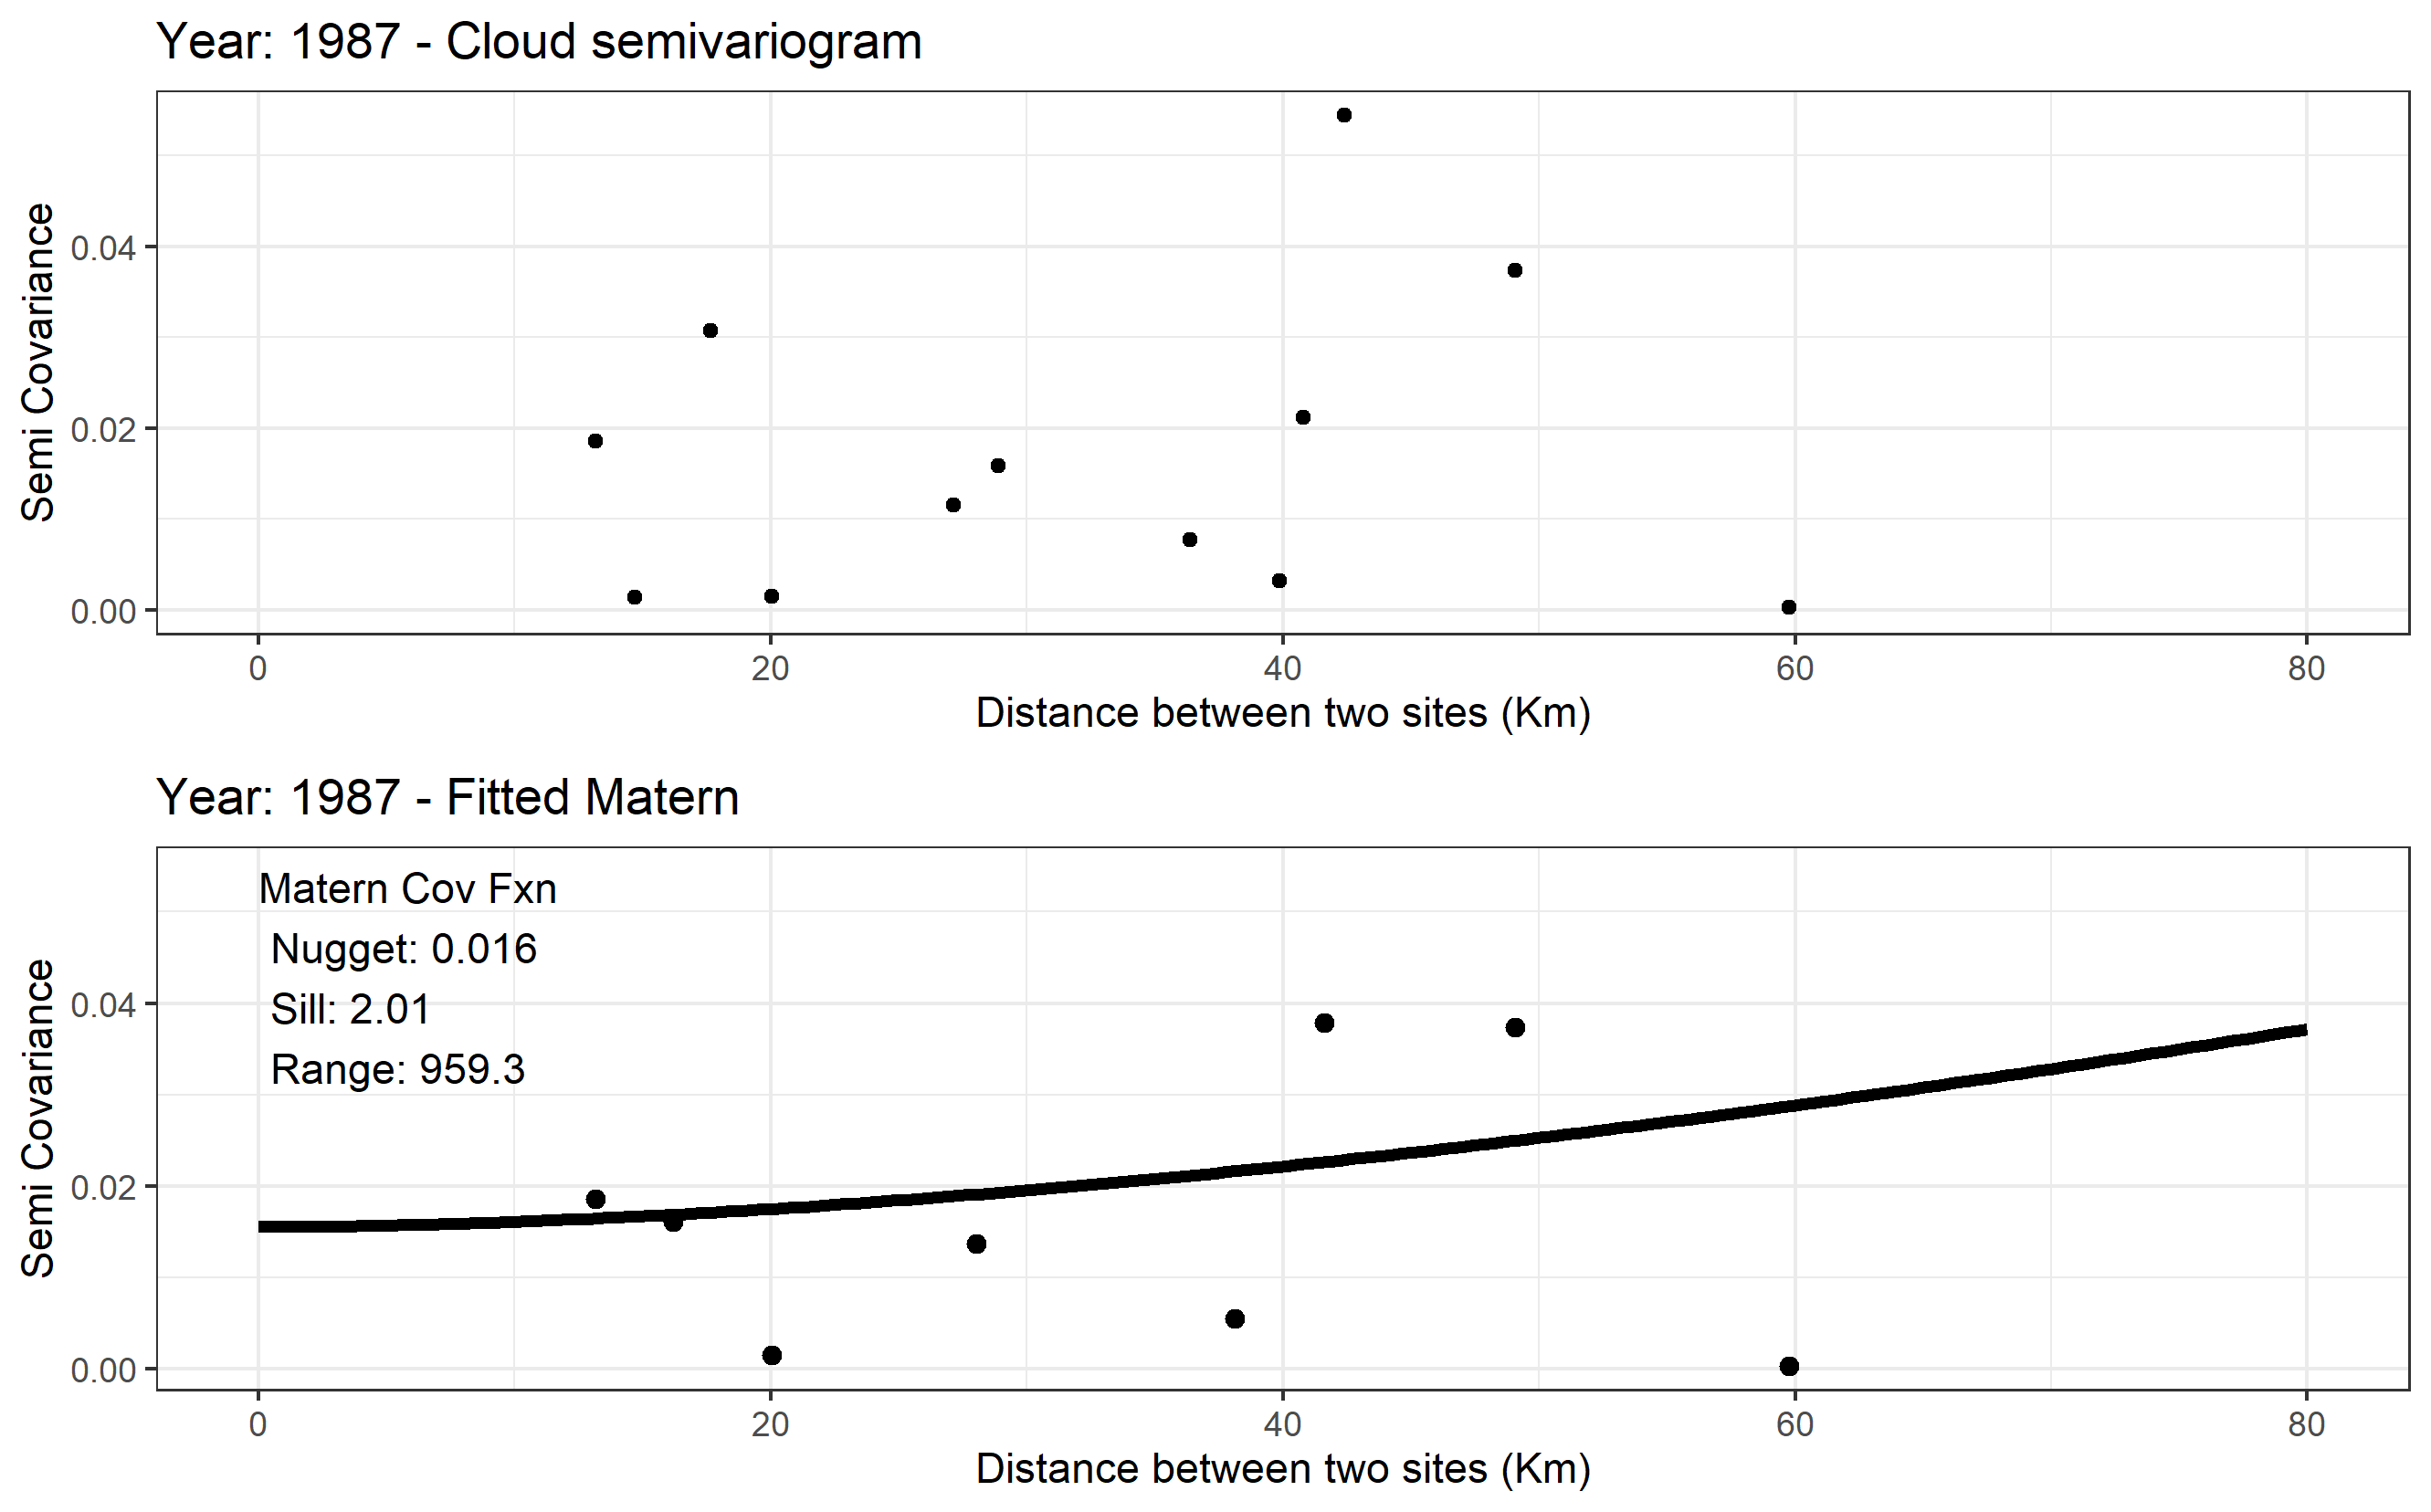}
    \caption{Caption}
    \label{fig:my_label}
\end{figure}

\begin{figure}
    \centering
    \includegraphics{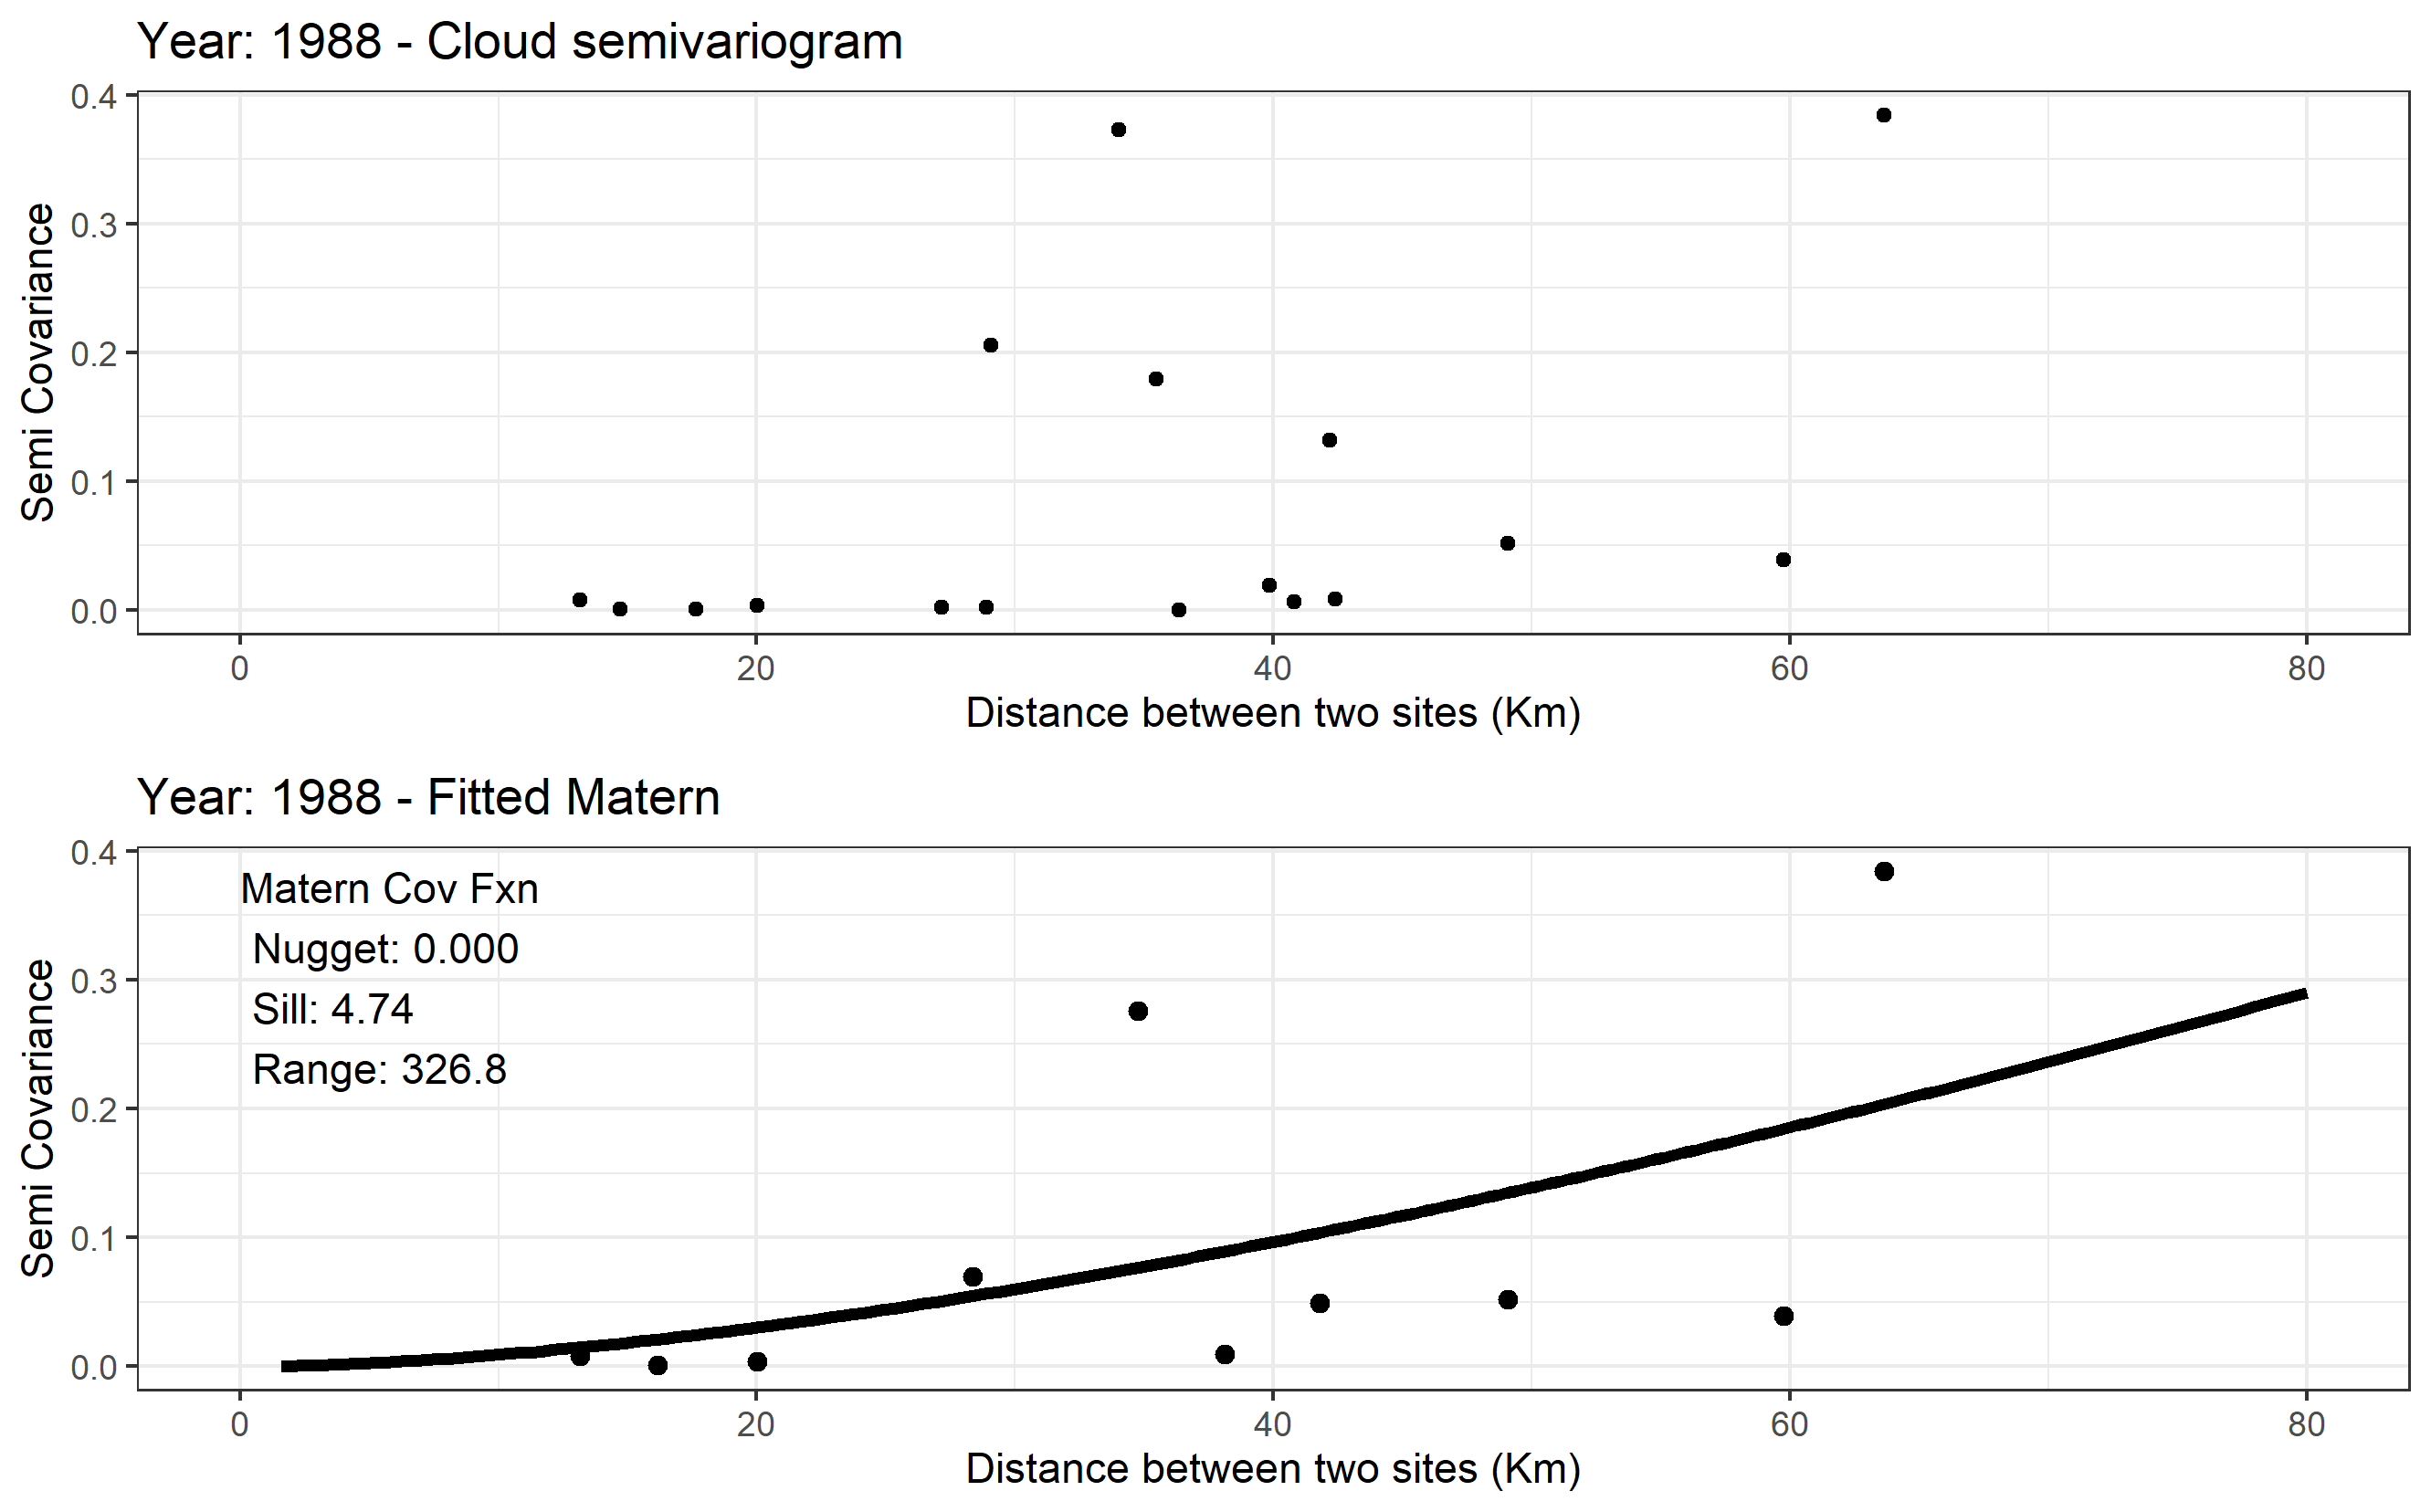}
    \caption{Caption}
    \label{fig:my_label}
\end{figure}

\begin{figure}
    \centering
    \includegraphics{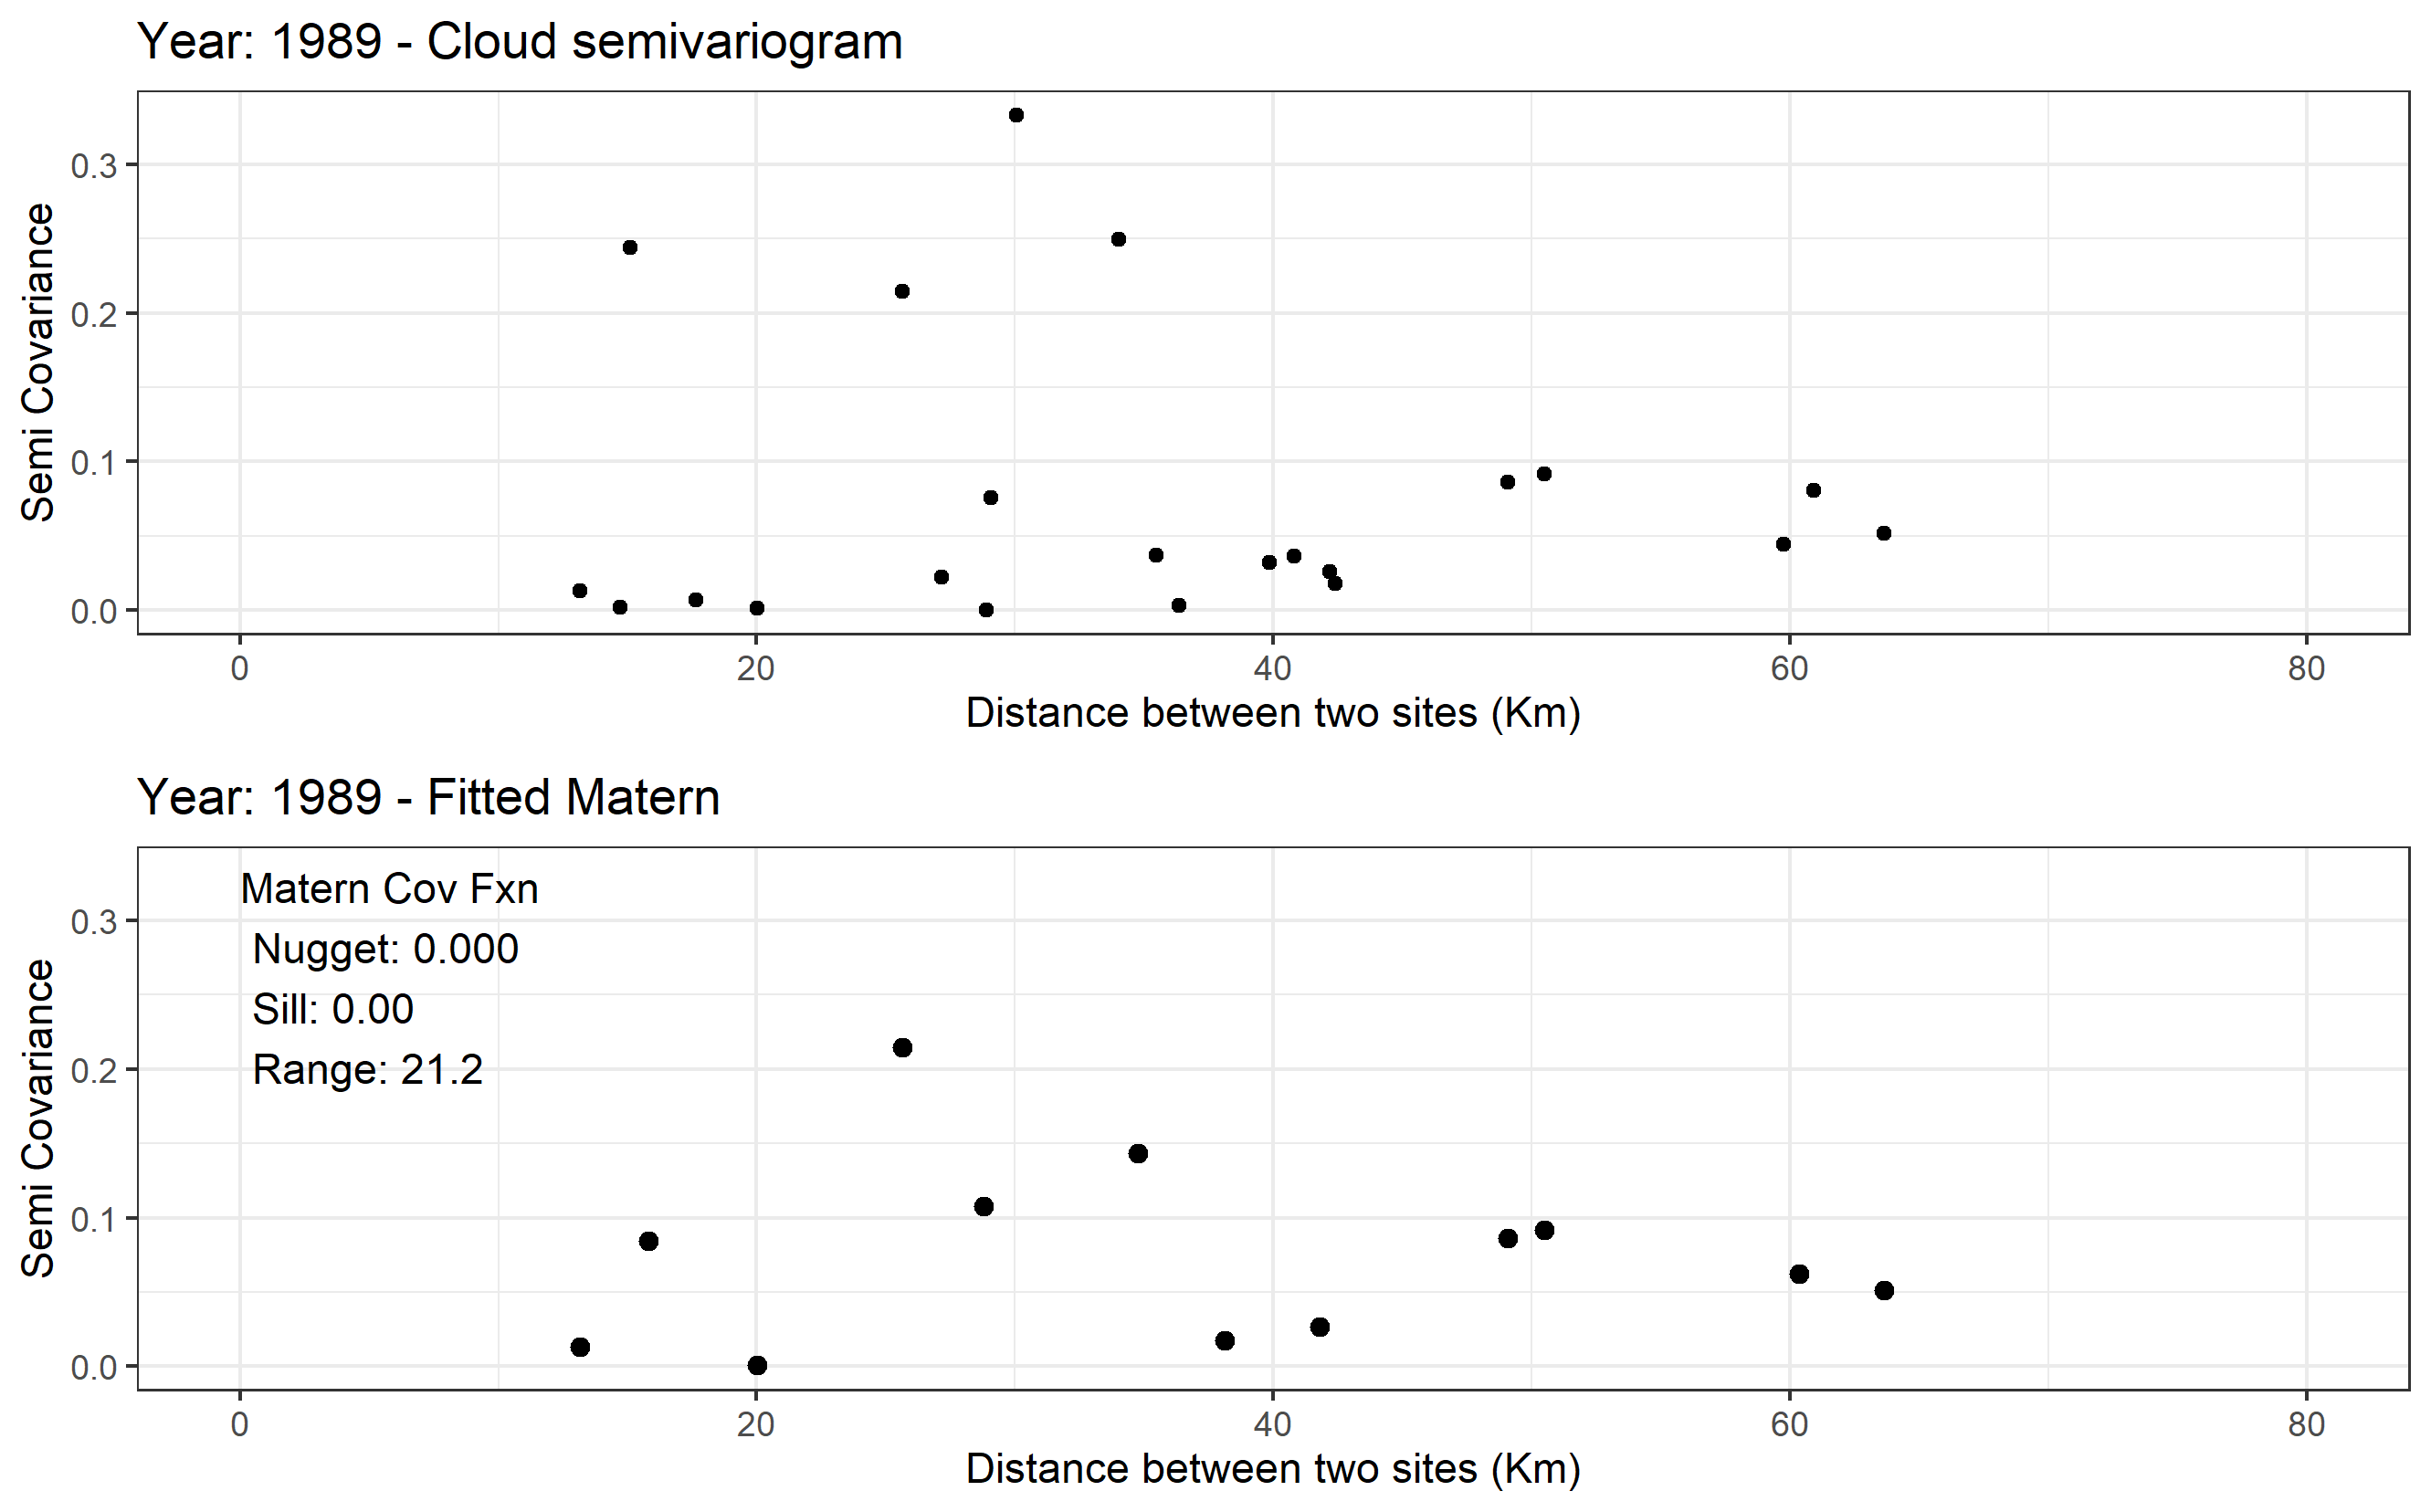}
    \caption{Caption}
    \label{fig:my_label}
\end{figure}

\begin{figure}
    \centering
    \includegraphics{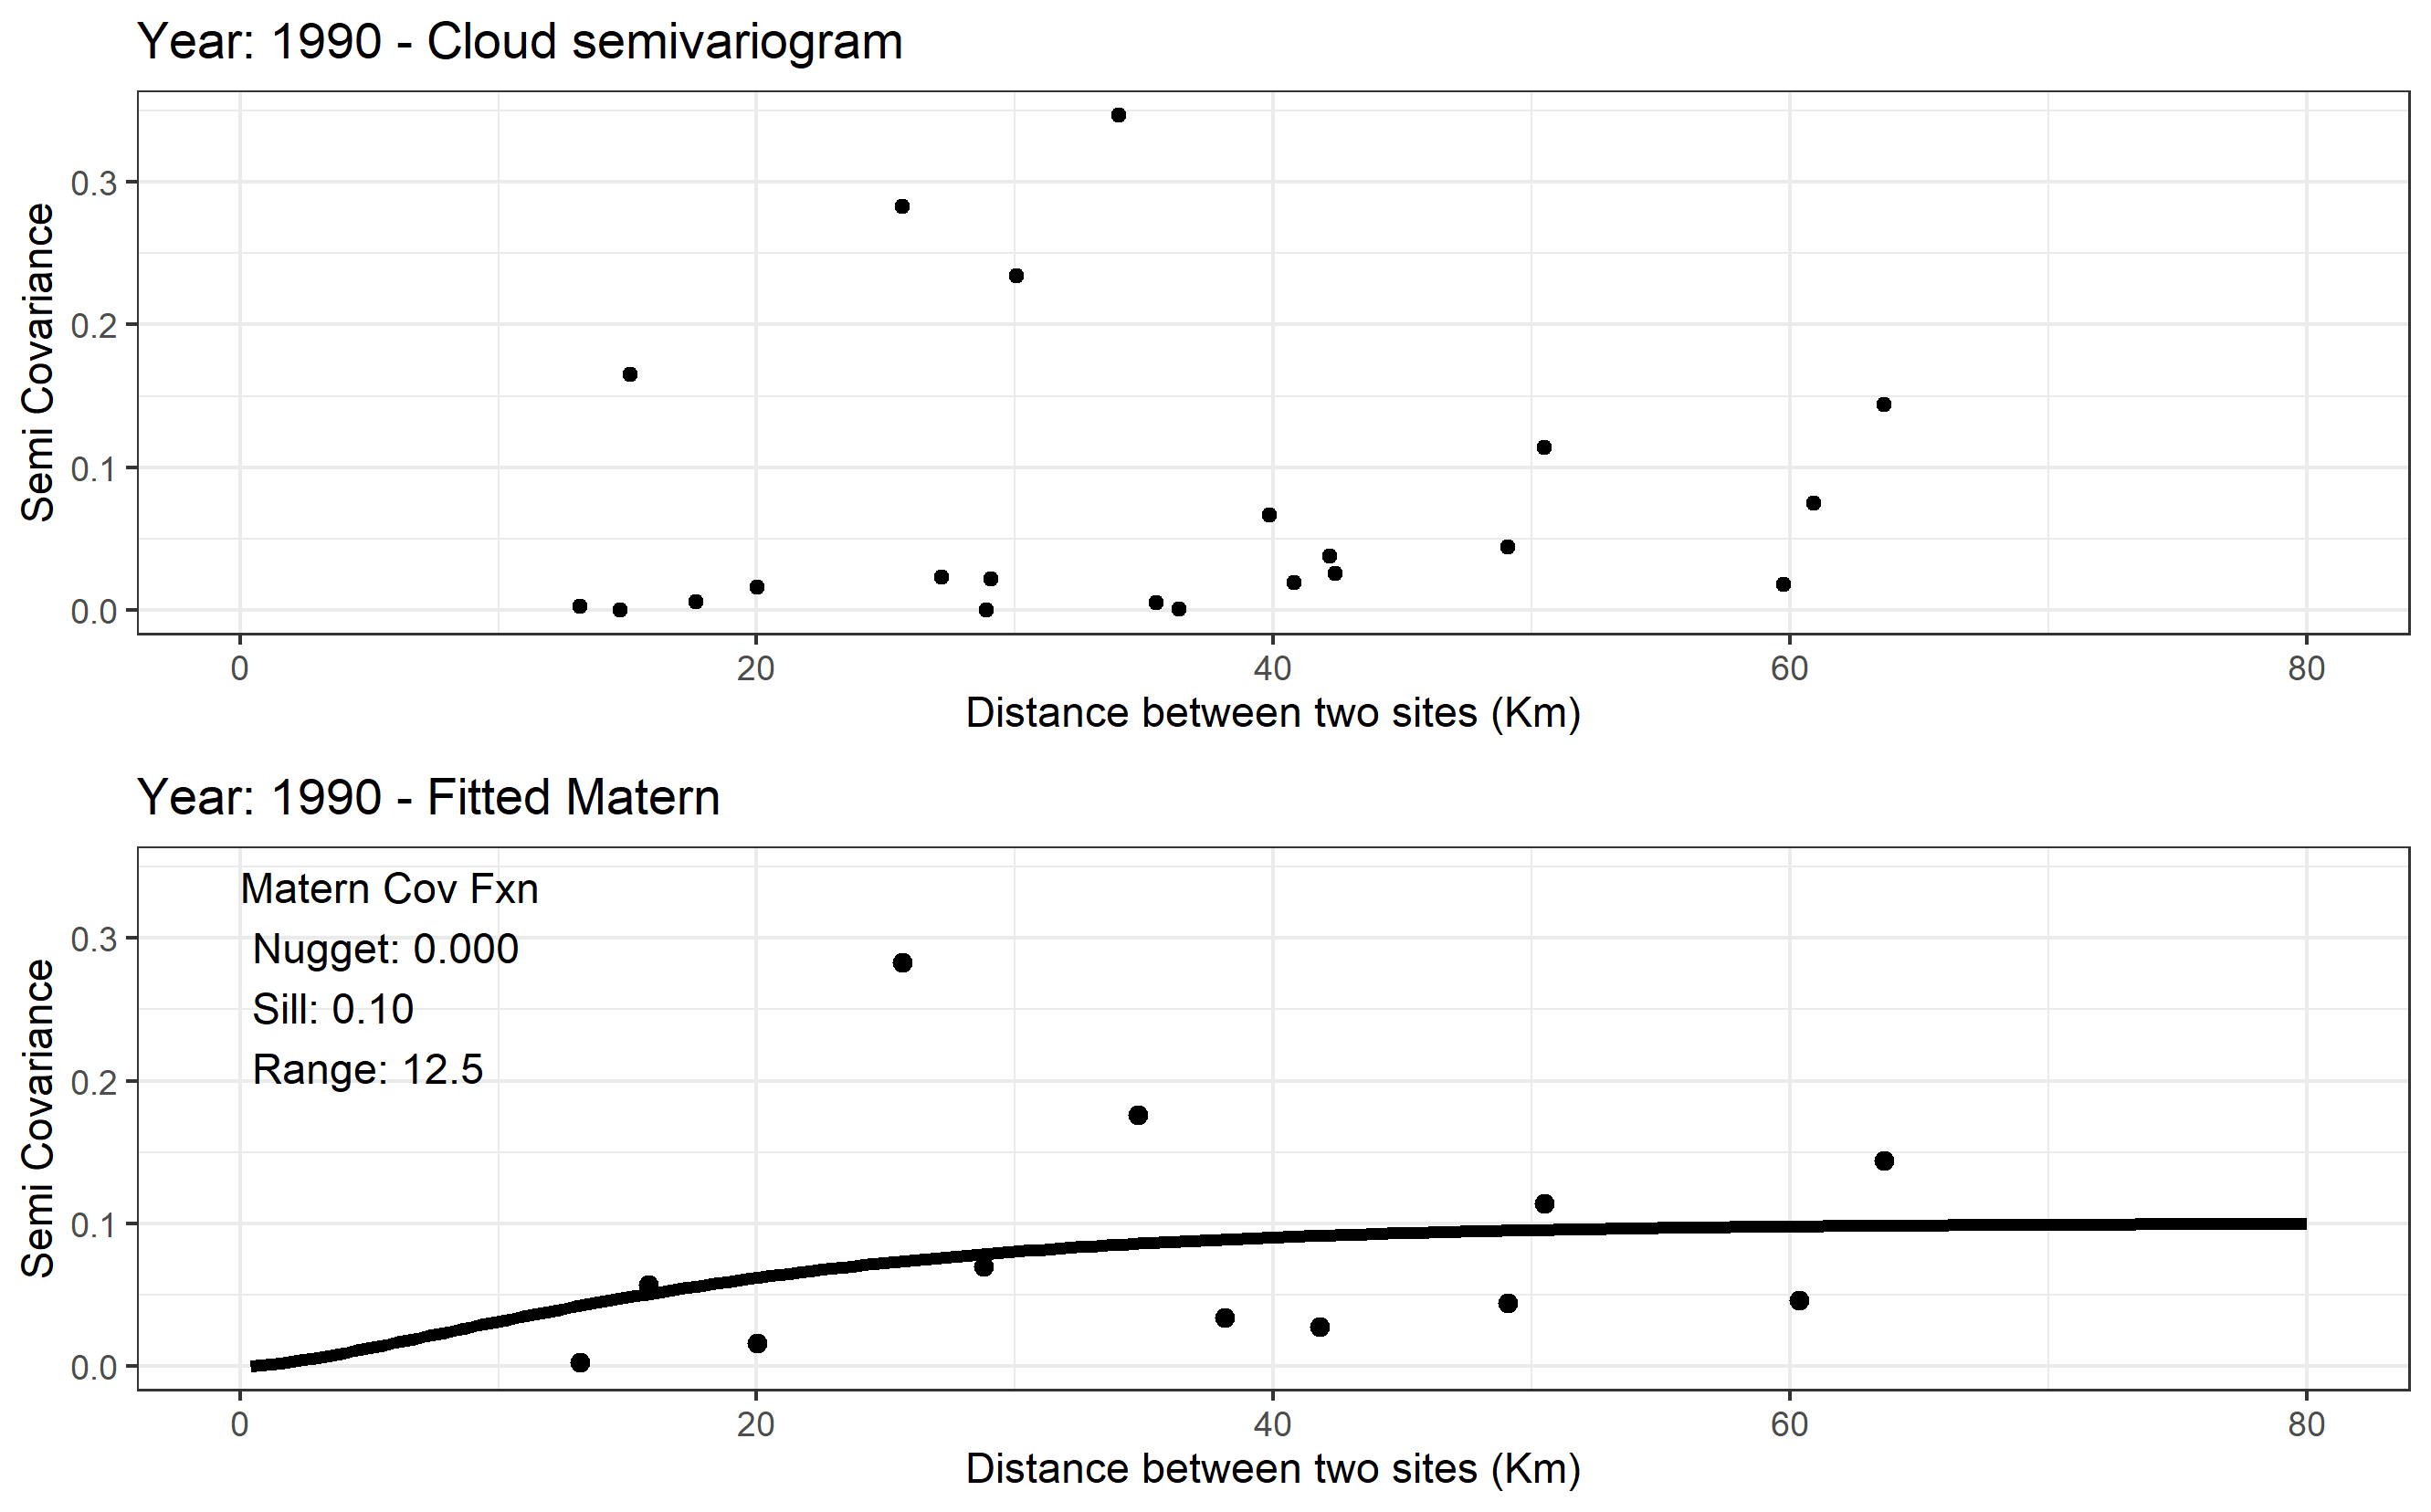}
    \caption{Caption}
    \label{fig:my_label}
\end{figure}

\begin{figure}
    \centering
    \includegraphics{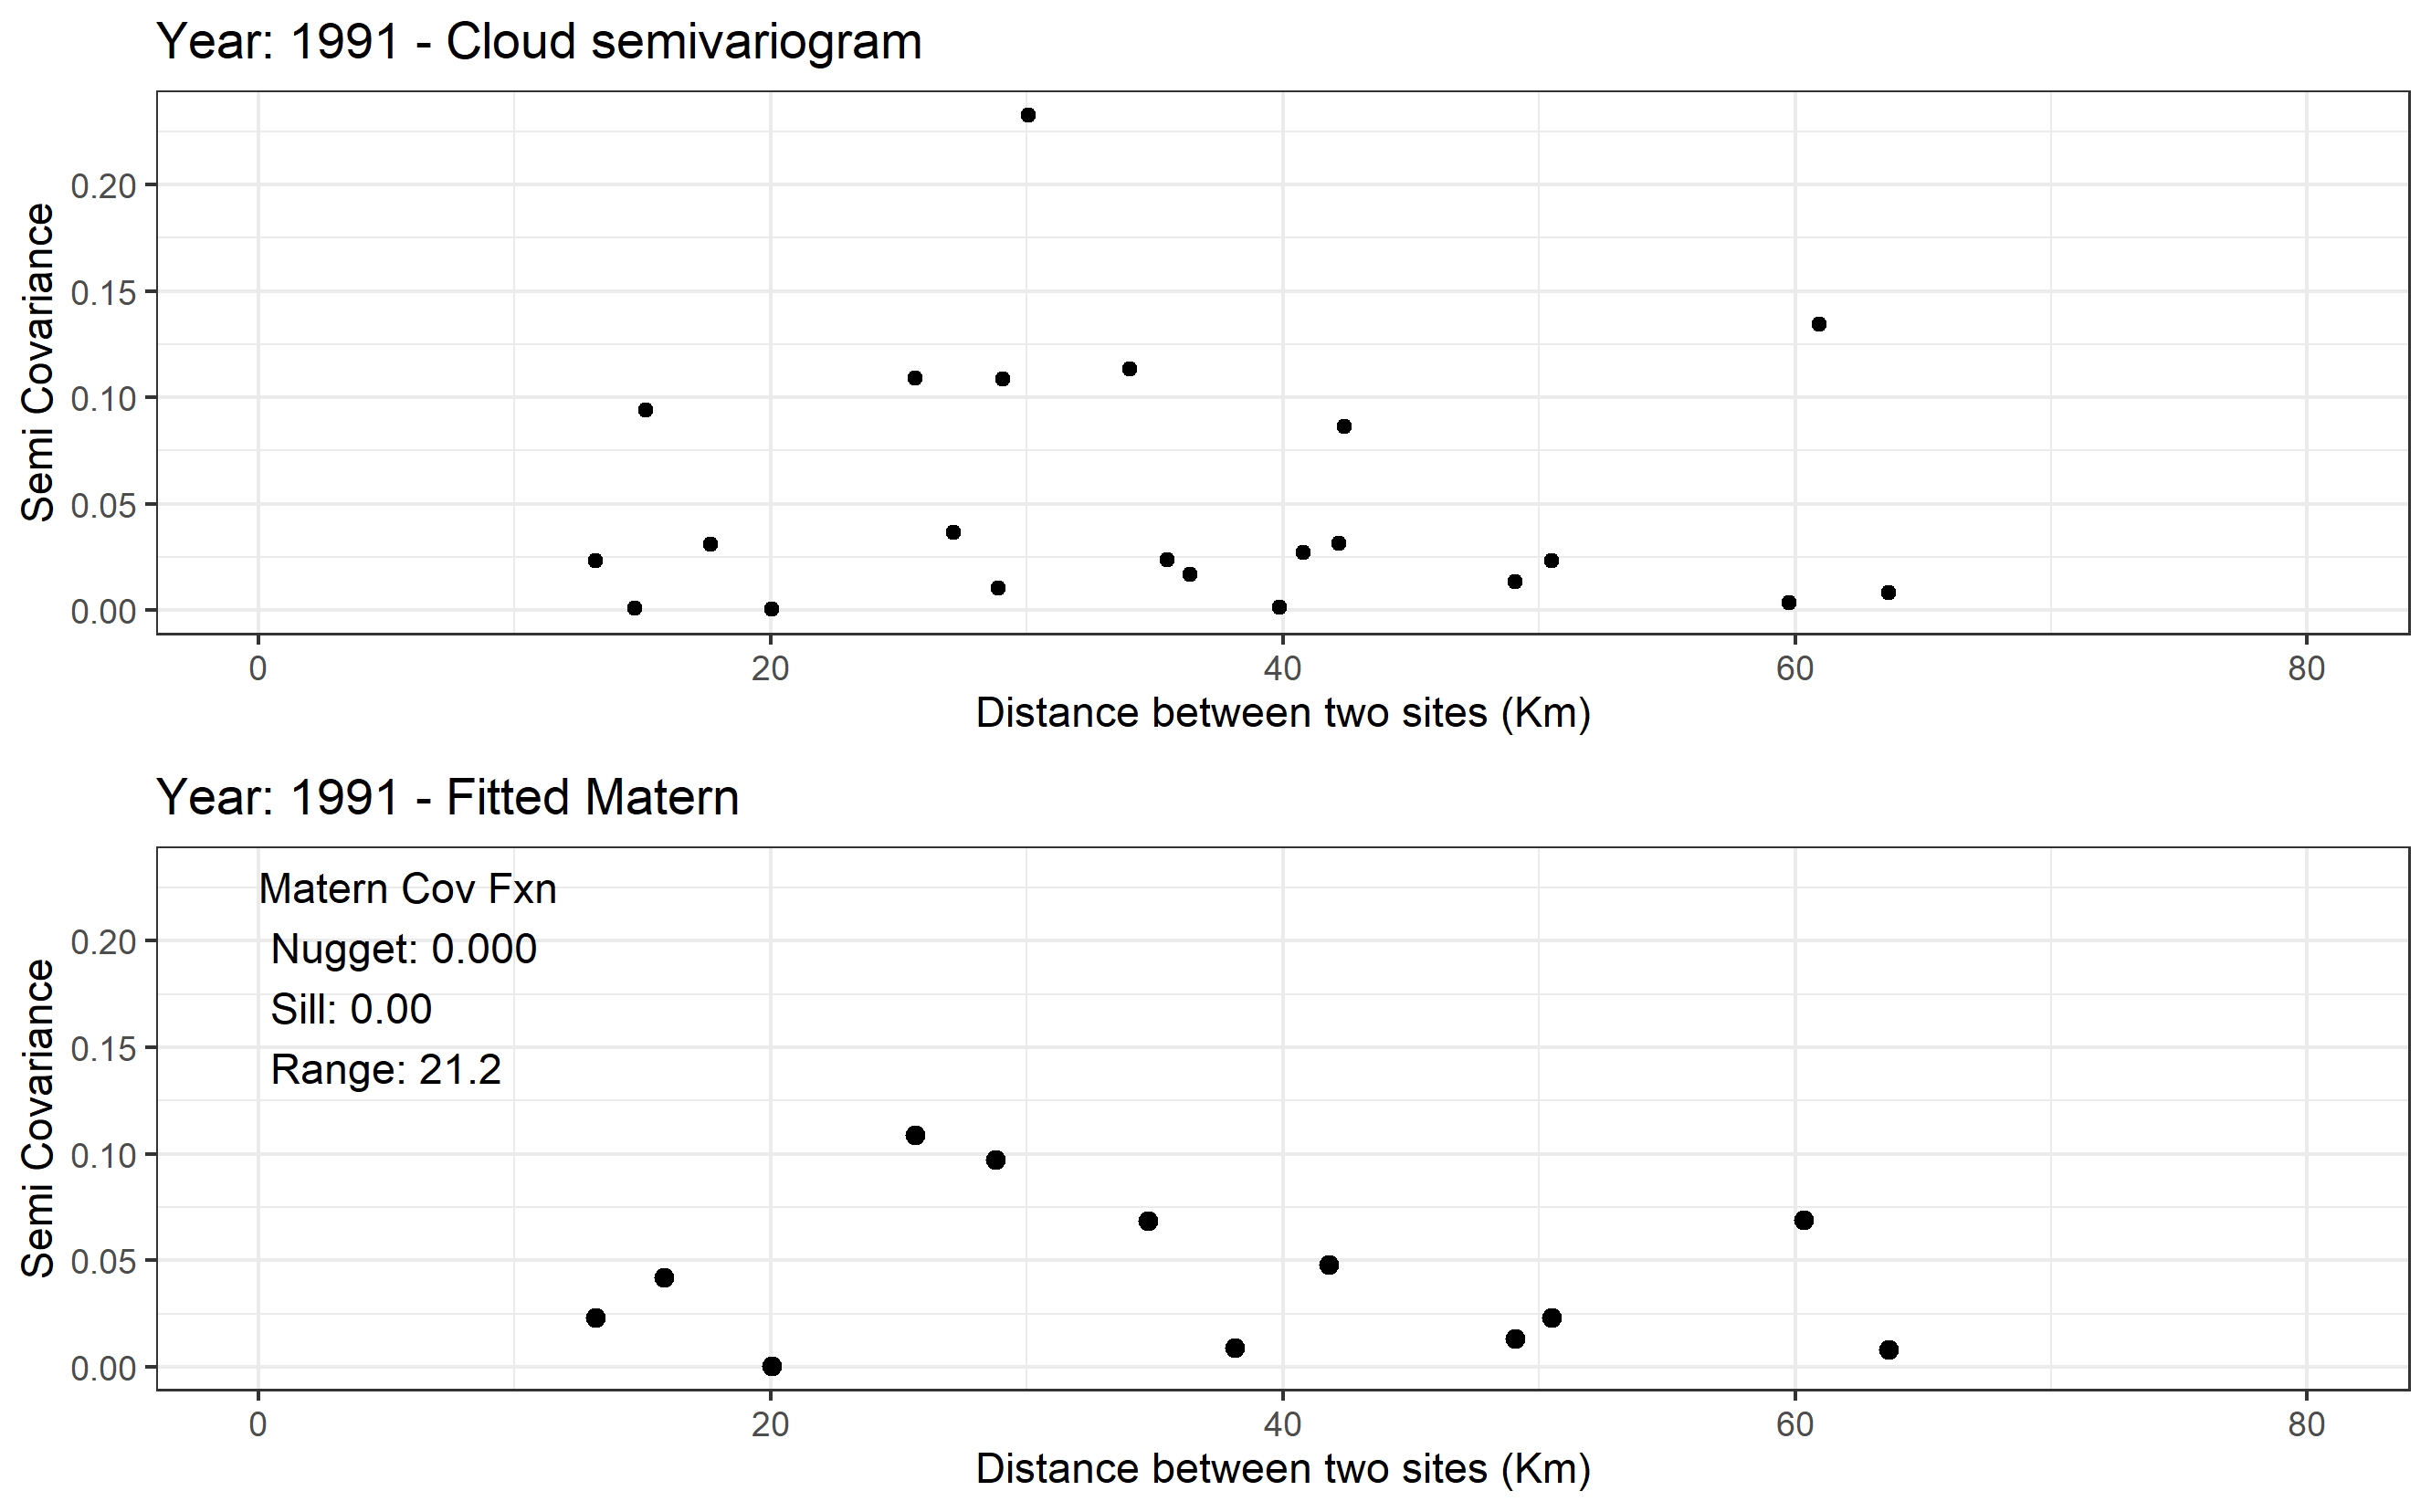}
    \caption{Caption}
    \label{fig:my_label}
\end{figure}

\begin{figure}
    \centering
    \includegraphics{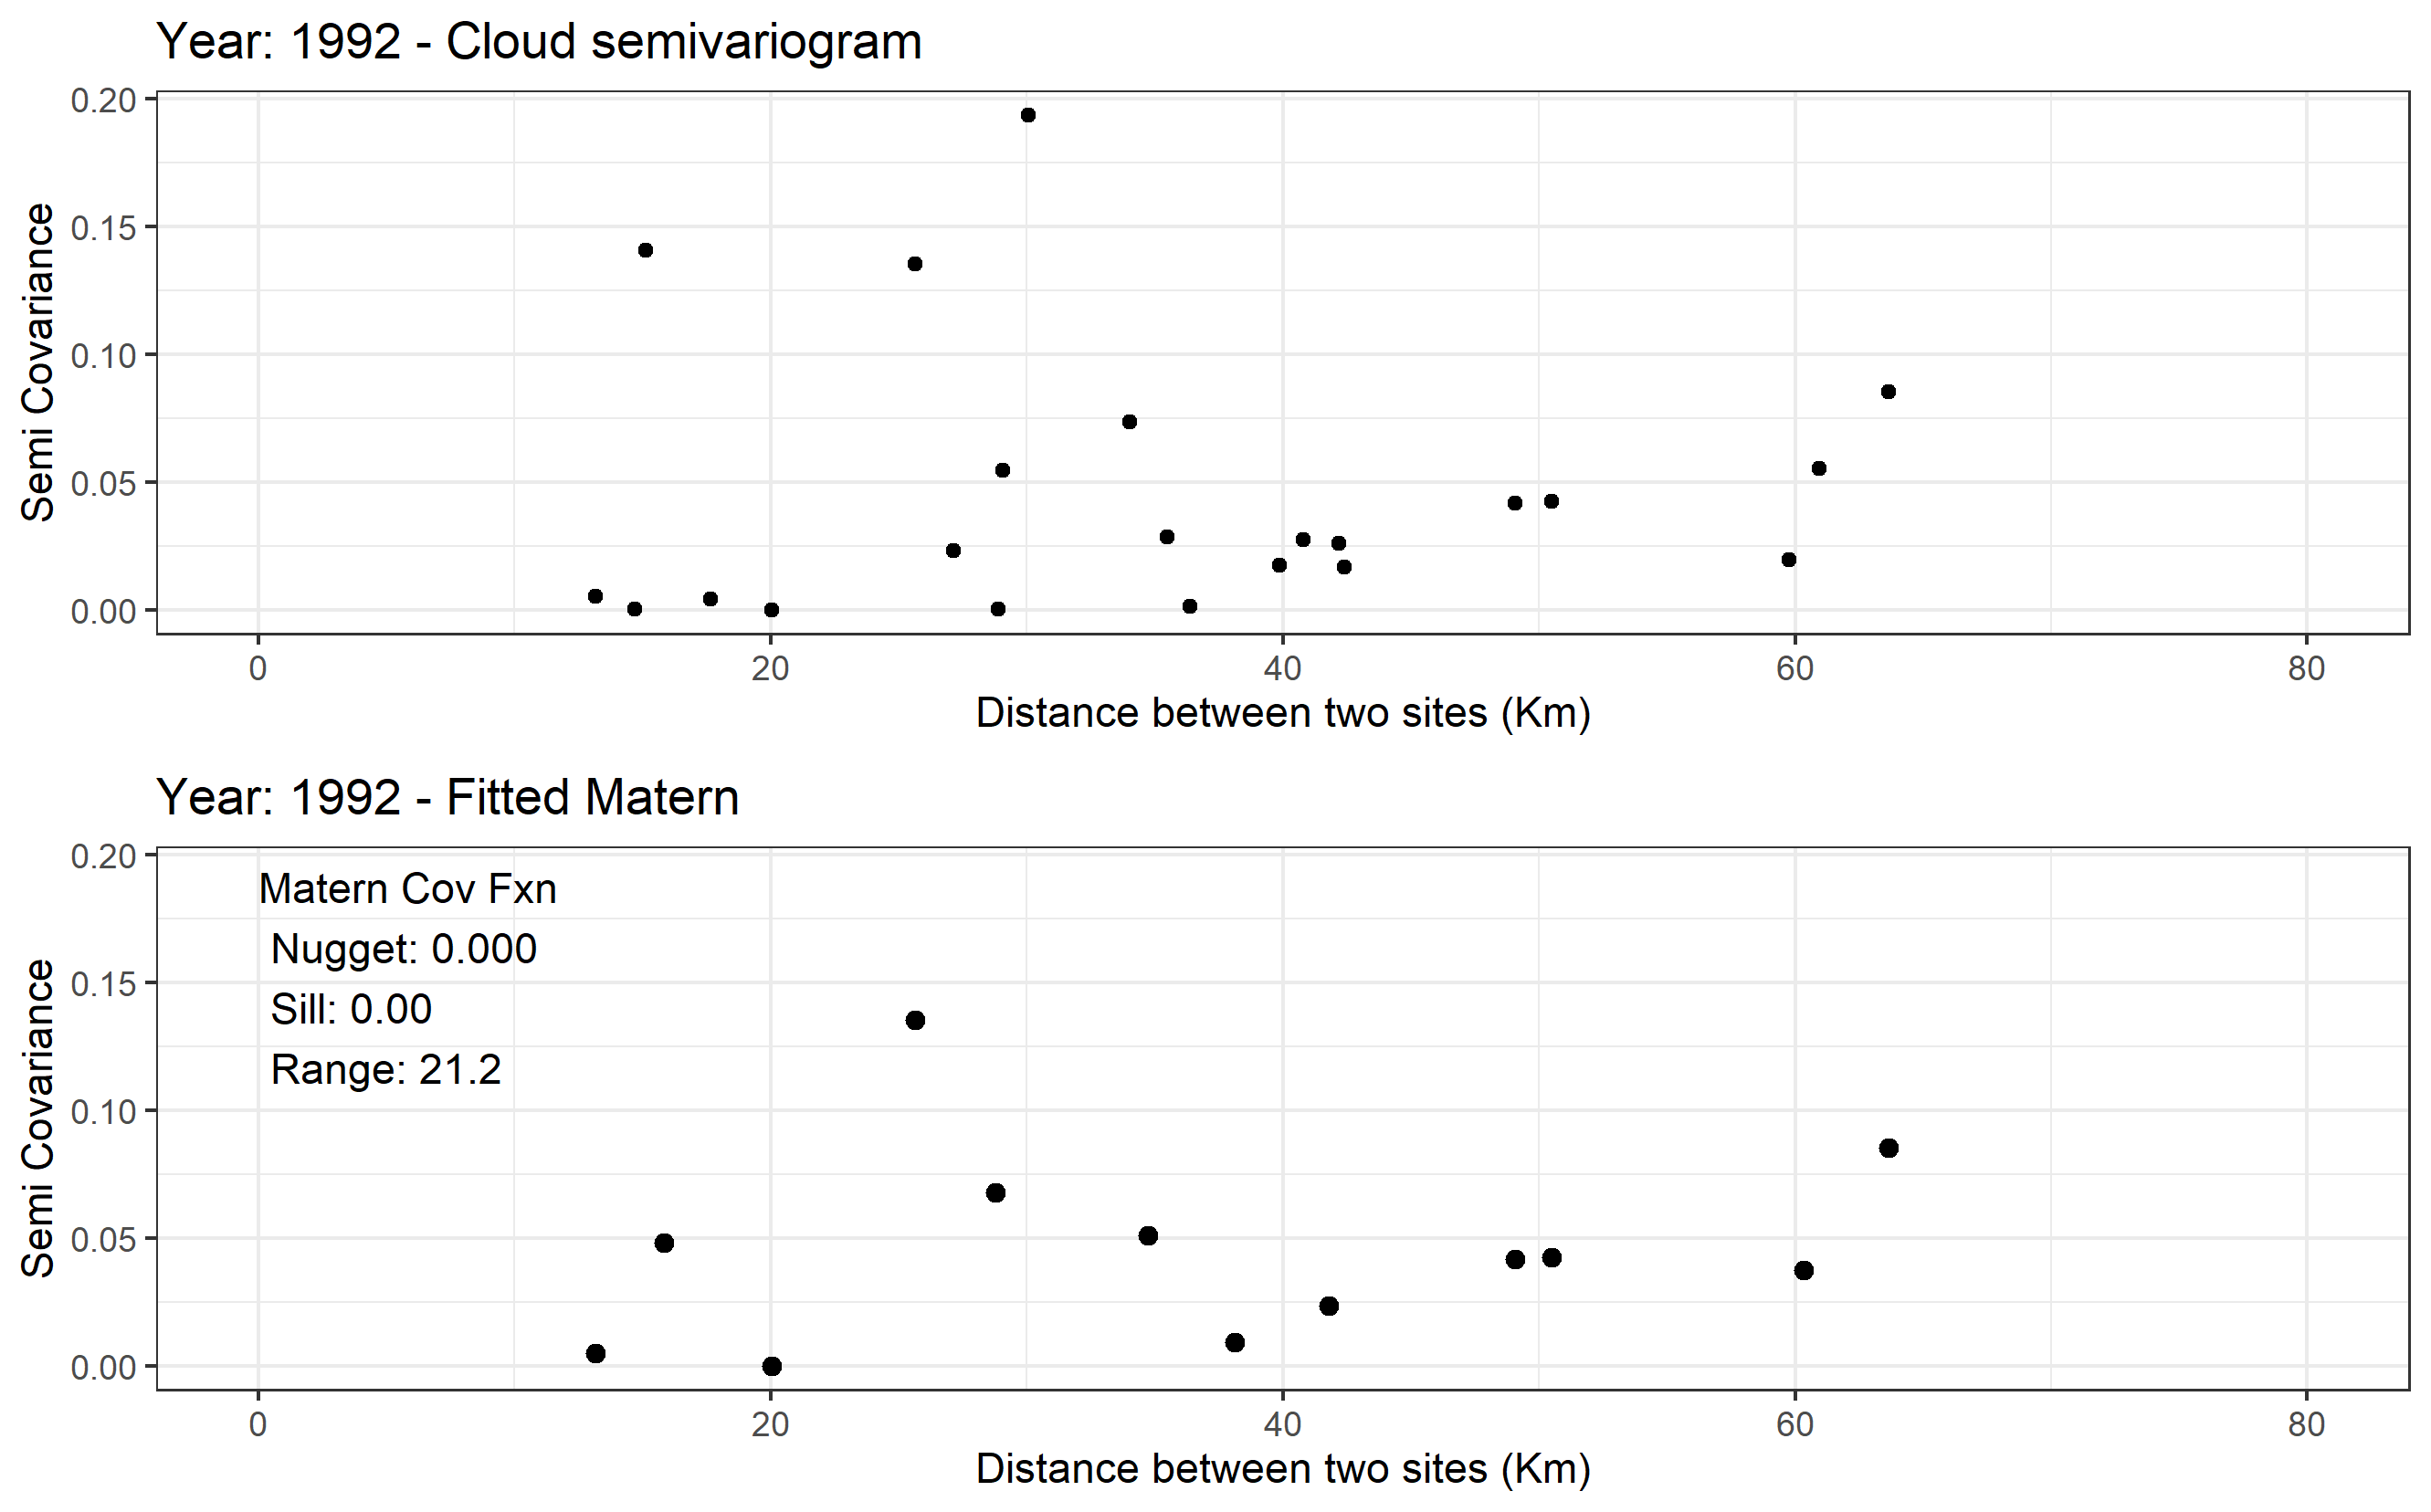}
    \caption{Caption}
    \label{fig:my_label}
\end{figure}

\begin{figure}
    \centering
    \includegraphics{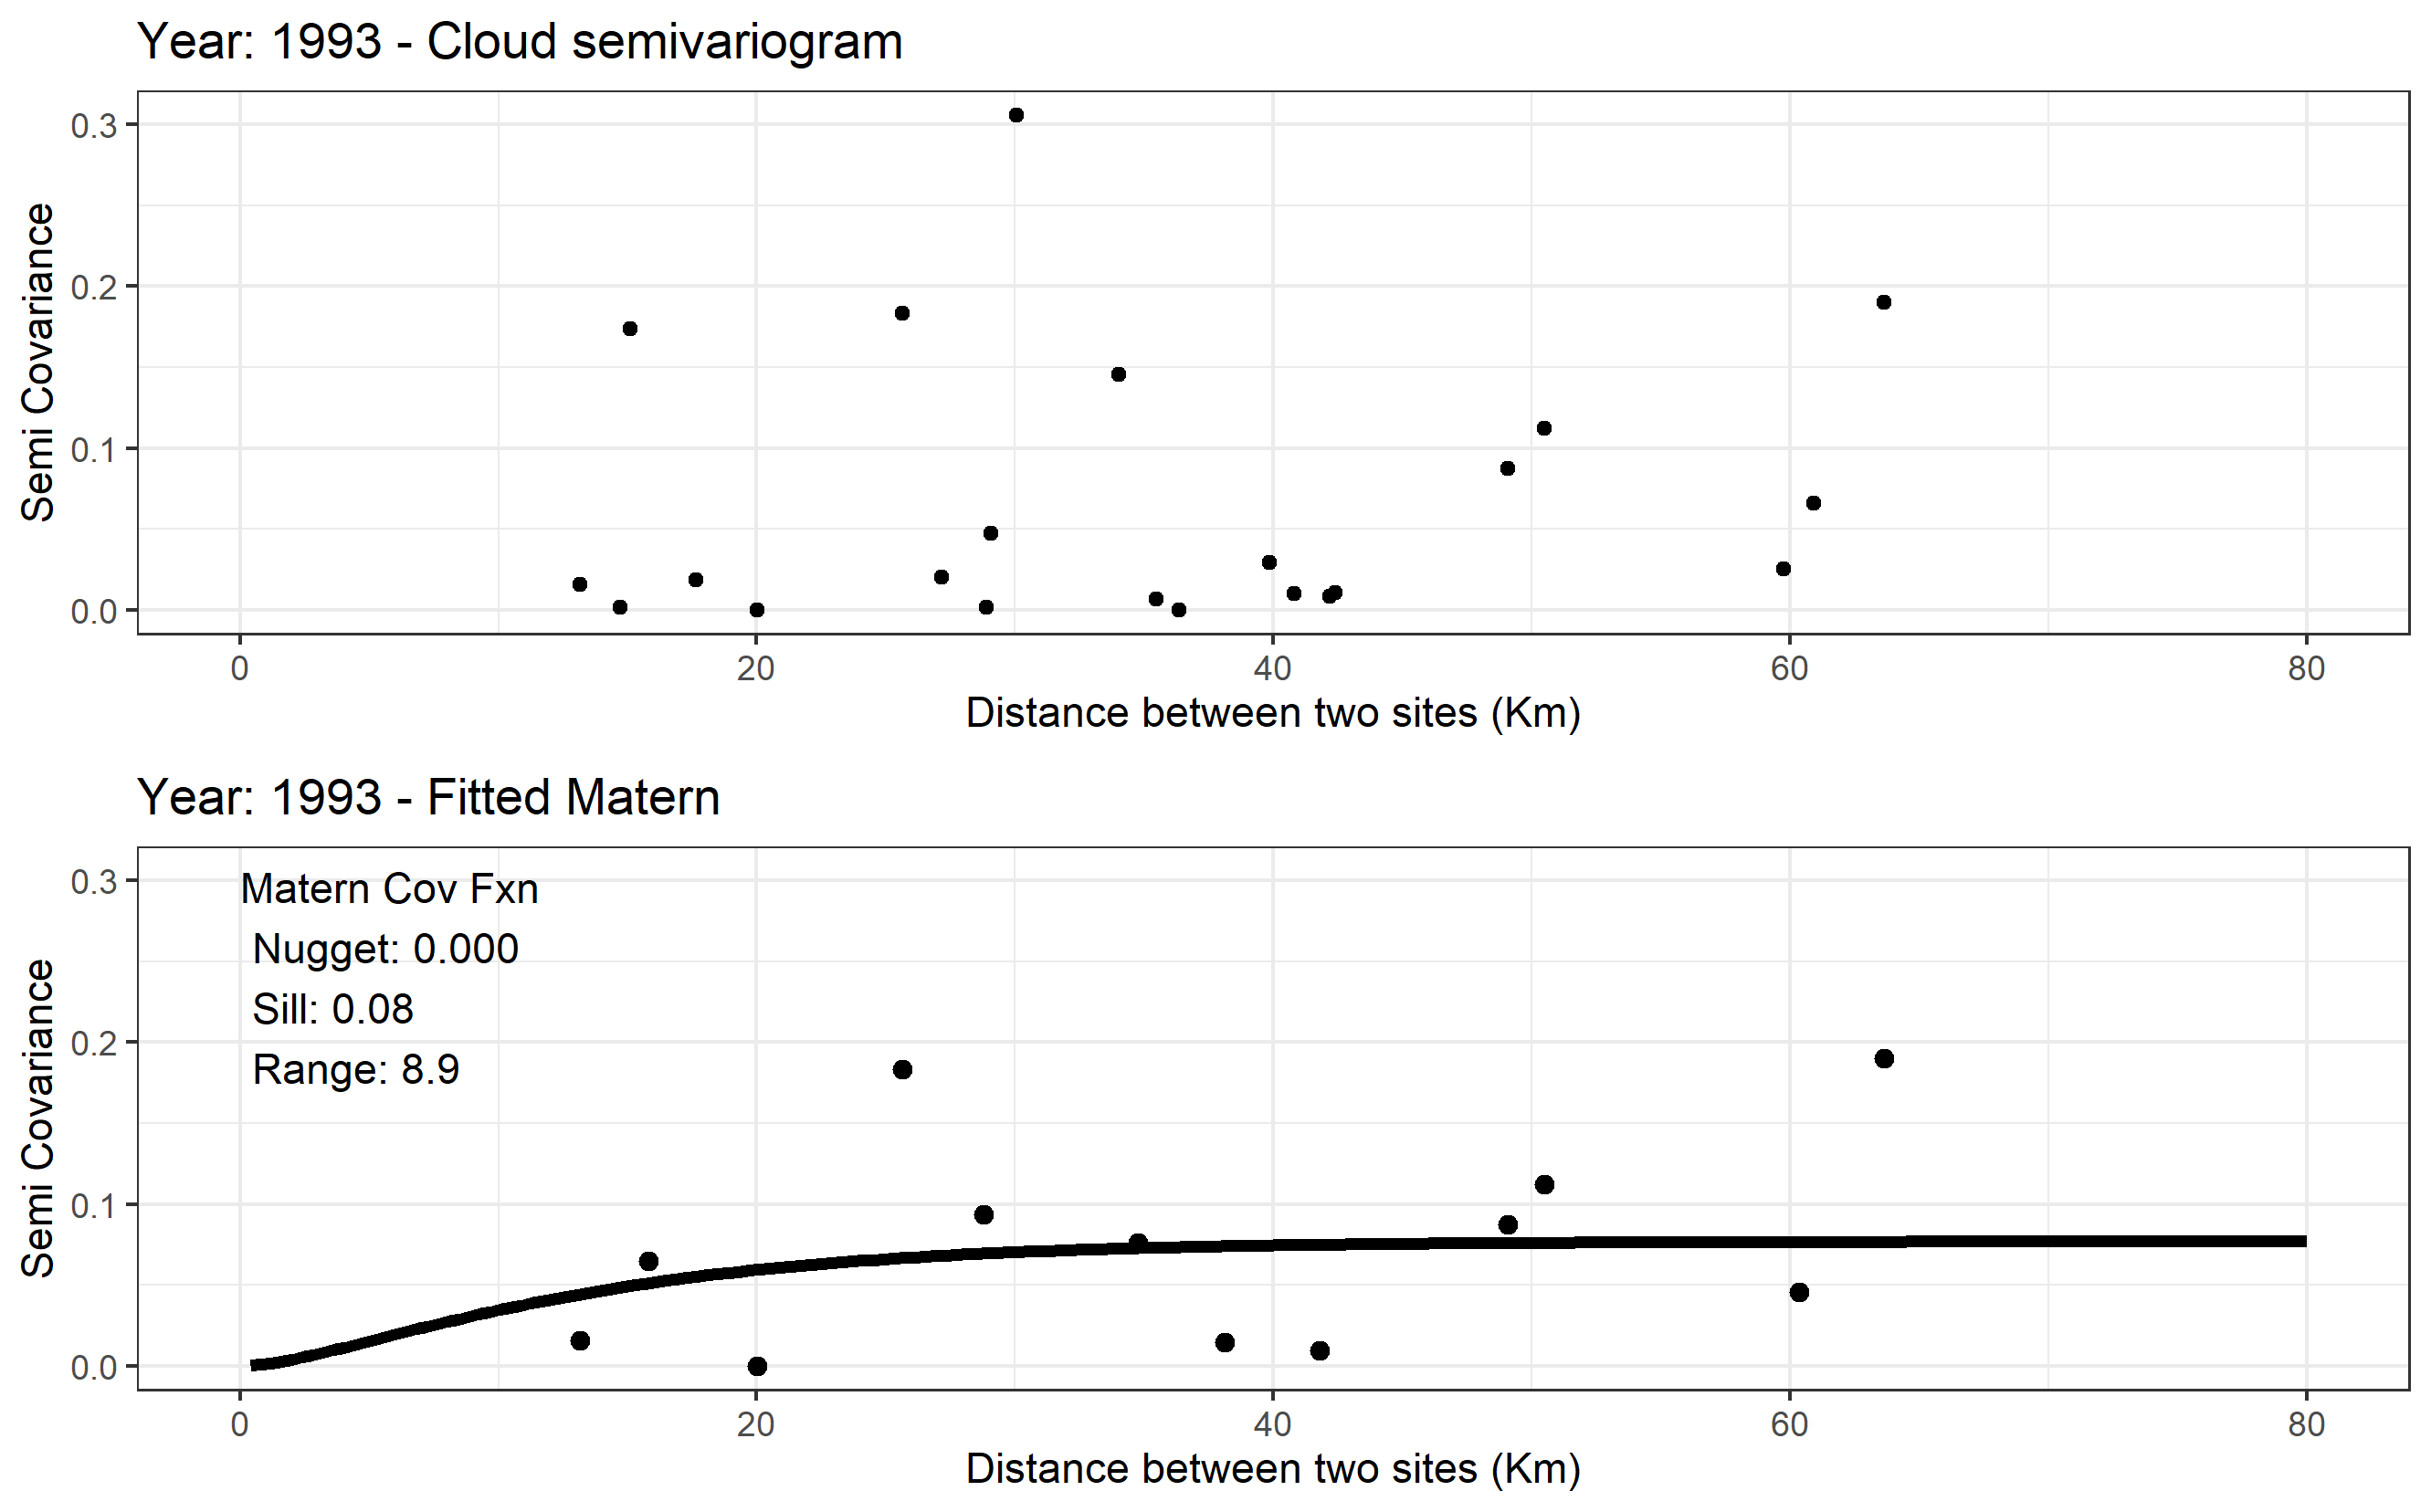}
    \caption{Caption}
    \label{fig:my_label}
\end{figure}

\begin{figure}
    \centering
    \includegraphics{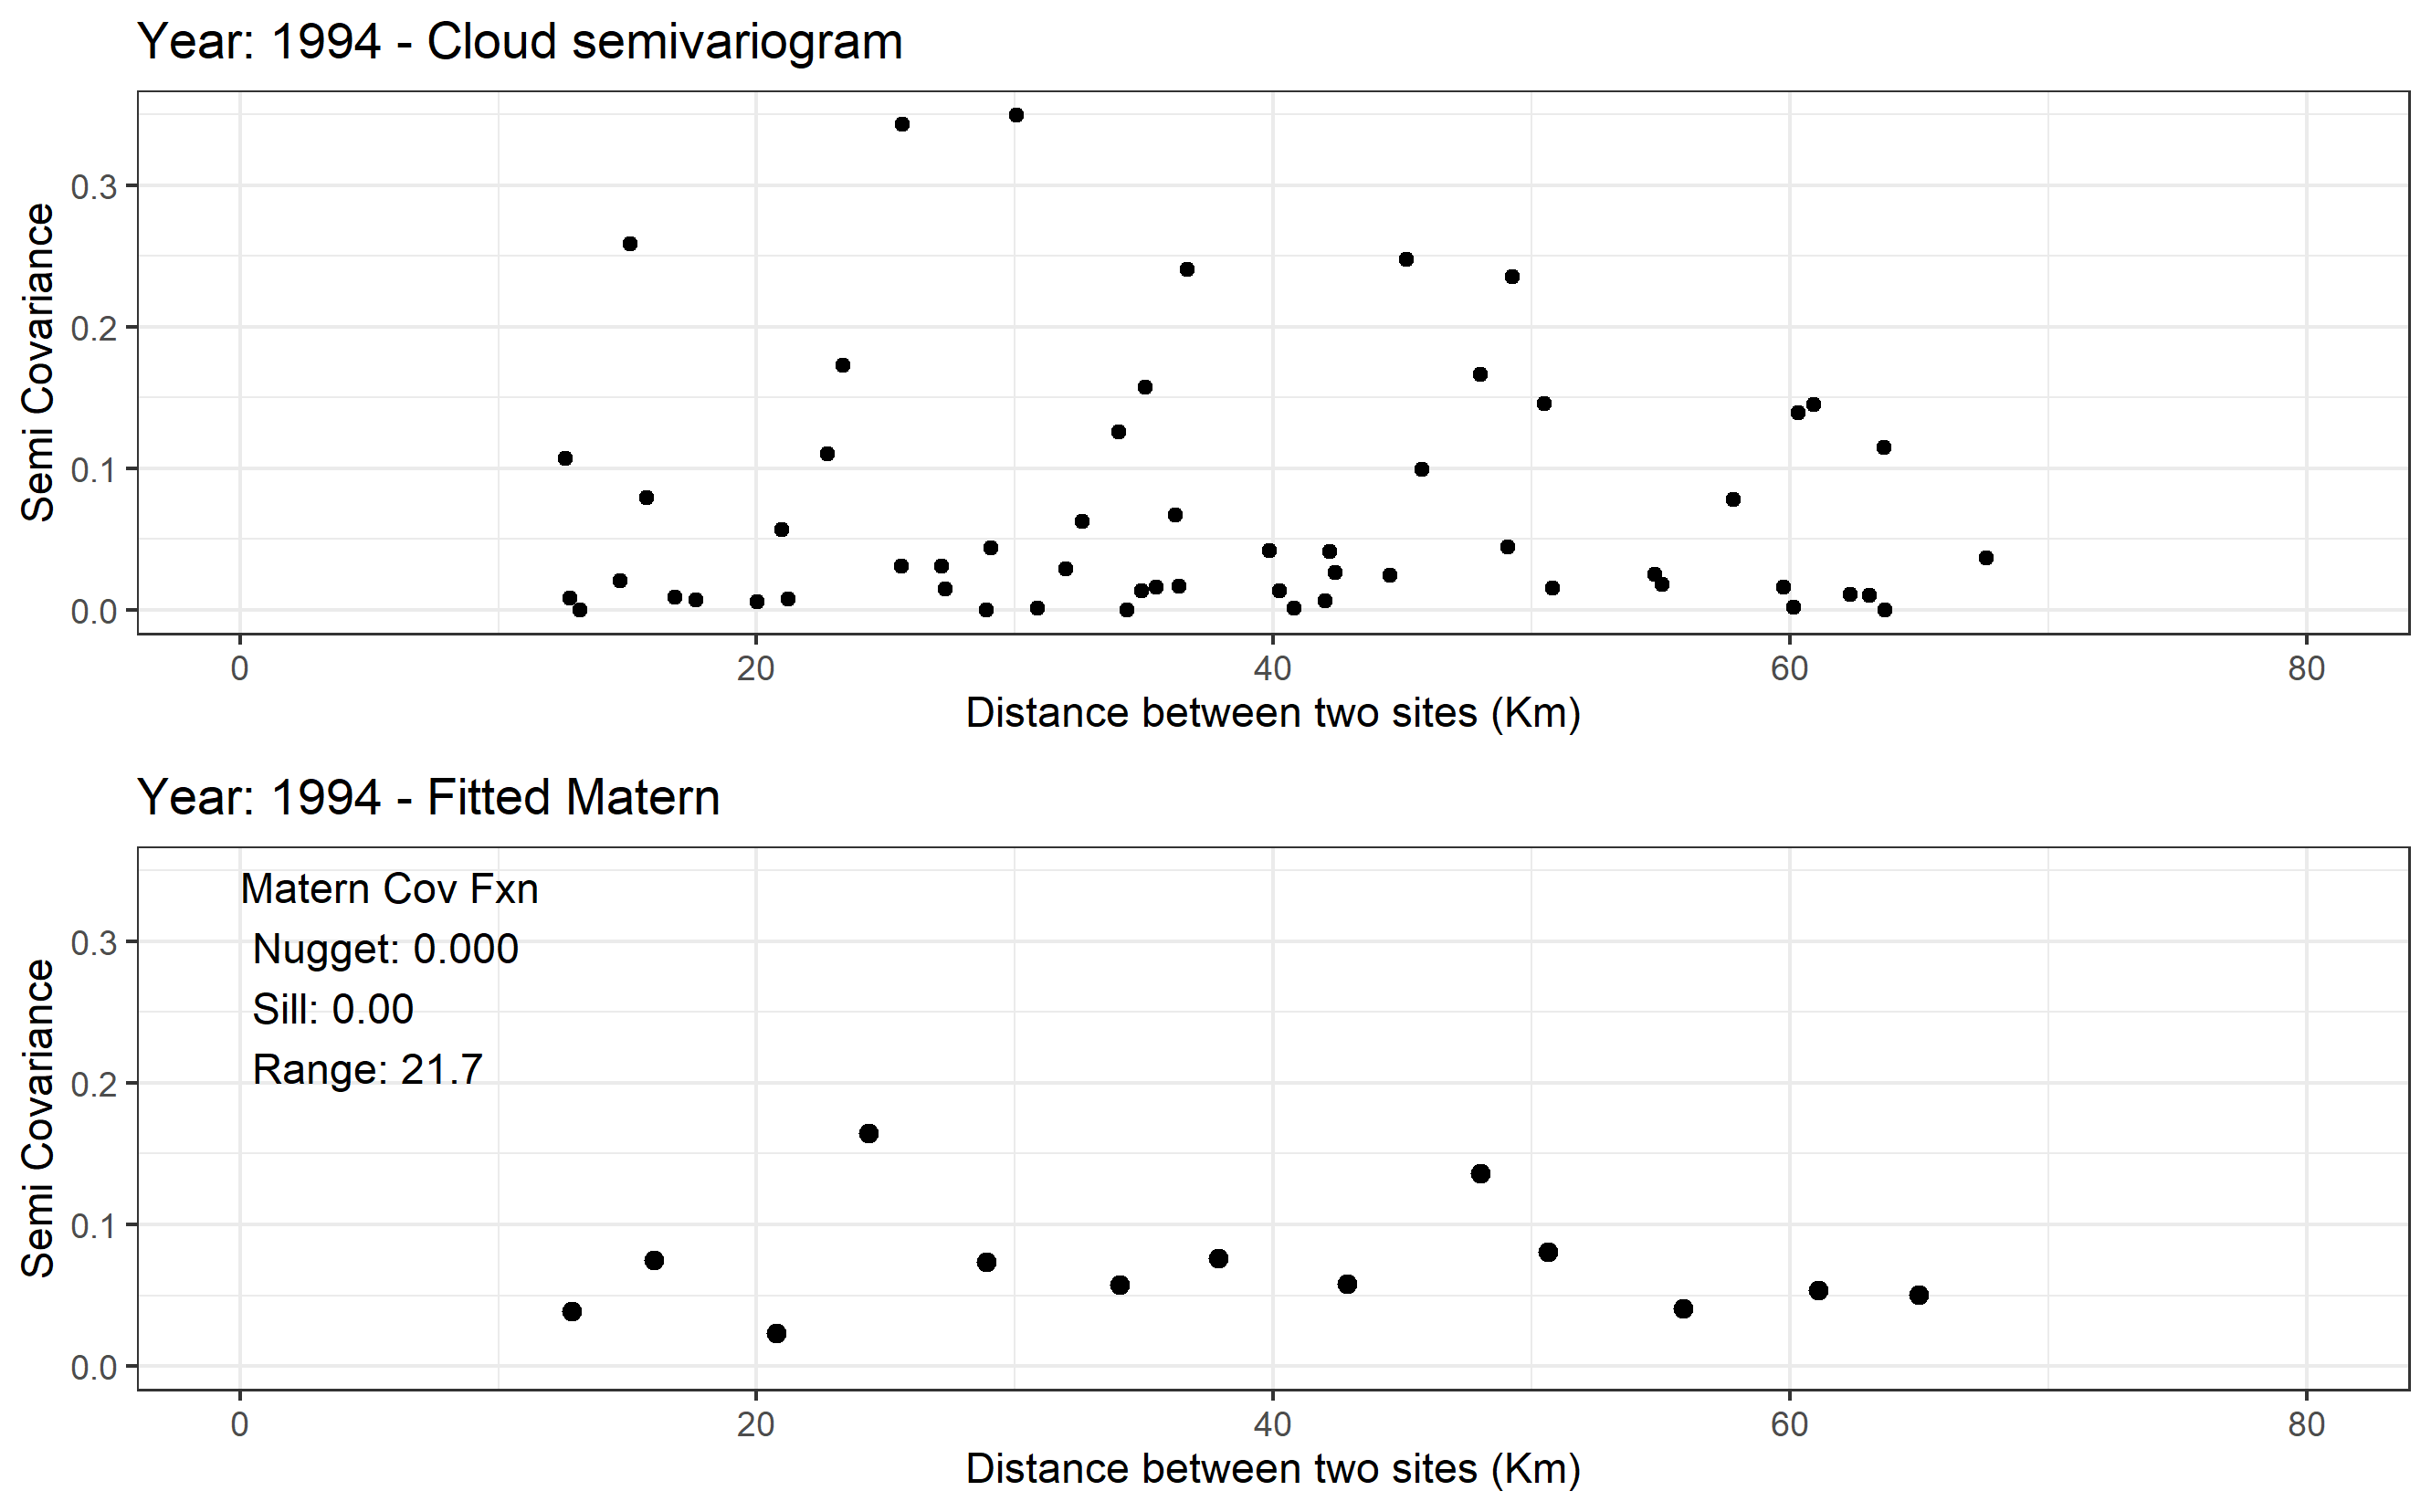}
    \caption{Caption}
    \label{fig:my_label}
\end{figure}

\begin{figure}
    \centering
    \includegraphics{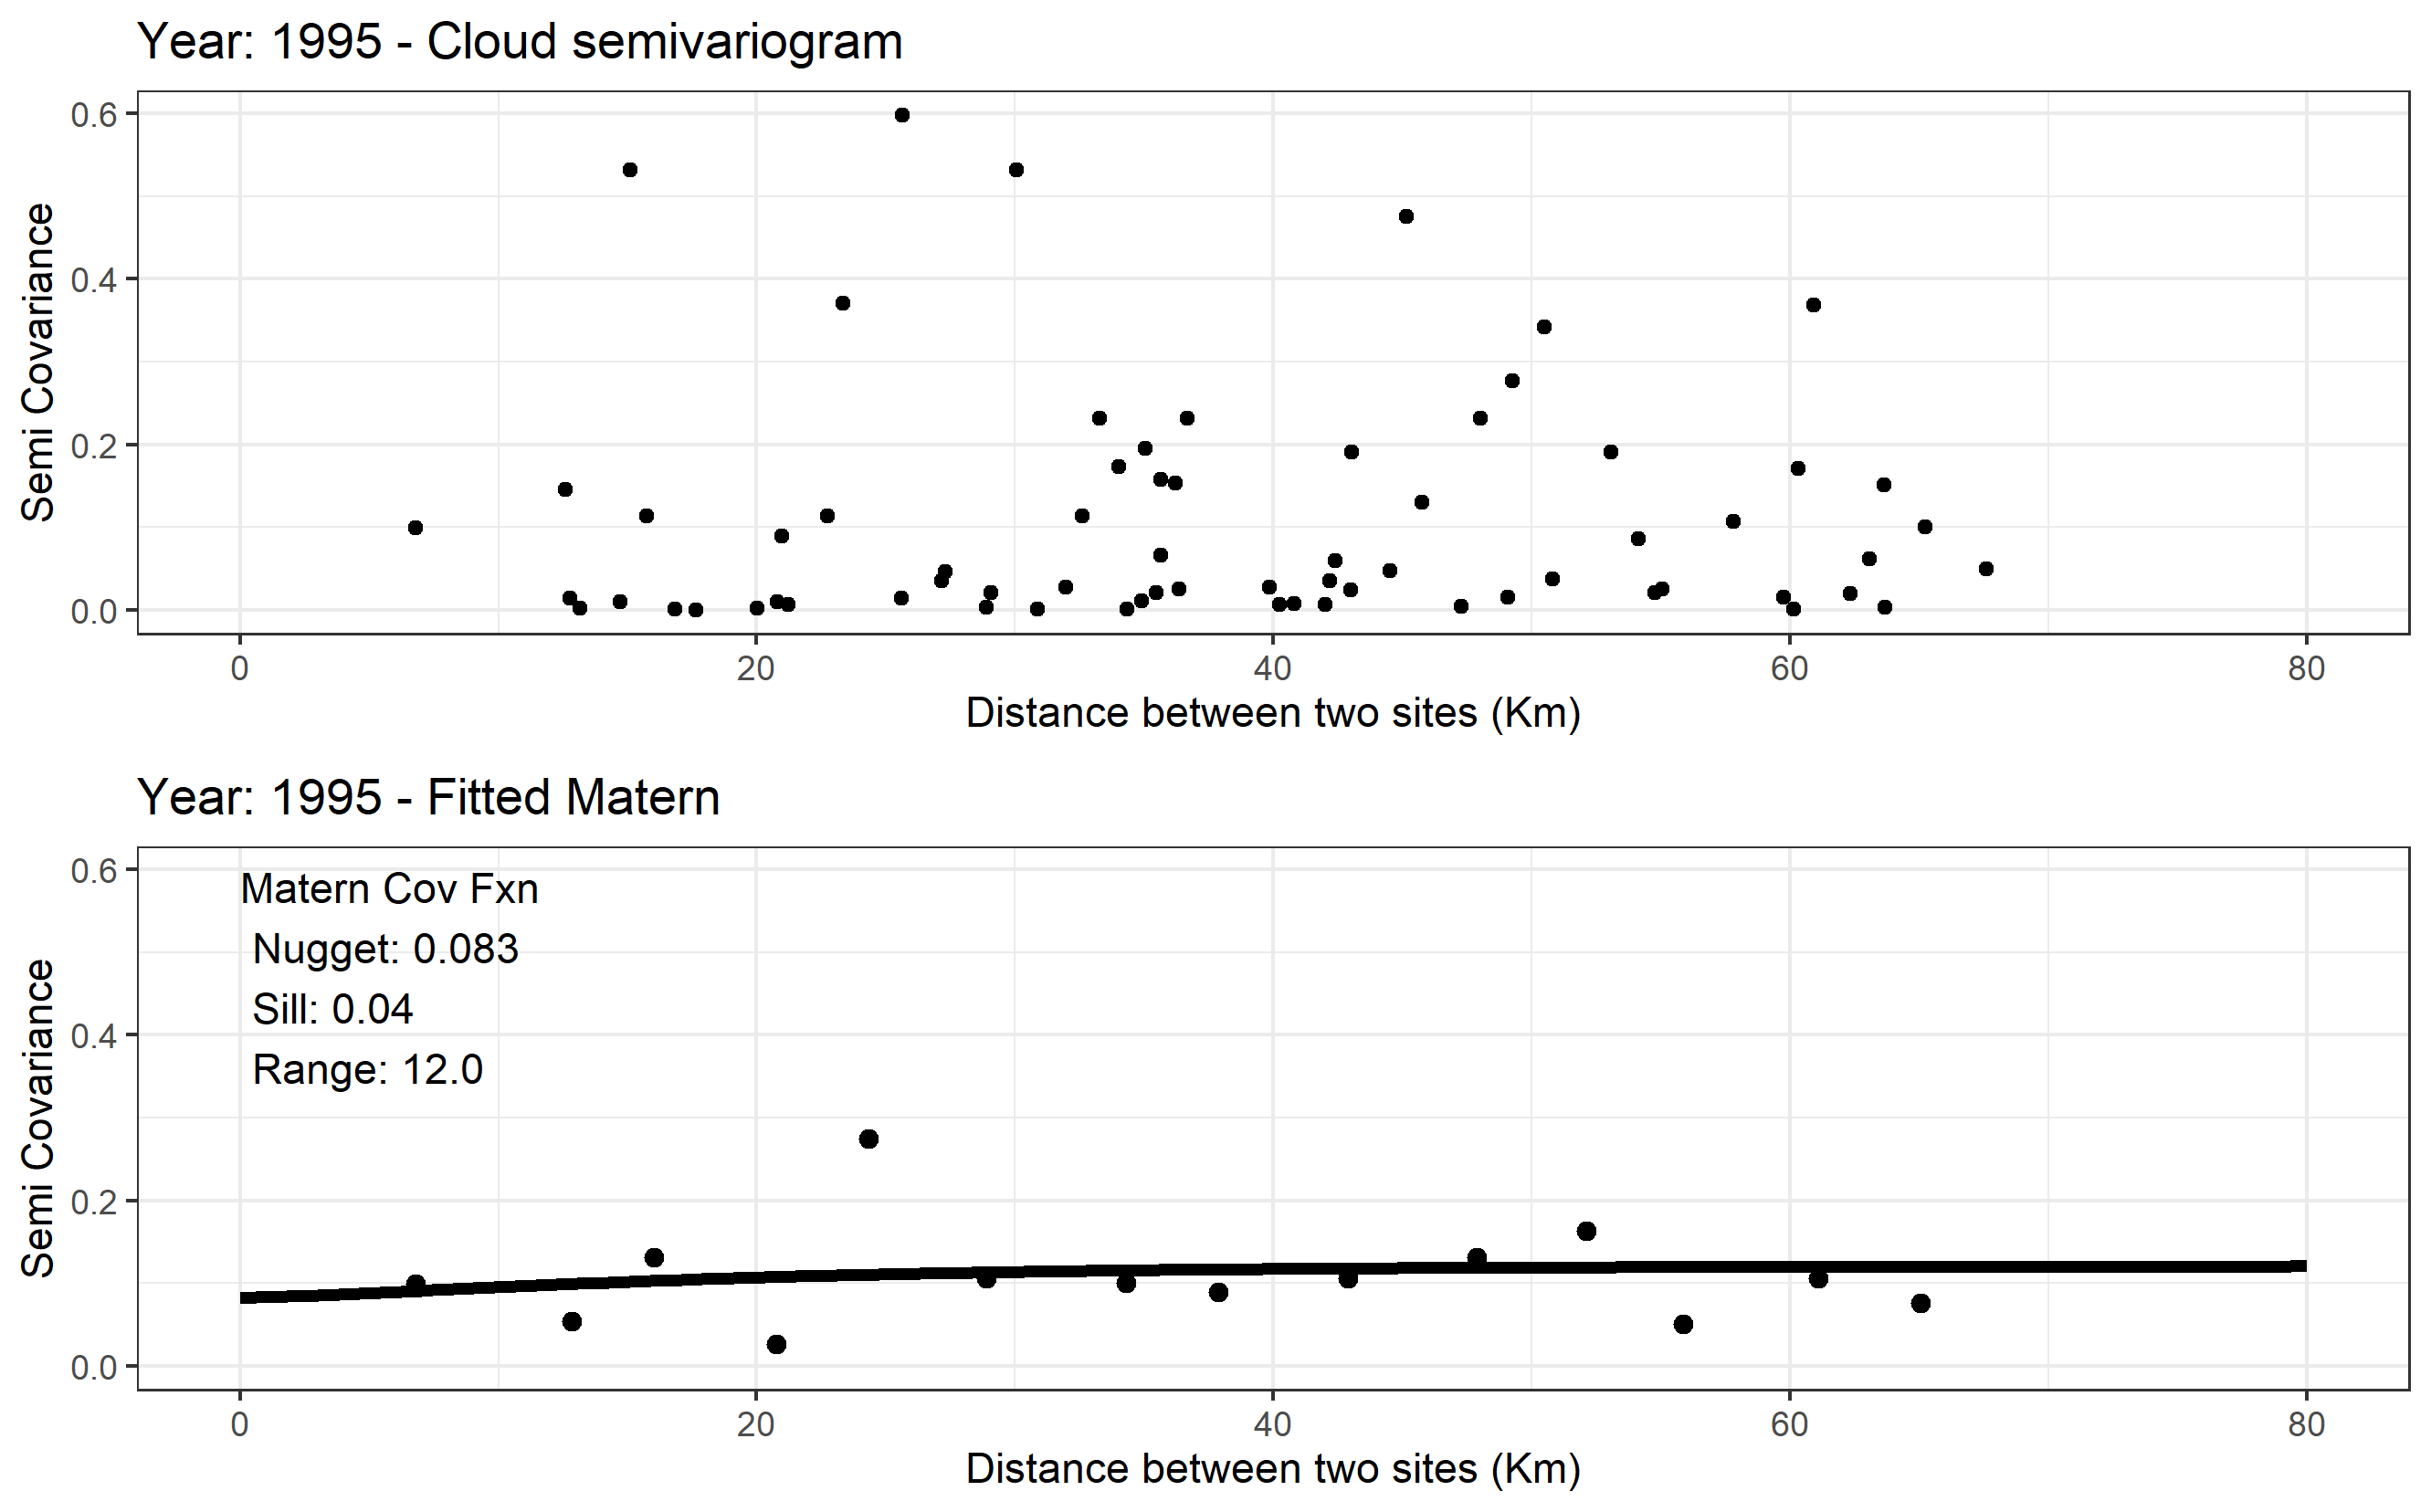}
    \caption{Caption}
    \label{fig:my_label}
\end{figure}

\begin{figure}
    \centering
    \includegraphics{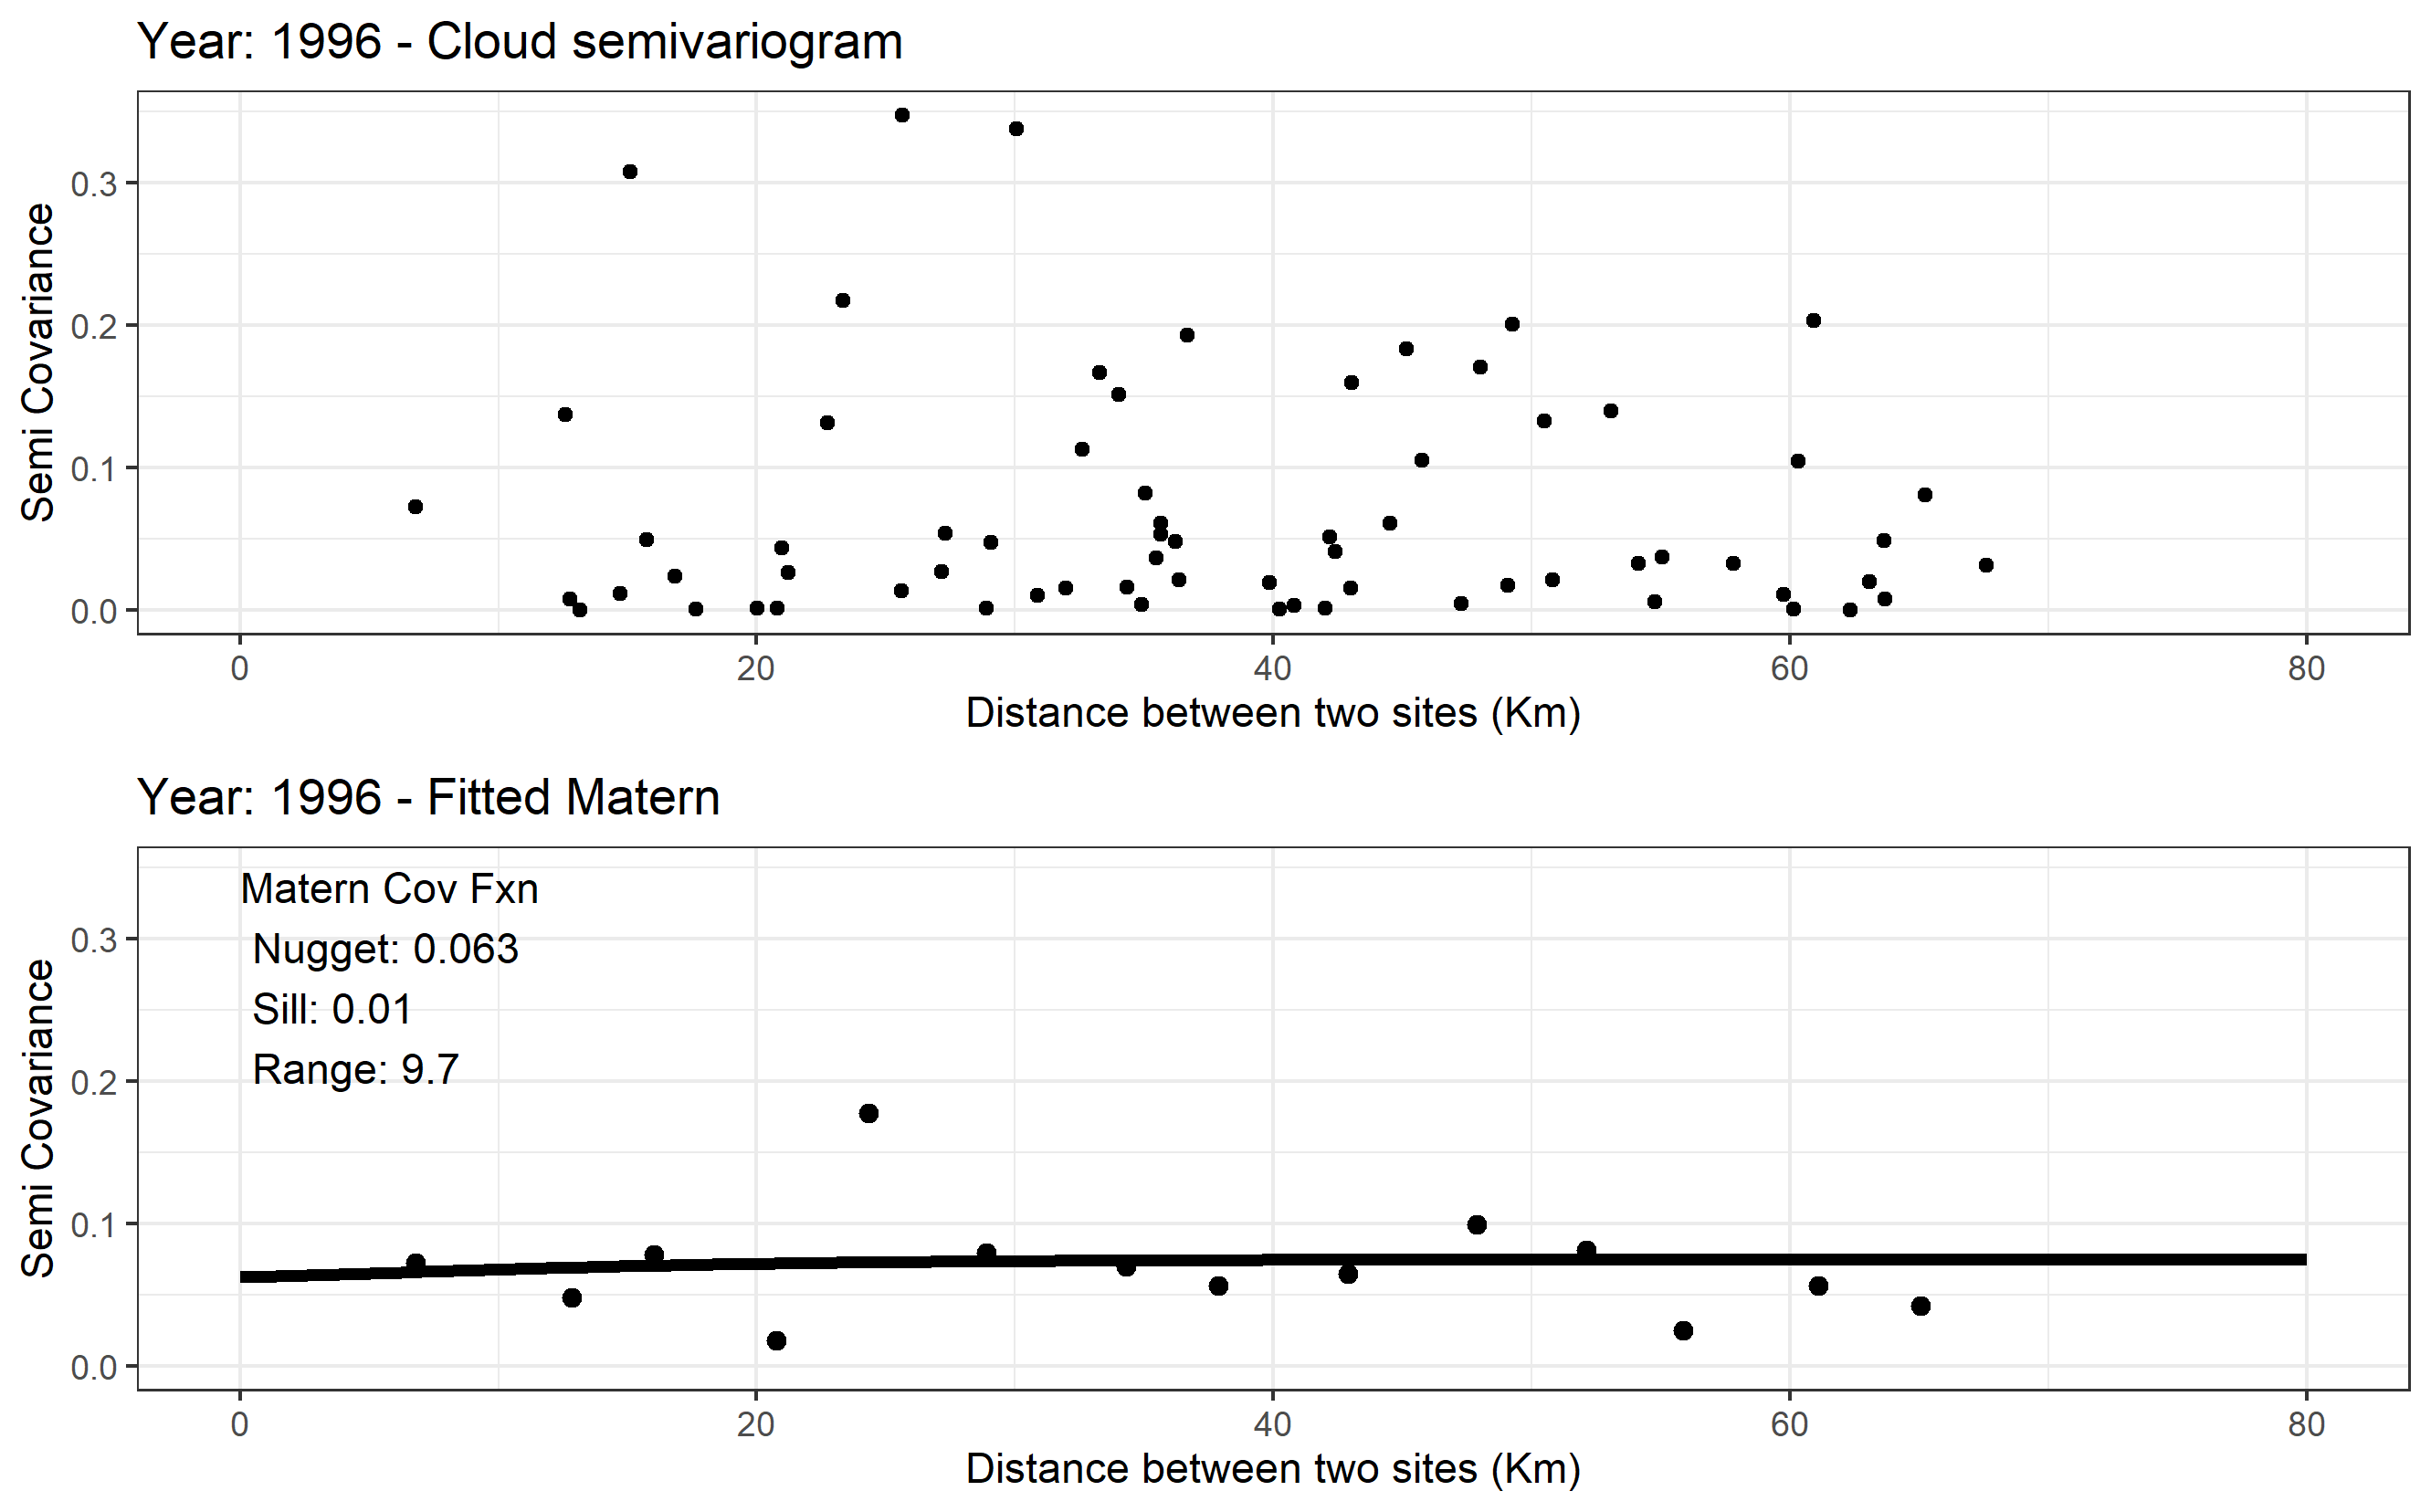}
    \caption{Caption}
    \label{fig:my_label}
\end{figure}

\begin{figure}
    \centering
    \includegraphics{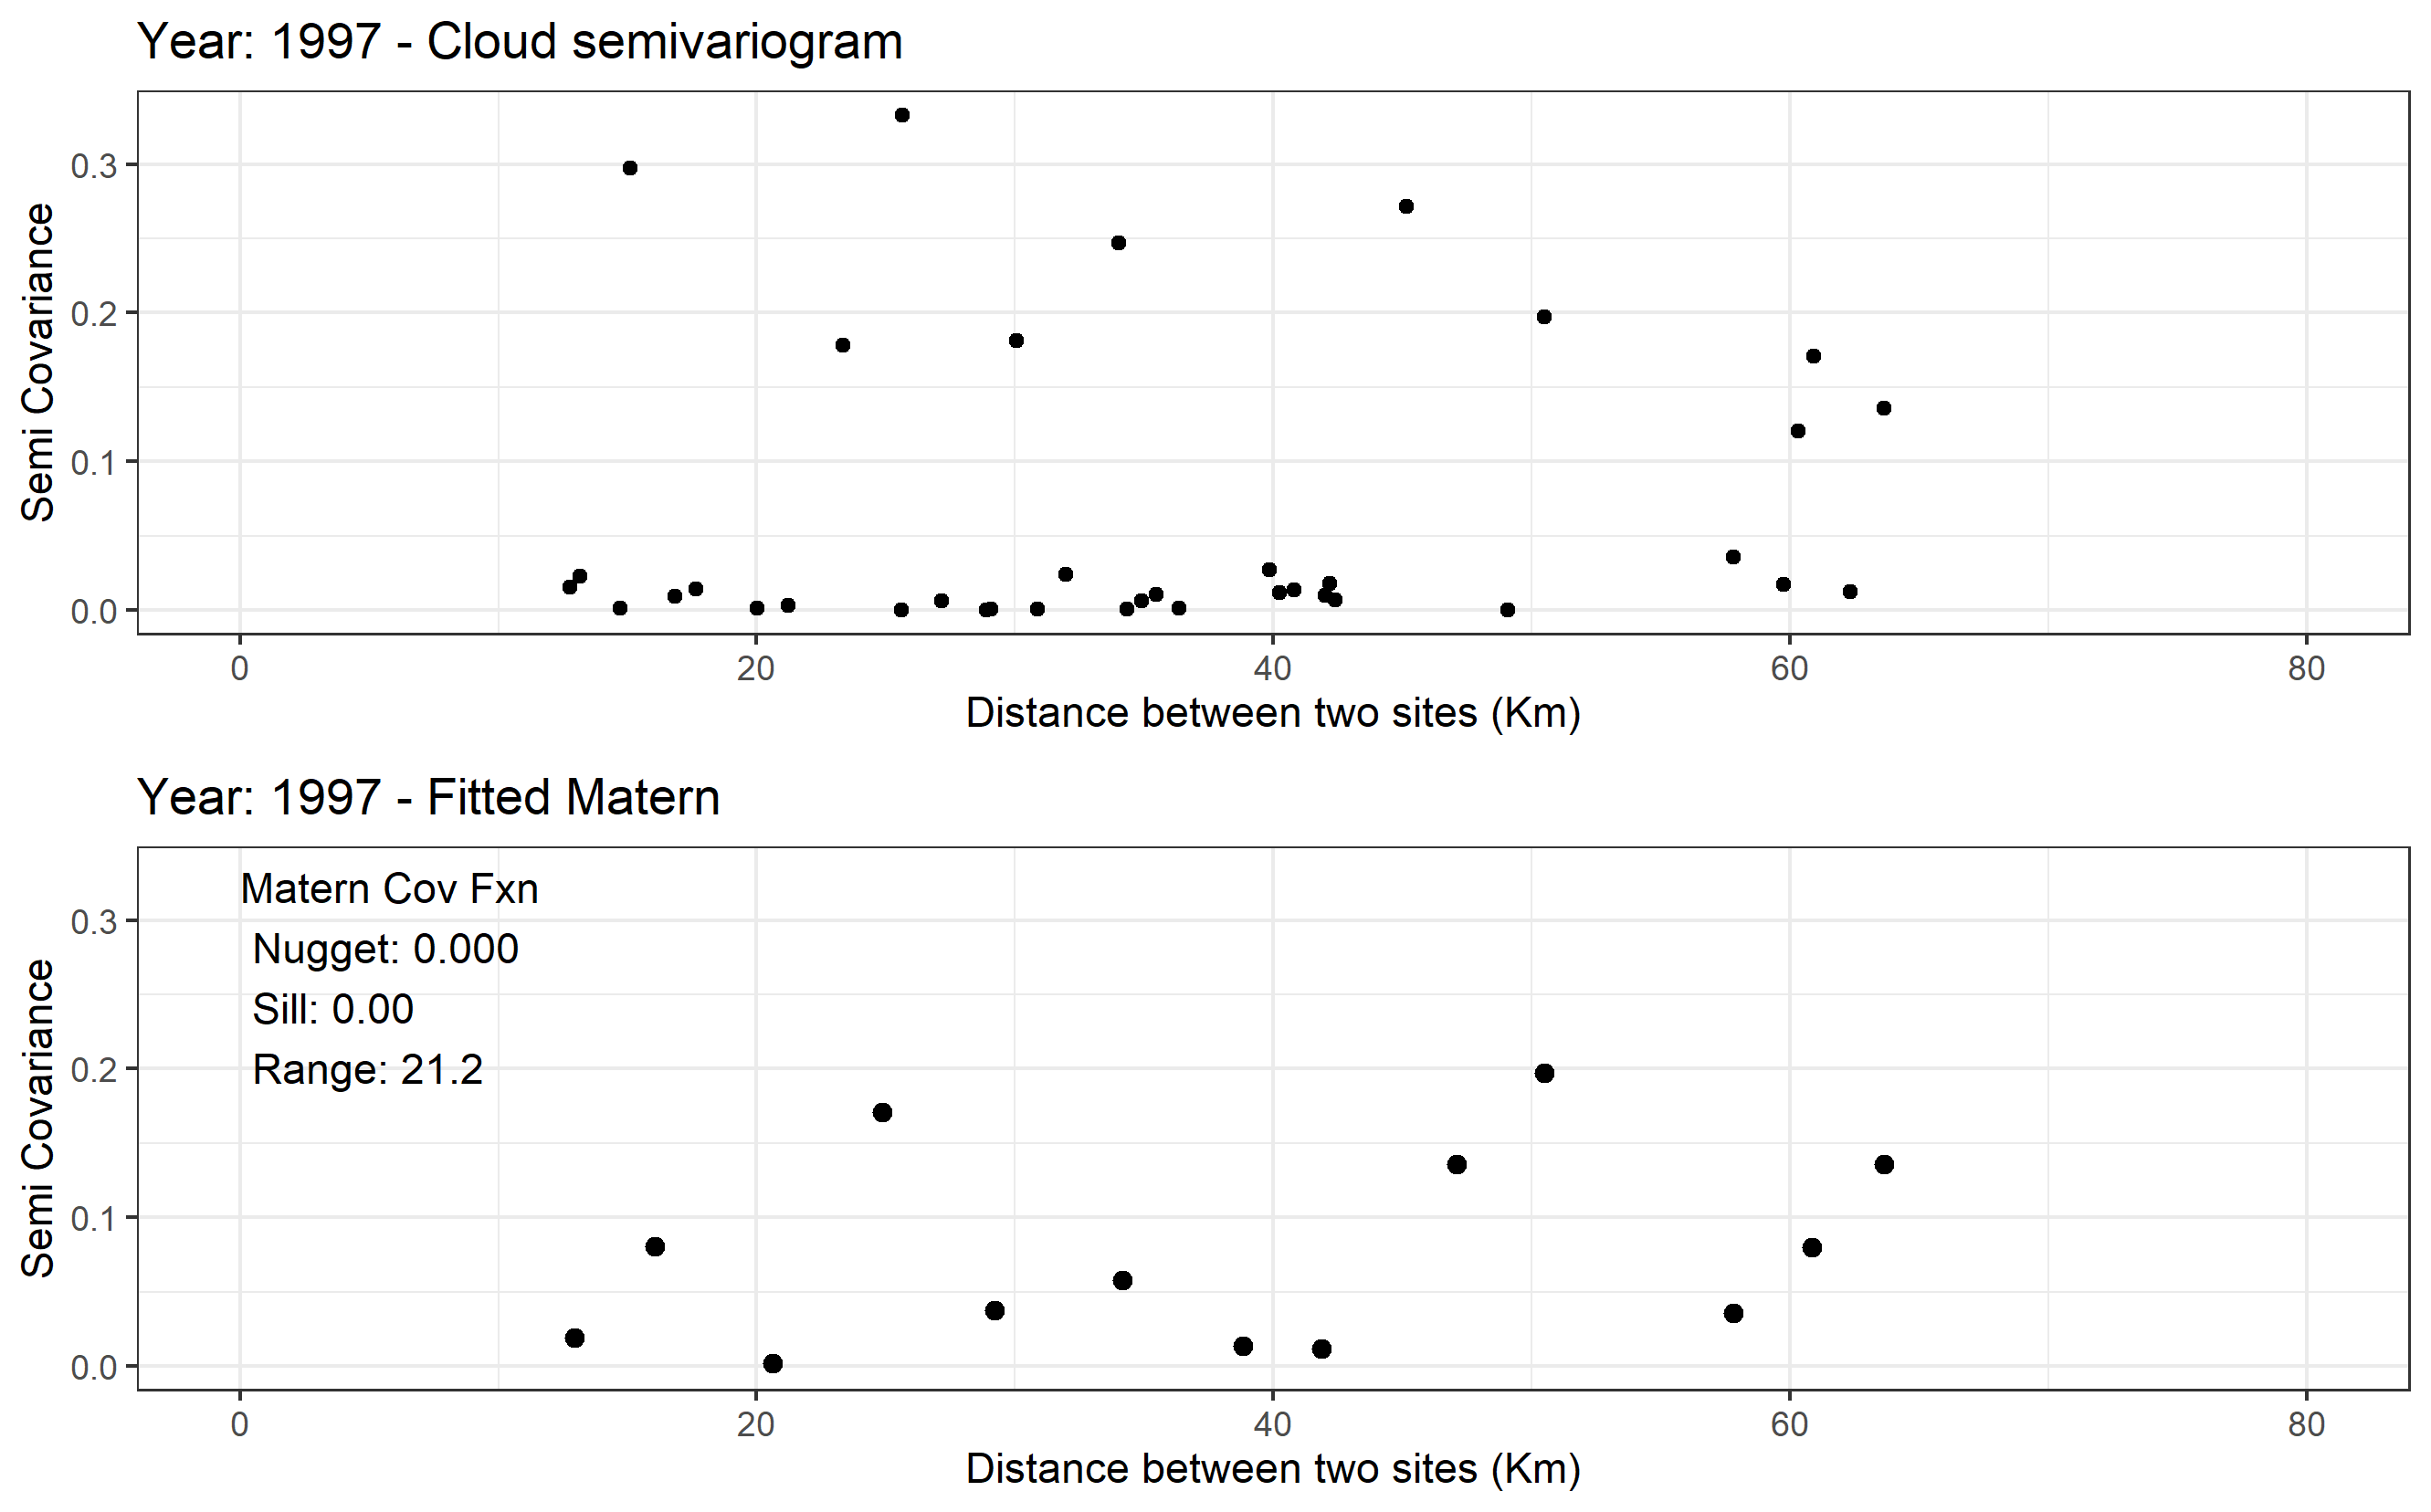}
    \caption{Caption}
    \label{fig:my_label}
\end{figure}

\begin{figure}
    \centering
    \includegraphics{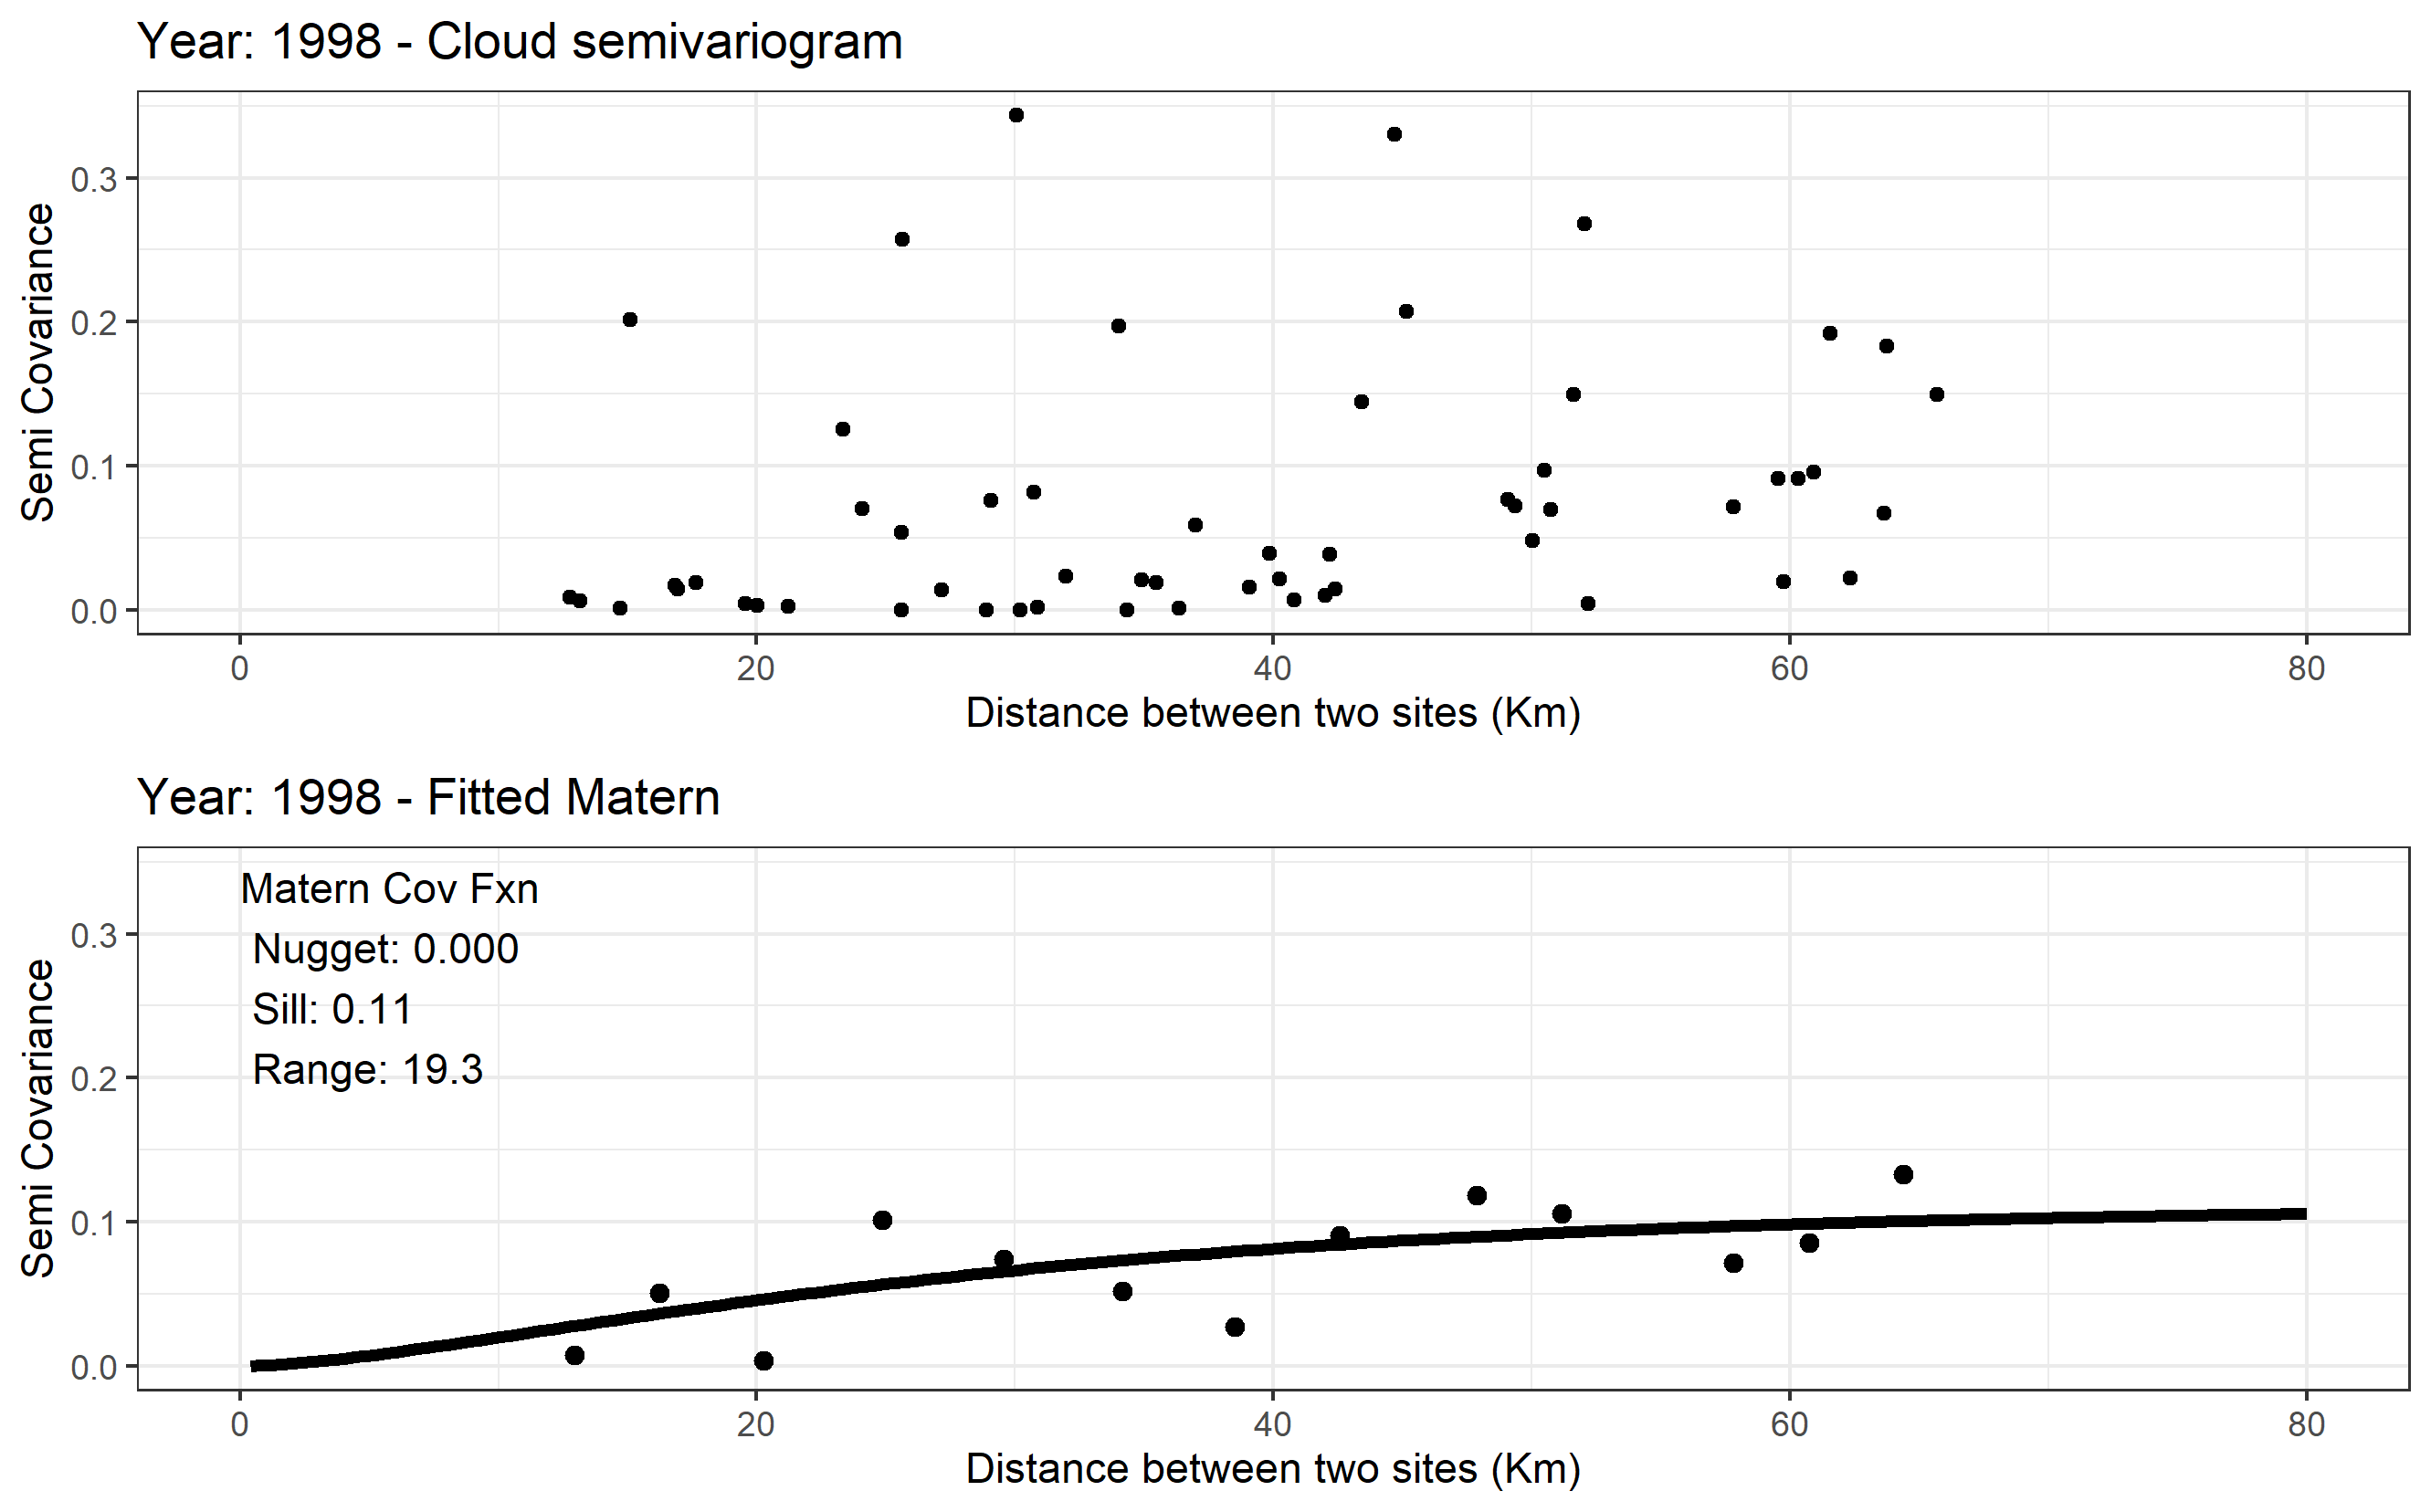}
    \caption{Caption}
    \label{fig:my_label}
\end{figure}

\begin{figure}
    \centering
    \includegraphics{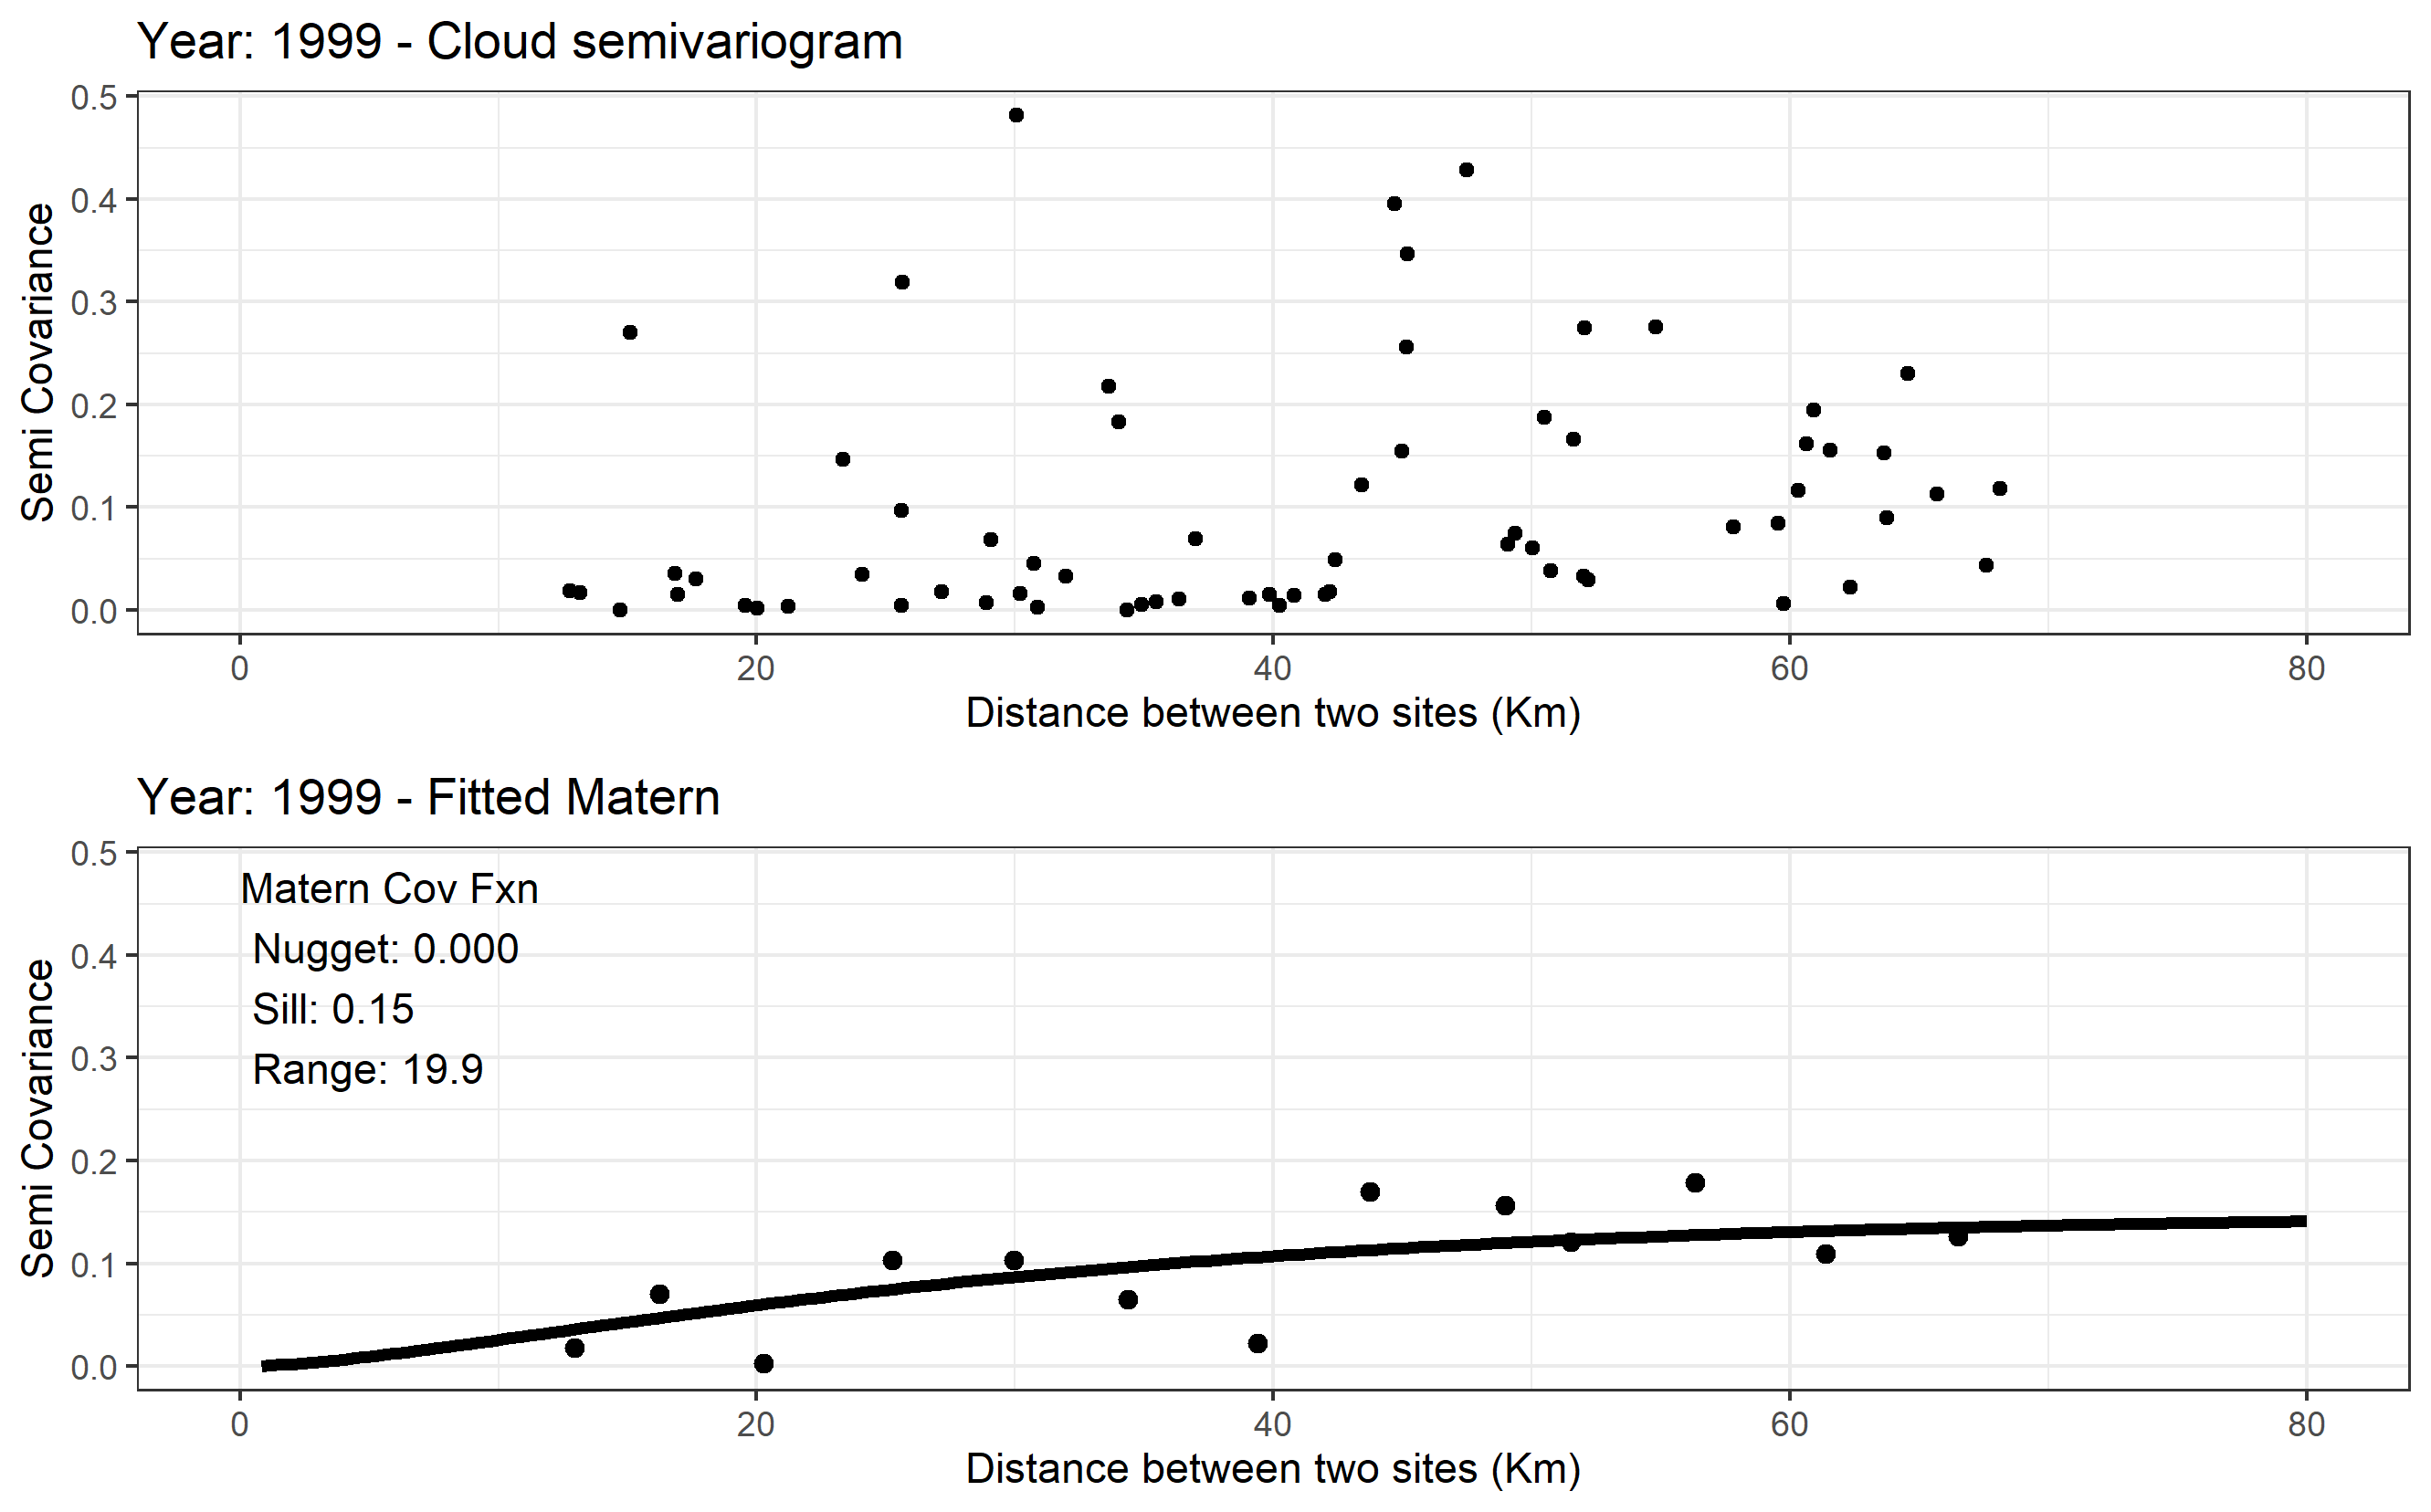}
    \caption{Caption}
    \label{fig:my_label}
\end{figure}

\begin{figure}
    \centering
    \includegraphics{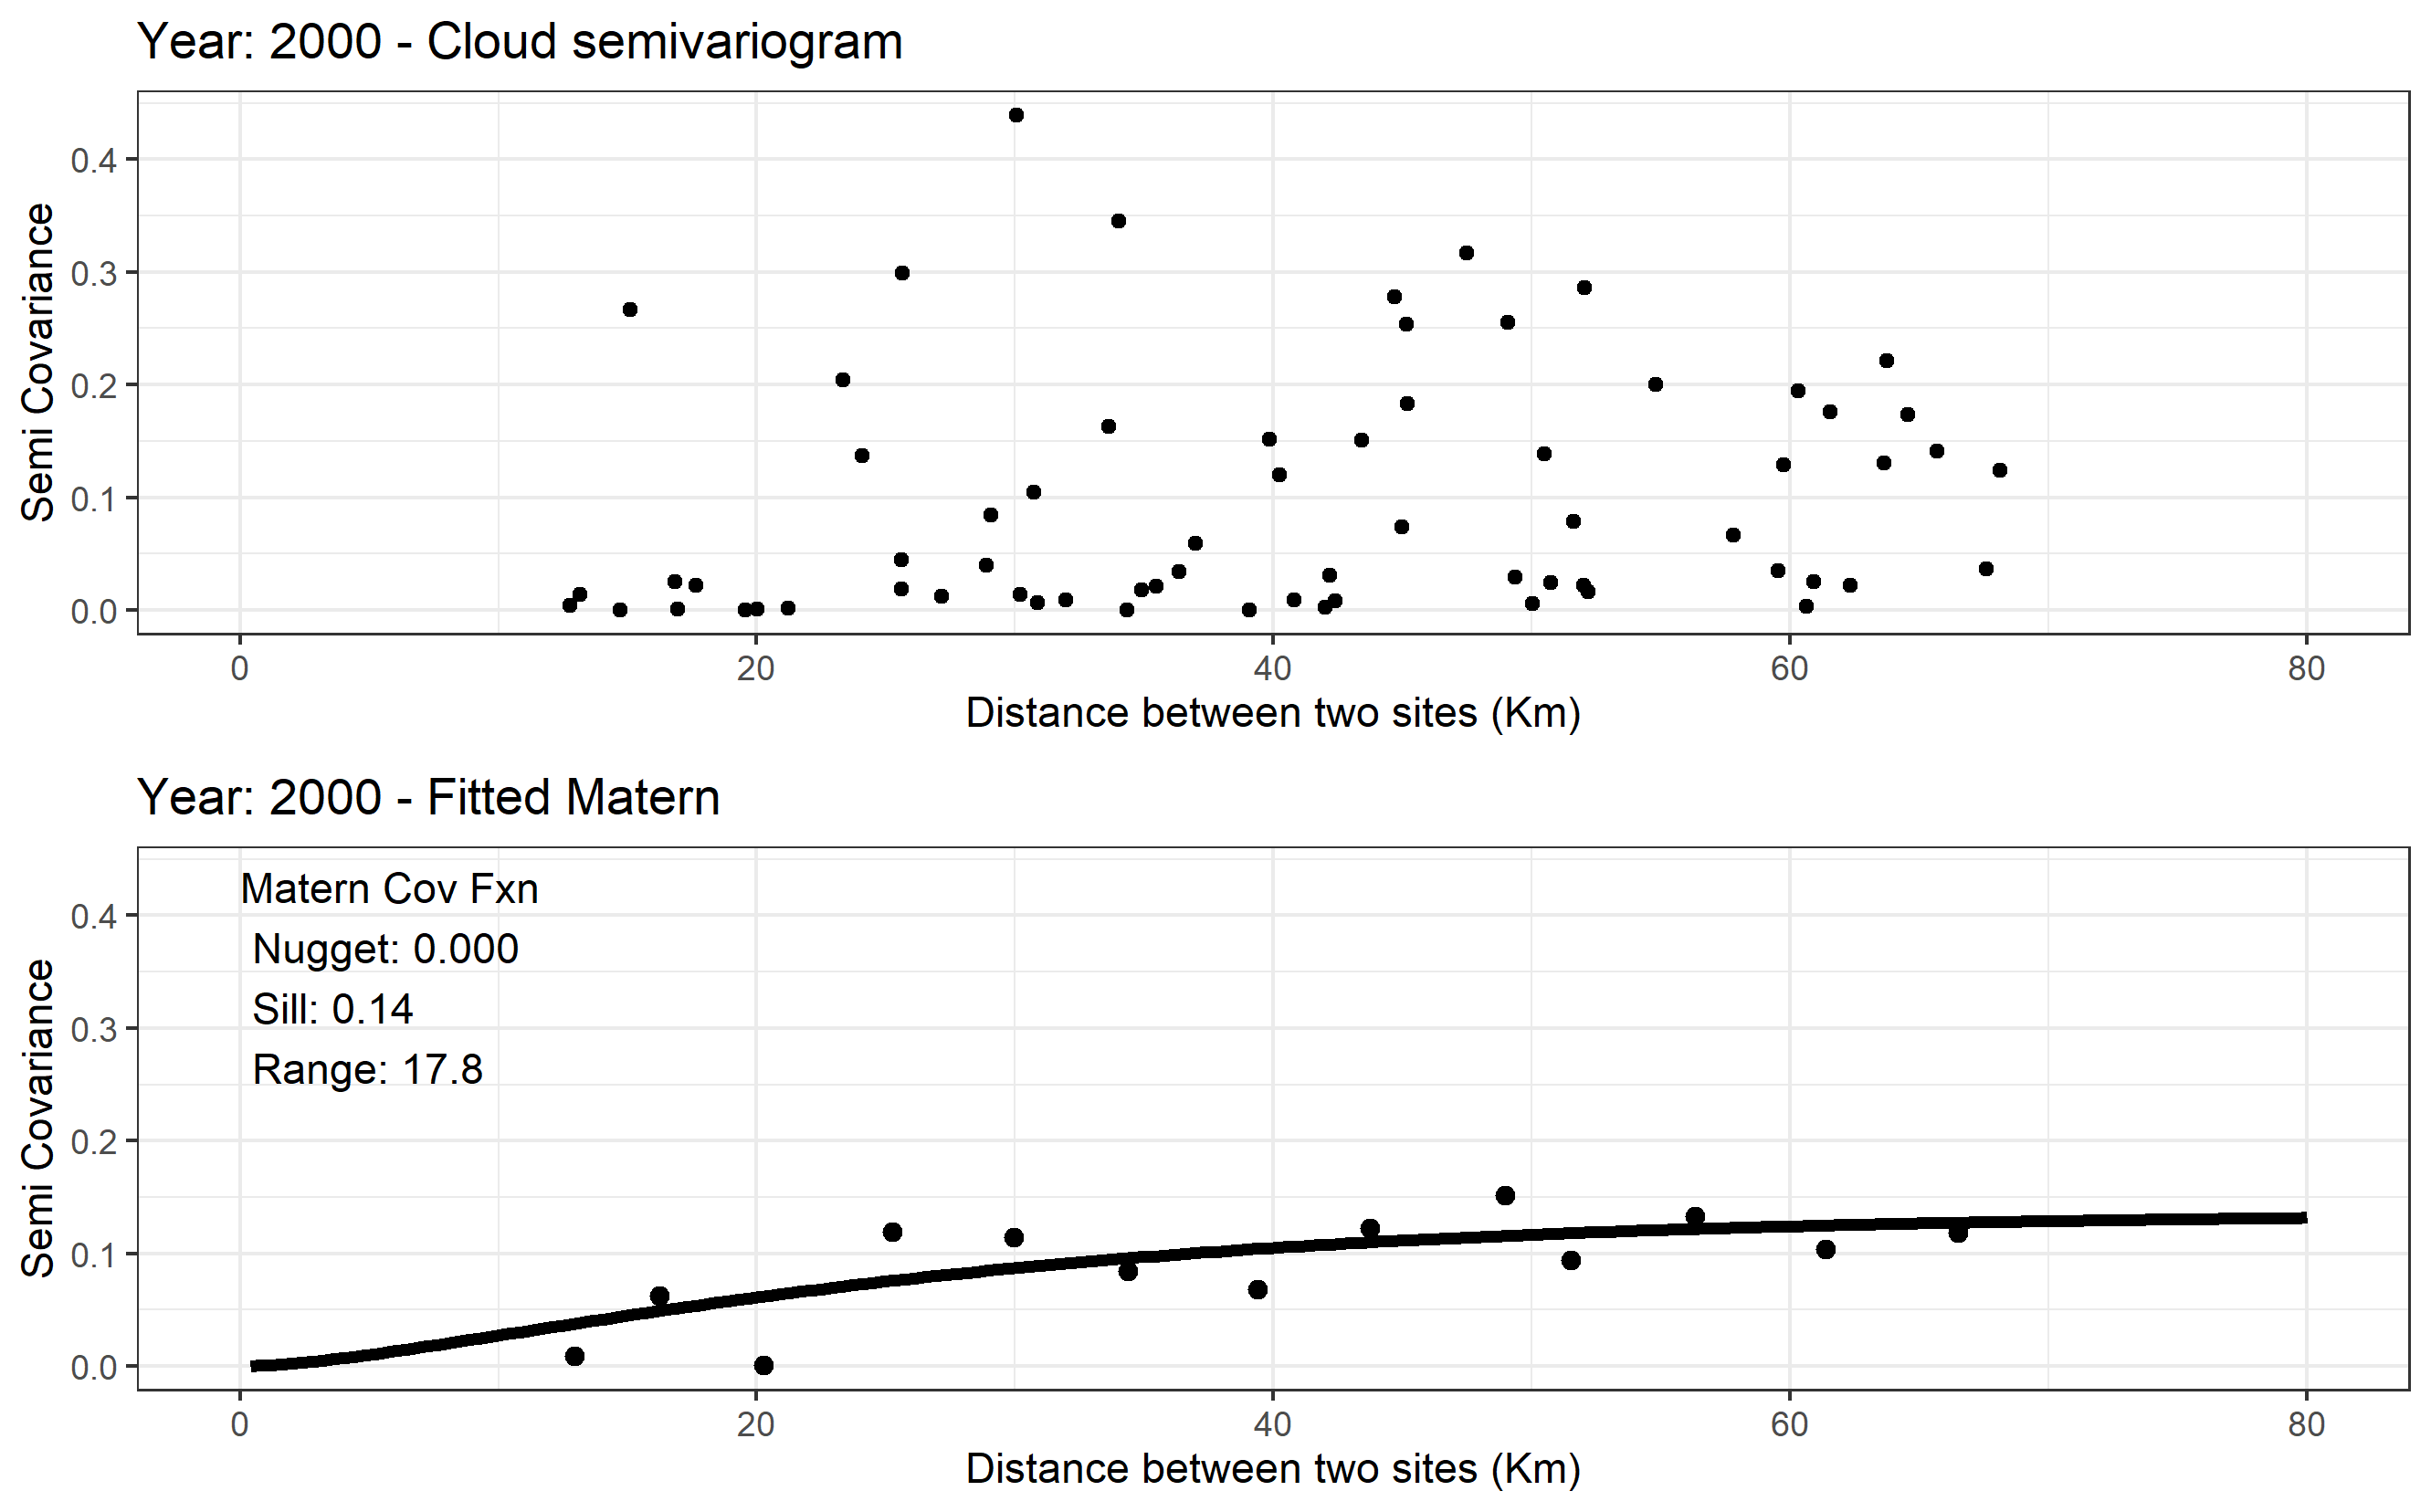}
    \caption{Caption}
    \label{fig:my_label}
\end{figure}

\begin{figure}
    \centering
    \includegraphics{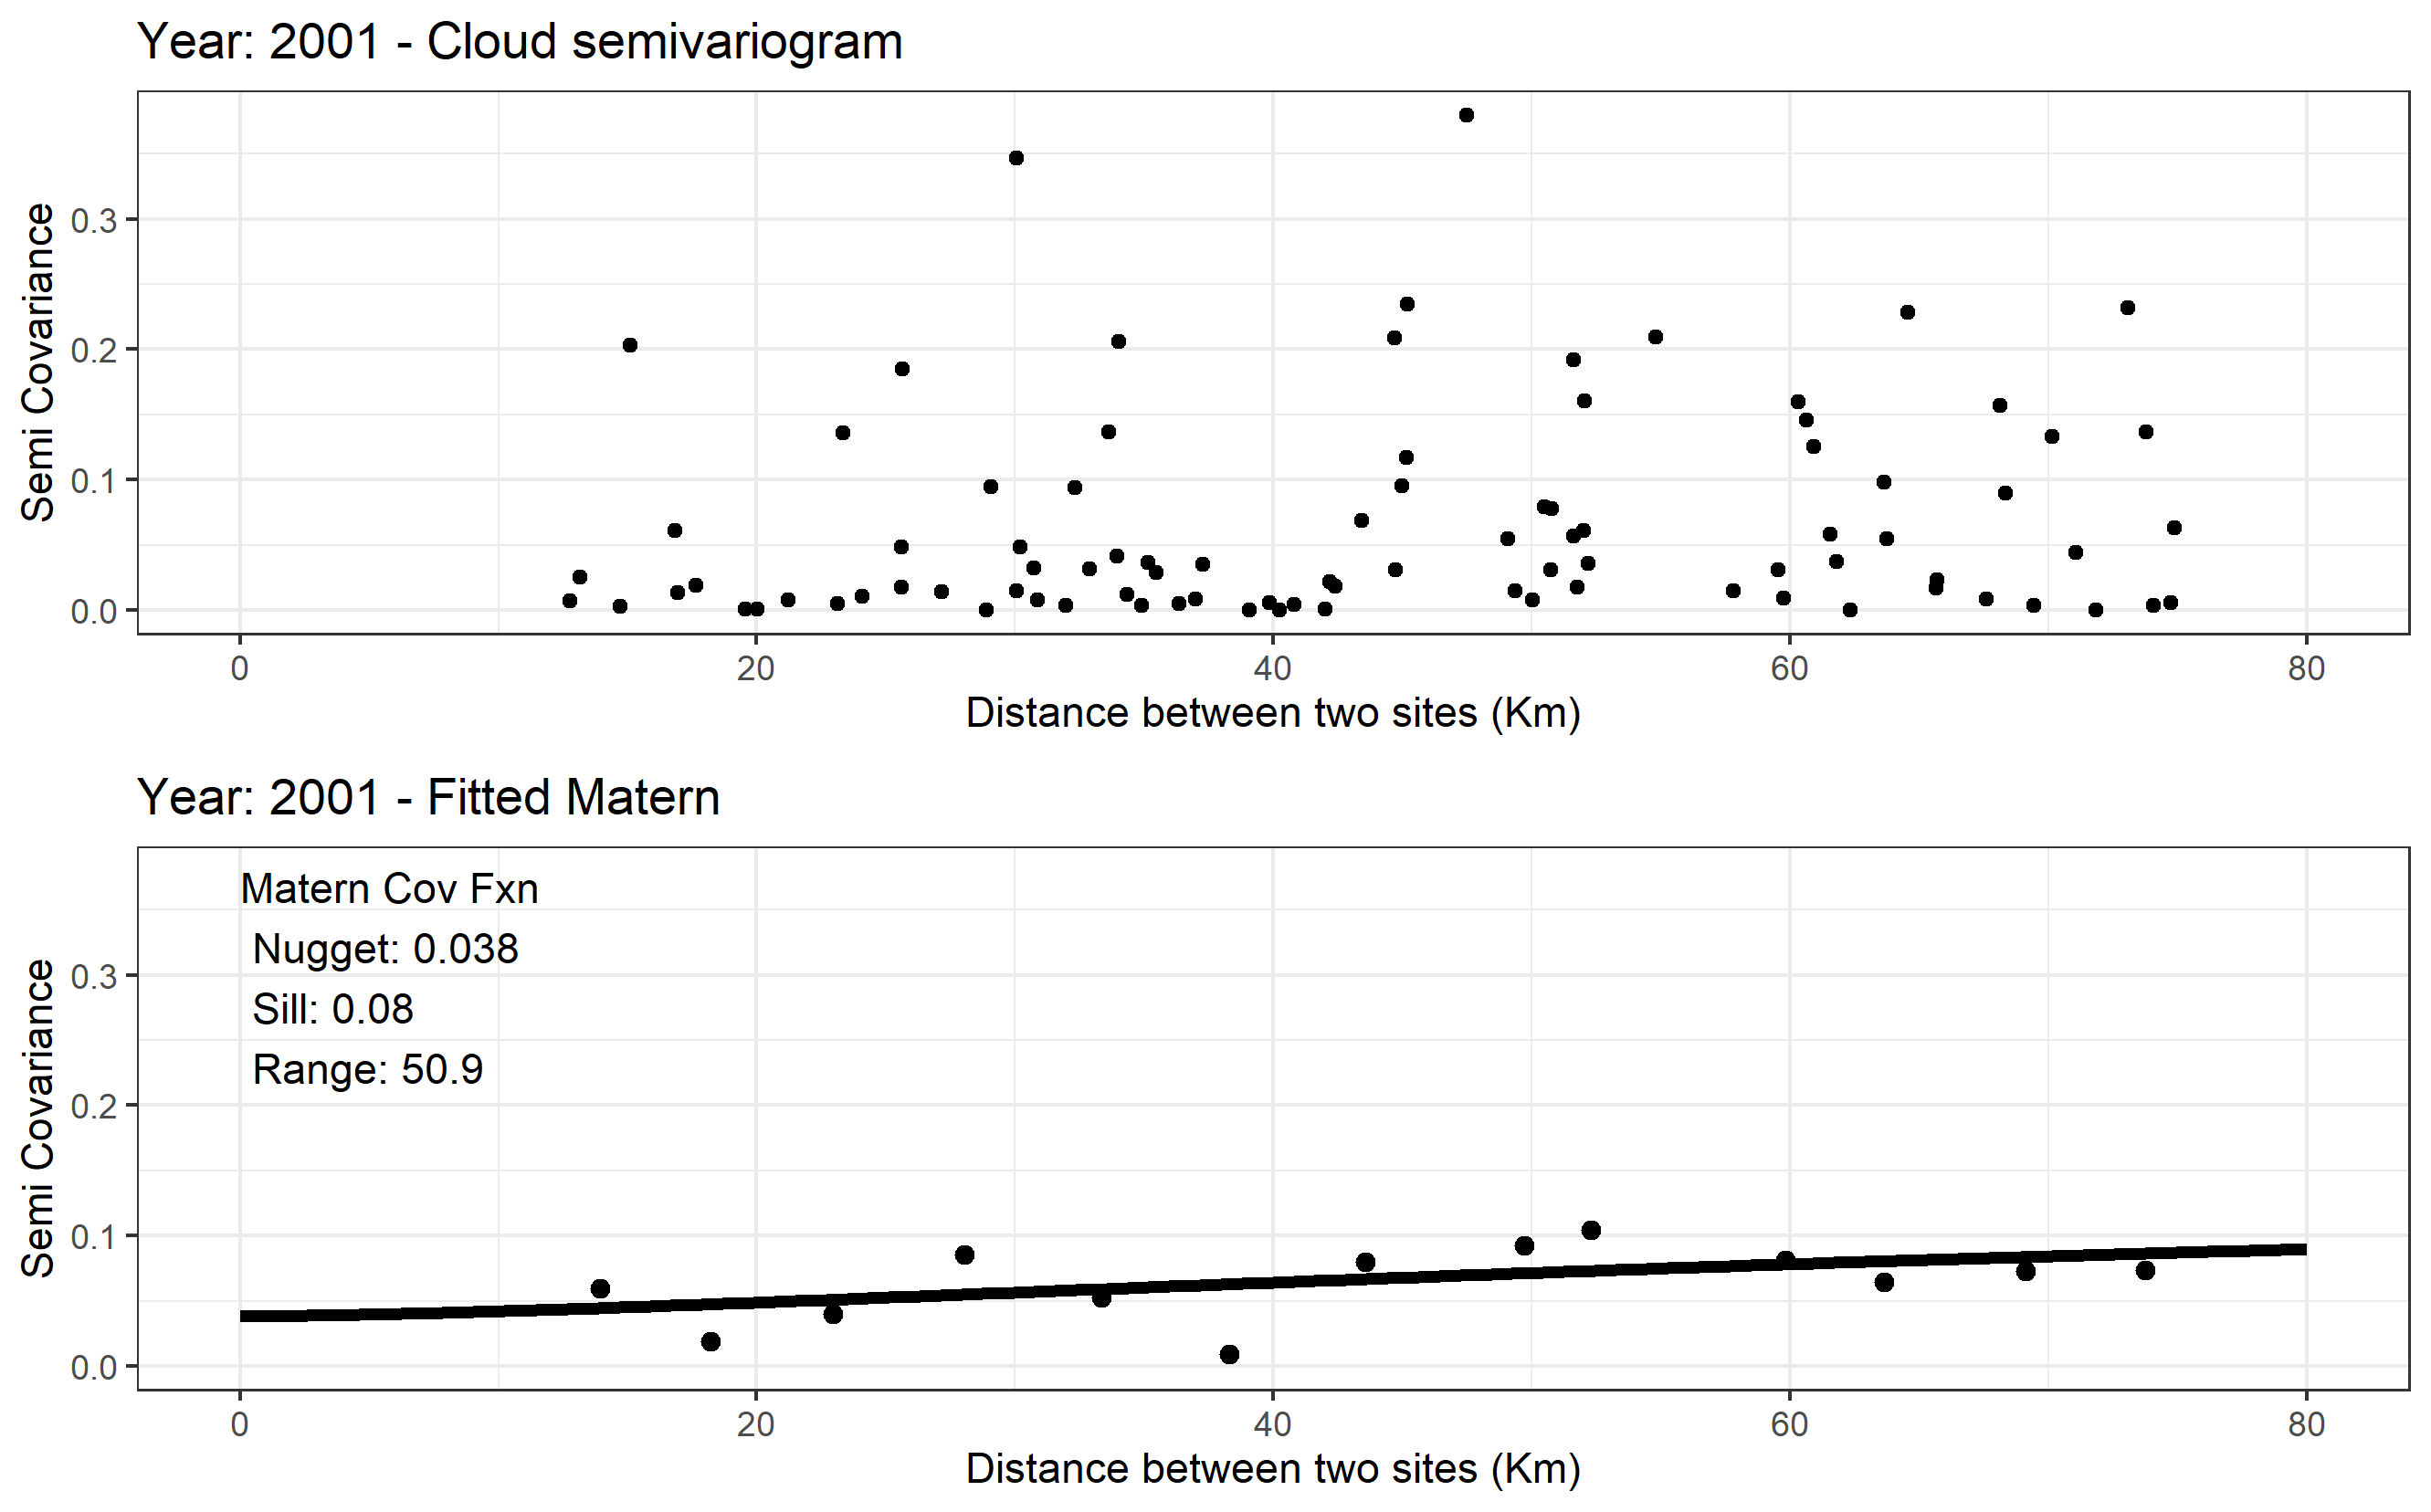}
    \caption{Caption}
    \label{fig:my_label}
\end{figure}

\begin{figure}
    \centering
    \includegraphics{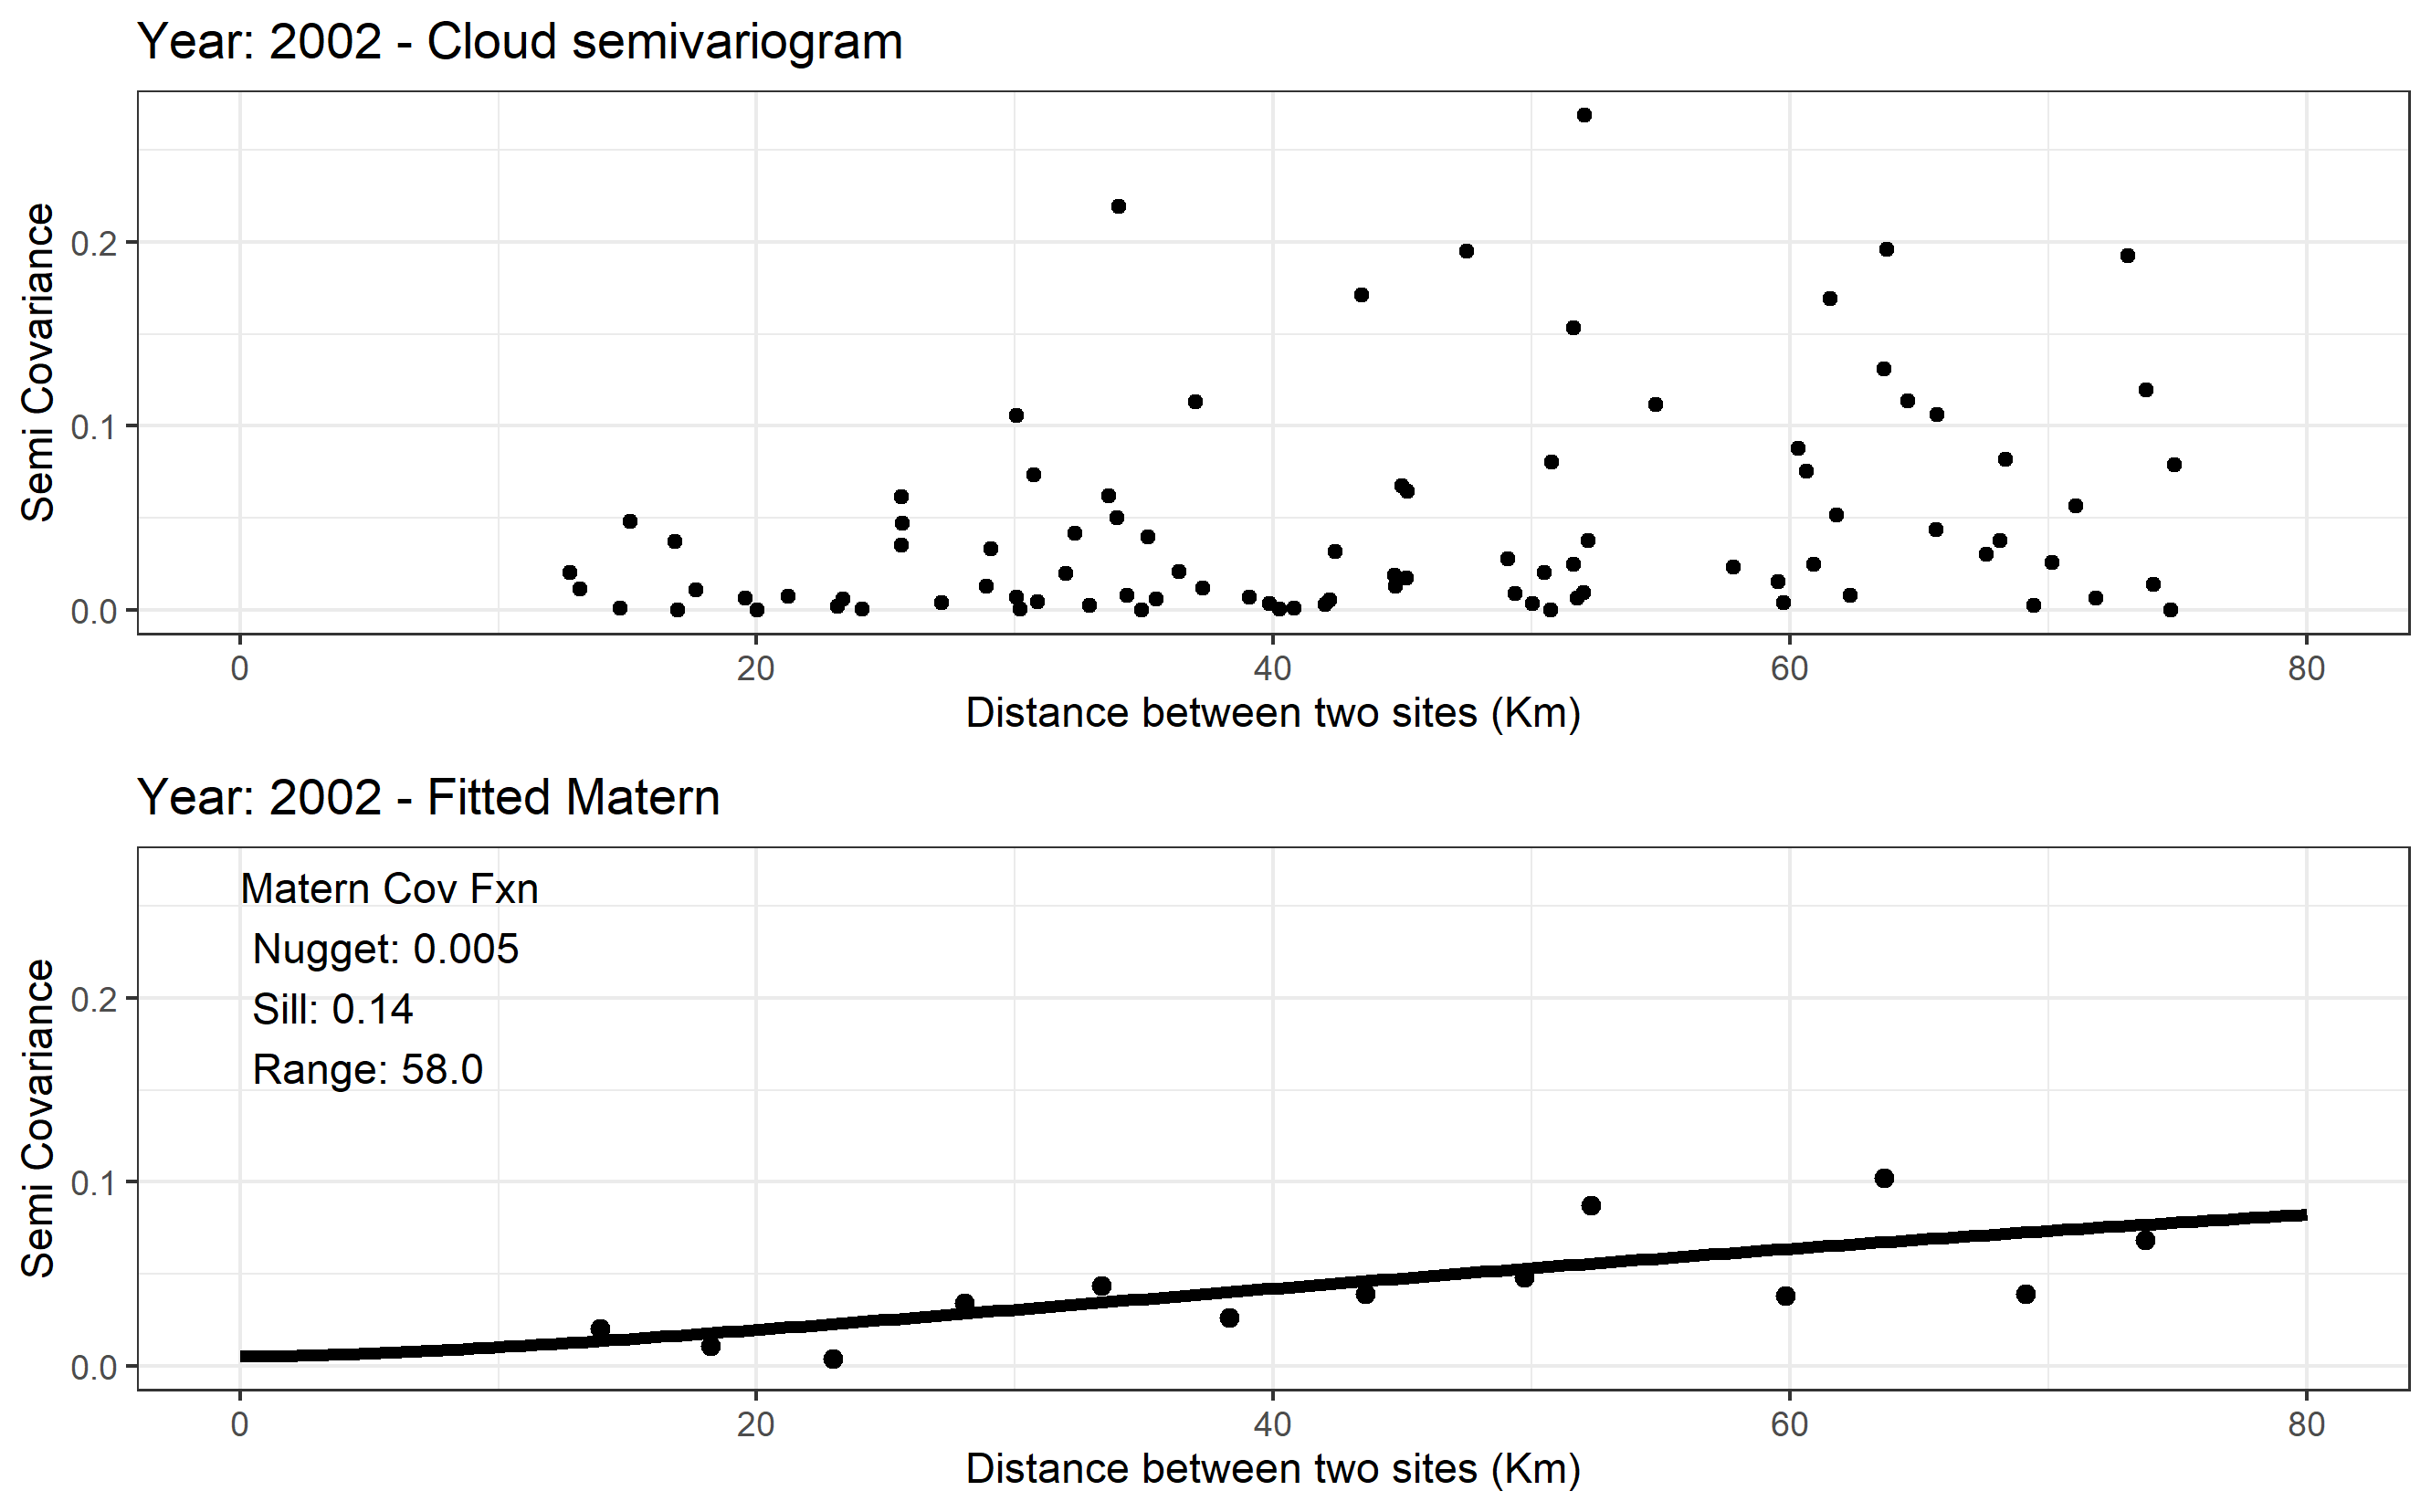}
    \caption{Caption}
    \label{fig:my_label}
\end{figure}

\begin{figure}
    \centering
    \includegraphics{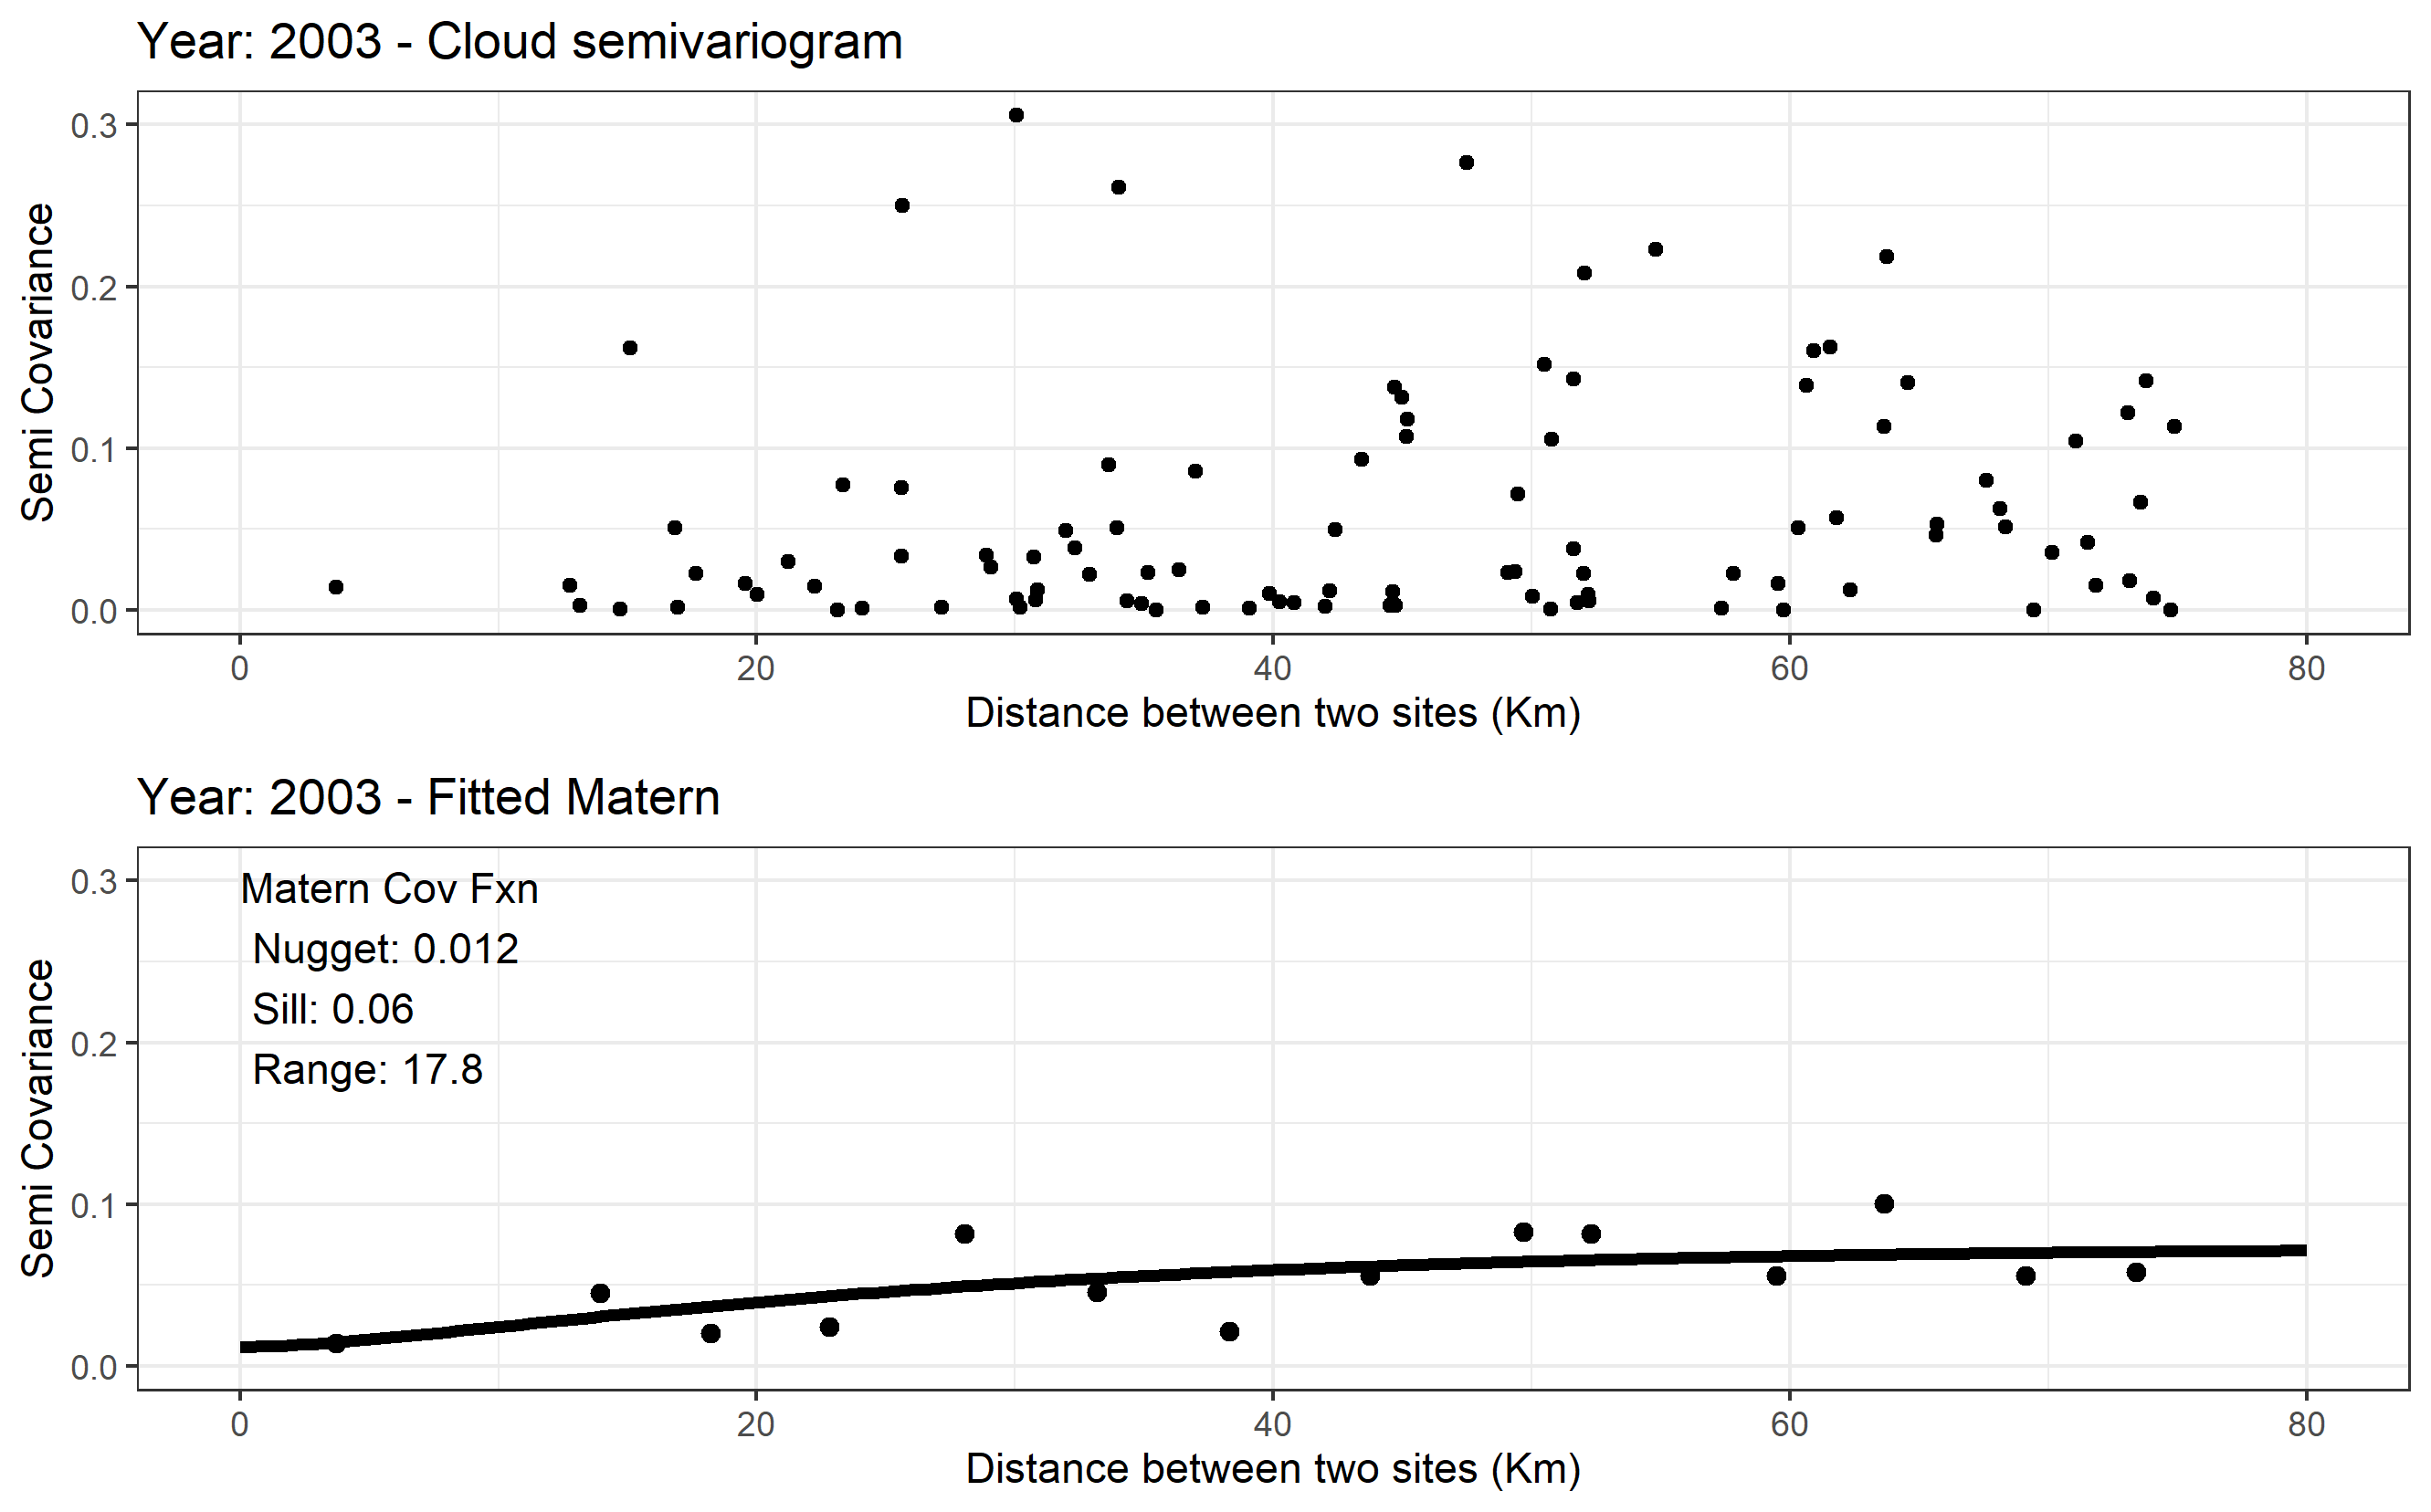}
    \caption{Caption}
    \label{fig:my_label}
\end{figure}

\begin{figure}
    \centering
    \includegraphics{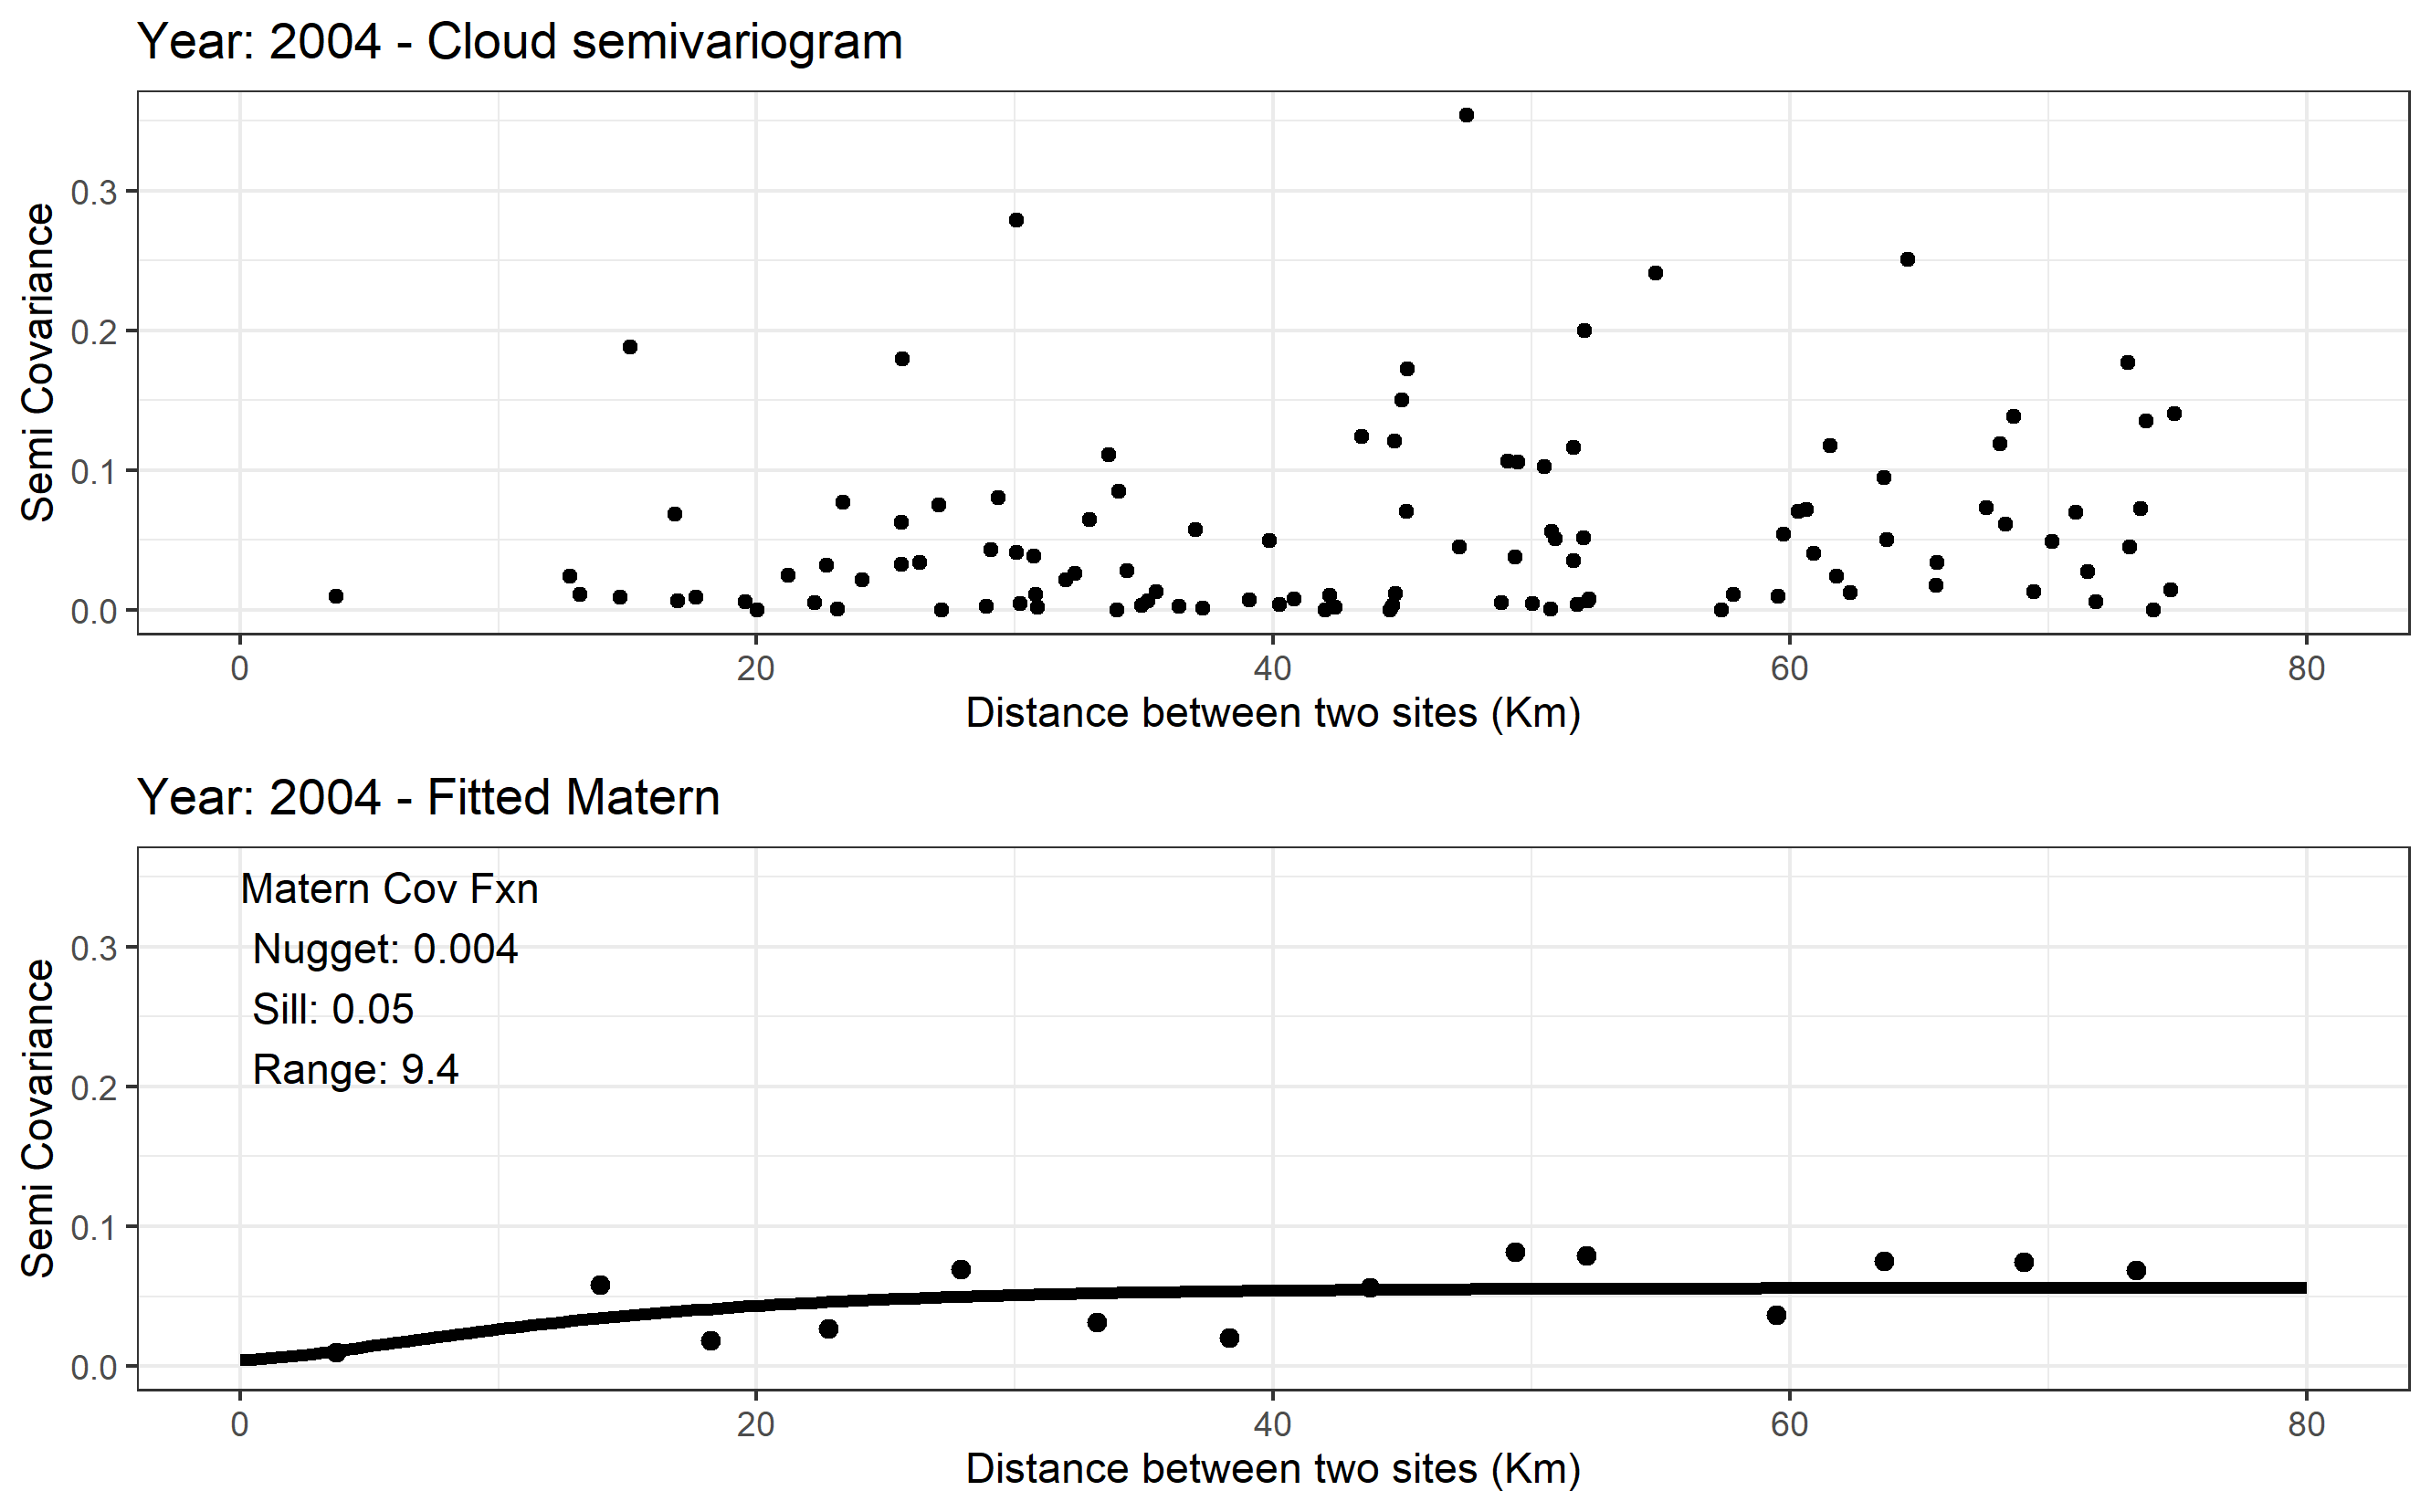}
    \caption{Caption}
    \label{fig:my_label}
\end{figure}

\begin{figure}
    \centering
    \includegraphics{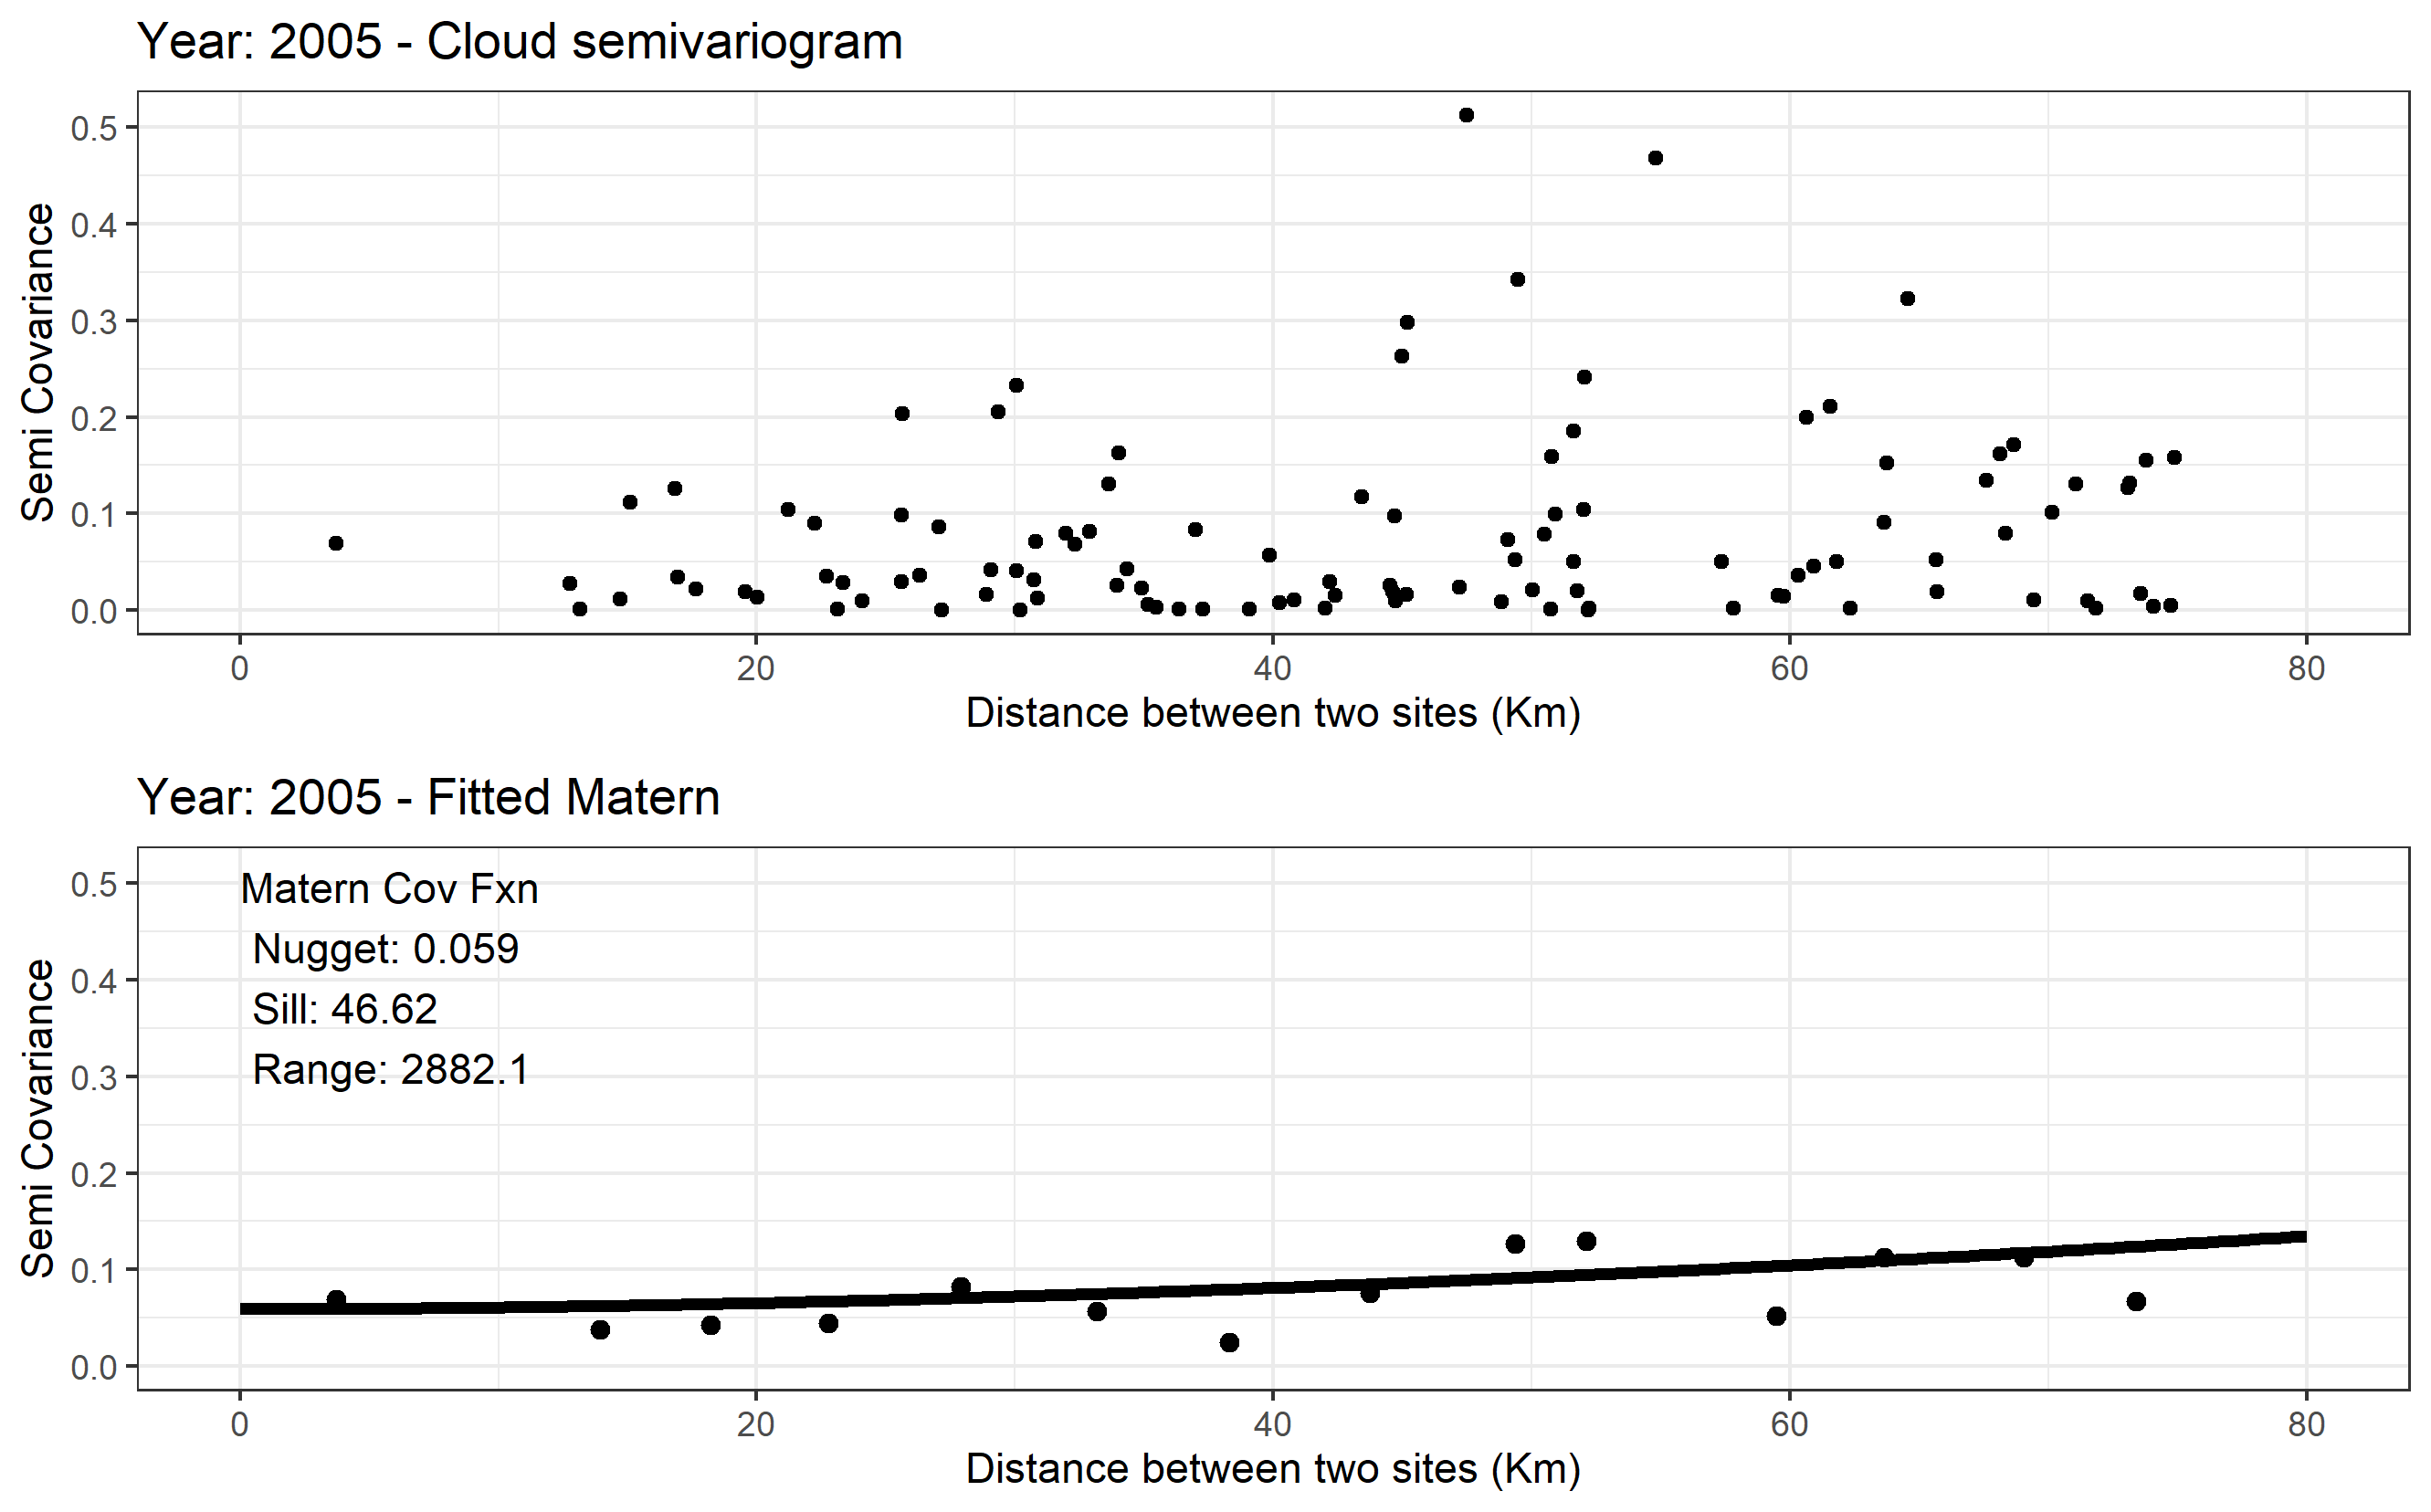}
    \caption{Caption}
    \label{fig:my_label}
\end{figure}

\begin{figure}
    \centering
    \includegraphics{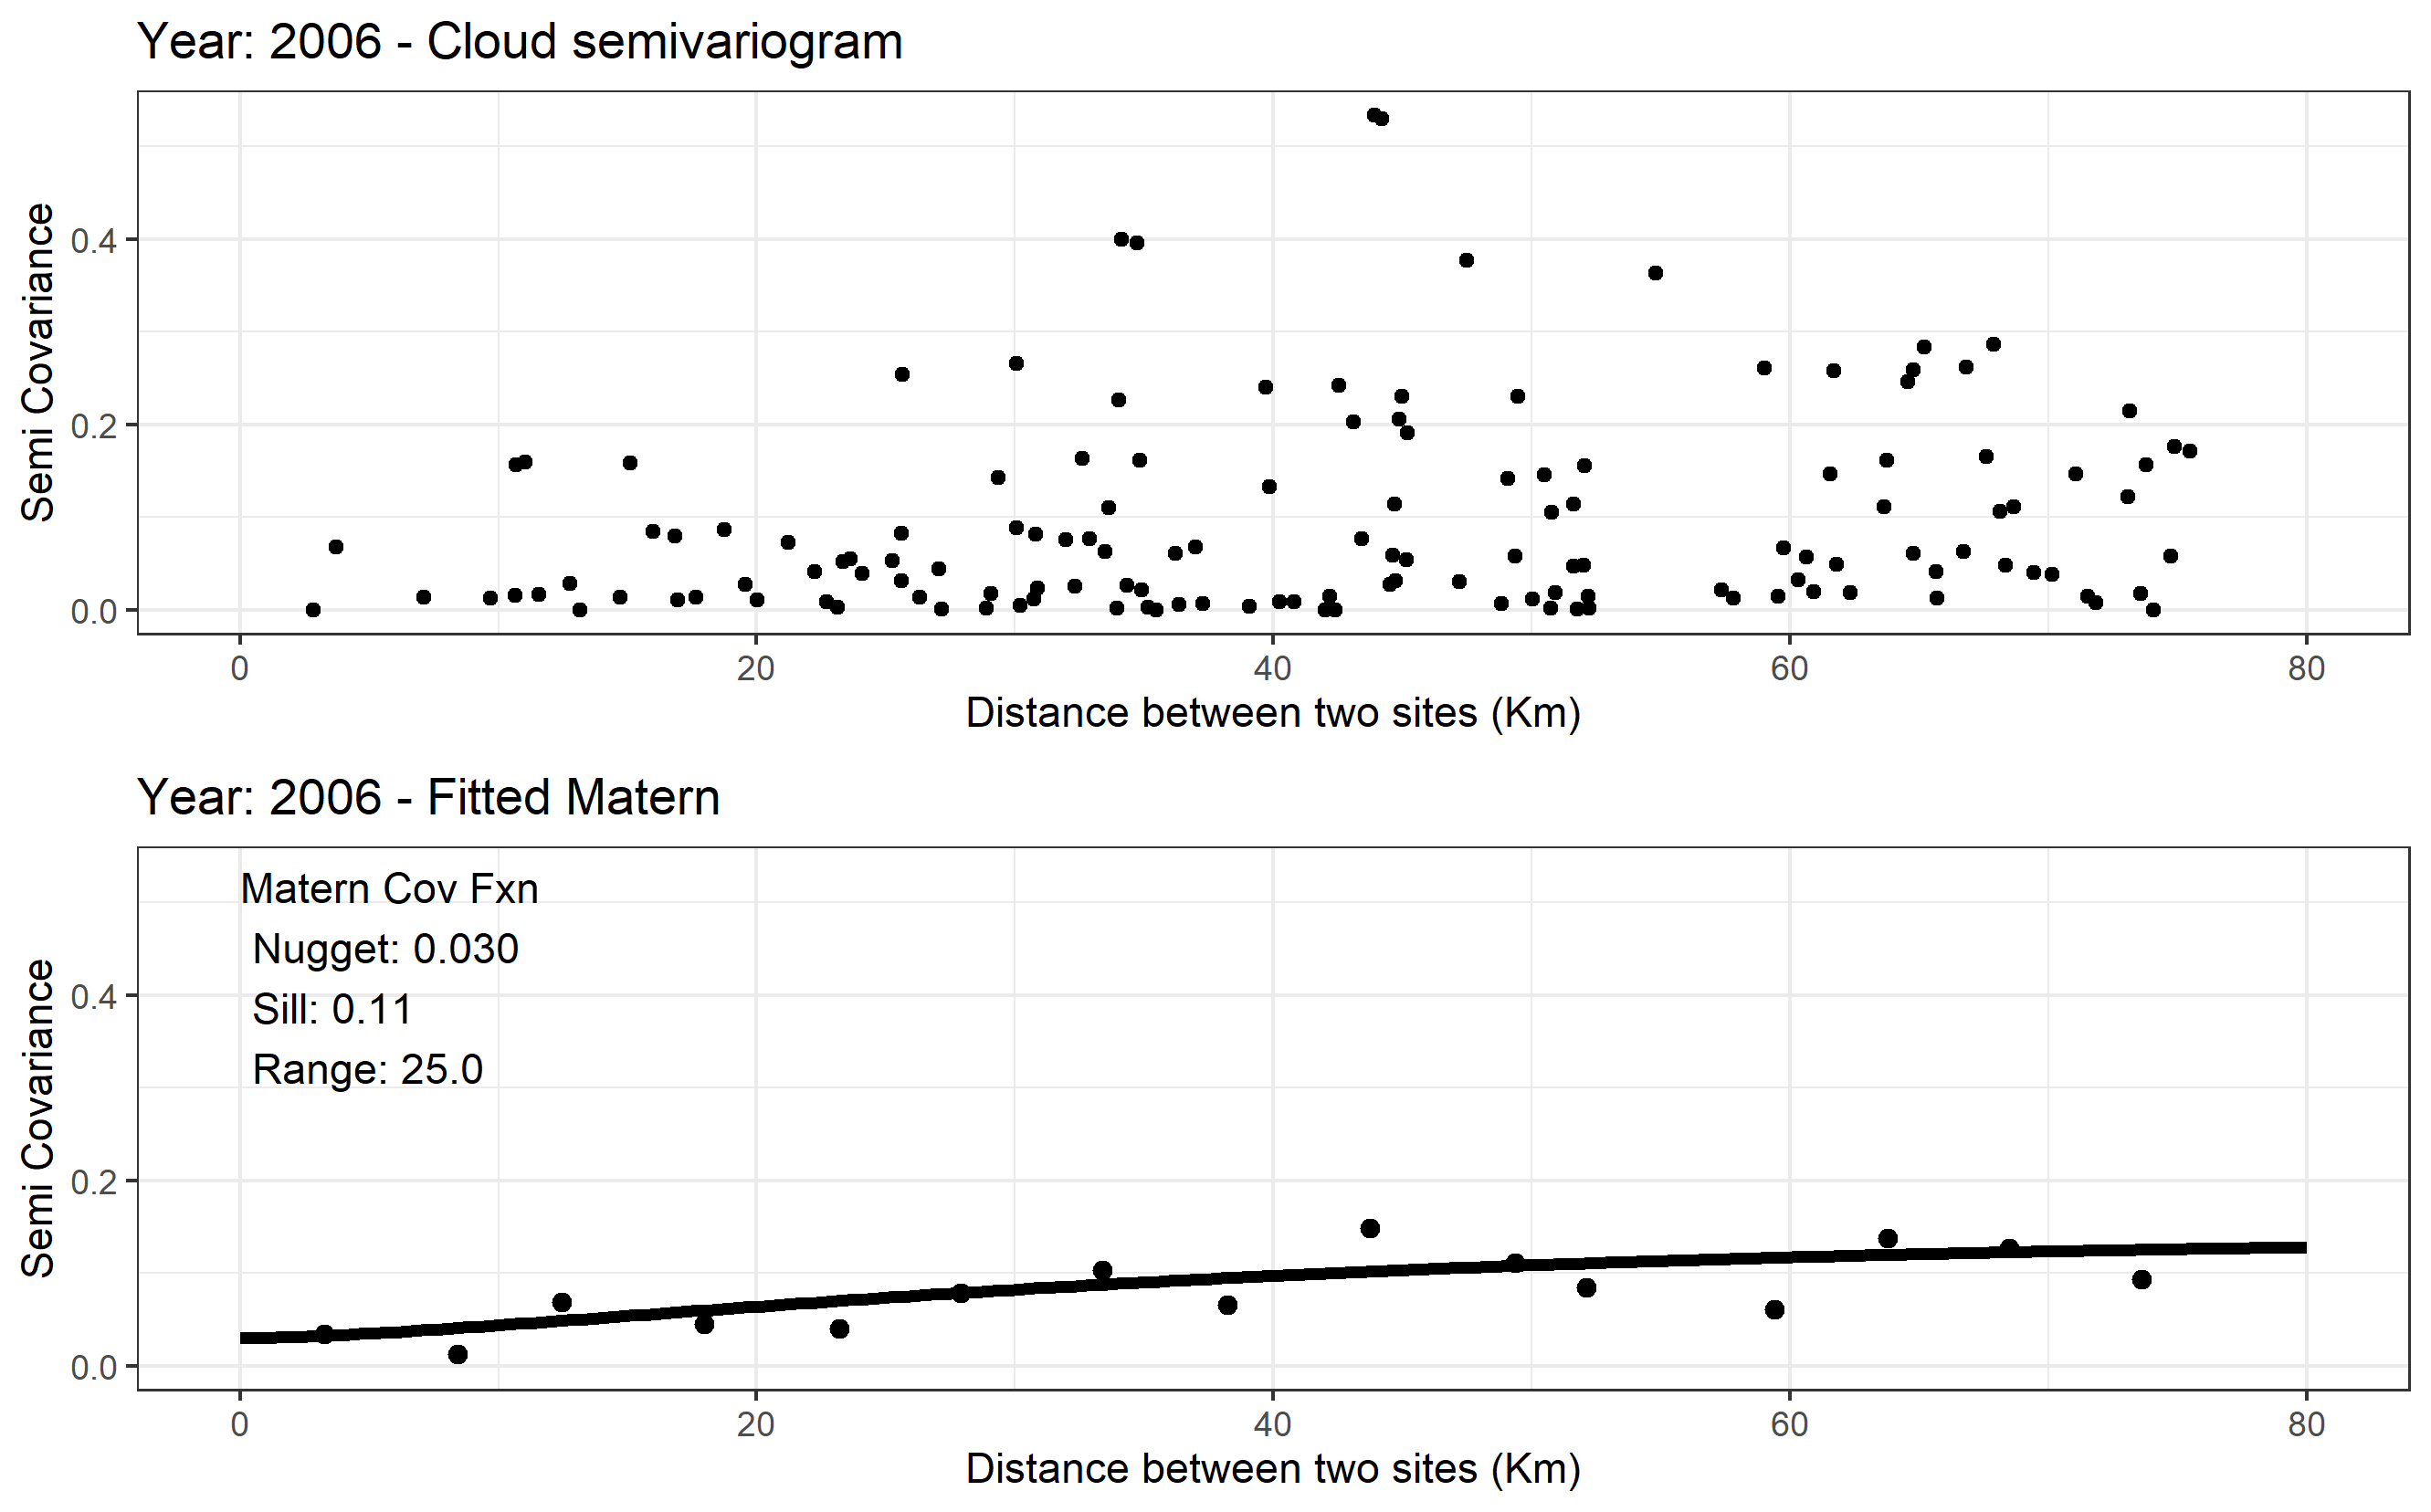}
    \caption{Caption}
    \label{fig:my_label}
\end{figure}

\begin{figure}
    \centering
    \includegraphics{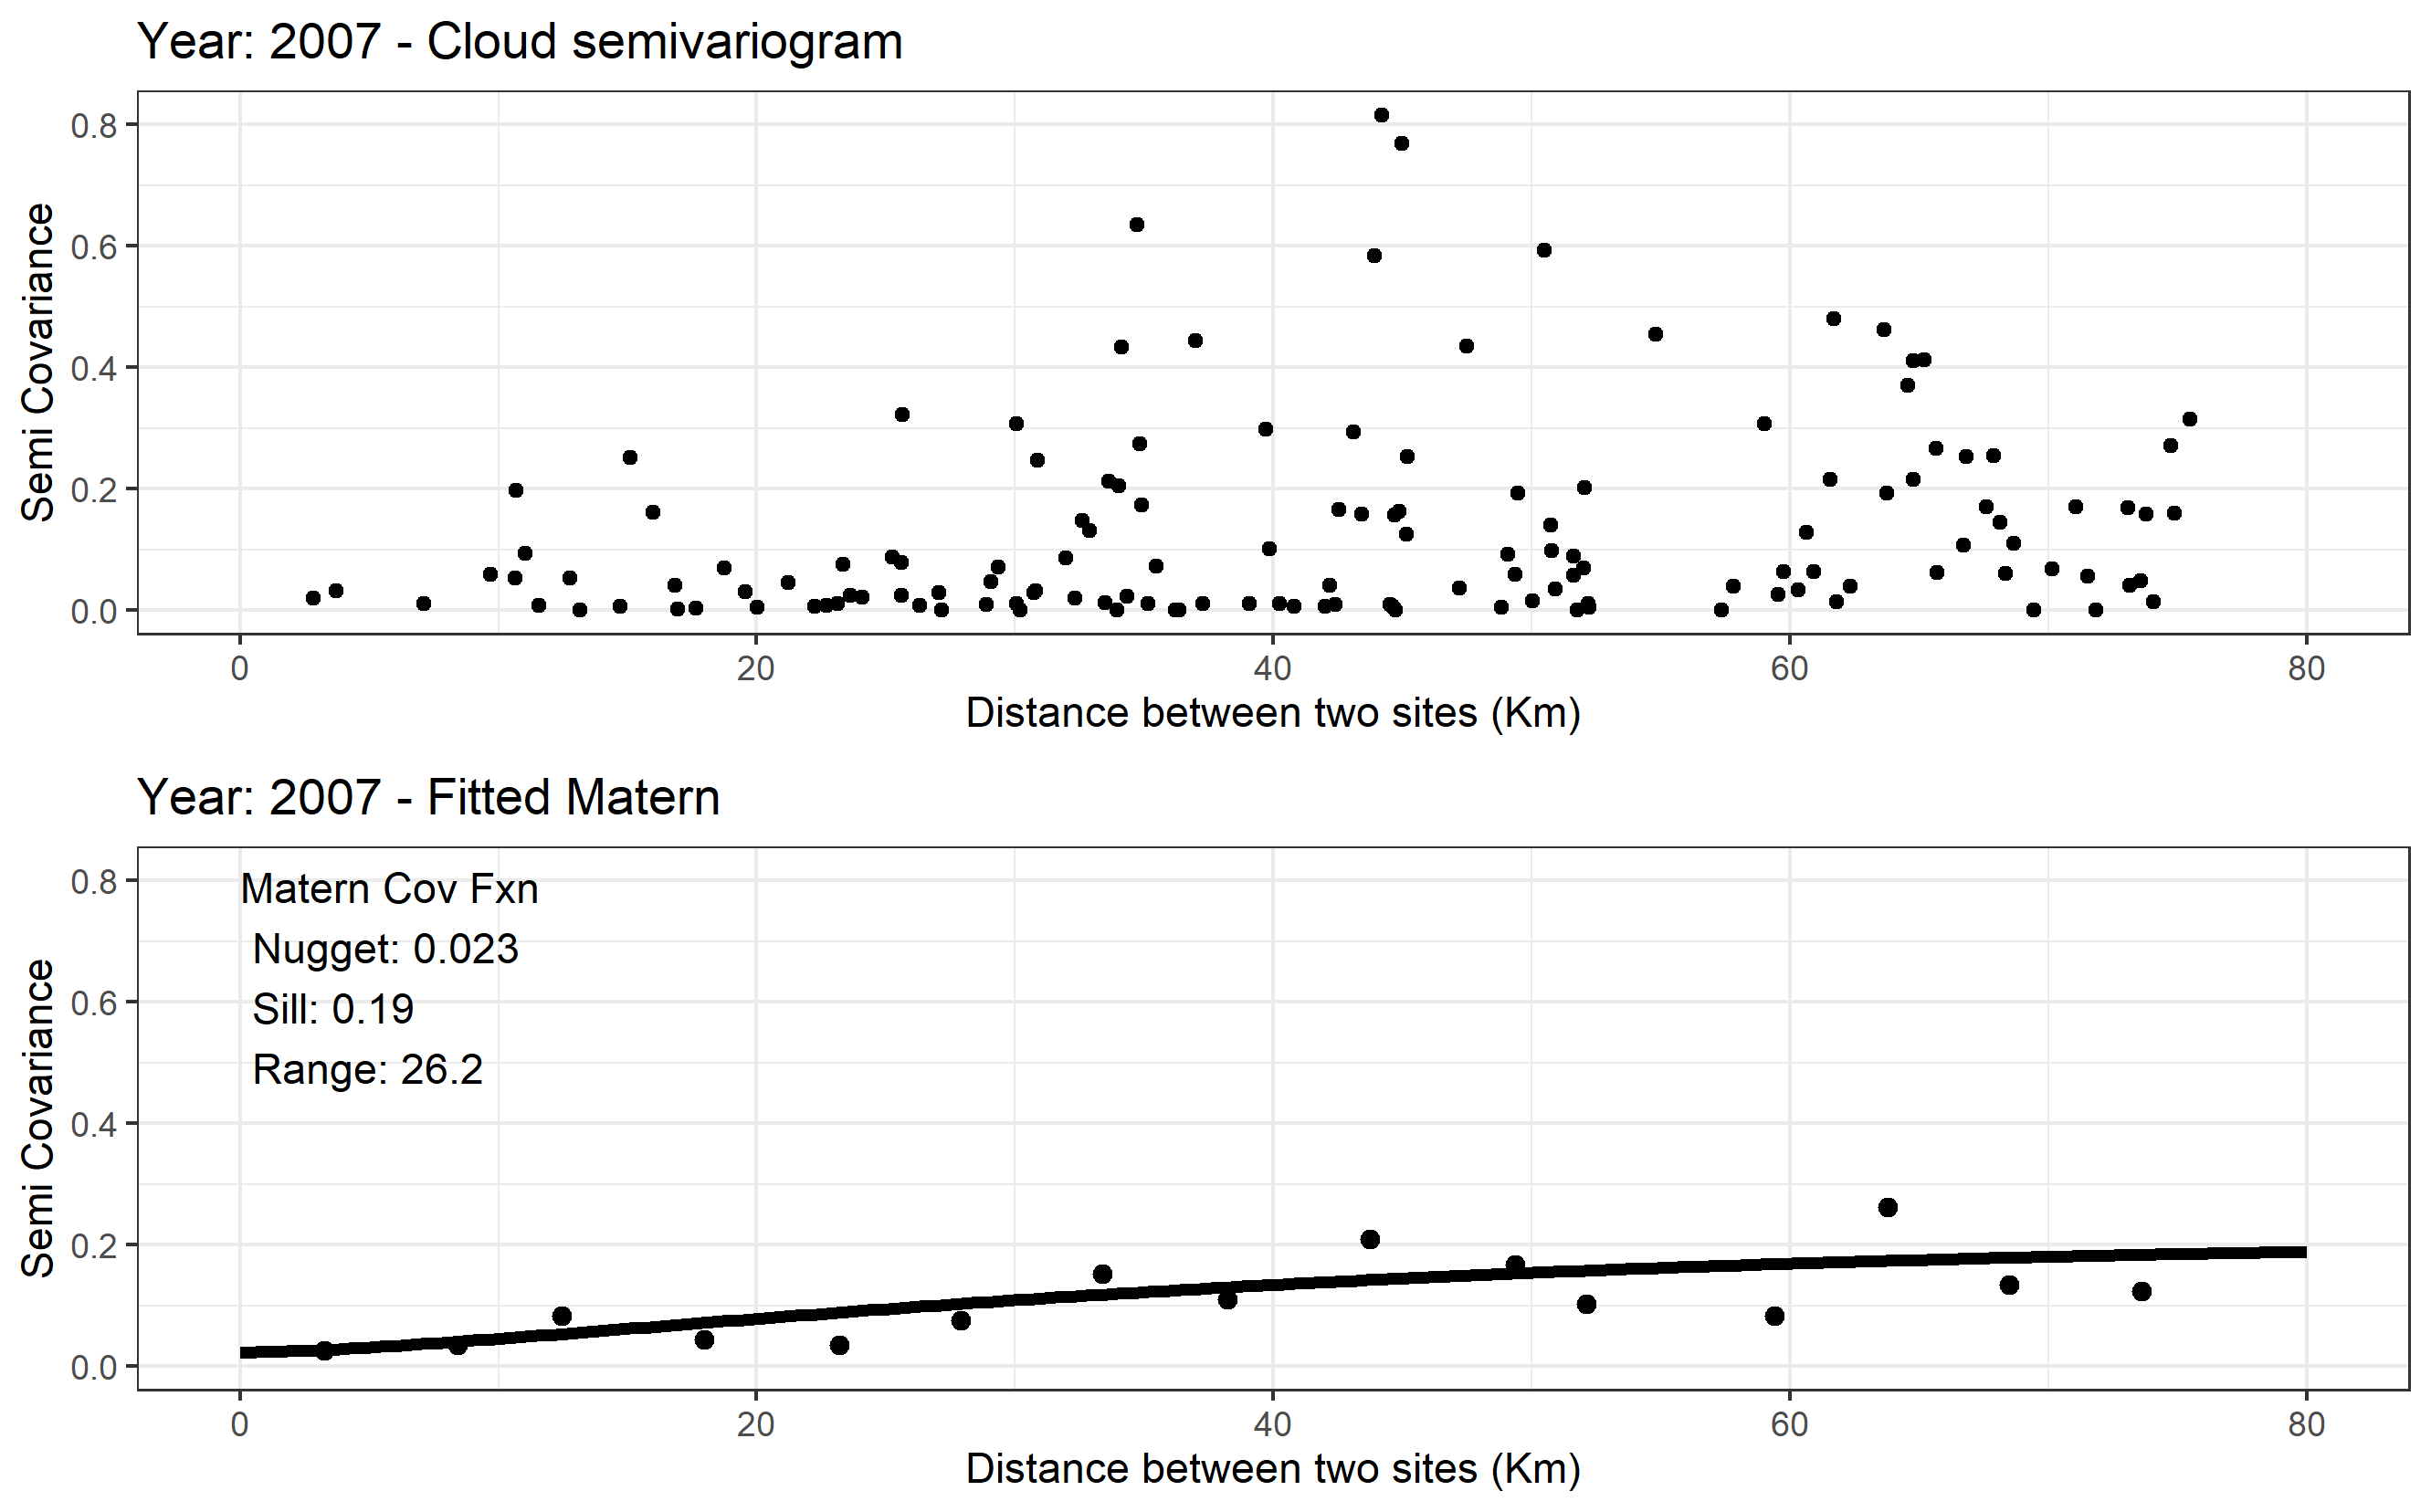}
    \caption{Caption}
    \label{fig:my_label}
\end{figure}

\begin{figure}
    \centering
    \includegraphics{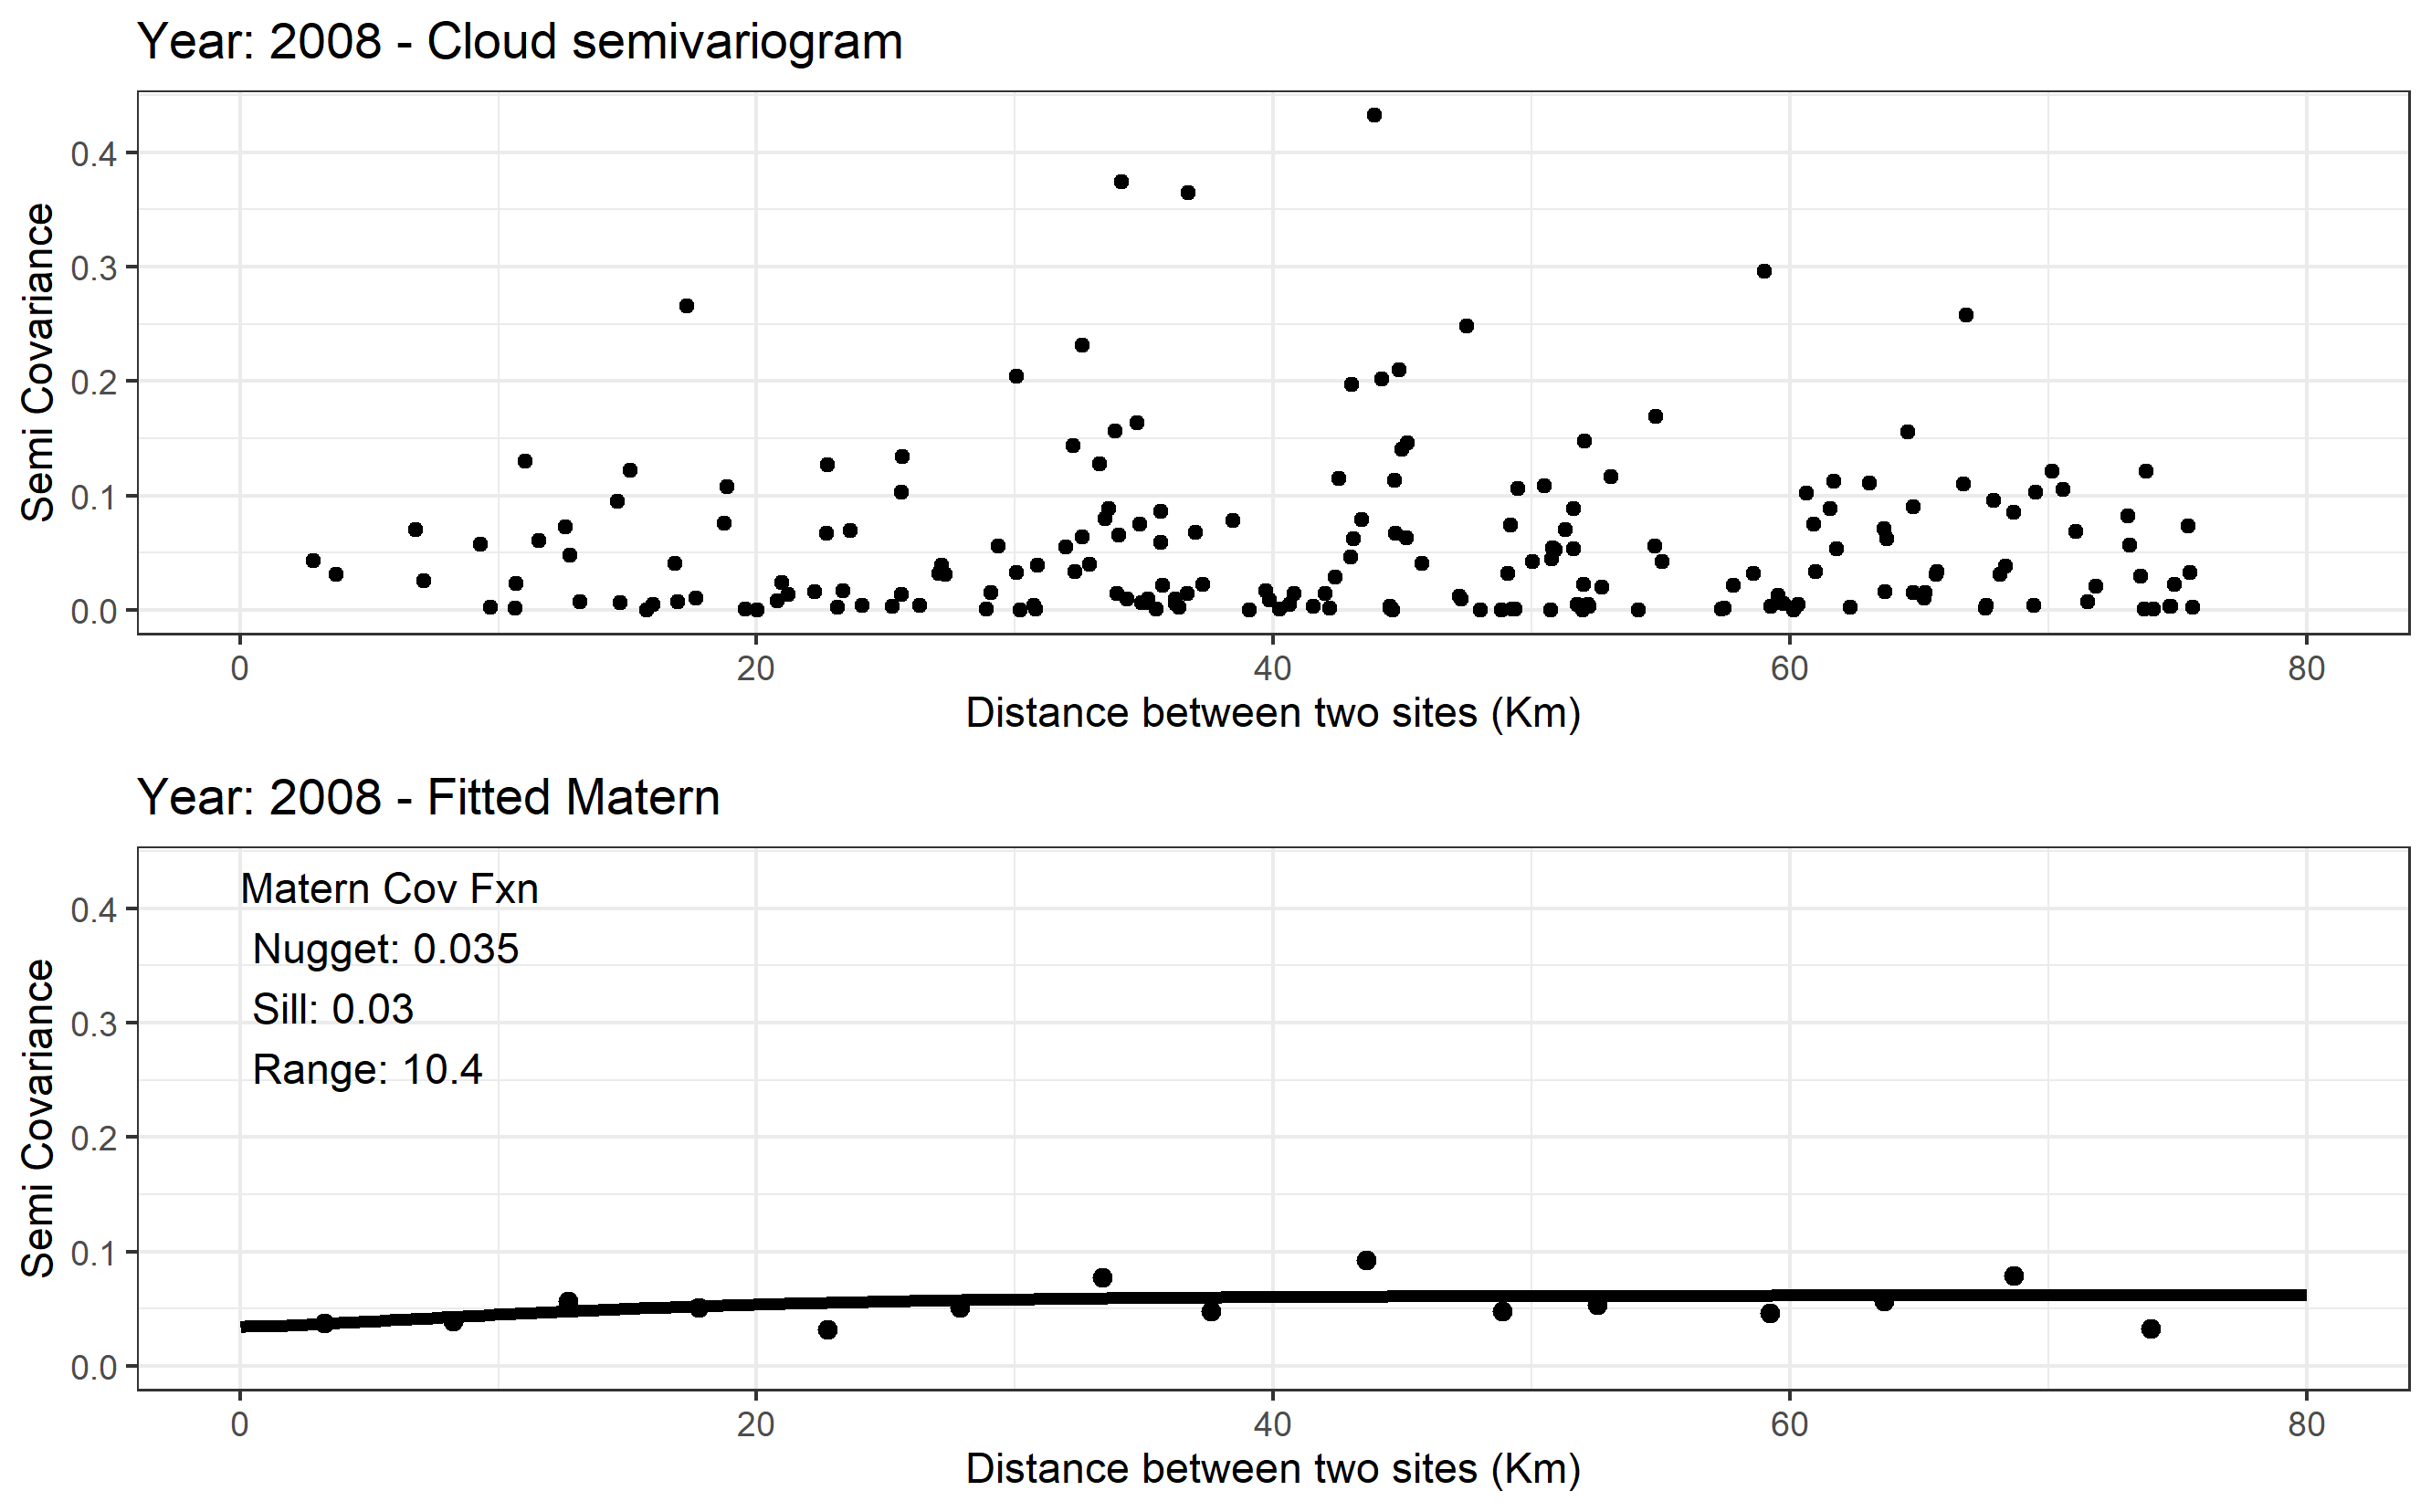}
    \caption{Caption}
    \label{fig:my_label}
\end{figure}

\begin{figure}
    \centering
    \includegraphics{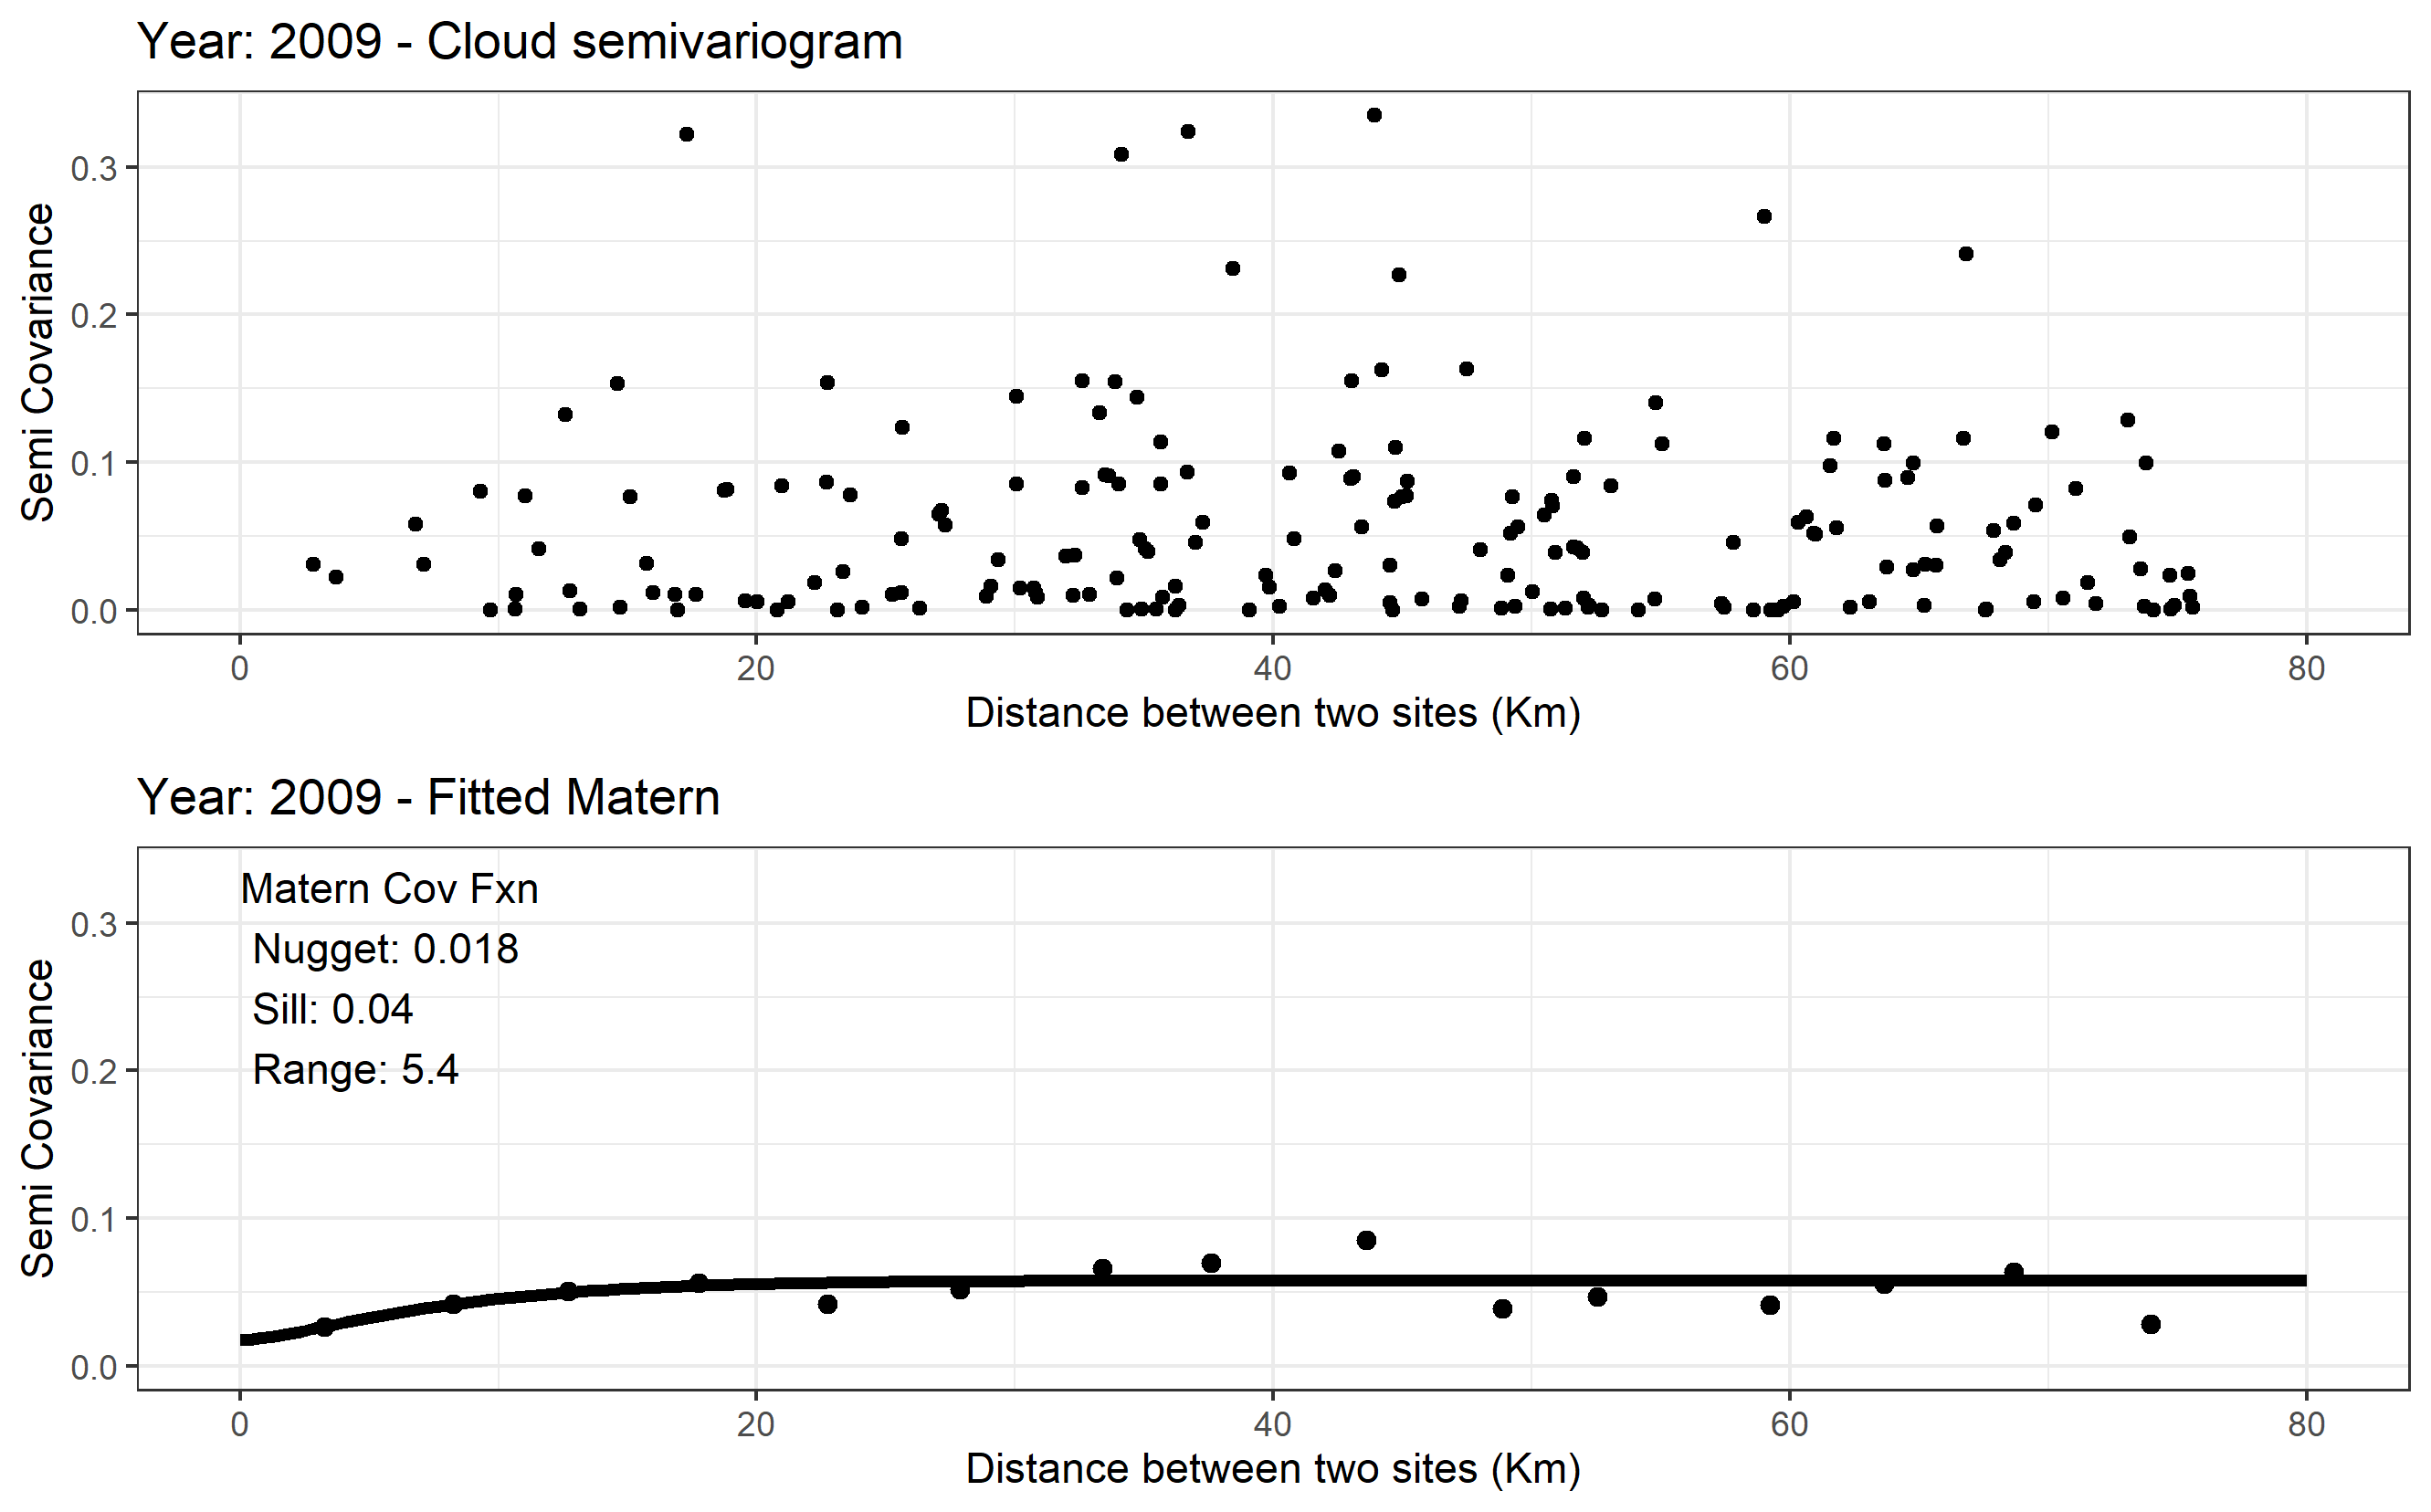}
    \caption{Caption}
    \label{fig:my_label}
\end{figure}

\begin{figure}
    \centering
    \includegraphics{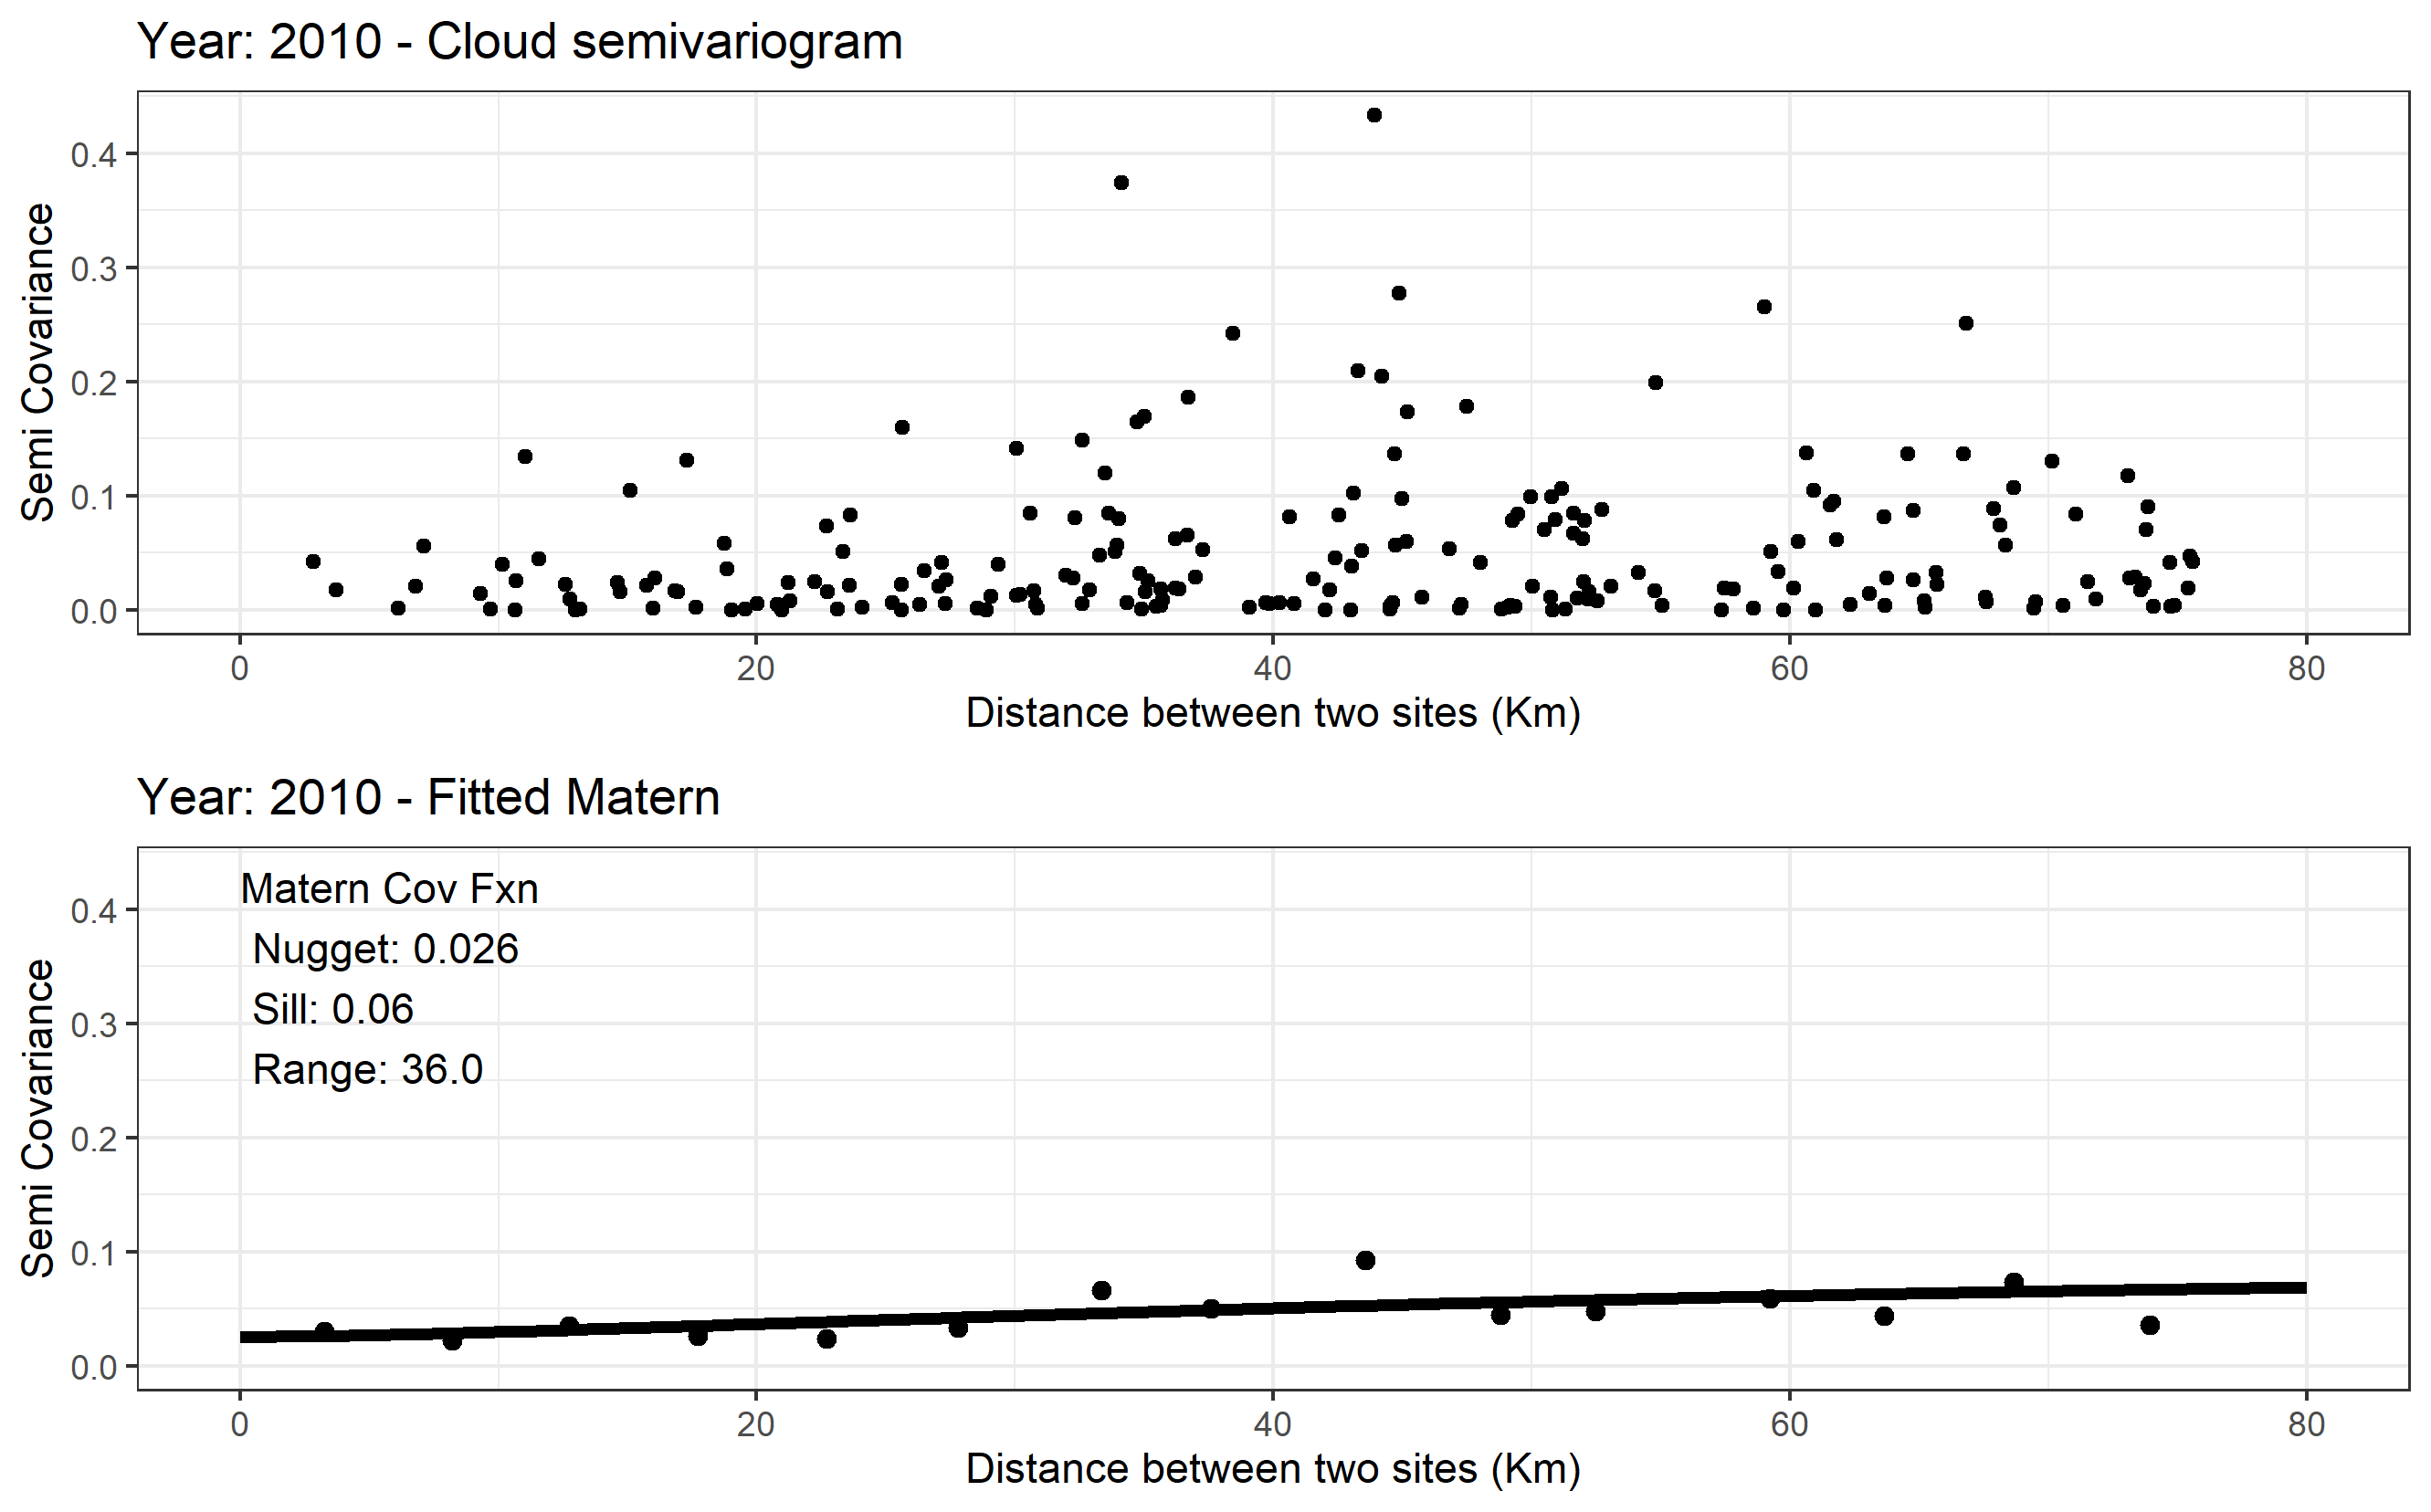}
    \caption{Caption}
    \label{fig:my_label}
\end{figure}

\begin{figure}
    \centering
    \includegraphics{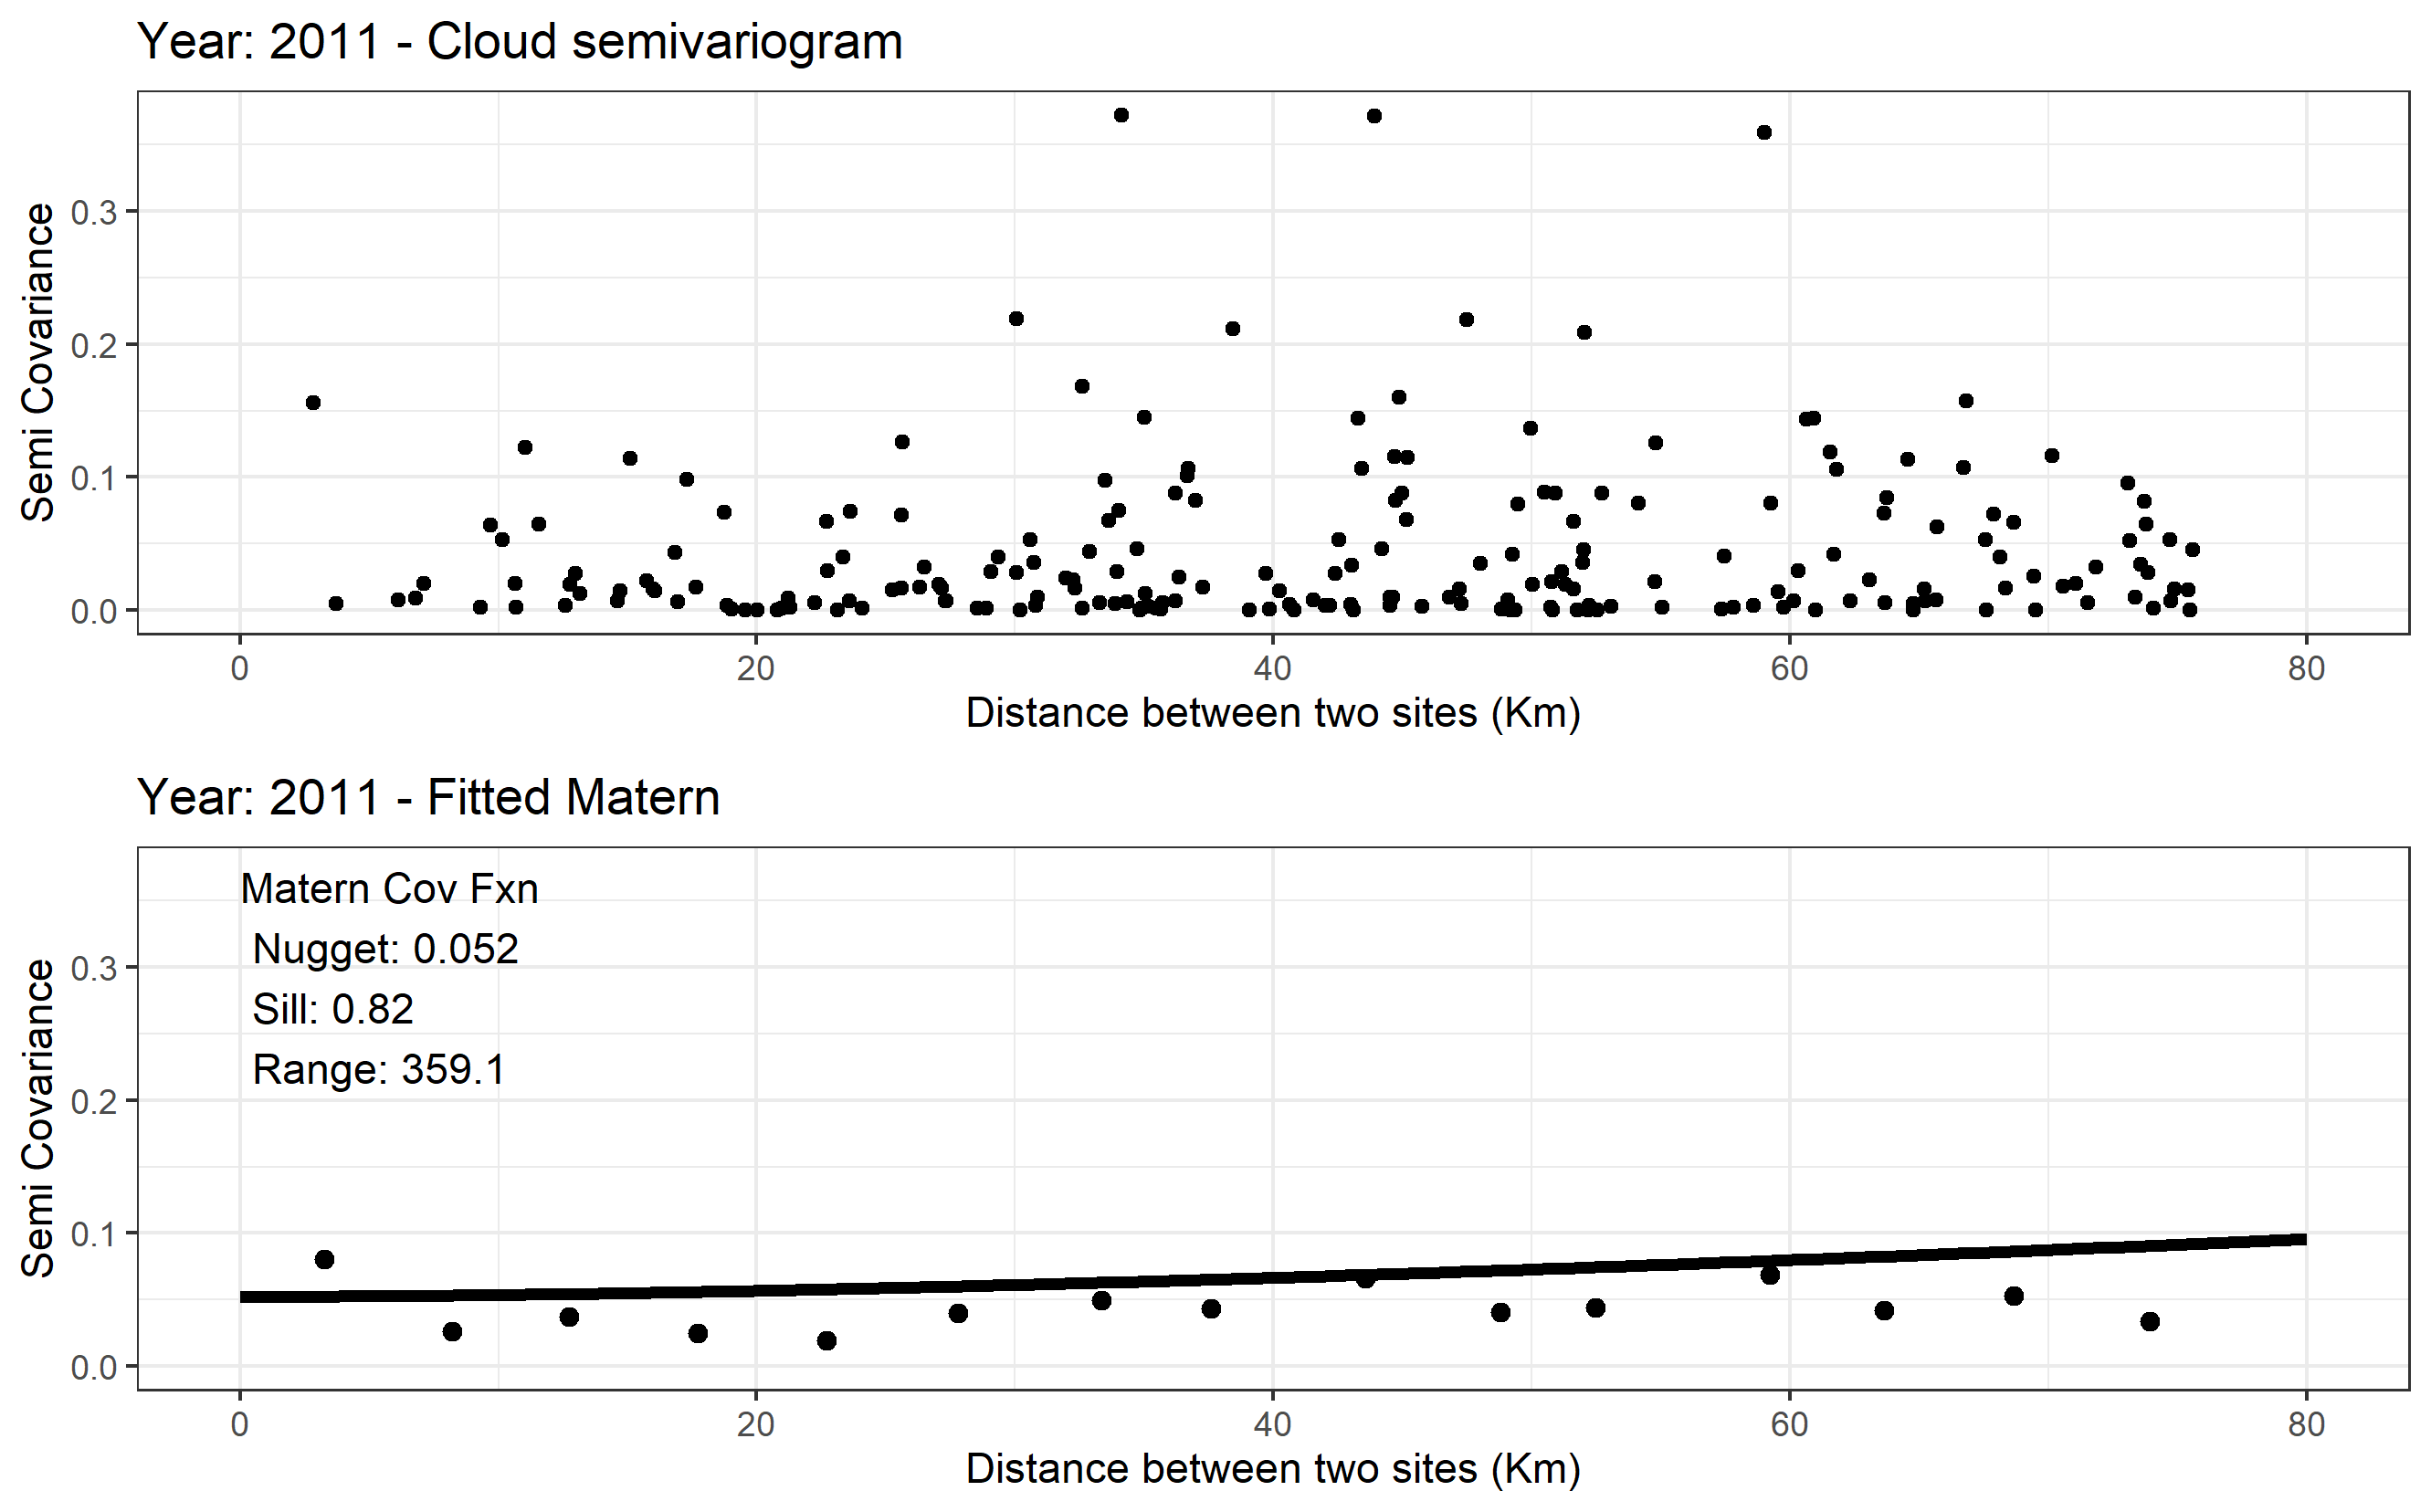}
    \caption{Caption}
    \label{fig:my_label}
\end{figure}

\begin{figure}
    \centering
    \includegraphics{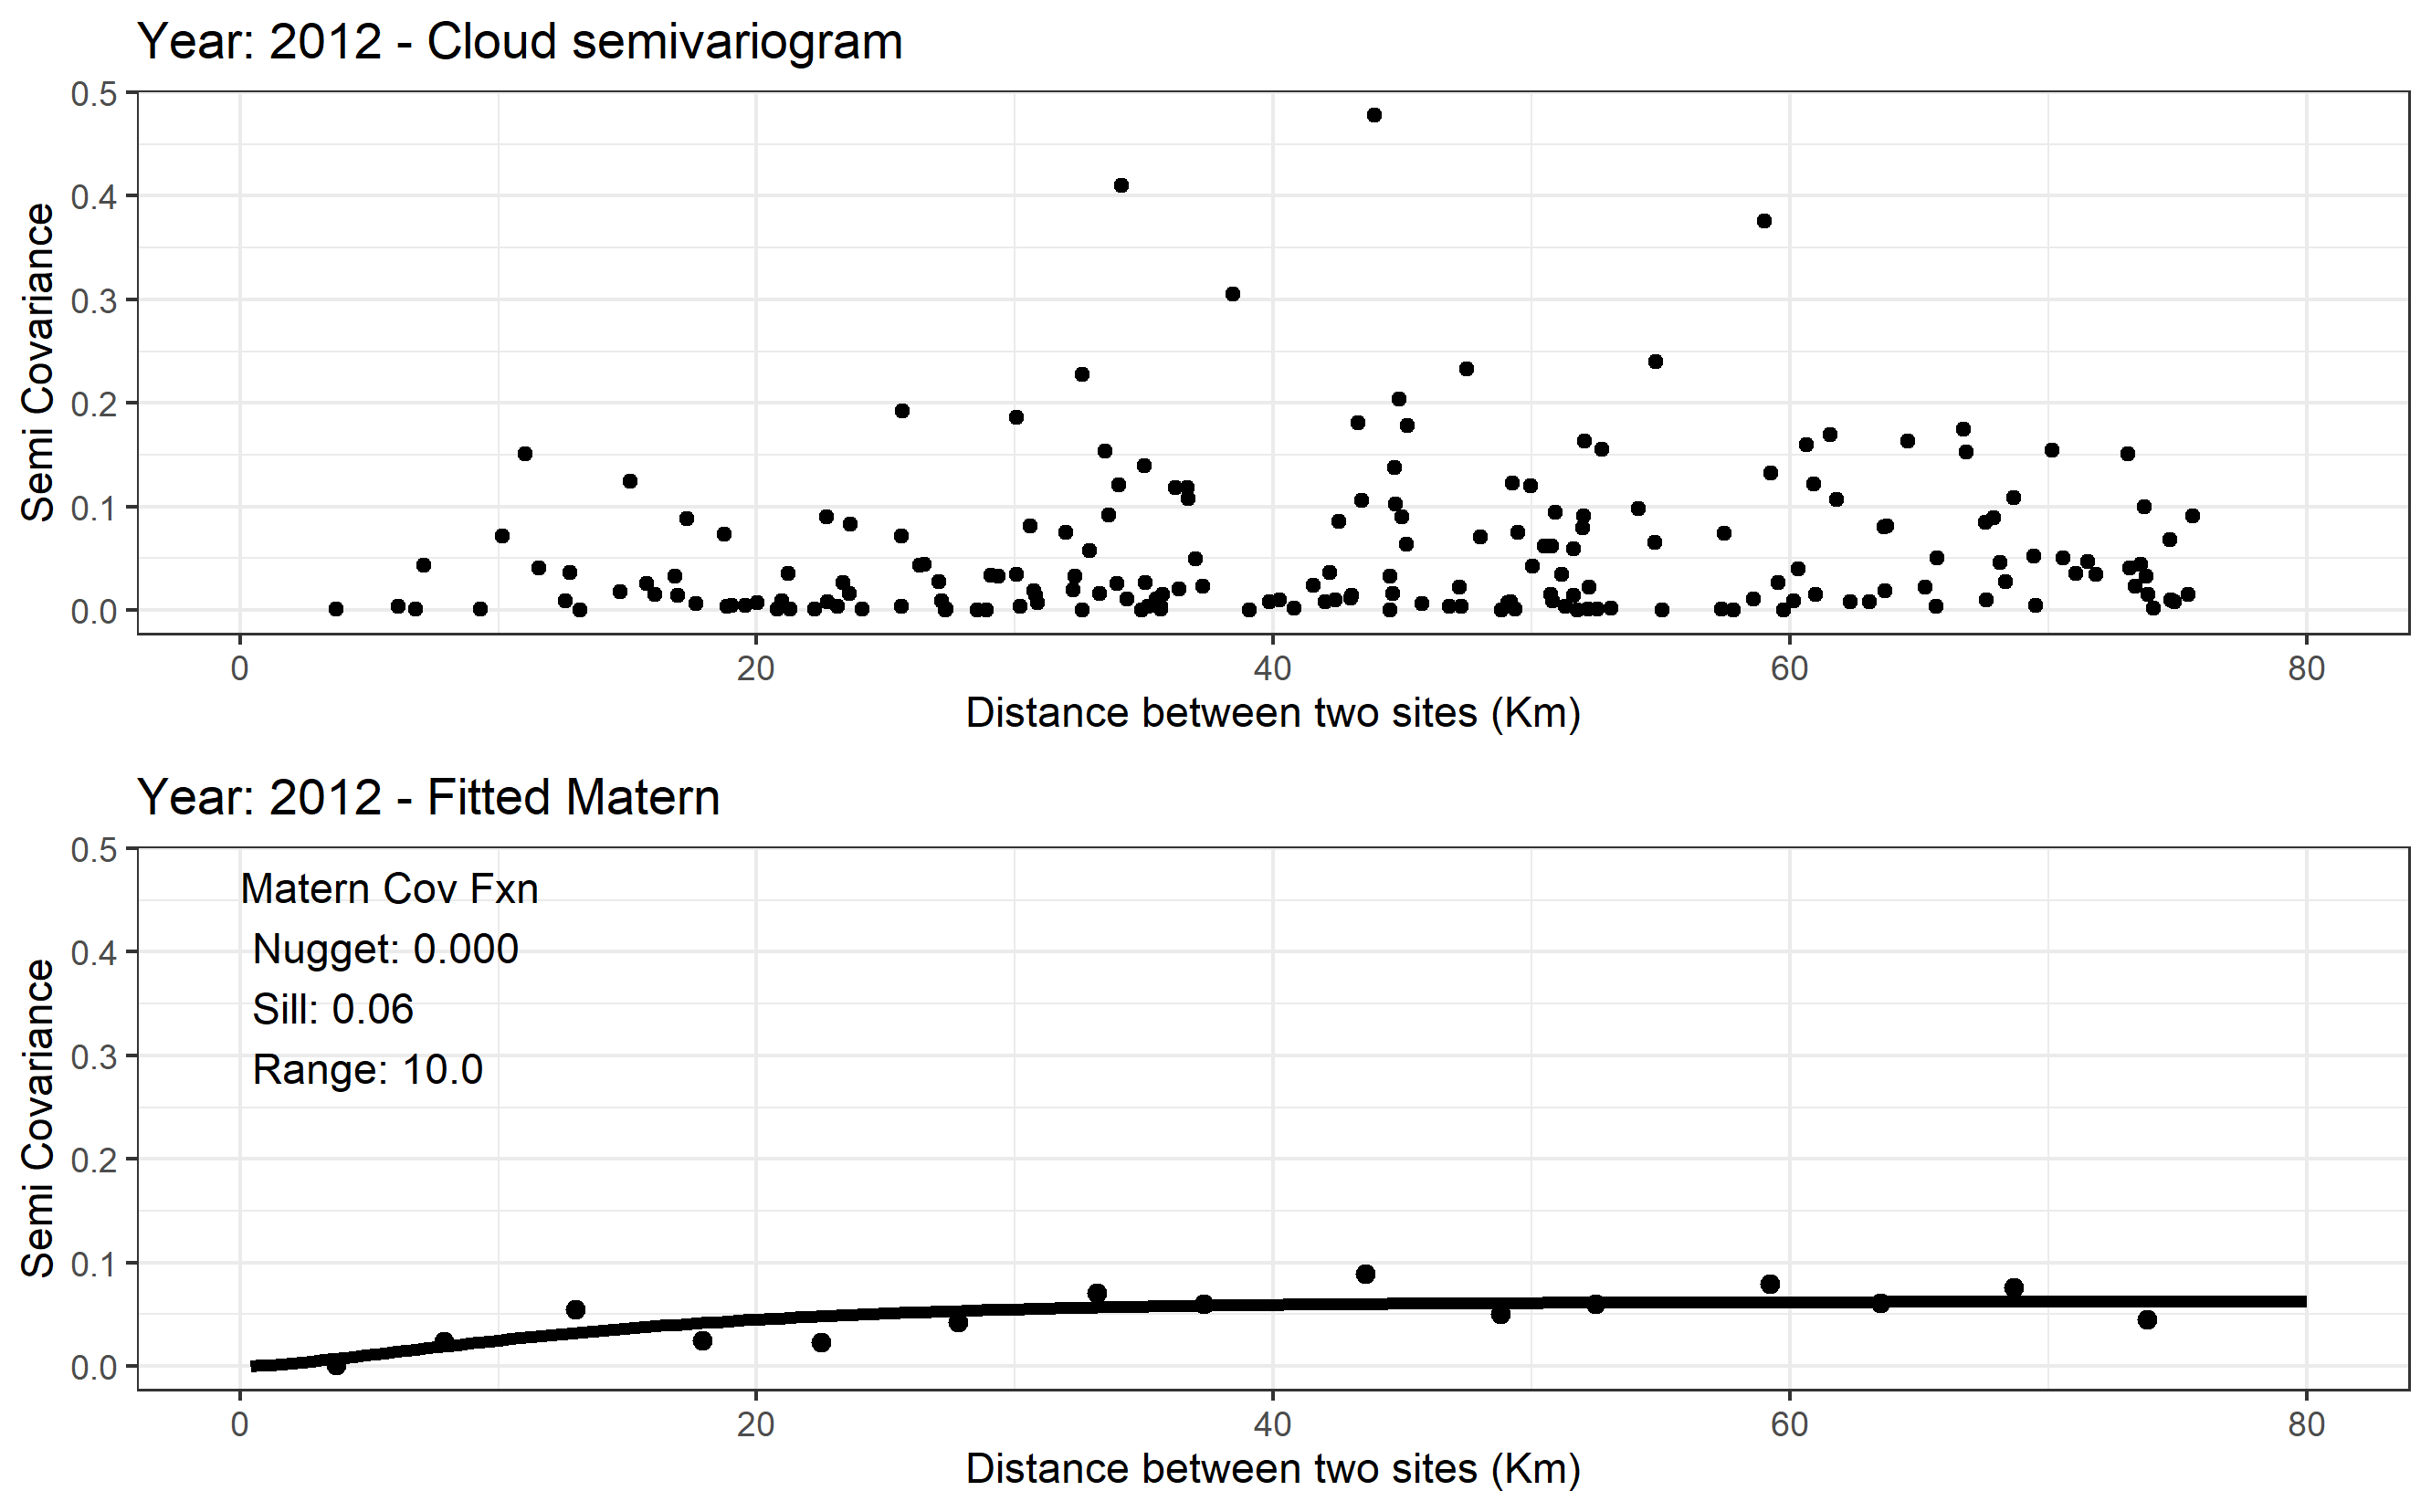}
    \caption{Caption}
    \label{fig:my_label}
\end{figure}

\begin{figure}
    \centering
    \includegraphics{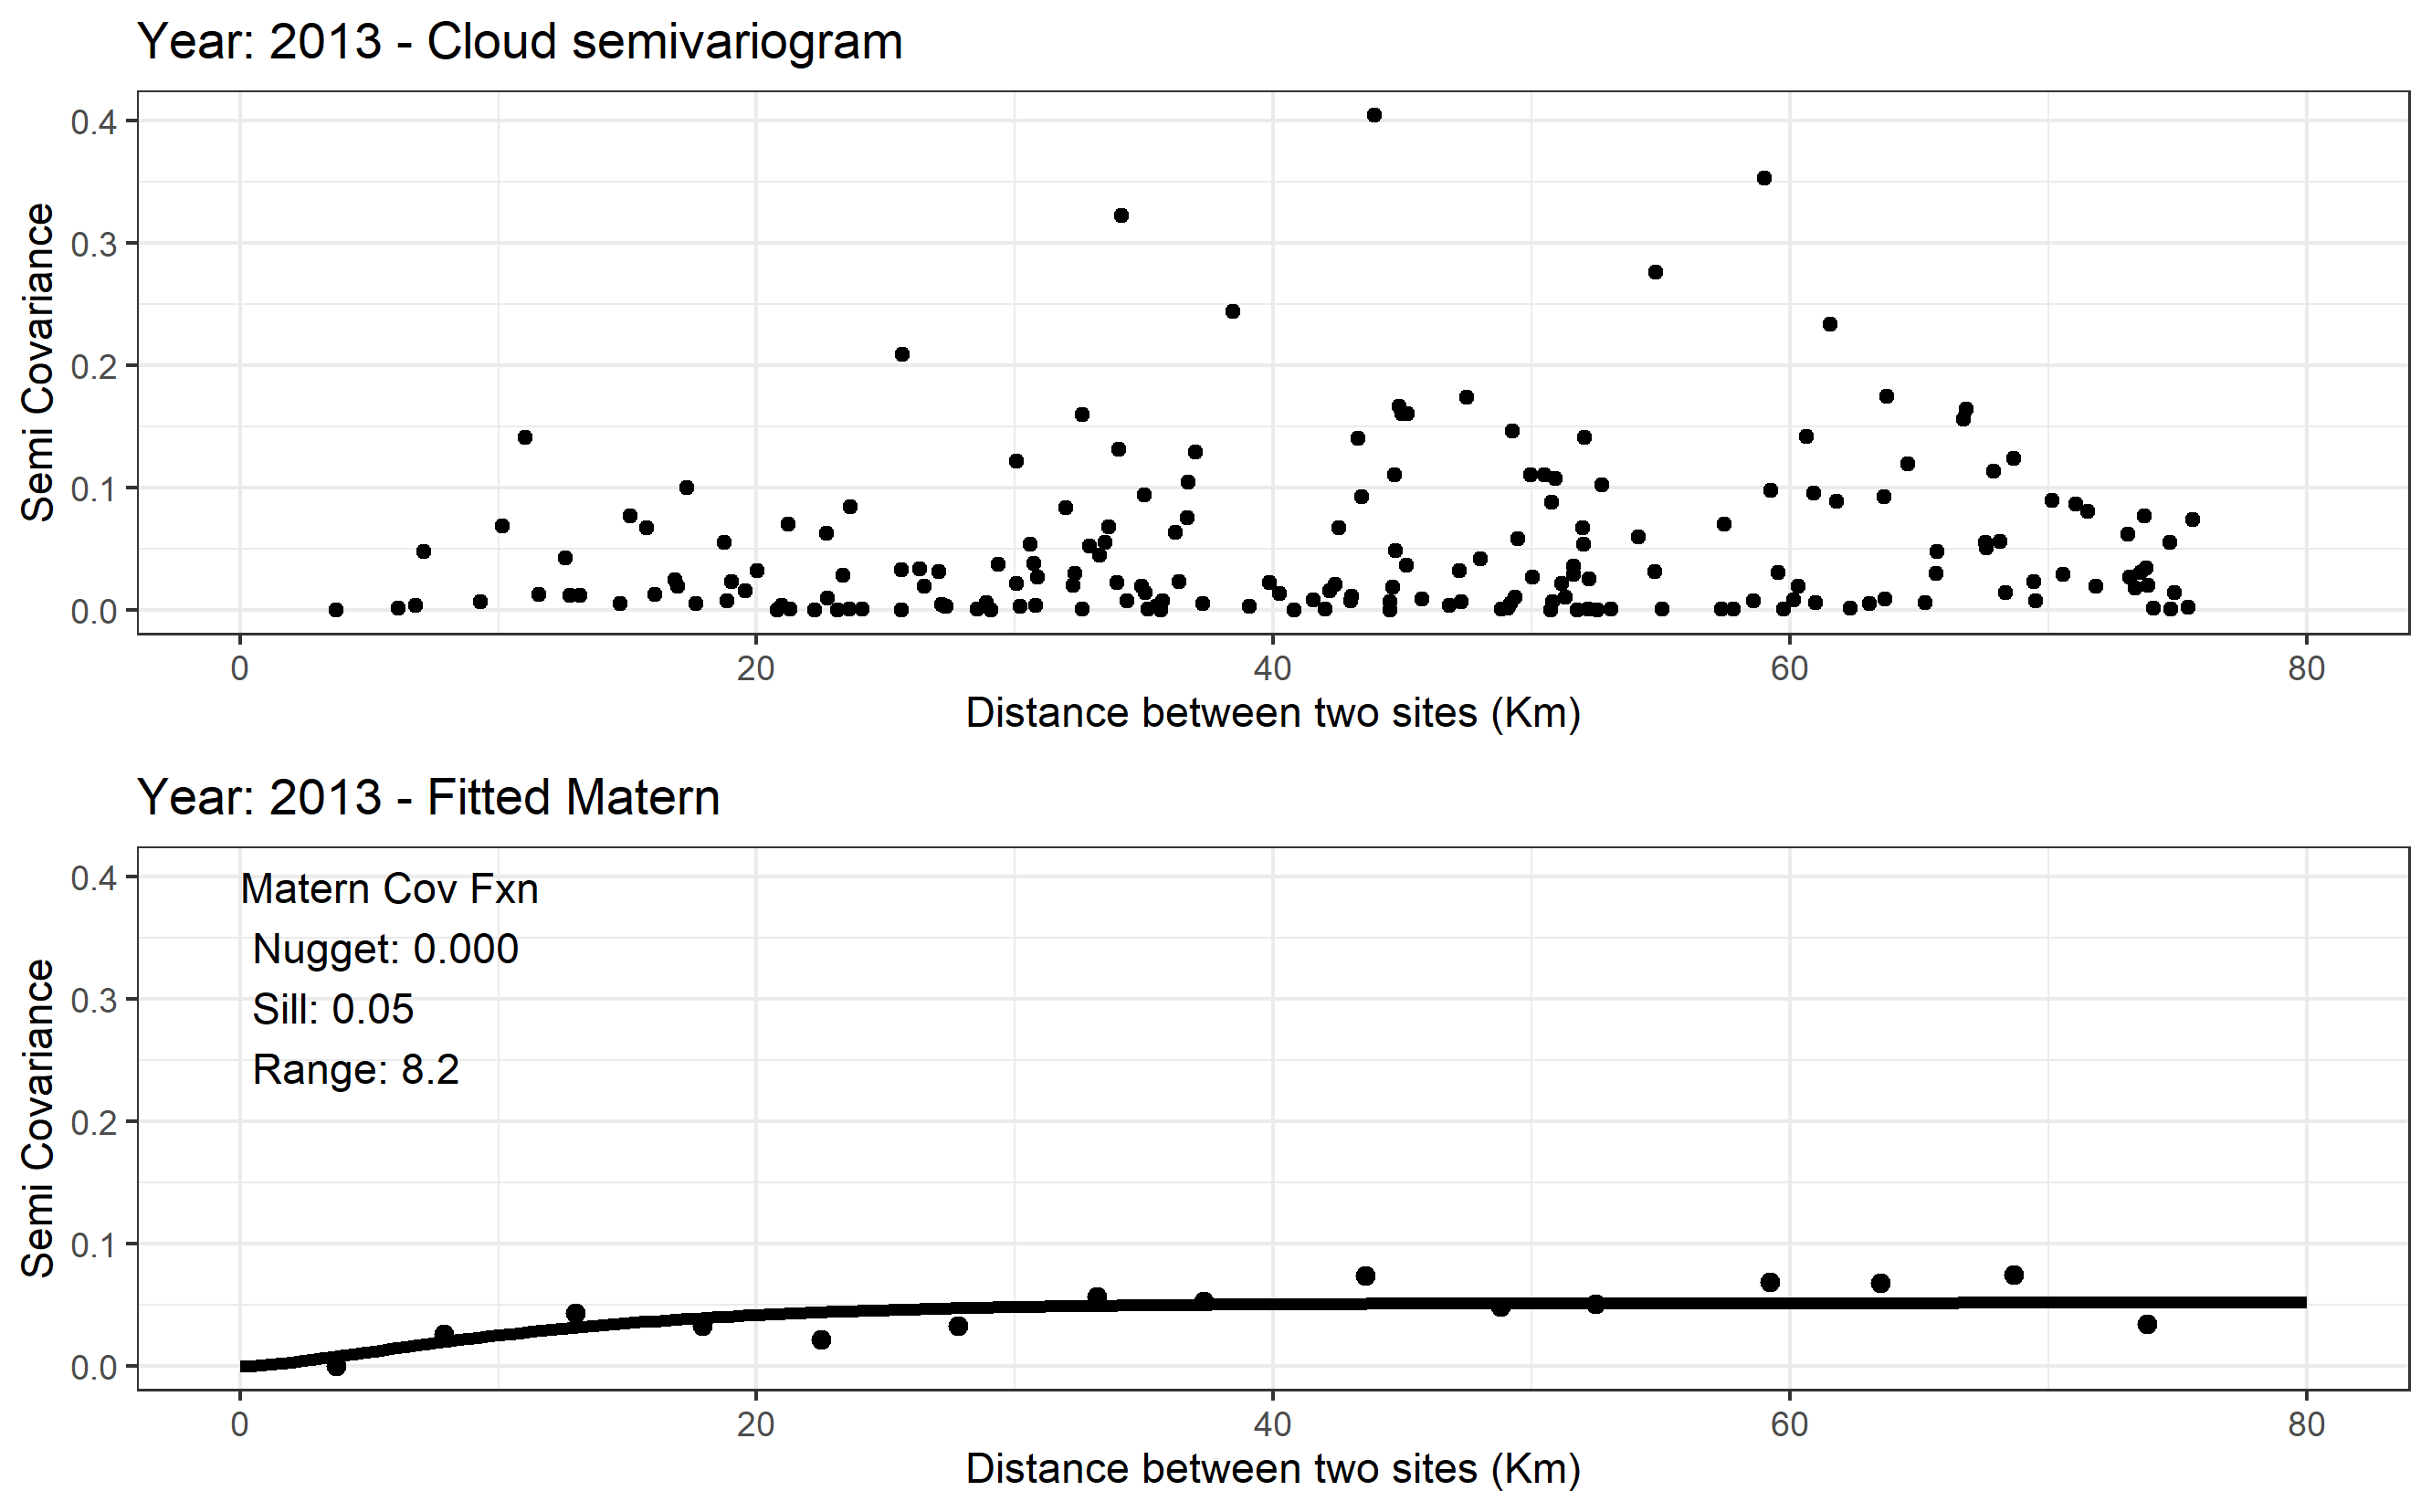}
    \caption{Caption}
    \label{fig:my_label}
\end{figure}

\begin{figure}
    \centering
    \includegraphics{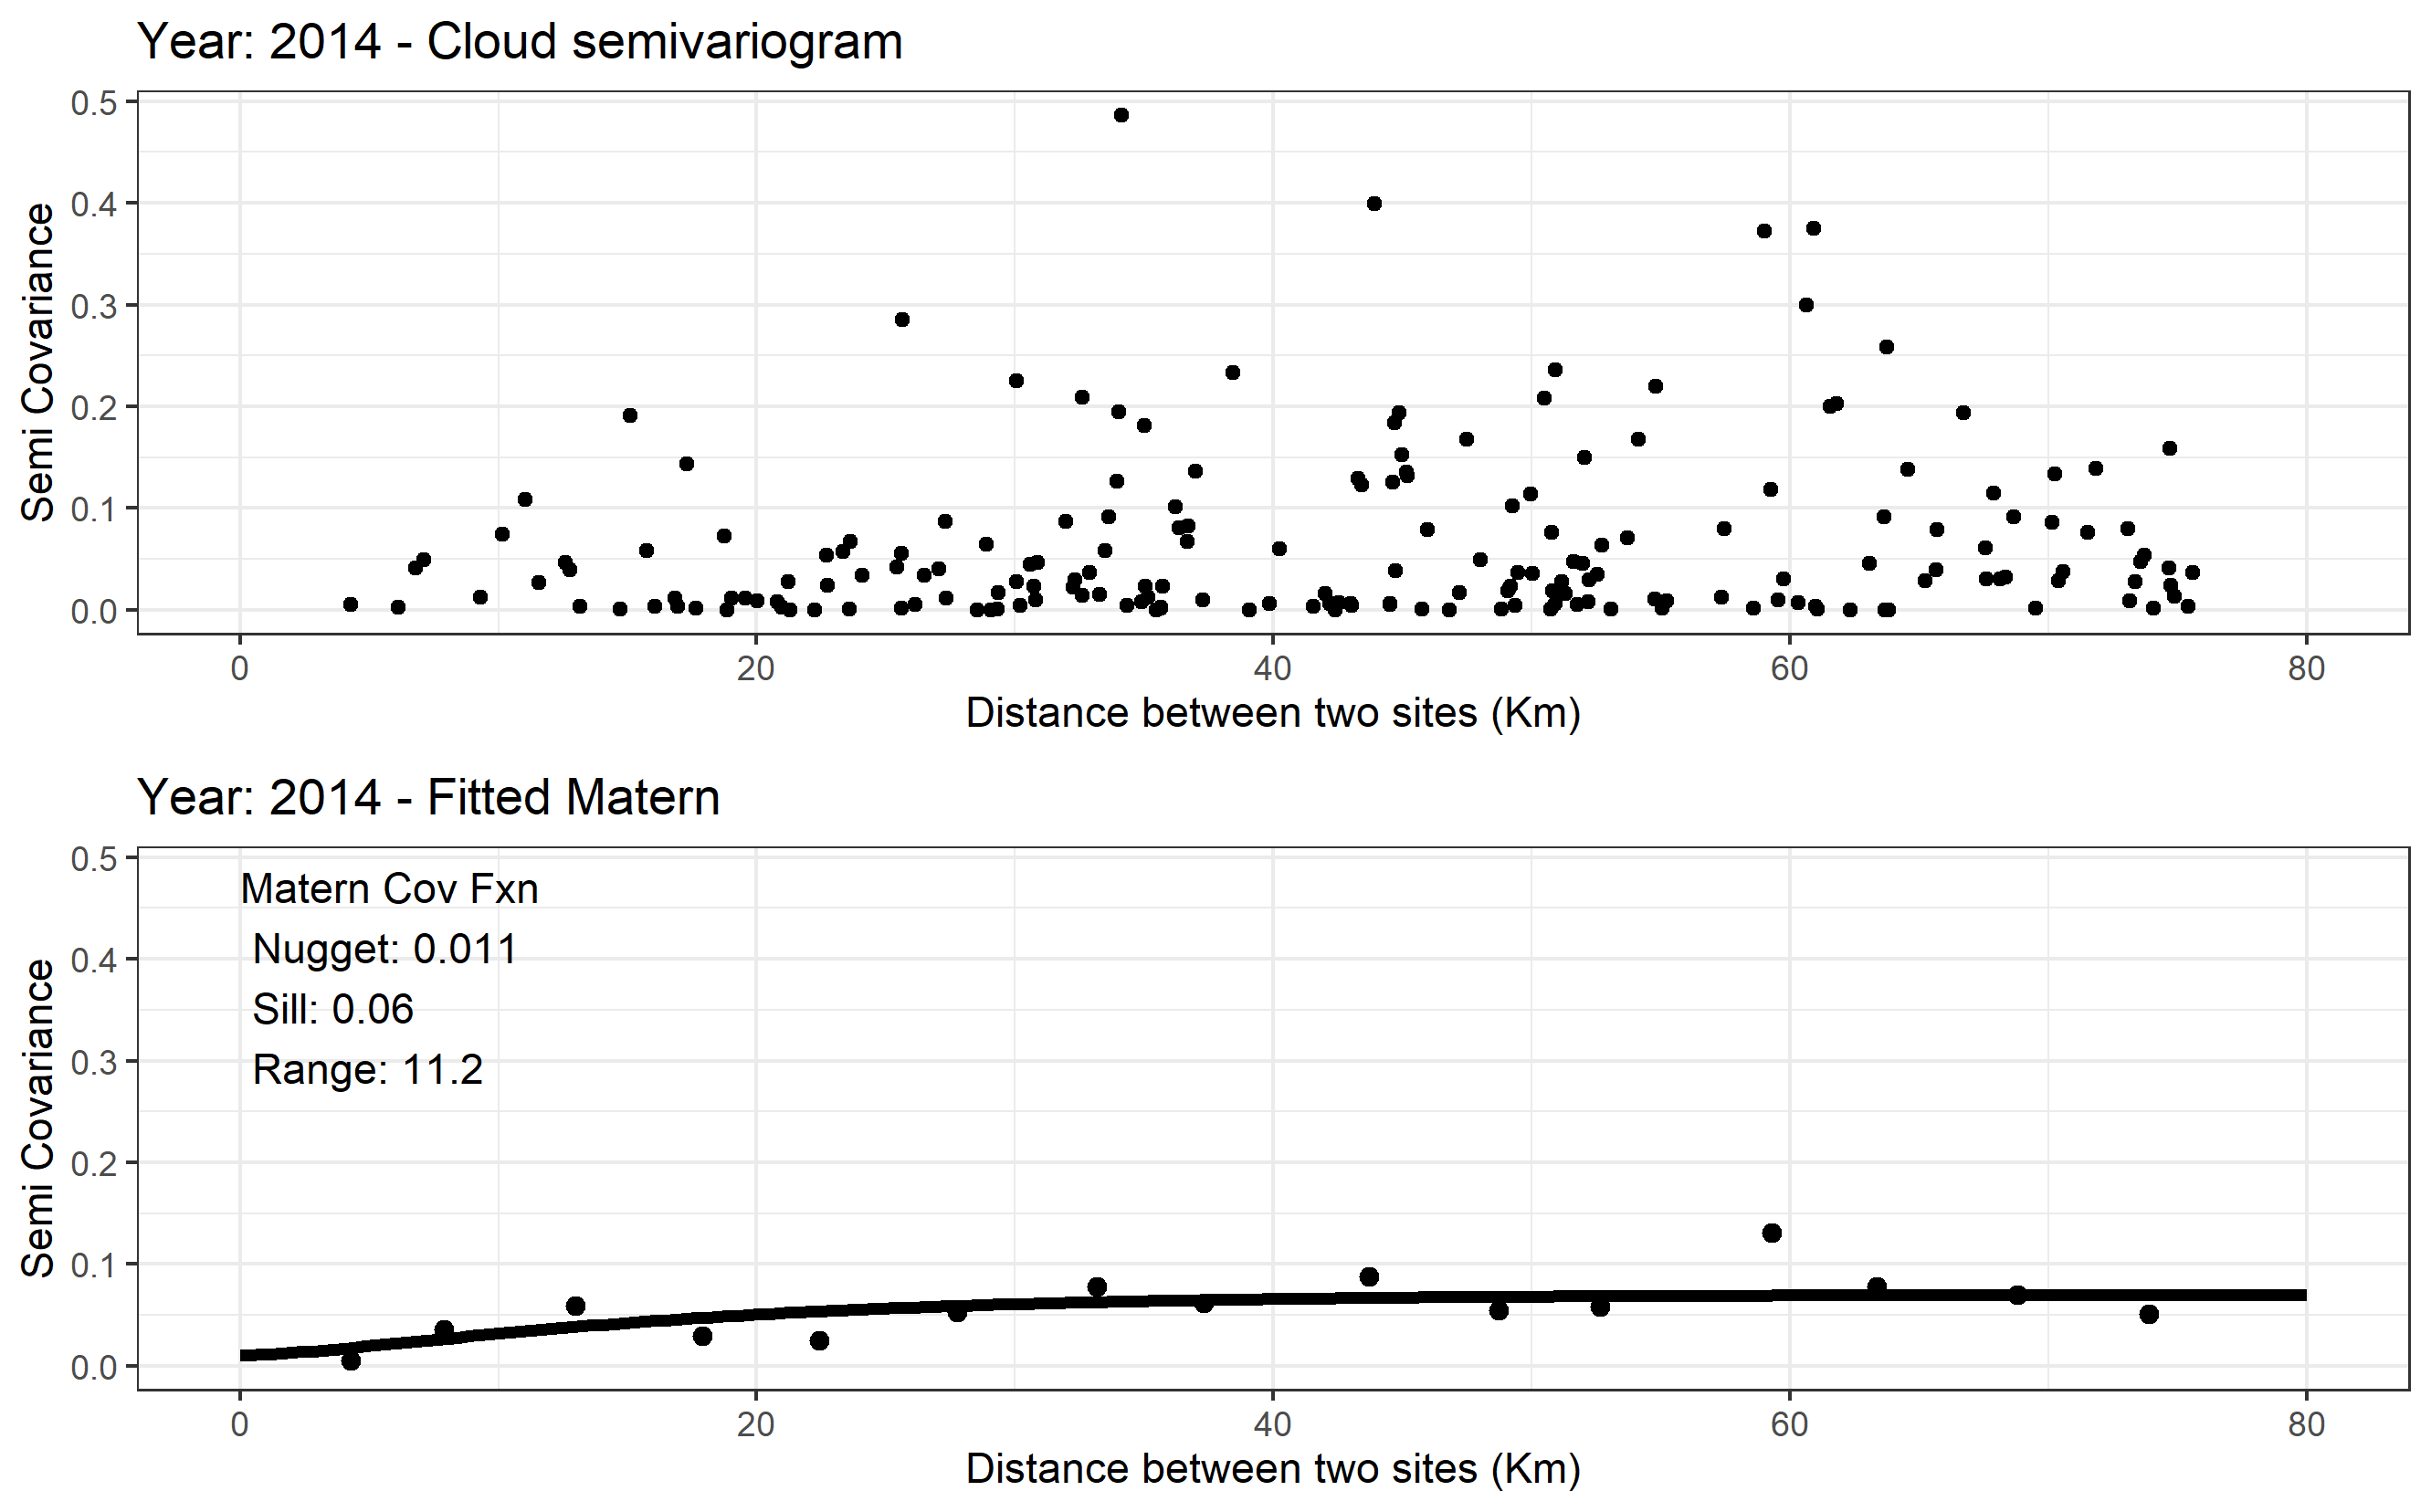}
    \caption{Caption}
    \label{fig:my_label}
\end{figure}

\begin{figure}
    \centering
    \includegraphics{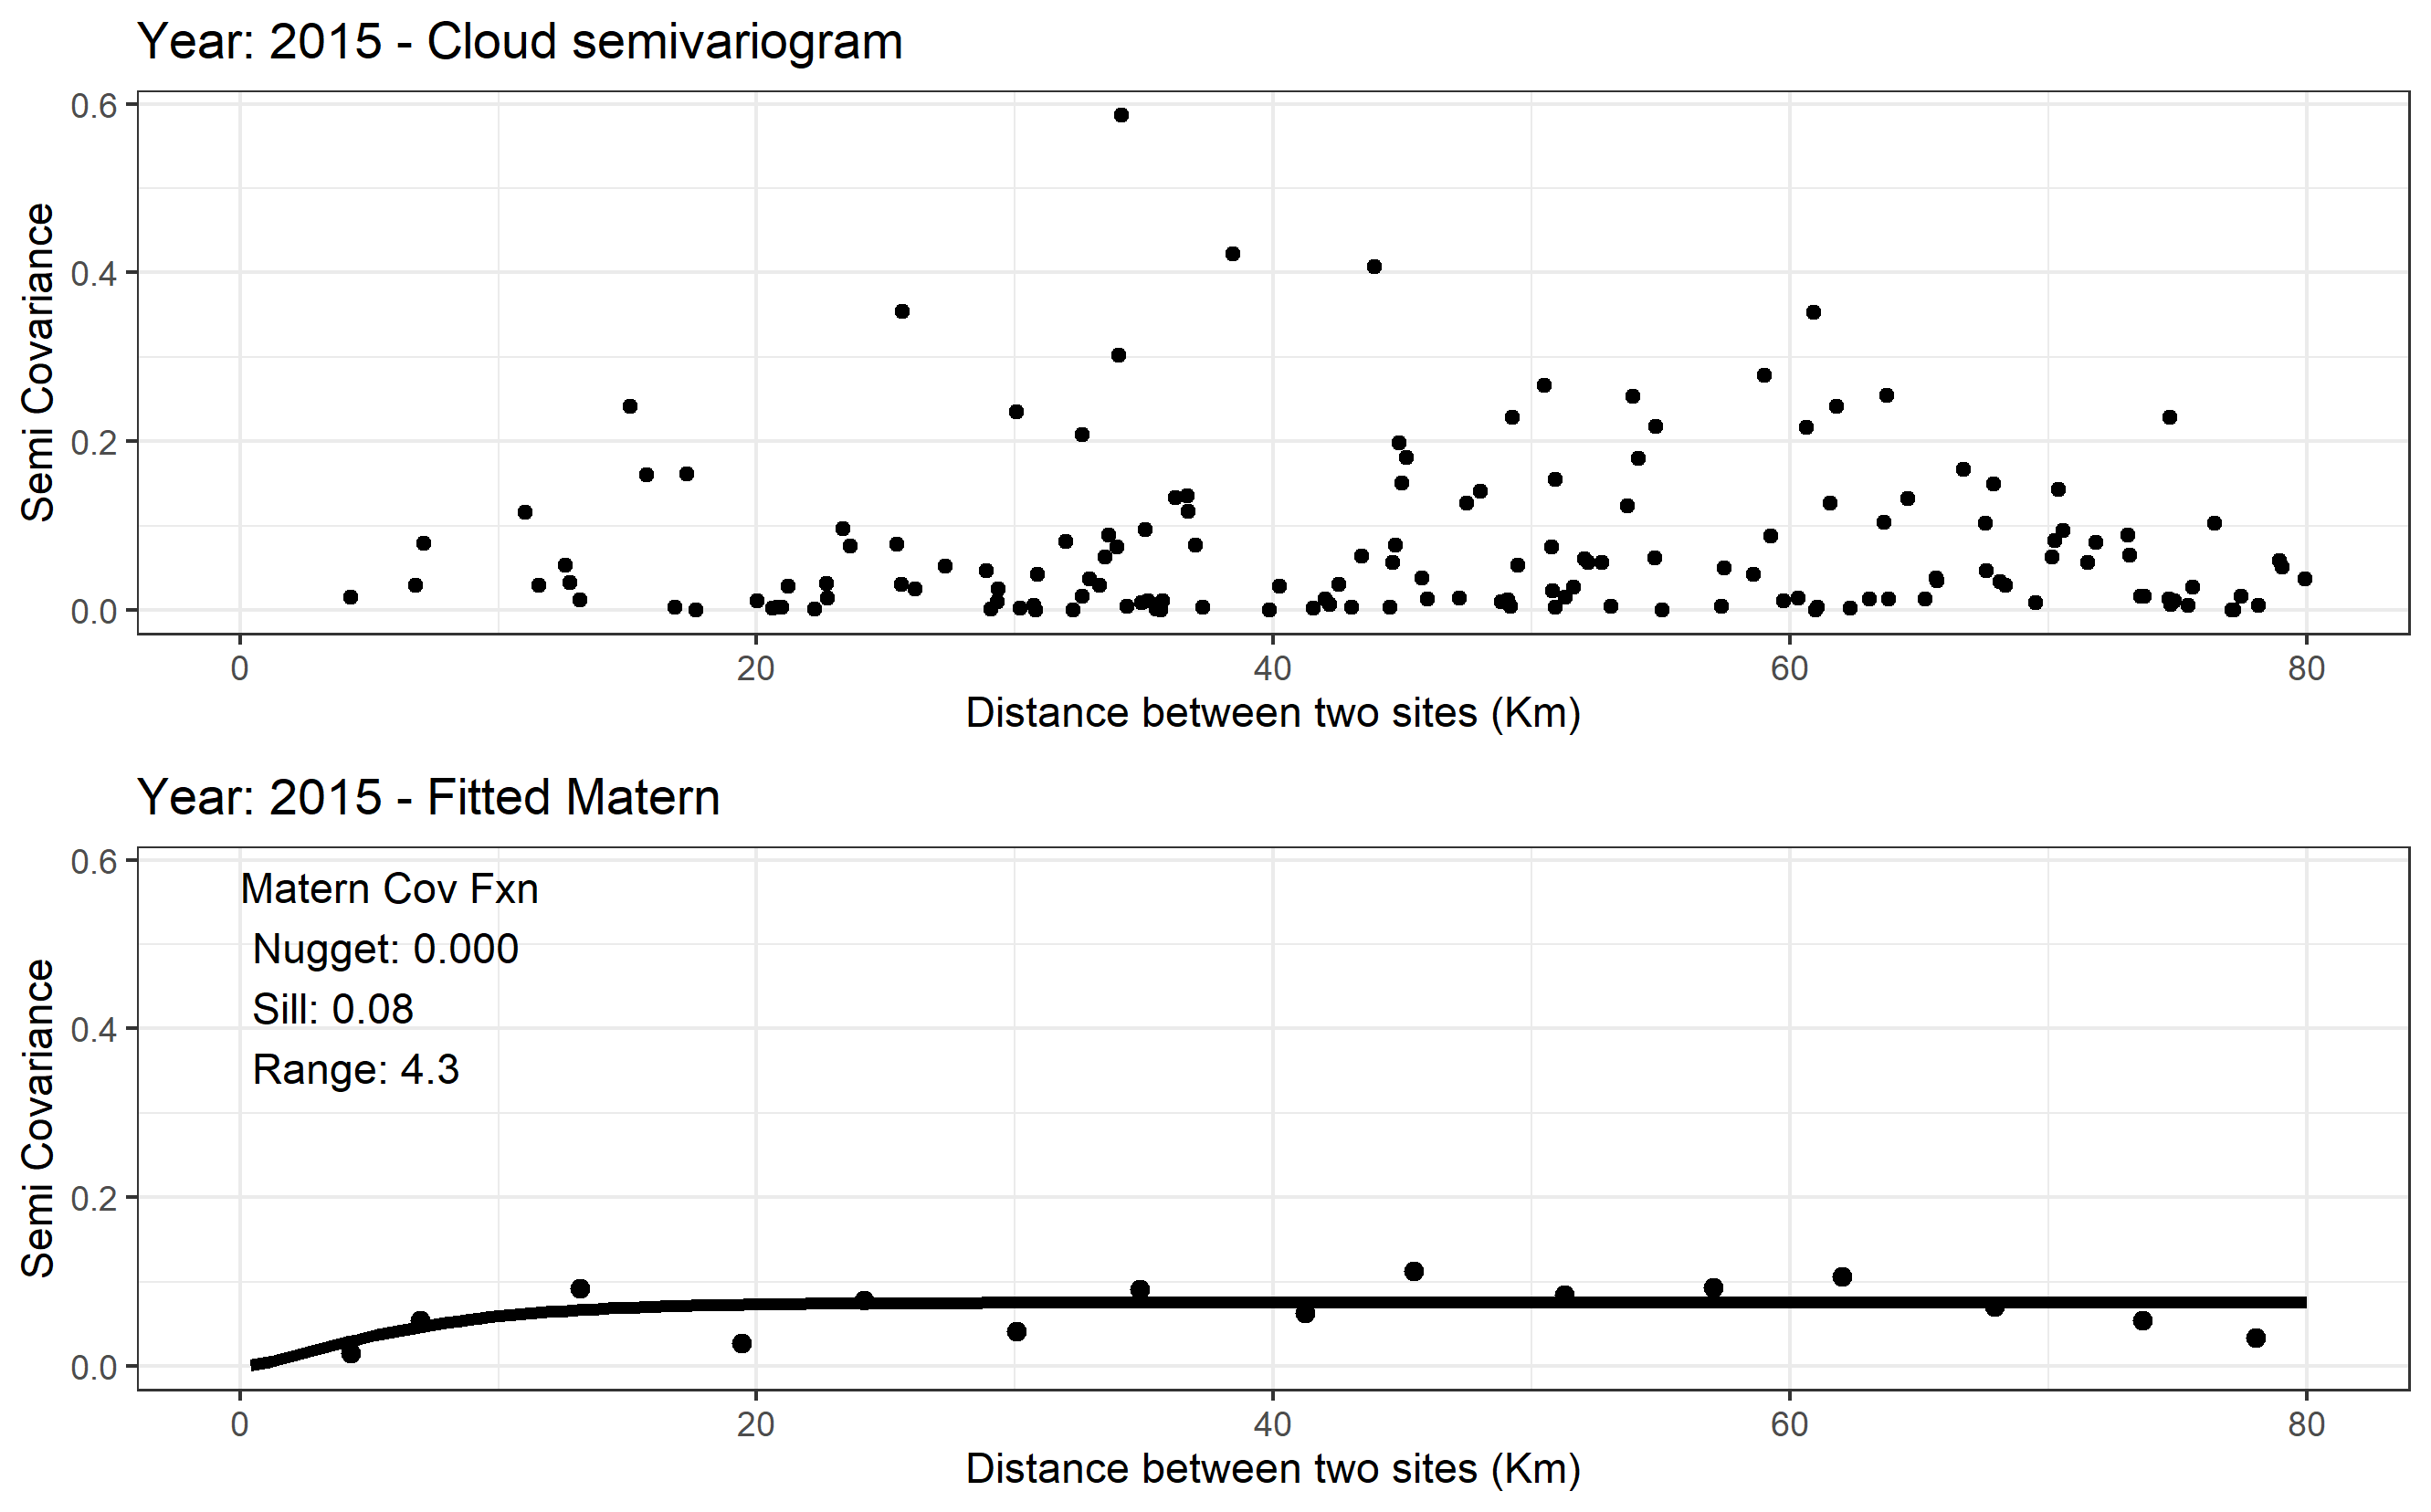}
    \caption{Caption}
    \label{fig:my_label}
\end{figure}

\begin{figure}
    \centering
    \includegraphics{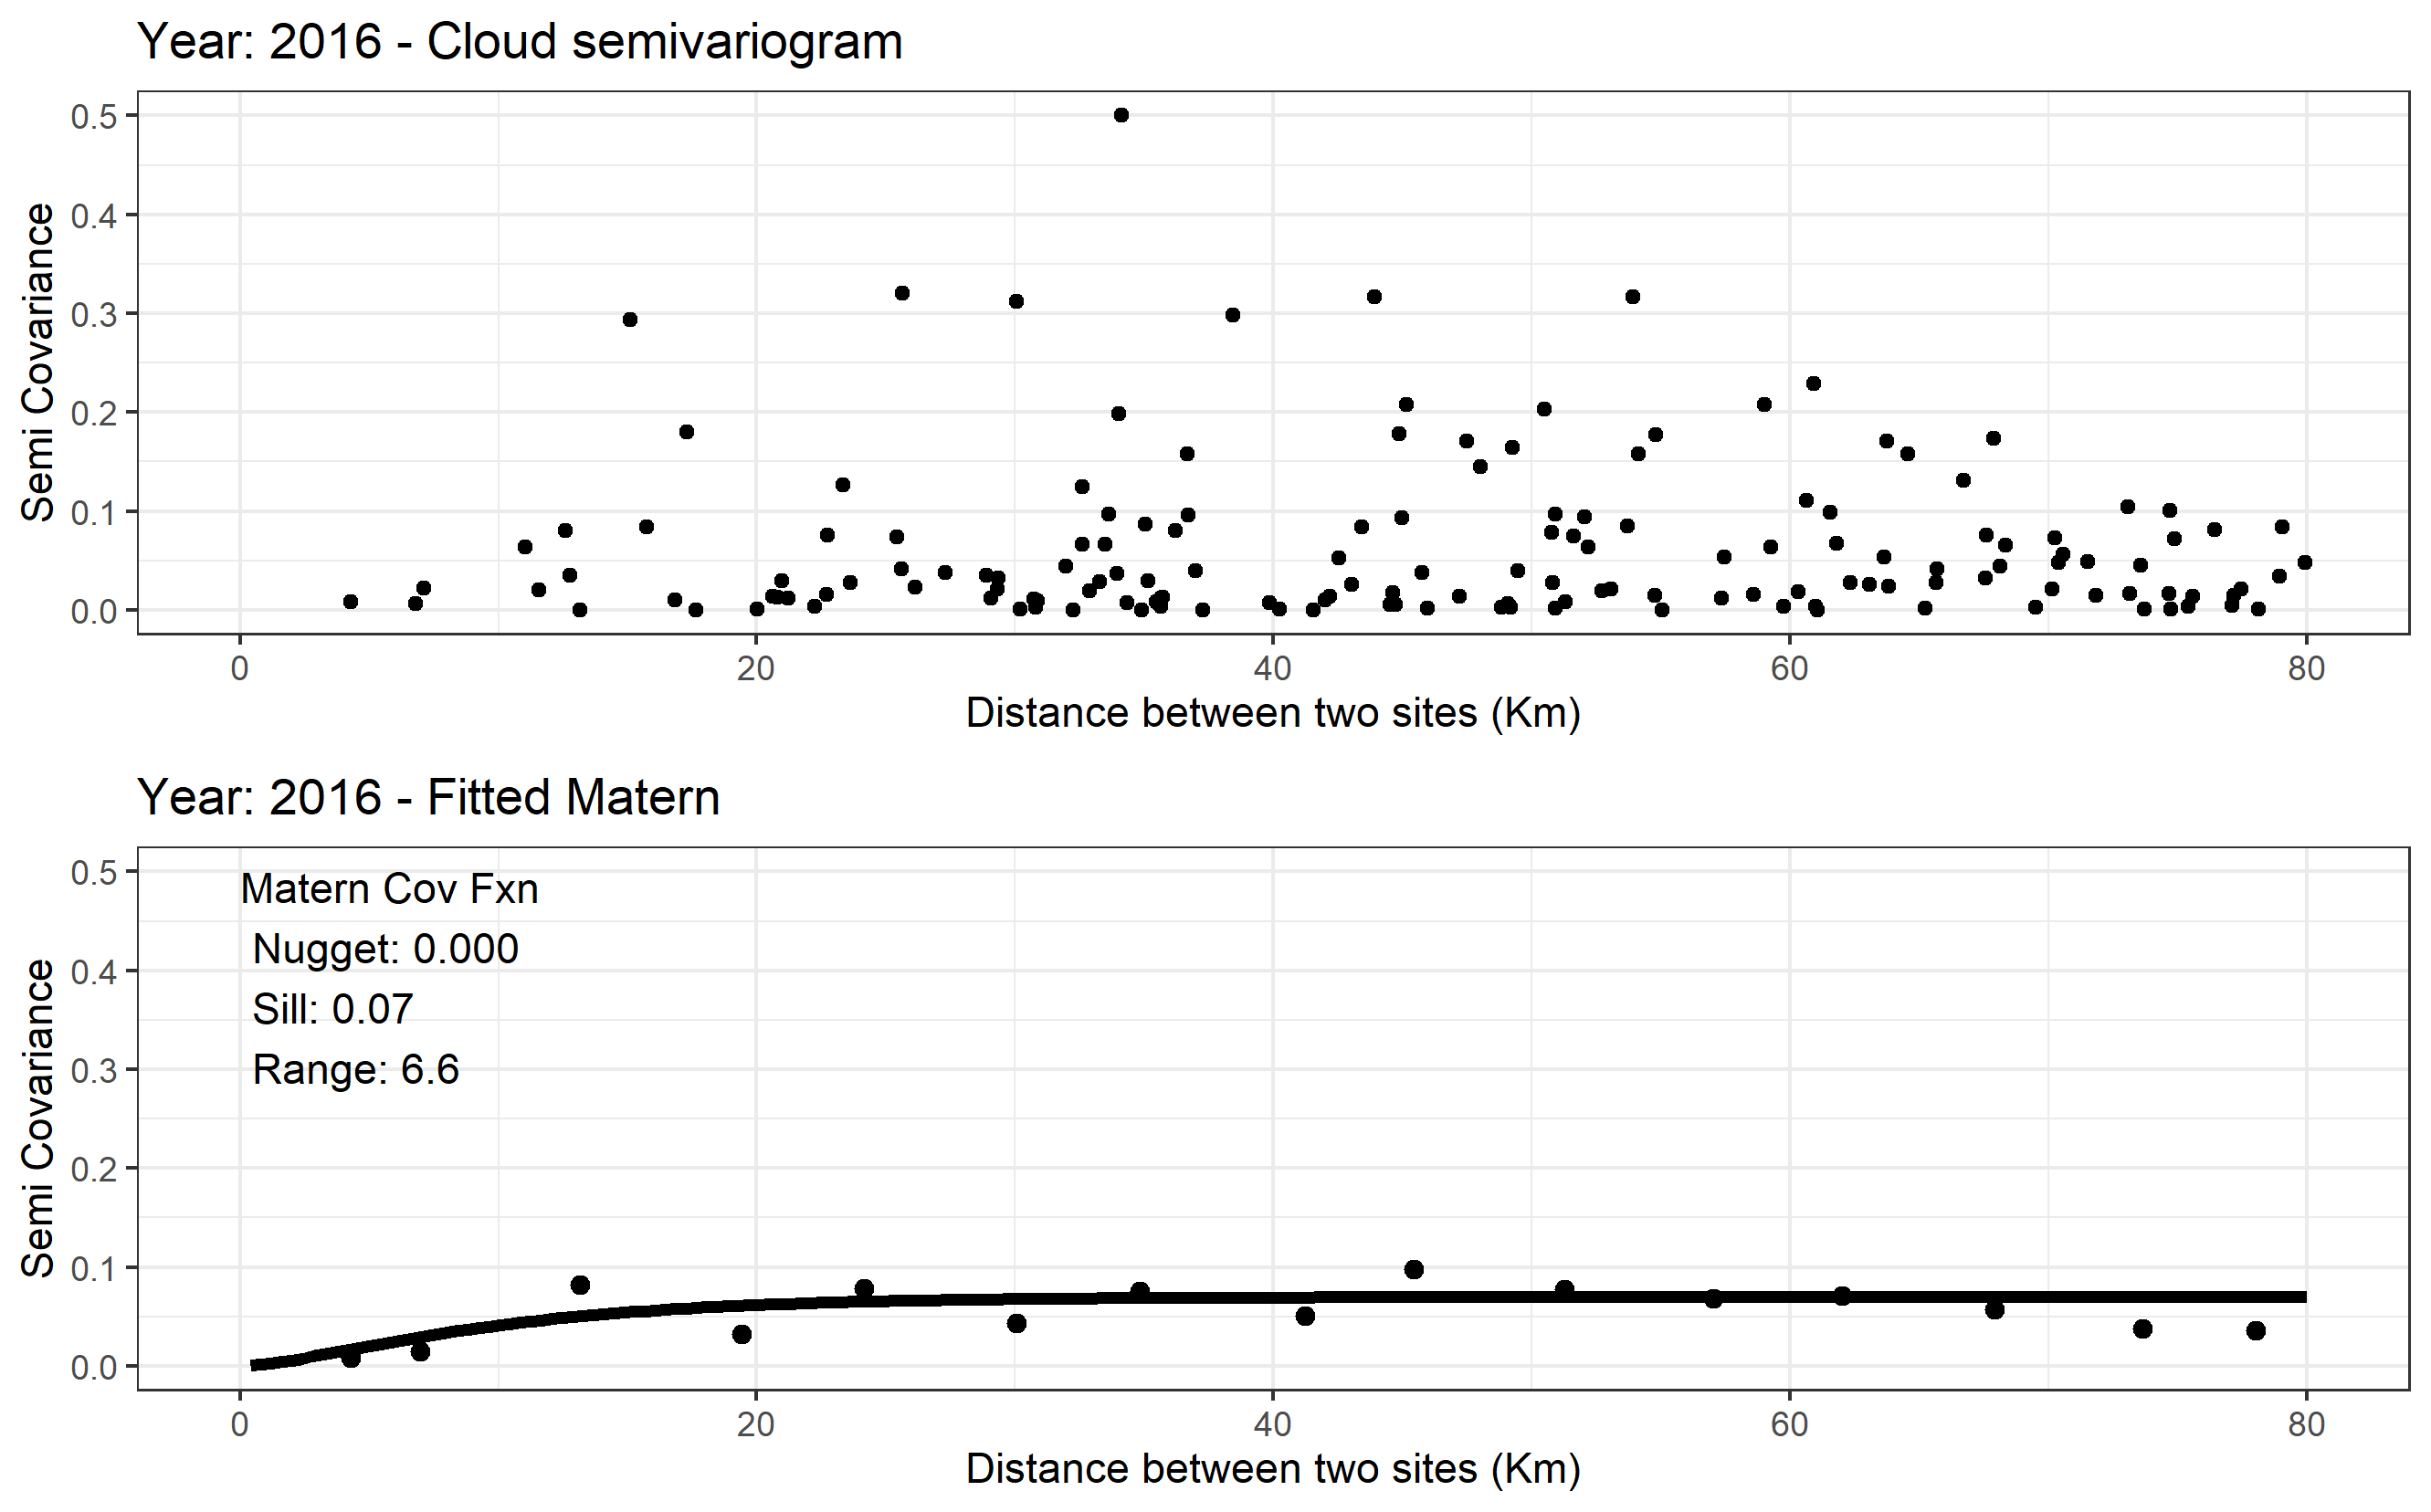}
    \caption{Caption}
    \label{fig:my_label}
\end{figure}

\begin{figure}
    \centering
    \includegraphics{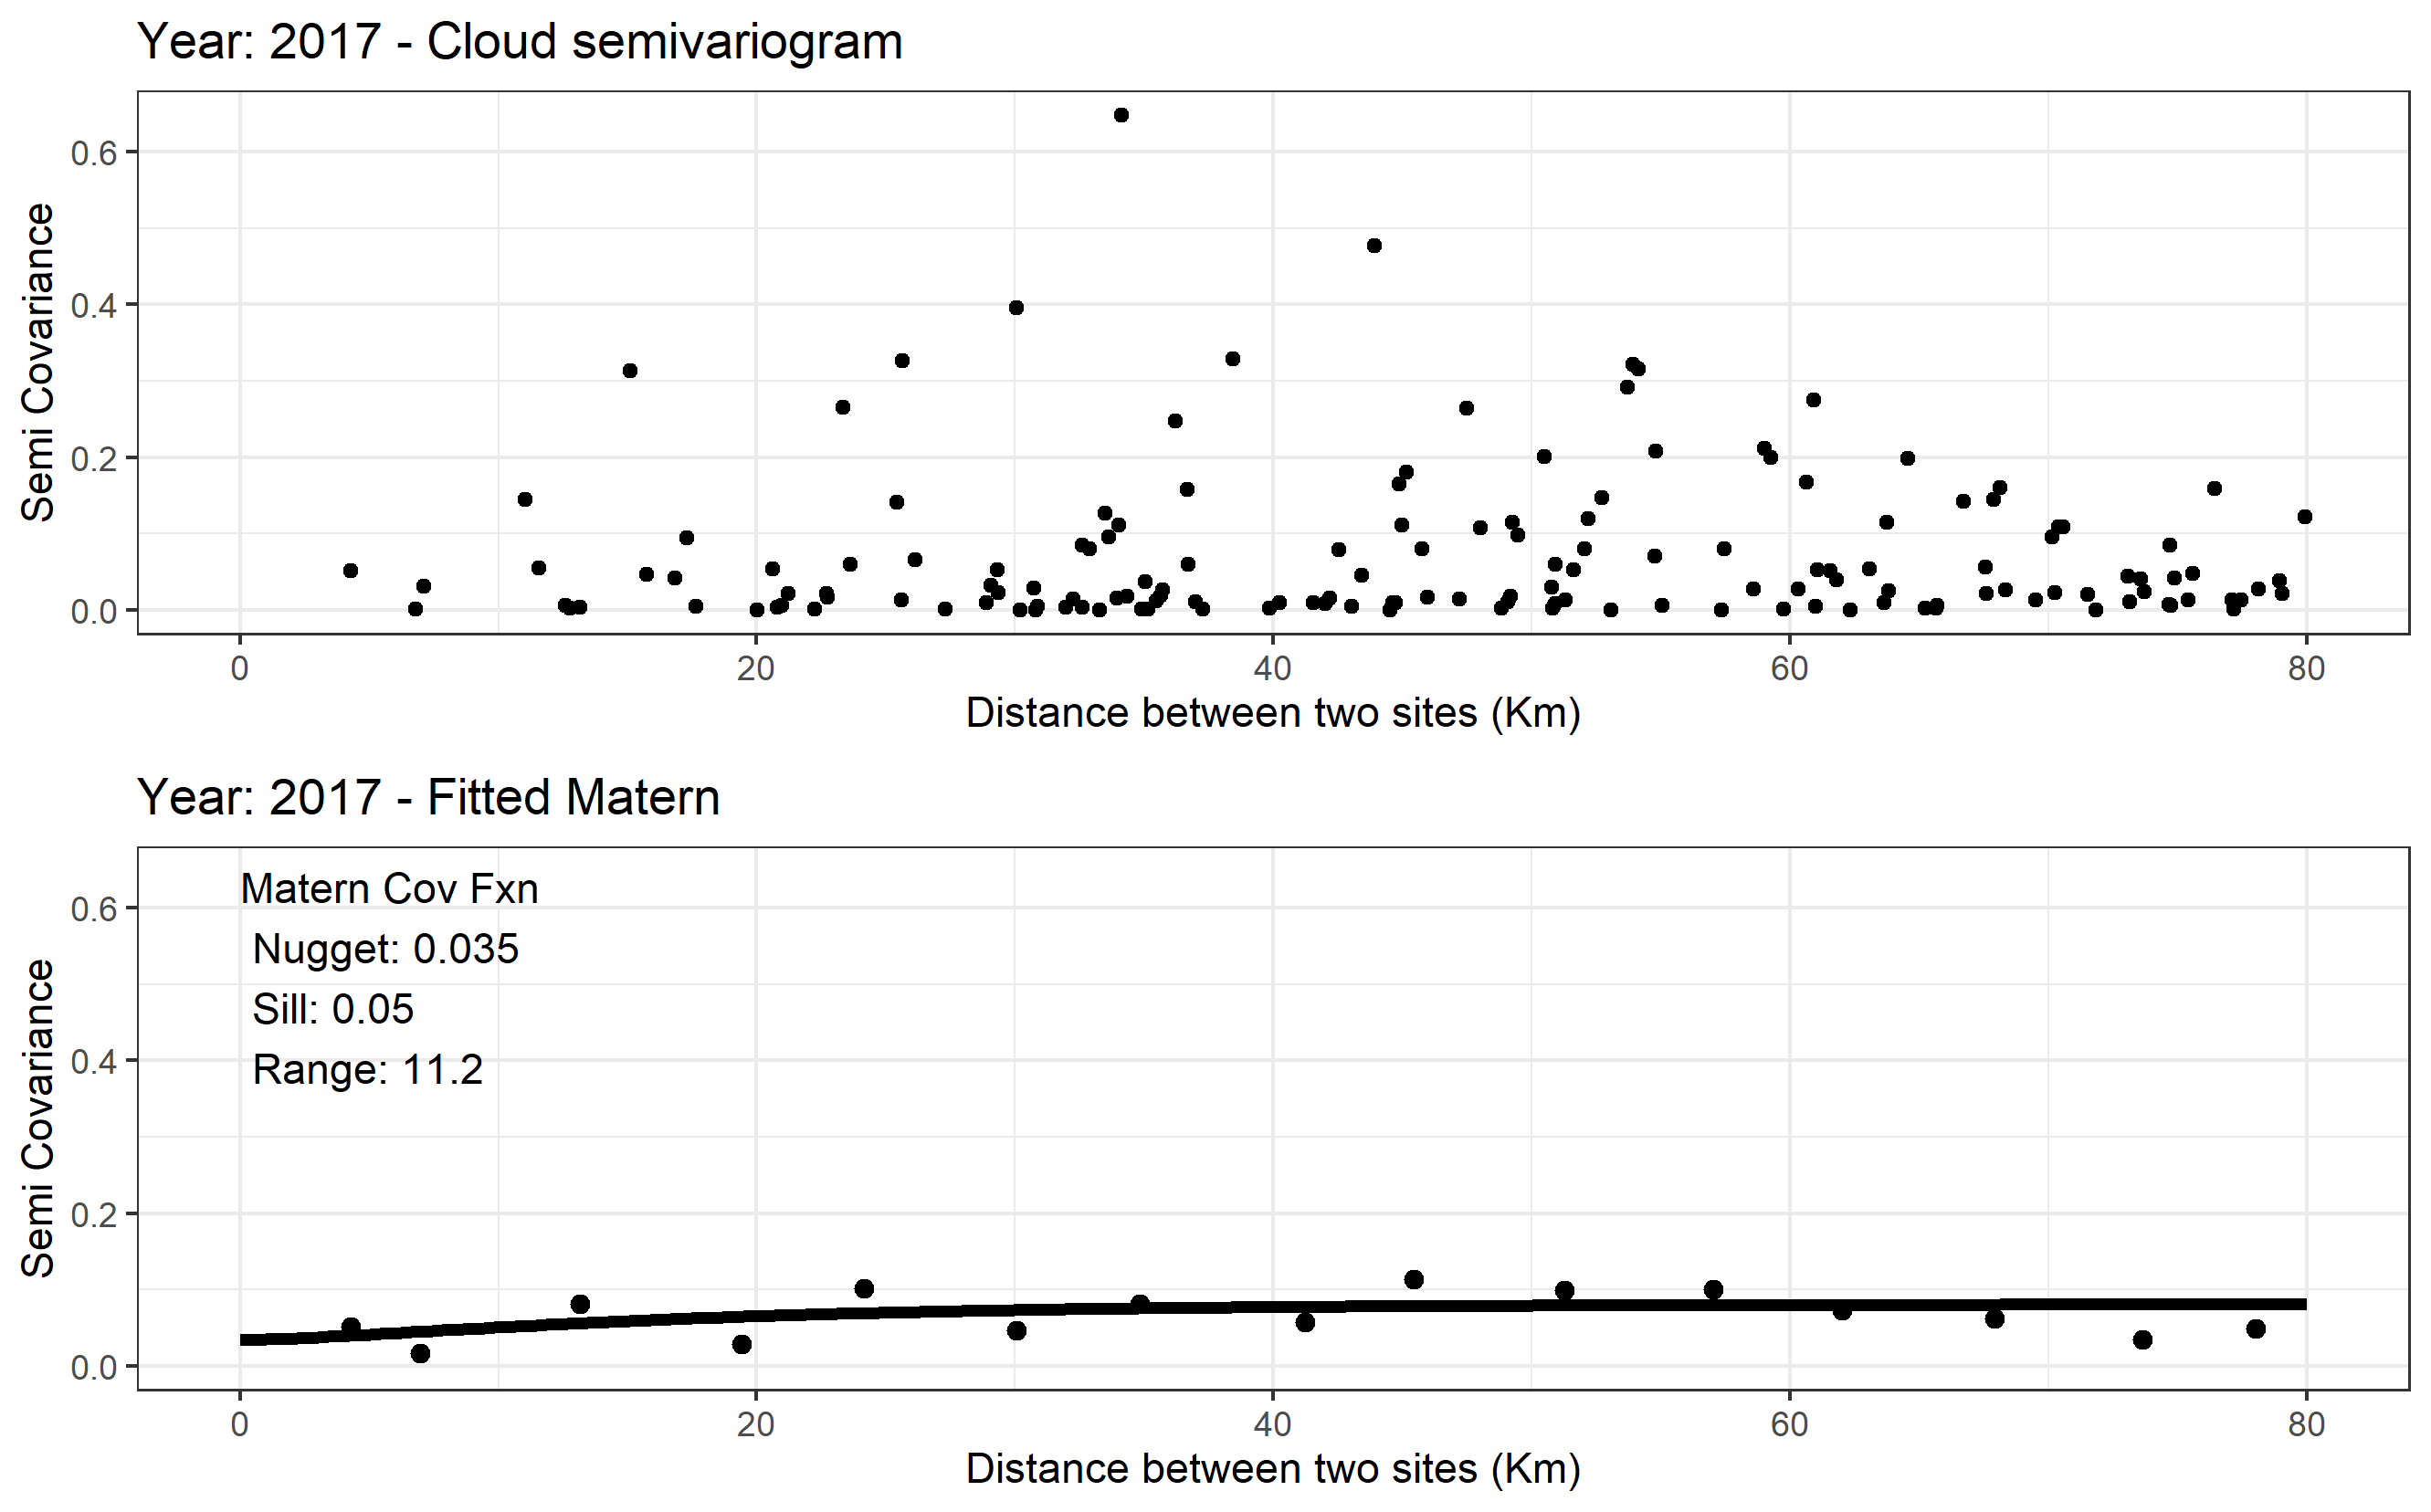}
    \caption{Caption}
    \label{fig:my_label}
\end{figure}

\begin{figure}
    \centering
    \includegraphics{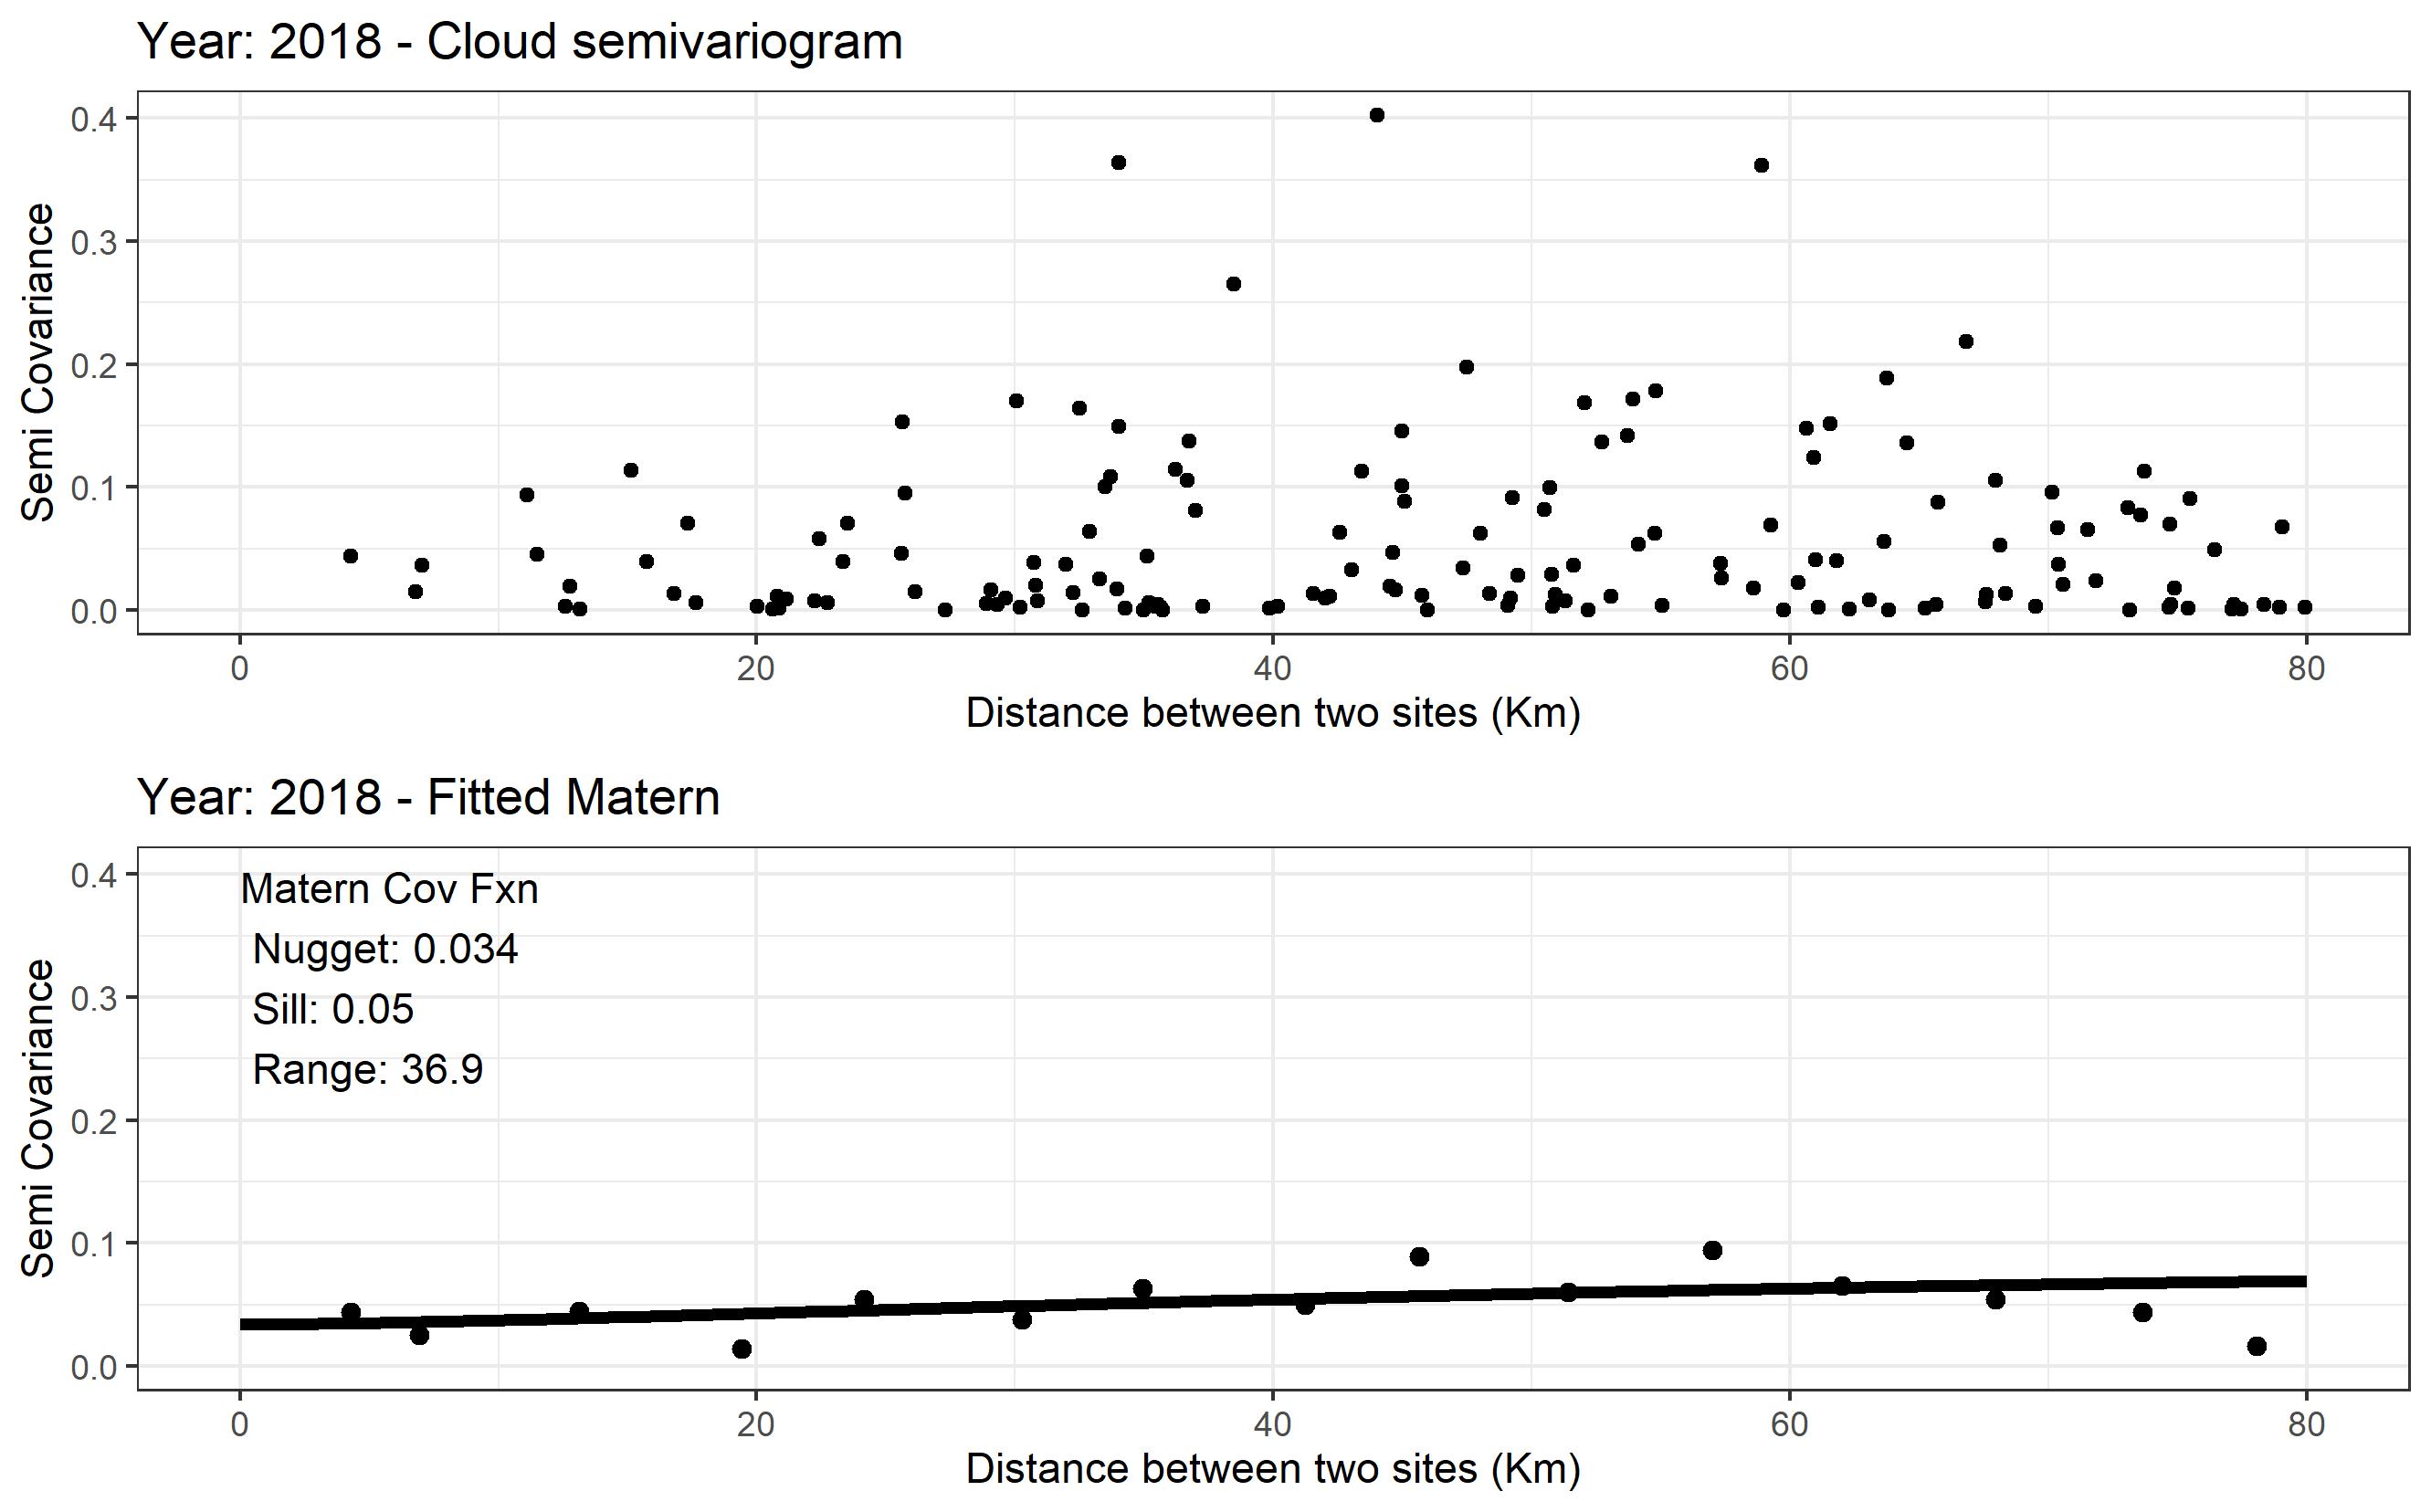}
    \caption{Caption}
    \label{fig:my_label}
\end{figure}

\begin{figure}
    \centering
    \includegraphics{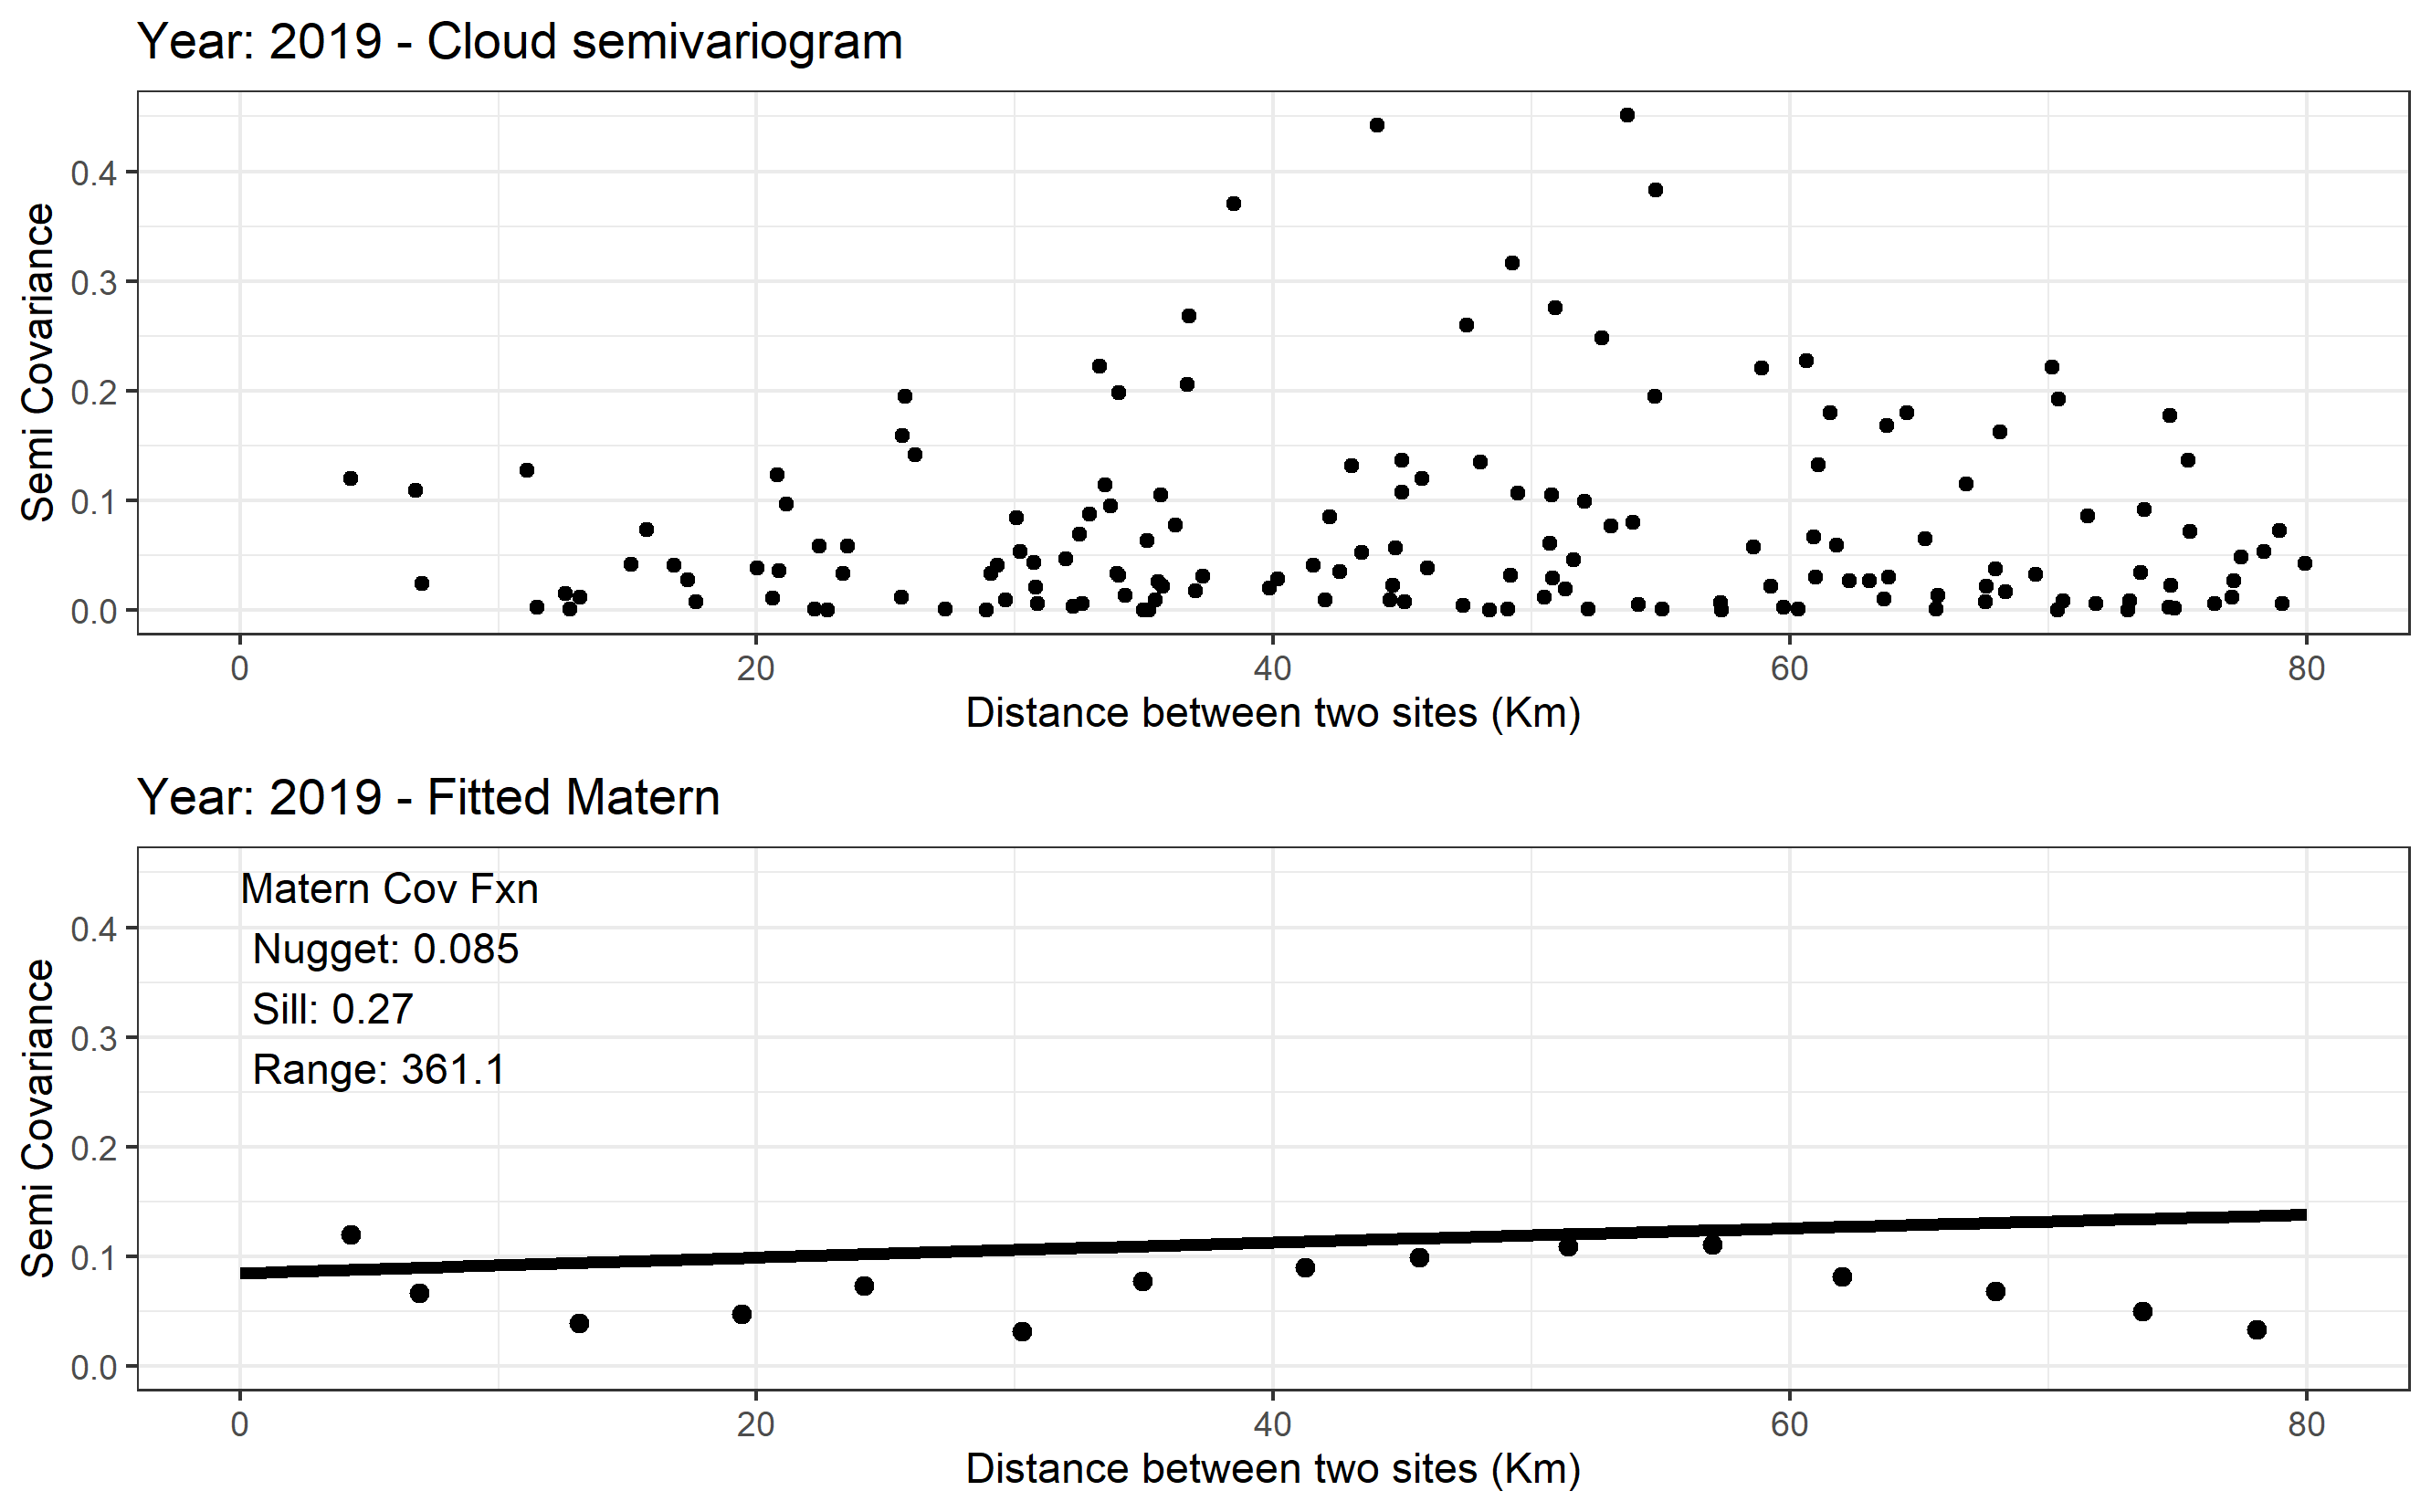}
    \caption{Caption}
    \label{fig:my_label}
\end{figure}
