# Supplementary material for: Preferential monitoring site location in the Southern California Air Quality Basin
Source: arXiv:2304.10006 source file (2023-04-19)
Supplement: Supplementary file 4 [file 99_AppendixD_MonitoringPurpose.tex]

The meaning of the Monitoring Purpose for each monitoring site as defined by the \ac{EPA}

\begin{itemize}
    \item Background Level monitoring is used to determine general background levels of air pollutants as they enter the Basin.
    \item High Concentration monitoring is conducted at sites to determine the highest concentration of an air pollutant in an area within the monitoring network. A monitoring network may have multiple high concentration sites (i.e., due to varying meteorology year to year).
    \item Pollutant Transport is the movement of pollutants between air basins or areas within an air basin. Transport monitoring is used to assess and mitigate upwind areas when transported pollutant affects neighboring downwind areas. Also, transport monitoring is used to determine the extent of regional pollutant transport among populated areas and to rural areas.
    \item Population Exposure monitoring is conducted to represent the air pollutant concentrations that a populated area is exposed to.
    \item Representative concentration monitoring is conducted to represent the air quality concentrations for a pollutant expected to be similar throughout a geographical area. These sites do not necessarily indicate the highest concentrations in the area for a particular pollutant.
    \item Source impact monitoring is used to determine the impact of significant sources or source categories of air quality emissions on ambient air quality. The air pollutant sources may be stationary or mobile.
    \item Trend analysis monitoring is useful for comparing and analyzing air pollution concentrations over time. Usually, trend analyses can be used to assess the progress in improving air quality for an area over a period of many years.
    \item Site Comparison monitoring is used to assess the effect on measured pollutant levels of moving a monitoring location a short distance (usually less than two miles). Some monitoring stations become no longer usable due to development, change of lease terms, or eviction. In these cases, attempts are made to conduct concurrent monitoring at the old and new site for a period of at least one year in order to compare pollutant concentrations.
    \item Real Time Reporting/Modelling is used to provide data to U.S. EPA’s AIRNOW system which reports conditions for air pollutants on a real-time basis to the general public. Data is also used to provide accurate and timely air quality forecast guidance to residents of the Basin.
\end{itemize}
\cite{AQMNP:2019}
